# Supplementary material for: $B \to \rho \ell \bar{\nu}$ resonance form factors from $B \to \pi\pi \ell \bar{\nu}$ in lattice QCD
Source: arXiv:2501.00903 ancillary file (2025-04-28)
Supplement: Supplementary file 1 [file supplemental_material.pdf]

## Supplemental Material for
## "$B \to \rho \ell \bar{\nu}$ resonance form factors from $B \to \pi\pi \ell \bar{\nu}$ in lattice QCD"


Luka Leskovec,[1,2,*] Stefan Meinel,[3,†] Marcus Petschlies,[4] John Negele,[5] Srijit Paul,[6] and Andrew Pochinsky[5]

[1]*Faculty of Mathematics and Physics, University of Ljubljana, Jadranska 19, 1000*
[2]*Jožef Stefan Institute, Jamova 39, 1000 Ljubljana, Slovenia*
[3]*Department of Physics, University of Arizona, Tucson, AZ 85721, USA*
[4]*Helmholtz-Institut für Strahlen- und Kernphysik, Rheinische Friedrich-Wilhelms-Universität Bonn, Nußallee 14-16, 53115 Bonn, Germany*
[5]*Center for Theoretical Physics, Massachusetts Institute of Technology, Cambridge, MA 02139, USA*
[6]*Maryland Center for Theoretical Physics, University of Maryland, College Park, USA*


### I. EVALUATING THE FORM-FACTOR RESULTS

In this section, we provide the details needed to reconstruct our final numerical results for the $B \to \pi\pi$ transition amplitude and the $B \to \rho$ form factors. All quantities are given in lattice units; to convert to physical units, the lattice spacing shown in Table III can be used.

The $B \to \pi\pi$ ($\ell = 1$, $I = 1$, $I_z = 1$) $V - A$ transition amplitude is

$$H^{\mu}_{\ell=1}(P,\varepsilon,p_B) = \left( K^{\mu}_{V}(P,\varepsilon,p_B)V(q^2,s) - \sum_{f=A_0,A_1,A_{12}} K^{\mu}_{f}(P,\varepsilon,p_B)f(q^2,s) \right) \frac{T(s)}{k}, \tag{1}$$

where the $K^{\mu}_{f}(P,\varepsilon,p_B)$ are the kinematic factors given in Eqs. (3) and (4) of the main manuscript, $V(q^2,s)$, $A_0(q^2,s)$, $A_1(q^2,s)$, and $A_{12}(q^2,s)$ are the $B \to \pi\pi$ form factors, $T(s)$ is the $\pi\pi$ scattering amplitude, and $k = \sqrt{s/4 - m_\pi^2}$ is the scattering momentum. We use the parametrization denoted `BWI` in Ref. [1] for the $\pi\pi$ scattering amplitude, which is given by

$$T(s) = \frac{16\pi\sqrt{s}}{k} \frac{\sqrt{s}\Gamma(s)}{m_\rho^2 - s - \mathrm{i}\sqrt{s}\Gamma(s)}, \qquad \Gamma(s) = \frac{g^2}{6\pi}\frac{k^3}{s}, \tag{2}$$

where $g$ models the $\rho$-$\pi\pi$ coupling.

We found no significant $s$ dependence of the $B \to \pi\pi$ form factors and parametrized their $q^2$ dependence with first-order $z$-expansions

$$f(q^2,s) = \frac{a_0^{(f)} + a_1^{(f)} z^{(f)}(q^2)}{1 - q^2/\left[m_P^{(f)}\right]^2}, \tag{3}$$

where

$$z^{(f)}(q^2) = \frac{\sqrt{t_+^{(f)} - q^2} - \sqrt{t_+^{(f)} - t_0^{(f)}}}{\sqrt{t_+^{(f)} - q^2} + \sqrt{t_+^{(f)} - t_0^{(f)}}}. \tag{4}$$


* luka.leskovec@ijs.si
† smeinel@arizona.edu

To evaluate $q^2$ and $z^{(f)}$, we use $am_B = 3.0696(15)$, $am_\pi = 0.18295(36)$, $a^2t_0^{(V)} = 6.0$, $a^2t_0^{(A_0,A_1,A_{12})} = 6.5$, and the pole masses and $a^2t_+^{(f)}$ values given in Table I.

| $f$ | $am_P^{(f)}$ | $a^2t_+^{(f)}$ |
|---|---|---|
| $V$ | $am_{B^\star} = 3.0956(15)$ | $(am_B + am_\pi)^2$ |
| $A_0$ | $am_B = 3.0696(15)$ | $(am_{B^\star} + am_\pi)^2$ |
| $A_1$ | $am_{B_1} = 3.3275(16)$ | $(am_{B^\star} + am_\pi)^2$ |
| $A_{12}$ | $am_{B_1} = 3.3275(16)$ | $(am_{B^\star} + am_\pi)^2$ |

TABLE I. $z$-expansion parameters $a^2t_+$ and pole locations $am_P$ for the four form-factors $f = V, A_0, A_1$ and $A_{12}$.

The results for the infinite-volume transition amplitudes are given in Tab. II, where the first column lists the parameter names, the second column lists parameter values and statistical uncertainties, and the remaining columns list the correlations between the parameters.

| Parameter | Value | Correlation matrix | | | | | | | | | |
|---|---|---|---|---|---|---|---|---|---|---|---|
| $am_\rho$ | 0.4616(19) | 1.00 | 0.35 | −0.16 | −0.47 | 0.10 | −0.78 | 0.00 | −0.81 | −0.05 | −0.77 |
| $g$ | 5.76(16) | 0.35 | 1.00 | −0.72 | −0.14 | −0.70 | −0.22 | −0.91 | −0.20 | −0.89 | −0.05 |
| $a_0^{(V)}$ | 0.0608(22) | −0.16 | −0.72 | 1.00 | 0.54 | 0.54 | 0.18 | 0.72 | 0.17 | 0.71 | 0.07 |
| $a_1^{(V)}$ | −0.262(47) | −0.47 | −0.14 | 0.54 | 1.00 | −0.06 | 0.47 | −0.01 | 0.49 | 0.02 | 0.48 |
| $a_0^{(A_0)}$ | 0.0652(19) | 0.10 | −0.70 | 0.54 | −0.06 | 1.00 | −0.14 | 0.78 | −0.17 | 0.80 | −0.28 |
| $a_1^{(A_0)}$ | −0.092(75) | −0.78 | −0.22 | 0.18 | 0.47 | −0.14 | 1.00 | −0.06 | 0.99 | 0.02 | 0.72 |
| $a_0^{(A_1)}$ | 0.02010(58) | 0.00 | −0.91 | 0.72 | −0.01 | 0.78 | −0.06 | 1.00 | −0.09 | 0.94 | −0.23 |
| $a_1^{(A_1)}$ | −0.0139(91) | −0.81 | −0.20 | 0.17 | 0.49 | −0.17 | 0.99 | −0.09 | 1.00 | −0.02 | 0.79 |
| $a_0^{(A_{12})}$ | 0.01709(47) | −0.05 | −0.89 | 0.71 | 0.02 | 0.80 | 0.02 | 0.94 | −0.02 | 1.00 | −0.25 |
| $a_1^{(A_{12})}$ | −0.040(15) | −0.77 | −0.05 | 0.07 | 0.48 | −0.28 | 0.72 | −0.23 | 0.79 | −0.25 | 1.00 |

TABLE II. The parameters for the `BWI` $\pi\pi$ scattering amplitude, form factors $V(q^2,s)$, $A_0(q^2,s)$, $A_1(q^2,s)$ and $A_{12}(q^2,s)$, where first order $z$-expansion was used for each. On the right, all correlations between all parameters are calculated from the parameters obtained in the full jackknife analysis. The central values and the covariance matrix of these parameters are also provided in the machine-readable file `params.dat`.

The scattering amplitude $T(s)$ can be related to the scattering phase shift through

$$T(s) = \frac{16\pi\sqrt{s}}{k}\frac{1}{\cot\delta - \mathrm{i}}, \tag{5}$$

which is shown in Fig. 1.

The pole of the scattering amplitude $T$, which corresponds to the $\rho$ resonance is located at $ak_\rho = 0.1394(14) - \mathrm{i}0.00920(30)$ and has a root of residual equal to $ac_\rho = 1.290(39) - \mathrm{i}0.198(17)$.

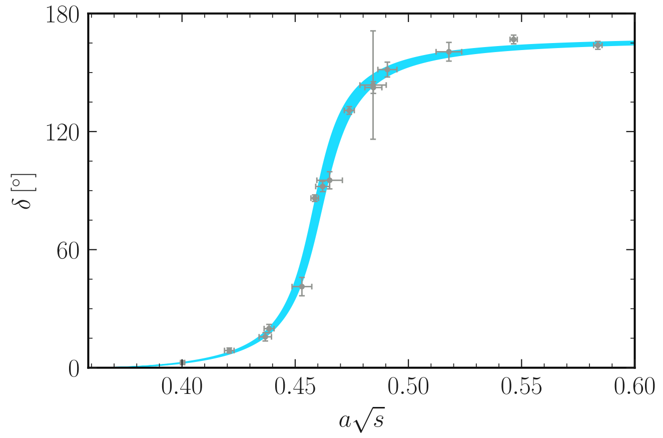


FIG. 1. The dependence of the scattering phase shift $\delta$ as a function of $\sqrt{s}$. The grey points mark the phase shift values at the discrete lattice energies, combined with statistical uncertainties in the $x$ and $y$ axes. The blue-shaded region indicated the fitted scattering phase shift; note that we fit the energies and not the phase shifts as discussed in Ref. [1]

## II. LATTICE ACTIONS AND PARAMETERS

### A. Light-quark and gluon actions

This work is based on a single ensemble of 1039 gauge field configurations with $N_f = 2+1$ dynamical Clover-Wilson fermions [2, 3], generated by Kostas Orginos, Balint Joó, Robert Edwards, and their collaborators. The gauge links in the clover action are smeared with one level of Stout smearing [4] with a staple weight of $\rho = 0.125$. The gluon action is the tadpole-improved tree-level Symanzik action [5–8]. We use the same clover action for the valence light quarks. We determined the lattice spacing $a$ from the $\Upsilon(2S) - \Upsilon(1S)$ splitting [9, 10] computed with improved lattice NRQCD [11]. The main parameters and properties of the ensemble are listed in Table III.

| Parameter | Value |
|---|---|
| $N_s^3 \times N_t$ | $32^3 \times 96$ |
| $\beta$ | 6.1 |
| $am_{u,d}$ | $-0.285$ |
| $am_s$ | $-0.245$ |
| $c_{\rm SW}$ | 1.2493 |
| $N_{\rm conf}$ | 1039 |
| $a$ [fm] | 0.11403(77) |
| $L$ [fm] | 3.649(25) |
| $am_\pi$ | 0.18295(36) |
| $am_K$ | 0.30475(17) |
| $m_\pi$ [MeV] | 316.6(0.6) |

TABLE III. Parameters of the gauge-field ensemble.

### B. Bottom-quark action

We implement the heavy $b$ quark through an anisotropic action of the form

$$S_Q = a^4 \sum_x \bar{Q} \left[ m_Q + \gamma_0 \nabla_0 - \frac{a}{2}\nabla_0^{(2)} + \nu \sum_{i=1}^{3} \left( \gamma_i \nabla_i - \frac{a}{2}\nabla_i^{(2)} \right) - c_E \frac{a}{2} \sum_{i=1}^{3} \sigma_{0i} F_{0i} - c_B \frac{a}{4} \sum_{i,\,j=1}^{3} \sigma_{ij} F_{ij} \right] Q \,. \tag{6}$$

The derivatives and gluon field strength tensor are defined as in Ref. [12], with unsmeared gauge links. Discretization errors proportional to powers of the heavy-quark mass can then be removed to all orders by allowing the coefficients $\nu$, $c_E$, and $c_B$ to depend on $am_Q$ and tuning them [12–18]. The remaining discretization errors are of order $a^2|\vec{p}|^2$, where $|\vec{p}|$ is the typical magnitude of the spatial momentum of the heavy quark inside the hadron. The scheme used by us is to consider $am_Q$ and $\nu$ as independent parameters that are tuned nonperturbatively using the $B_s$ meson dispersion relation, while the coefficients $c_E$ and $c_B$ are functions of $\nu$ given by the tadpole-improved tree-level values [12]

$$c_E = \frac{(1+\nu)}{2u_0^3}, \qquad c_B = \frac{\nu}{u_0^3} \,. \tag{7}$$

Here, we set $u_0$ to the 4th root of the mean plaquette,

$$u_0 = 0.8497942. \tag{8}$$

To tune $am_Q$ and $\nu$, we computed $B_s$ meson two-point functions at zero and nonzero spatial momentum for four different trial choices of $am_Q$ and $\nu$, and extracted the $B_s$ energies from single-exponential fits in the plateau regions. From the $B_s$ energies, we computed the speed of light squared

$$c^2 = \frac{(aE_{B_s}(\vec{p}^2))^2 - (aE_{B_s}(0))^2}{(a\vec{p})^2} \tag{9}$$

with $\vec{p}^2 = 1 \cdot (2\pi/L)^2$. The results are given in Table IV.

| $am_Q$ | $\nu$ | $aE_{B_s}(0)$ | $c^2$ |
|---|---|---|---|
| 6.98705 | 4.17852 | 3.0886(12) | 1.230(16) |
| 8.11769 | 2.96449 | 3.1545(19) | 0.825(18) |
| 6.98705 | 2.96449 | 3.0376(17) | 0.899(16) |
| 8.11769 | 4.17852 | 3.2006(14) | 1.138(17) |

TABLE IV. $B_s$ energy at zero momentum, and speed of light squared (computed using one unit of momentum), for four different choices of anisotropic-clover parameters.

We then performed linear interpolation fits of $aE_{B_s}(0)$ and $c^2$ as functions of $am_Q$ and $\nu$. Fully correlated fits fail, with very large $\chi^2$/d.o.f. due to small eigenvalues in the data correlation matrix combined with a slight nonlinearity in the data. An uncorrelated fit gave $\chi^2$/d.o.f $= 1.4$. Using the results of the uncorrelated fit, we then solved the equations

$$c^2 = 1, \tag{10}$$
$$aE_{B_s}(0) = aM_{\rm exp} \tag{11}$$

for $am_Q$ and $\nu$, using $M_{\rm exp}(B_s) = 5366.79(23)$ MeV. This gave the following solution:

$$am_Q = 7.41366, \tag{12}$$
$$\nu = 3.44759, \tag{13}$$
$$c_E = 3.62371, \tag{14}$$
$$c_B = 5.61790. \tag{15}$$

We used these values for the main computations in this work.

For the non-strange $B$ meson, we computed the energies for the lowest four values of $\vec{p}^2$ and performed a fit of the form

$$aE_B = \sqrt{(am_B)^2 + c^2(a\vec{p})^2}. \tag{16}$$

This fit is shown in Fig. 2 and yields

$$am_B = 3.0696(15), \tag{17}$$
$$c = 1.0105(76). \tag{18}$$

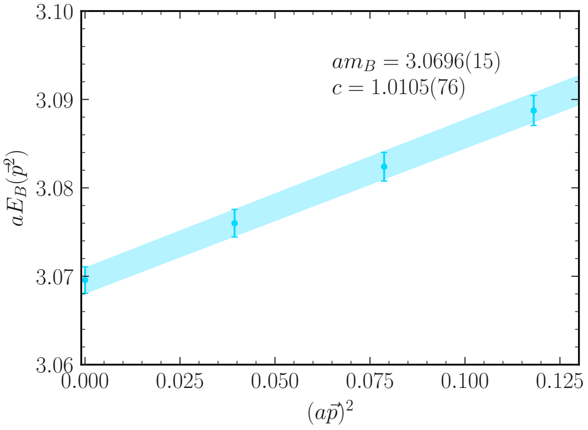


FIG. 2. The $B$-meson dispersion relation.

### C. Renormalization and $O(a)$ improvement of the heavy-light currents

We use the so-called "mostly nonperturbative method" [19, 20], where we write the renormalized $b \to u$ current containing a gamma matrix $\Gamma$ as

$$J_\Gamma(y) = \sqrt{Z_V^{(uu)} Z_V^{(bb)}}\rho_\Gamma \left( \overline{u}(y)\,\Gamma\, b(y) \;+\; d_1^{(b)}\;\overline{u}(y)\,\Gamma \sum_{i=1}^{3} \gamma^i \left(\overrightarrow{\nabla}_i b\right)(y) \right). \tag{19}$$

Above, $Z_V^{(uu)}$ and $Z_V^{(bb)}$ are the renormalization factors for the temporal vector currents $\bar{u}\gamma_0 u$ and $\bar{b}\gamma_0 b$, which are determined fully nonperturbatively using charge conservation. The factor $\sqrt{Z_V^{(uu)} Z_V^{(bb)}}$ accounts for the bulk of the

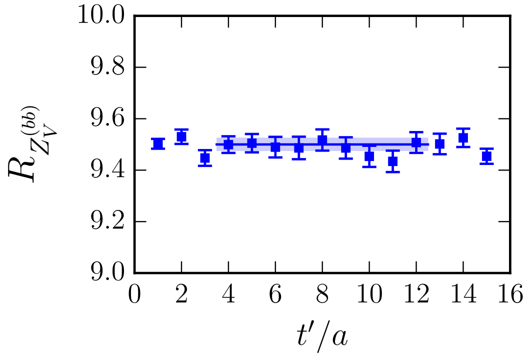


FIG. 3. Numerical results for the ratio defined in Eq. (21).

renormalization of $J_\Gamma(y)$. The remaining correction factors $\rho_\Gamma$ are equal to 1 at tree-level, and can be computed using lattice perturbation theory. Experience shows that the loop corrections to $\rho_\Gamma$ are very small (typically less than 5 percent for $b \to q$), and we set $\rho_\Gamma = 1$ because a one-loop calculation is currently unavailable. We are considering alternative, fully nonperturbative renormalization schemes for future work.

For $Z_V^{(uu)}$, we use the value determined previously by the LHP collaboration using charge conservation [21],

$$Z_V^{(uu)} = 0.7903(2). \tag{20}$$

To determine $Z_V^{(bb)}$, we computed $B_s$ meson two-point and three-point functions with $V_0^{(bb)} = \bar{b}\gamma_0 b$ and formed the ratio

$$R_{Z_V^{(bb)}}(t,t') = \frac{\sum_{\vec{z}} \left\langle O_{B_s}(x_0+t,\vec{z}) \;\; O^\dagger_{B_s}(x_0,\vec{x})\right\rangle}{\sum_{\vec{y},\vec{z}} \left\langle O_{B_s}(x_0+t,\vec{z}) \;\; V_0^{(bb)}(x_0+t',\vec{y}) \;\; O^\dagger_{B_s}(x_0,\vec{x})\right\rangle} \tag{21}$$

A plot of the ratio is shown in the Fig. 3, and the resulting value for $Z_V^{(bb)}$ obtained from a constant fit is

$$Z_V^{(bb)} = 9.500(25). \tag{22}$$

The term with coefficient $d_1^{(b)}$ in Eq. (19) eliminates $\mathcal{O}(a)$ heavy-quark discretization errors at tree level. In that term, the $\gamma^i$ are Euclidean gamma matrices, and $\overrightarrow{\nabla}_i$ is the symmetric derivative

$$\left(\overrightarrow{\nabla}_i b\right)(y) = \frac{1}{2}\left[U_i(y)b(y+\hat{i}) - U_i^\dagger(y-\hat{i})b(y-\hat{i})\right] \tag{23}$$

(without any smearing on the gauge links). The tadpole-improved tree-level value of $d_1^{(b)}$ that we use is

$$d_1^{(b)} = 0.07498. \tag{24}$$

## III. THREE-POINT CORRELATION FUNCTION DATA

### A. Three-point correlation functions

Here, we describe the construction of our optimized three-point correlation functions and the mathematical models we use to extract the matrix elements. The three-point correlation functions definition is

$$C_3^i(t_{\pi\pi}, t_J, t_B) = \langle O_i^{\vec{P},\Lambda,r}(t_{\pi\pi}) J_\Gamma^{\vec{q}}(t_J) O_B^{\vec{p}_B}(t_B) \rangle, \tag{25}$$

where $O_B^{\vec{p}_B}(t_B) = \sum_{\vec{x}} e^{i\vec{p}_B\cdot\vec{x}} \bar{b}(t_B,\vec{x})\gamma_5 q(t_B,\vec{x})$ is the $B$-meson interpolating operator, $J_\Gamma^{\vec{q}}(t_J)$ is the current (19), projected to momentum $\vec{q}$, and $O_i^{\vec{P},\Lambda,r}(t_{\pi\pi})$ is an interpolating operator for the $\pi\pi$ system in row $r$ of irrep $\Lambda$, with the index $i$ labeling different types of operators (quark-antiquark and $\pi\pi$ with different relative momenta [1, 22])[1]. For the total momenta of the initial and final states, we use all configurations with $|\vec{P}| \leq \sqrt{3}\frac{2\pi}{L}$ and $|\vec{p}_B| \leq \sqrt{3}\frac{2\pi}{L}$. The light quarks in all hadron interpolating fields are smeared using gauge-invariant Gaussian (Wuppertal) smearing [23] with spatially APE-smeared gauge links [24], with the parameters $N_{\rm Wup} = 20$, $\alpha_{\rm Wup} = 3.0$, $\alpha_{\rm APE} = 2.5$. The bottom quark in $O_B$ is smeared using $N_{\rm Wup} = 10$, $\alpha_{\rm Wup} = 2$, with gauge links that are spatially Stout-smeared using $N_{\rm Stout} = 10$, $\rho_{\rm Stout} = 0.08$. The Wick contractions are symbolically depicted in Fig. 4 and are evaluated using forward, sequential, and stochastic propagators similarly to Ref. [22], except that here the $b$-quark propagator, shown in black in Fig. 4, is a sequential rather than stochastic propagator to reduce noise.

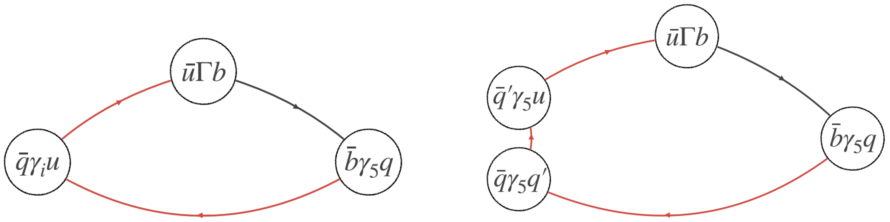


FIG. 4. The Wick contractions relevant to the $B \to \pi\pi\ell\bar{\nu}$ transition. Left is the Wick contraction for the quark-antiquark $\rho$-meson operator, $\bar{q}\gamma_i u$, while the right is the Wick contraction for the two-pion operators.

The three-point functions $C_3^i$ overlap to all states in the source and sink irreps:

$$C_3^i(t_{\pi\pi}, t_J, t_B) = \sum_{n,m} \langle 0| O_i^{\vec{P},\Lambda,r} |n\rangle \langle n| J_\Gamma^{\vec{q}} |m\rangle \langle m| O_B^{\vec{p}_B} |0\rangle \frac{e^{-E_n(t_{\pi\pi}-t_J)} e^{-E_m(t_J-t_B)}}{2E_n 2E_m}, \tag{26}$$

where $E_n$ are the energies in the two-hadron spectrum, while $E_m$ are the energies in the heavy-meson spectrum. We construct three-point functions with a dominant overlap to a single well-defined finite-volume state through a linear combination of $C_3^i$, with coefficients $u_i^n$ taken as the $n$-th state generalized eigenvector of the GEVP analysis [1], $C_3^n = u_i^n C_3^i$. Equivalently at the operator level $O_n^{\vec{P},\Lambda,r} = u_i^n O_i^{\vec{P},\Lambda,r}$. The projection results in an optimized correlation function (or operator) which has a large overlap to a specific finite-volume state, $|n\rangle$, and much smaller

---

[1] In the main manuscript, we write $\Delta t = t_{\pi\pi} - t_B$ and set $t_B = 0$ for simplicity.

overlaps to other states:

$$C_3^n(t_{\pi\pi}, t_J, t_B) = \sum_m \langle 0|O_n^{\vec{P},\Lambda,r}|n\rangle\langle n|J_\Gamma^{\vec{q}}|m\rangle\langle m|O_B^{\vec{p}_B}|0\rangle \frac{e^{-E_n(t_{\pi\pi}-t_J)}e^{-E_m(t_J-t_B)}}{2E_n 2E_m} + \sum_{n',m} \langle 0|O_n^{\vec{P},\Lambda,r}|n'\rangle\langle n'|J_\Gamma^{\vec{q}}|m\rangle\langle m|O_B^{\vec{p}_B}|0\rangle \frac{e^{-E_{n'}(t_{\pi\pi}-t_J)}e^{-E_m(t_J-t_B)}}{2E_{n'} 2E_m}, \quad (27)$$

where in the index $m$ we are only interested in the ground state, which corresponds to the $B$-meson. Note, that $\langle 0|O_n^{\vec{P},\Lambda,r}|n\rangle = \sqrt{2E_n}e^{E_n t_0/2}$ due to the GEVP normalizations, where $t_0/a = 3$ is the reference time we use for the GEVP. Here $n$ is the state we are projecting to with $u_i^n$, and $n'$ labels the excited states not removed by the GEVP.

By projecting to all 15 finite-volume states in 8 different irreducible representations and 4 different total momenta listed in Tab. III of Ref. [22], we are able to determine matrix elements in the high-$q^2$ and low-$\sqrt{s}$ region as depicted in Fig. 5.

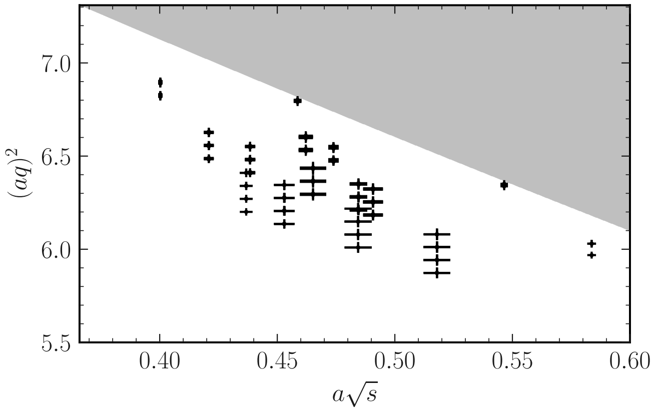


FIG. 5. The values of $\sqrt{s}$ and $q^2$ used in our analysis. The dark-shaded region is kinematically forbidden.

### B. Fitting the three-point correlation functions

To extract the finite-volume transition matrix elements from the optimized three-point functions, we construct the quantity

$$d_n(t_J, t_{\pi\pi}, t_B) = C_3^n(t_{\pi\pi}, t_J, t_B) \frac{2E_n 2E_B}{\langle 0|O_n^{\vec{P},\Lambda,r}|n\rangle\langle B|O_B^{\vec{p}_B}|0\rangle} e^{E_n(t_{\pi\pi}-t_J)}e^{E_B(t_J-t_B)}, \quad (28)$$

which, up to excited-state contamination, is equal to $\langle n|J_\Gamma|B\rangle$. Here, $E_B$ and $\langle B|O_B^{\vec{p}_B}|0\rangle$ are obtained from single-exponential fits to the $B$-meson two-point function, while $E_n$ and $\langle 0|O_n^{\vec{P},\Lambda,r}|n\rangle = \sqrt{2E_n}e^{E_n t_0/2}$ are obtained from

the GEVP. Showing the excited-state contamination explicitly, we have

$$d_n(t_J, t_{\pi\pi}, t_B) = \langle n|J_\Gamma^{\vec{q}}|B\rangle + \sum_{n',m'} \langle n'|J_\Gamma^{\vec{q}}|m'\rangle \left(\frac{\langle 0|O_n^{\vec{P},\Lambda,r}|n'\rangle\langle m'|O_B^{\vec{p}_B}|0\rangle}{\langle 0|O_n^{\vec{P},\Lambda,r}|n\rangle\langle B|O_B^{\vec{p}_B}|0\rangle}\right)\left(\frac{2E_n 2E_B}{2E_{n'}2E_{m'}}\right) e^{-(E_{n'}-E_n)(t_{\pi\pi}-t_J)} e^{-(E_{m'}-E_B)(t_J-t_B)}. \tag{29}$$

We consider the following two models to fit the data for $d_n$:

i) "$C_3$ − single-state" model assumes no excited state contamination in either the initial $B$-meson or the final two-hadron state:

$$d_n(t, t_{\pi\pi}, t_B) = \langle n|J_\Gamma^{\vec{q}}|B\rangle, \tag{30}$$

ii) "$C_3$ − two-state" model includes, in addition to the desired matrix element $\langle n|J_\Gamma^{\vec{q}}|B\rangle$, also the matrix element between the $B$ and an excited $n'$, $\langle n'|J_\Gamma^{\vec{q}}|B\rangle$, and the matrix element between an excited $m'$ and the state $n$, $\langle n|J_\Gamma^{\vec{q}}|m'\rangle$:

$$d_n(t, t_{\pi\pi}, t_B) = \langle n|J_\Gamma^{\vec{q}}|B\rangle + \alpha_{n'} e^{-\Delta E_{n'}(t_{\pi\pi}-t_J)} + \alpha_{m'} e^{-\Delta E_{m'}(t_J-t_B)}, \tag{31}$$

The matrix elements from the $C_3$ fits are shown in Sections V and VI as the blue shaded region, while the data is shown with blue circles.

### C. Fitting ratios of correlation functions

We construct a ratio from the optimized three-point correlation functions, $C_3^n$, the principal correlator, $\lambda_n^{\vec{P},\Lambda}$, and the $B$-meson two-point function, $C_2^{\vec{p}_B}$ as:

$$R_n(t_{\pi\pi}, t_J, t_B) = \frac{C_3^n(t_{\pi\pi}, t_J, t_B) C_3^{n\,\dagger}(t_{\pi\pi}, t_B + t_{\pi\pi} - t_J, t_B)}{\lambda_n^{\vec{P},\Lambda}(t_{\pi\pi} - t_B, t_0) C_2^{\vec{p}_B}(t_{\pi\pi} - t_B)}, \tag{32}$$

which can be used to define $r_n((t_{\pi\pi}, t_J, t_B)$ as:

$$r_n^2(t_{\pi\pi}, t_J, t_B) = 2E_n\, 2E_B\, R_n(t_{\pi\pi}, t_J, t_B). \tag{33}$$

Because all matrix elements are real-valued, this quantity is equal to

$$\begin{aligned} r_n^2(t_{\pi\pi}, t_J, t_B) &= \langle n|J_\Gamma^{\vec{q}}|B\rangle^2 + \\ &+ \langle n|J_\Gamma^{\vec{q}}|B\rangle\langle n'|J_\Gamma^{\vec{q}}|B\rangle \frac{\langle 0|O_n^{\vec{P},\Lambda,r}|n'\rangle}{\langle 0|O_n^{\vec{P},\Lambda,r}|n\rangle} \frac{E_n}{E_{n'}} \left(e^{-(E_{n'}-E_n)(t_J-t_B)} + e^{-(E_{n'}-E_n)(t_{\pi\pi}-t_J)}\right) \\ &+ \langle n|J_\Gamma^{\vec{q}}|B\rangle\langle n|J_\Gamma^{\vec{q}}|m'\rangle \frac{\langle m'|O_B^{\vec{p}_B}|0\rangle}{\langle B|O_B^{\vec{p}_B}|0\rangle} \frac{E_B}{E_{m'}} \left(e^{-(E_{m'}-E_B)(t_J-t_B)} + e^{-(E_{m'}-E_B)(t_{\pi\pi}-t_J)}\right) \\ &+ \ldots \end{aligned} \tag{34}$$

where the first line is the square of the desired matrix element, and the second and third lines show the leading terms originating from the excited-state contamination in the three-point functions. Excited-state contamination from the two-point functions is suppressed by propagation through the full source-sink separation.

Our ratio data are insufficient to resolve the difference in the energy gaps $(E_{m'} - E_B)$ and $(E_{n'} - E_n)$. We consider two possible models to fit to the data for $r_n$:

i) "$R-$single-state" model assumes no excited state contamination:

$$r_n(t_{\pi\pi}, t_J, t_B) = \langle n|J_\Gamma^{\vec{q}}|B\rangle. \tag{35}$$

ii) "$R-$two-state" model, contains in addition to the desired matrix element also a term aimed at approximating the second and third lines of Eq. (34):

$$r_n(t_{\pi\pi}, t_J, t_B) = \langle n|J_\Gamma^{\vec{q}}|B\rangle + \beta\left(e^{-\Delta E(t_J - t_B)} + e^{-\Delta E(t_{\pi\pi} - t_J)}\right). \tag{36}$$

The matrix elements from the $R$ fits are shown in Sections V and VI as the red-shaded region, while the data is shown with red diamonds.

### D. Model-averaging of the matrix-element fits

To obtain the final values of the matrix elements $\langle n|J_\Gamma^{\vec{q}}|B\rangle$, we use the following procedure. For each set of the data, ratios and three-point functions, we perform model averages using the "perfect-model" Akaike Information Criterion (AIC) [25] over the results from different fit ranges and fit models. Prior to the averaging, any fit ranges that include boundary points are excluded to avoid large discretization errors and fits with $\chi^2$ values above 1.51 are removed. From this refined set of fits, up to 40 fits with the lowest $\chi^2/\text{dof}$ for $C_3$ and $R$ separately are selected.

For the further analysis of the form factors, we primarily choose the model-averaged matrix elements extracted from the three-point functions ($C_3$). For certain kinematic points, we believe the ratio fits to be more reliable, and use them instead. The specific choices are listed in the ancillary files me_V.dat and me_A.dat with `include = c3`, or `include = rat`. To account for the systematic uncertainty resulting from this choice, we add [26]

$$\Delta\sigma = \max\left(|\langle n|J_\Gamma^{\vec{q}}|B\rangle_R - \langle n|J_\Gamma^{\vec{q}}|B\rangle_{C_3}|, \sqrt{|\sigma_R^2 - \sigma_{C_3}^2|}\right) \tag{37}$$

in quadrature to the diagonal elements of the covariance matrix that enters the global form-factor analysis; here $\sigma$ denotes the uncertainty of the model-averaged matrix element as determined from the three-point or ratio fits.

### E. Ancillary files

The data obtained from the fits for both types of models are listed in the ancillary files `me_V.dat` (contains matrix elements without kinematic prefactors) and `me_A.dat` (contains matrix elements with kinematic prefactors), where we give the model type, source-sink separations used in the fit, the fit-ranges for each of the source-sink separations, the resulting $\frac{\chi^2}{\text{dof}}$ and the matrix element value with the uncertainty. At the end of each entry, the model-averaged "AIC" quantity [25] is listed, which enters our transition amplitude fits at the jackknife level. An example is listed below.

```
==========================================================================================
include = c3
\vec{P} = \frac{2\pi}{L} (1,1,1) \Lambda = E r = 2 n = 1 \vec{p}_B = \frac{2\pi}{L} (0,1,1)
\mu = 2
------------------------------------------------------------------------------------------
C_3-two-state    (8,10,12)    2-6,2-7,4-10     0.90     0.1932(85)
...
C_3-two-state    (8,10,12)    2-6,3-7,2-8      0.75     0.1936(88)
AIC:                                                    0.1931(88)
------------------------------------------------------------------------------------------
R-two-state      (10,12)      2-5,2-6          0.59     0.193(18)
...
R-single-state   (10,12)      1-5,0-6          1.44     0.1953(39)
AIC:                                                    0.1930(29)
```

## IV. PLOTS OF THE FITS FOR THE VECTOR-CURRENT REDUCED MATRIX ELEMENTS

Due to the simplicity of the Lorentz decomposition of the vector-current insertion, we factor out the kinematical prefactors from the vector-current matrix elements and present $V(q^2, s)$ as determined on the lattice in the Figures below.

Each figure corresponds to one choice of momenta, current indices, polarizations, and excitation. The three panels in each figure show the three different source-sink separations, $\Delta t/a = 8, 10, 12$. The blue circles correspond to the matrix elements determined from the three-point functions, $d_n$, and the red diamonds correspond to the ratios, $r_n$. The light-shaded bands going through the data points correspond to the fit models with the highest AIC weights. The horizontal red-shaded bands with the dashed line indicate the value of the AIC average from the three-point function analysis, while the horizontal blue-shaded bands with a full line indicate the AIC average from the ratio analysis.

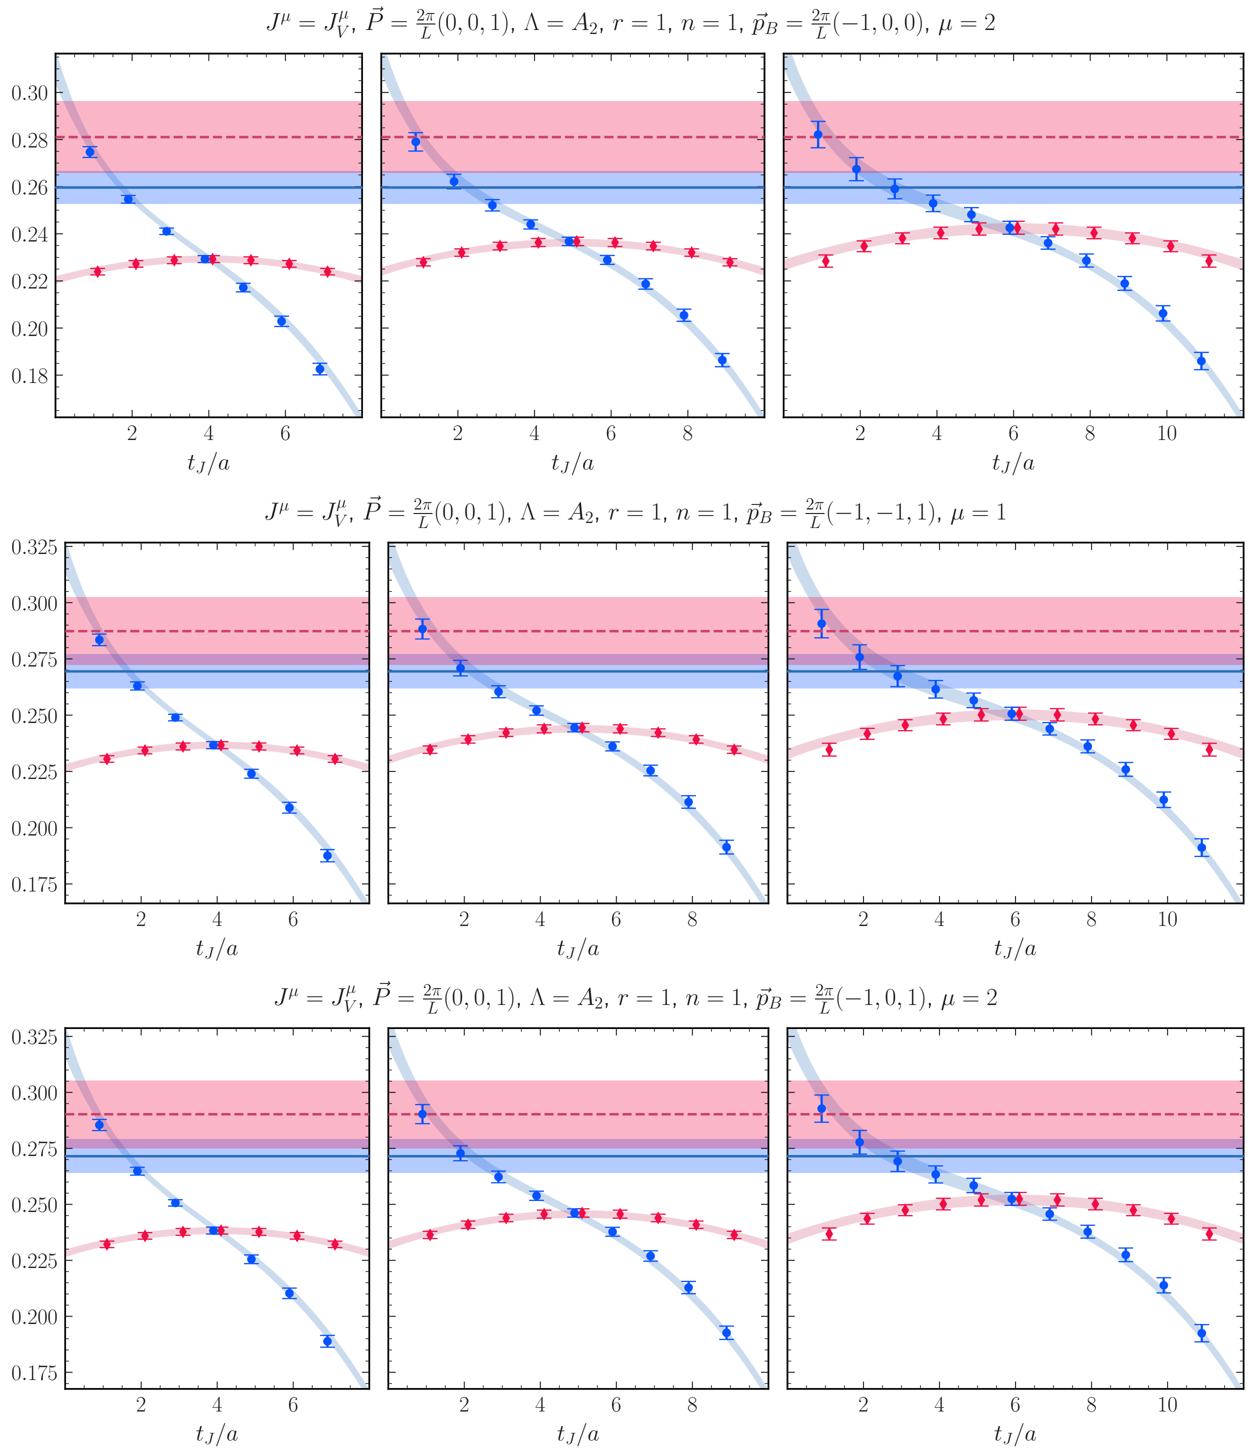

$J^\mu = J_V^\mu$, $\vec{P} = \frac{2\pi}{L}(0,0,1)$, $\Lambda = A_2$, $r = 1$, $n = 1$, $\vec{p}_B = \frac{2\pi}{L}(-1,0,0)$, $\mu = 2$
0.30
0.28
0.26
0.24
0.22
0.20
0.18
2
4
6
8
10
$t_J/a$
$J^\mu = J_V^\mu$, $\vec{P} = \frac{2\pi}{L}(0,0,1)$, $\Lambda = A_2$, $r = 1$, $n = 1$, $\vec{p}_B = \frac{2\pi}{L}(-1,-1,1)$, $\mu = 1$
0.325
0.300
0.275
0.250
0.225
0.200
0.175
$t_J/a$
$J^\mu = J_V^\mu$, $\vec{P} = \frac{2\pi}{L}(0,0,1)$, $\Lambda = A_2$, $r = 1$, $n = 1$, $\vec{p}_B = \frac{2\pi}{L}(-1,0,1)$, $\mu = 2$
$t_J/a$

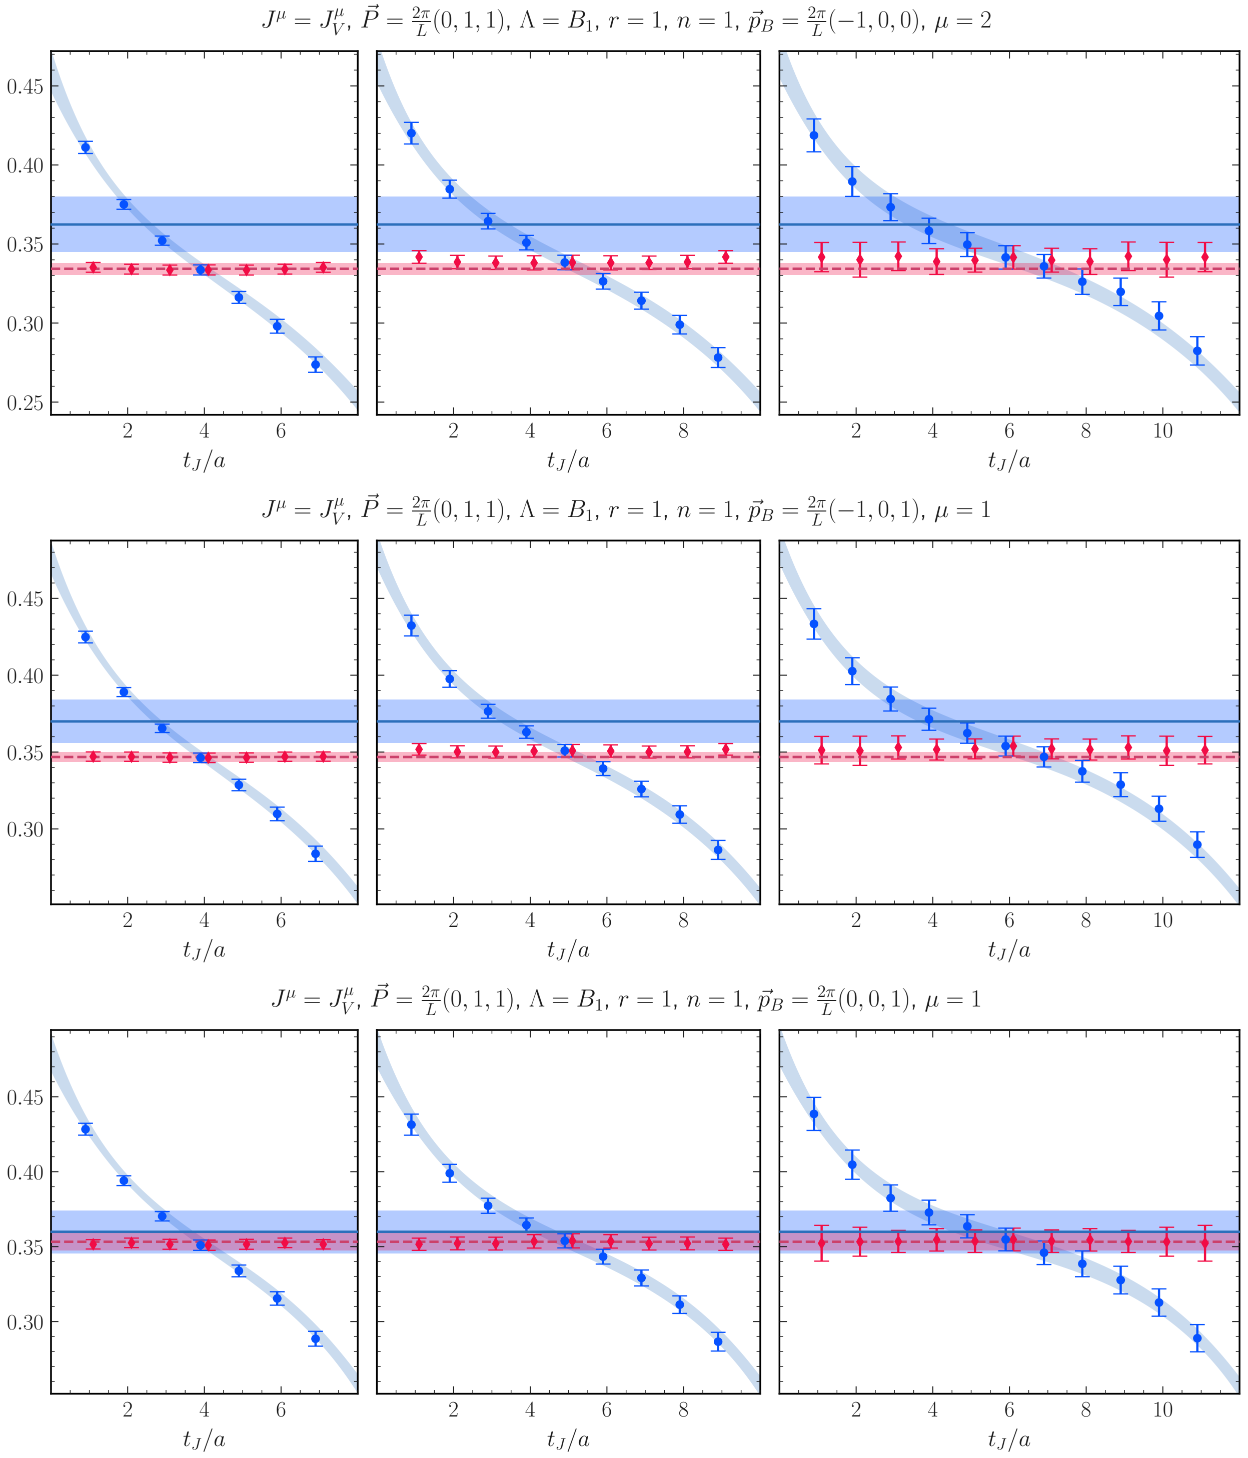

$J^\mu = J_V^\mu$, $\vec{P} = \frac{2\pi}{L}(0,1,1)$, $\Lambda = B_1$, $r = 1$, $n = 1$, $\vec{p}_B = \frac{2\pi}{L}(-1,0,0)$, $\mu = 2$
$J^\mu = J_V^\mu$, $\vec{P} = \frac{2\pi}{L}(0,1,1)$, $\Lambda = B_1$, $r = 1$, $n = 1$, $\vec{p}_B = \frac{2\pi}{L}(-1,0,1)$, $\mu = 1$
$J^\mu = J_V^\mu$, $\vec{P} = \frac{2\pi}{L}(0,1,1)$, $\Lambda = B_1$, $r = 1$, $n = 1$, $\vec{p}_B = \frac{2\pi}{L}(0,0,1)$, $\mu = 1$
0.25
0.30
0.35
0.40
0.45
2
4
6
8
10
$t_J/a$

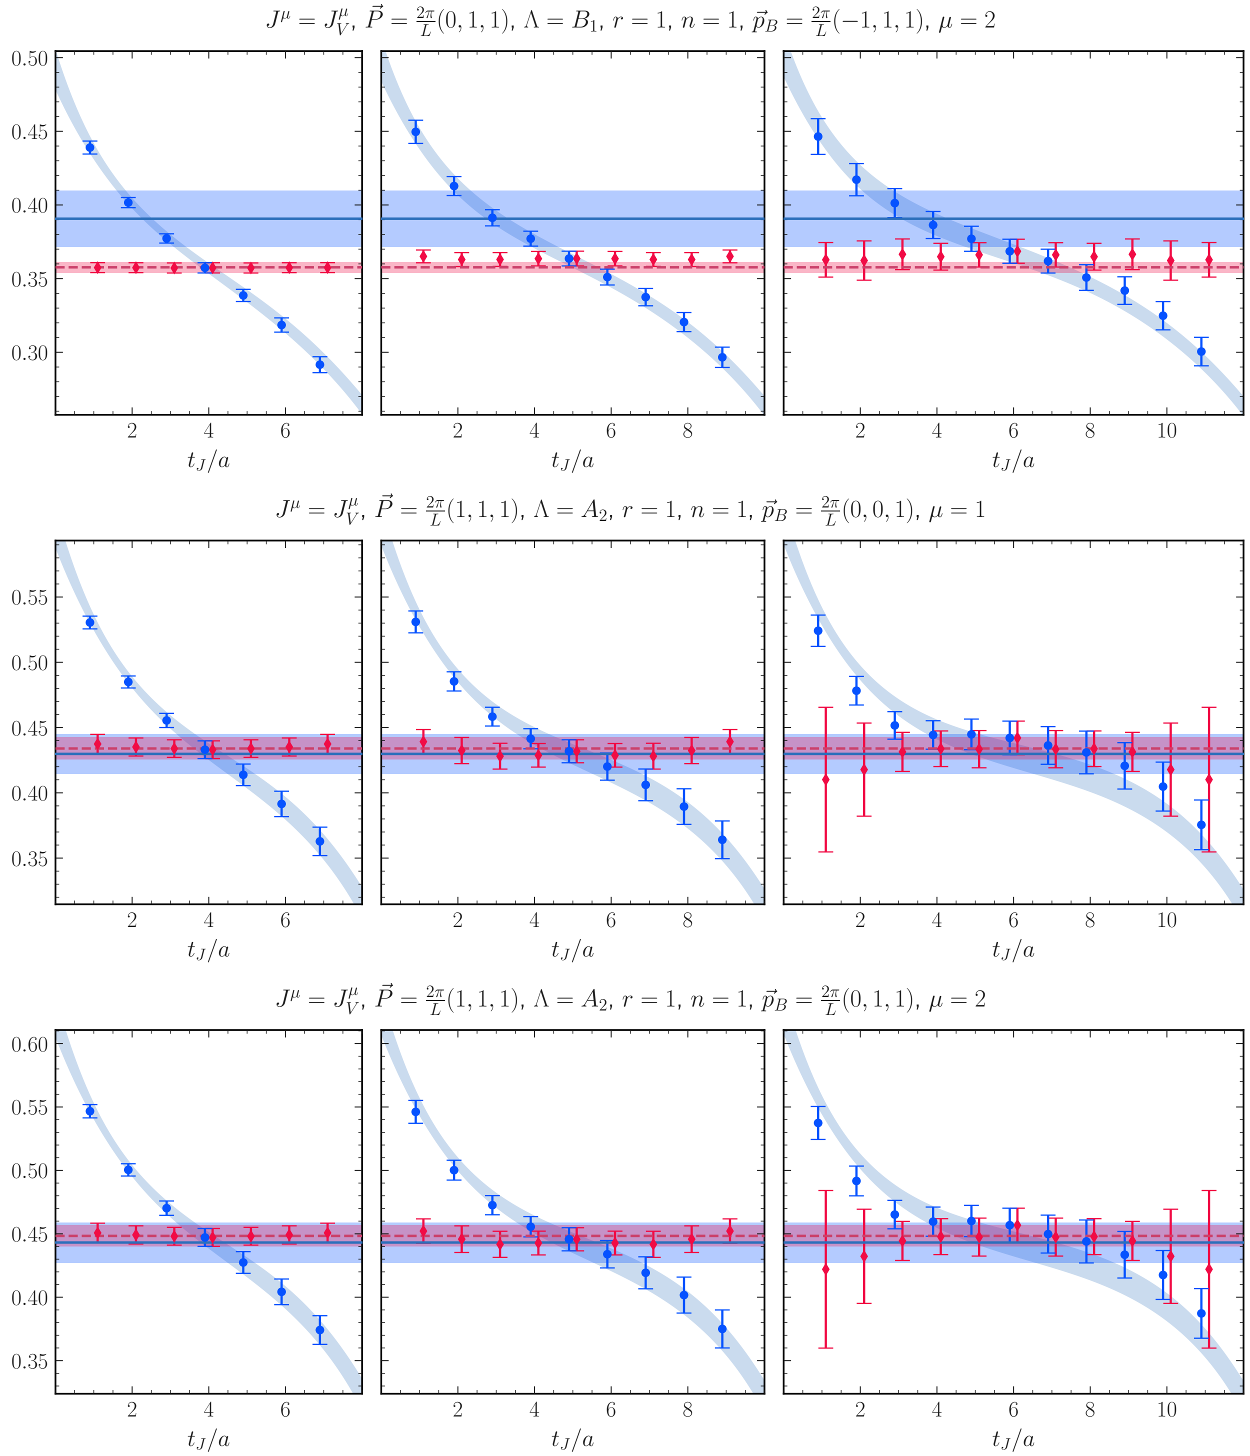

$J^\mu = J_V^\mu$, $\vec{P} = \frac{2\pi}{L}(0,1,1)$, $\Lambda = B_1$, $r = 1$, $n = 1$, $\vec{p}_B = \frac{2\pi}{L}(-1,1,1)$, $\mu = 2$
$J^\mu = J_V^\mu$, $\vec{P} = \frac{2\pi}{L}(1,1,1)$, $\Lambda = A_2$, $r = 1$, $n = 1$, $\vec{p}_B = \frac{2\pi}{L}(0,0,1)$, $\mu = 1$
$J^\mu = J_V^\mu$, $\vec{P} = \frac{2\pi}{L}(1,1,1)$, $\Lambda = A_2$, $r = 1$, $n = 1$, $\vec{p}_B = \frac{2\pi}{L}(0,1,1)$, $\mu = 2$
$t_J/a$

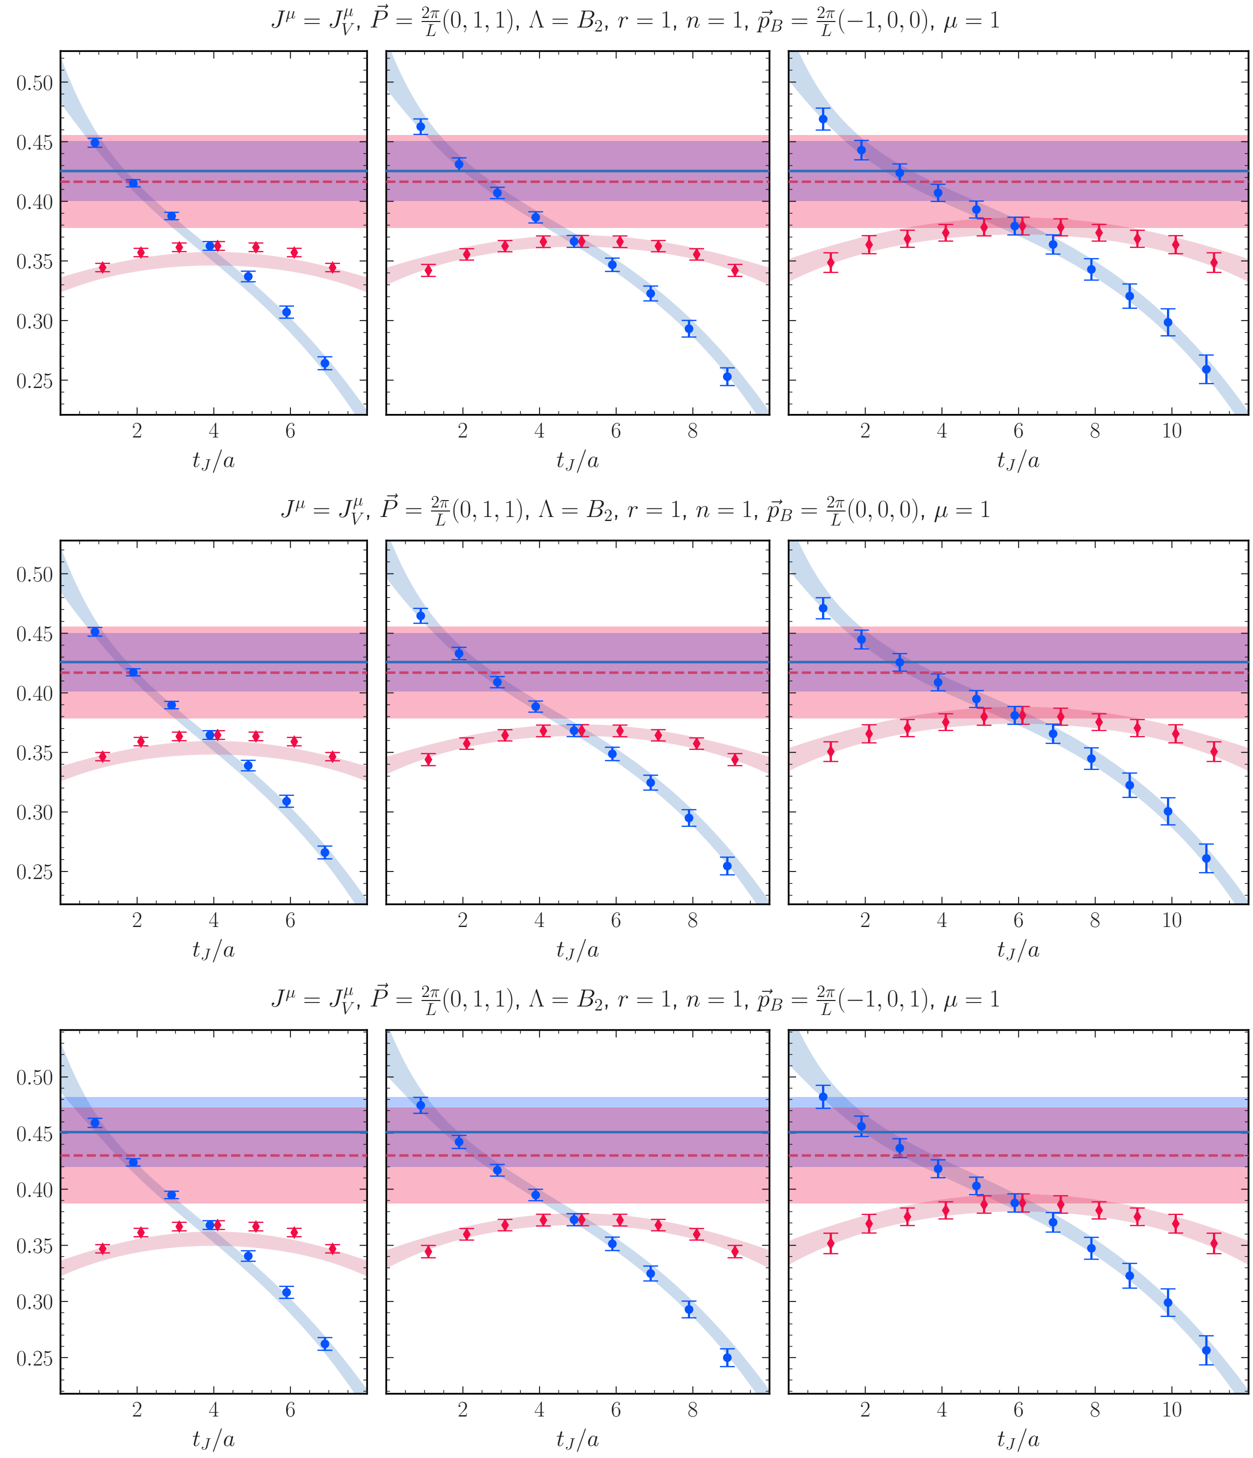

$J^\mu = J^\mu_V$, $\vec{P} = \frac{2\pi}{L}(0,1,1)$, $\Lambda = B_2$, $r = 1$, $n = 1$, $\vec{p}_B = \frac{2\pi}{L}(-1,0,0)$, $\mu = 1$
$J^\mu = J^\mu_V$, $\vec{P} = \frac{2\pi}{L}(0,1,1)$, $\Lambda = B_2$, $r = 1$, $n = 1$, $\vec{p}_B = \frac{2\pi}{L}(0,0,0)$, $\mu = 1$
$J^\mu = J^\mu_V$, $\vec{P} = \frac{2\pi}{L}(0,1,1)$, $\Lambda = B_2$, $r = 1$, $n = 1$, $\vec{p}_B = \frac{2\pi}{L}(-1,0,1)$, $\mu = 1$
$t_J/a$
0.25
0.30
0.35
0.40
0.45
0.50
2
4
6
8
10

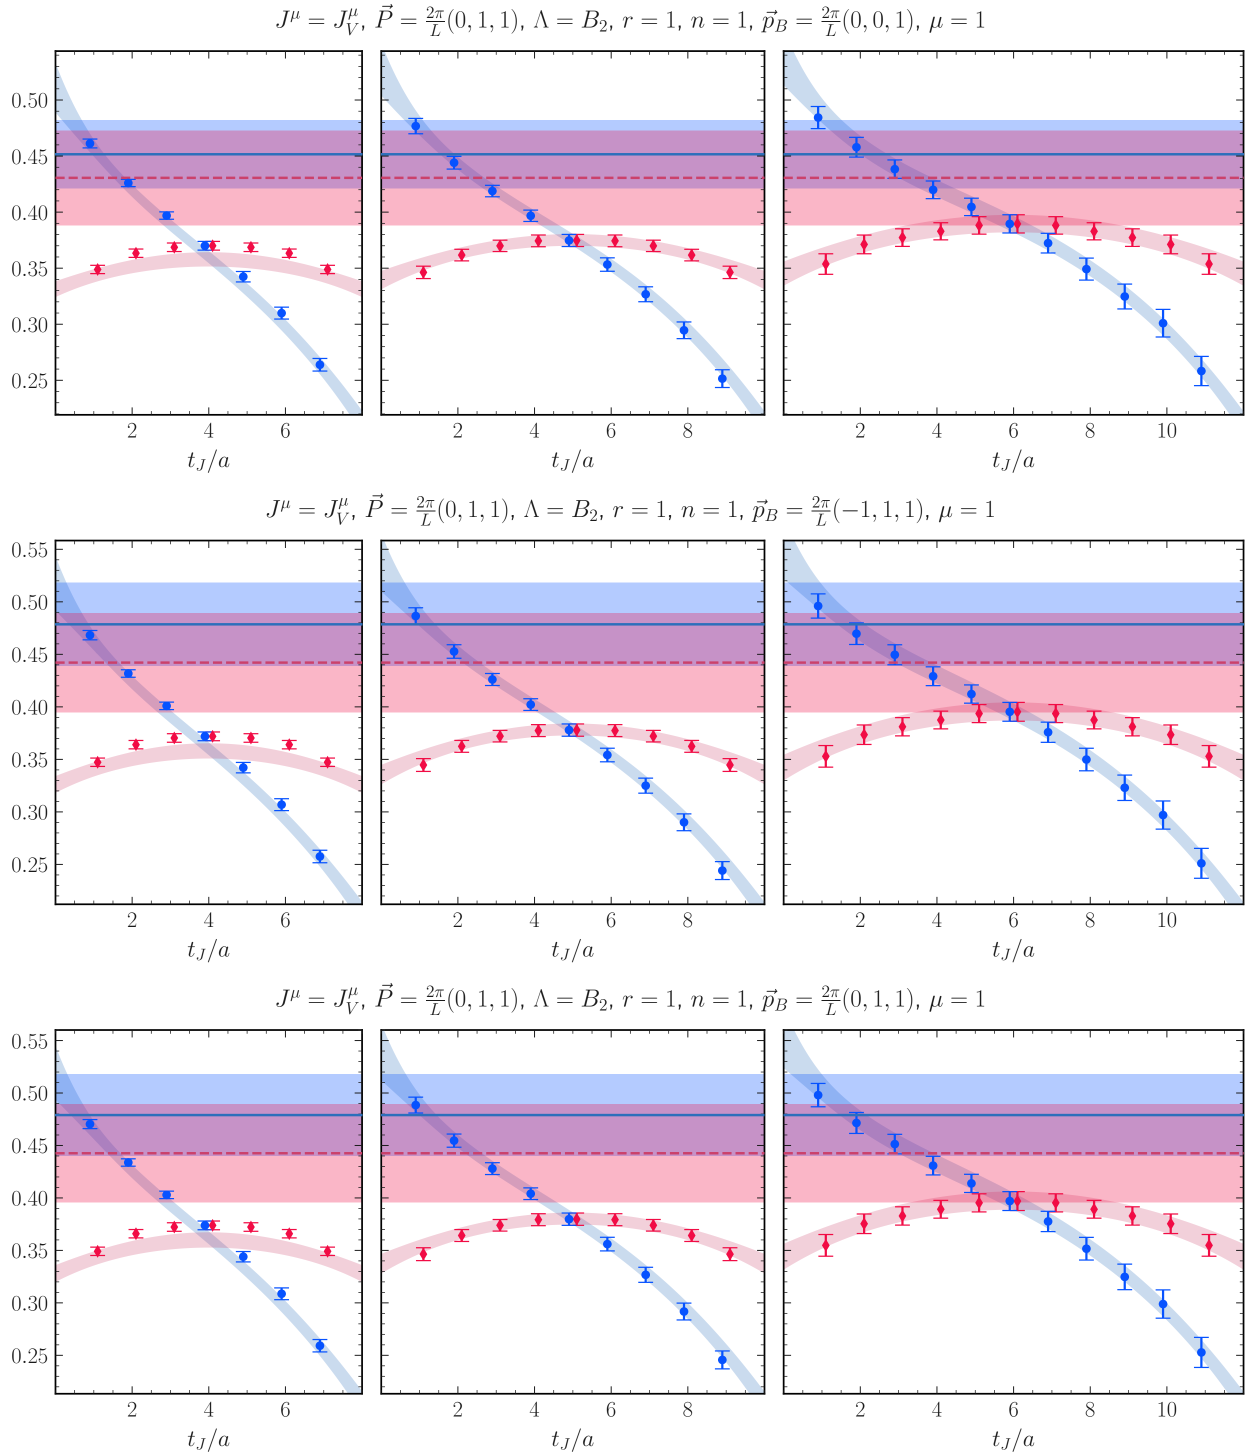
$J^\mu = J_V^\mu$, $\vec{P} = \frac{2\pi}{L}(0,1,1)$, $\Lambda = B_2$, $r=1$, $n=1$, $\vec{p}_B = \frac{2\pi}{L}(0,0,1)$, $\mu = 1$
$J^\mu = J_V^\mu$, $\vec{P} = \frac{2\pi}{L}(0,1,1)$, $\Lambda = B_2$, $r=1$, $n=1$, $\vec{p}_B = \frac{2\pi}{L}(-1,1,1)$, $\mu = 1$
$J^\mu = J_V^\mu$, $\vec{P} = \frac{2\pi}{L}(0,1,1)$, $\Lambda = B_2$, $r=1$, $n=1$, $\vec{p}_B = \frac{2\pi}{L}(0,1,1)$, $\mu = 1$
$t_J/a$

$J^\mu = J_V^\mu$, $\vec{P} = \frac{2\pi}{L}(1,1,1)$, $\Lambda = E$, $r = 1$, $n = 1$, $\vec{p}_B = \frac{2\pi}{L}(0,0,0)$, $\mu = 1$

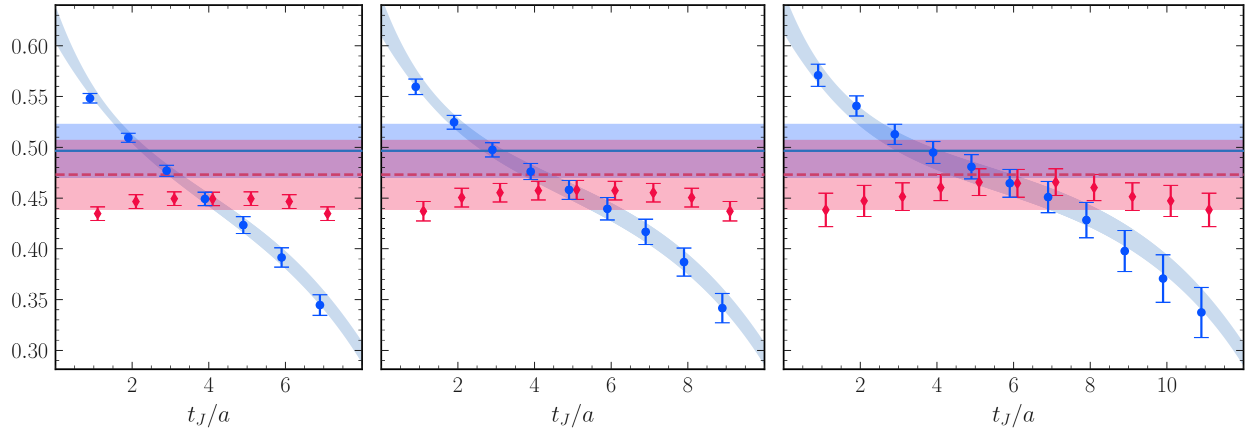


$J^\mu = J_V^\mu$, $\vec{P} = \frac{2\pi}{L}(1,1,1)$, $\Lambda = E$, $r = 1$, $n = 1$, $\vec{p}_B = \frac{2\pi}{L}(0,0,1)$, $\mu = 1$

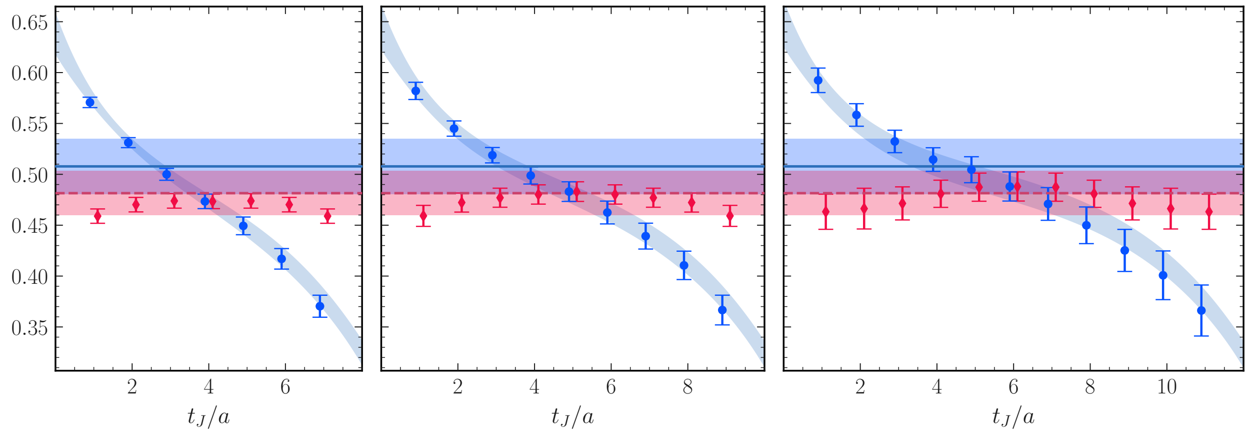


$J^\mu = J_V^\mu$, $\vec{P} = \frac{2\pi}{L}(1,1,1)$, $\Lambda = E$, $r = 1$, $n = 1$, $\vec{p}_B = \frac{2\pi}{L}(0,1,1)$, $\mu = 1$

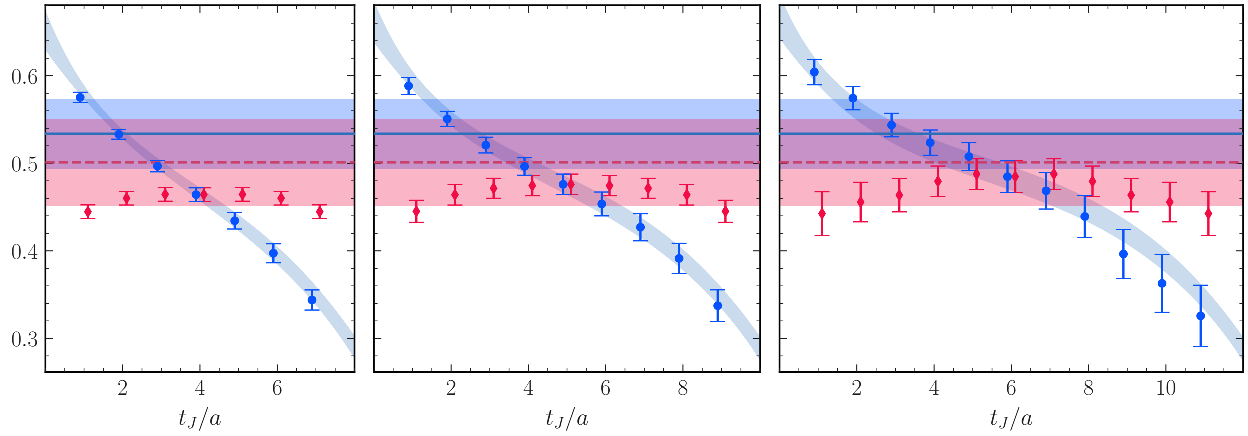

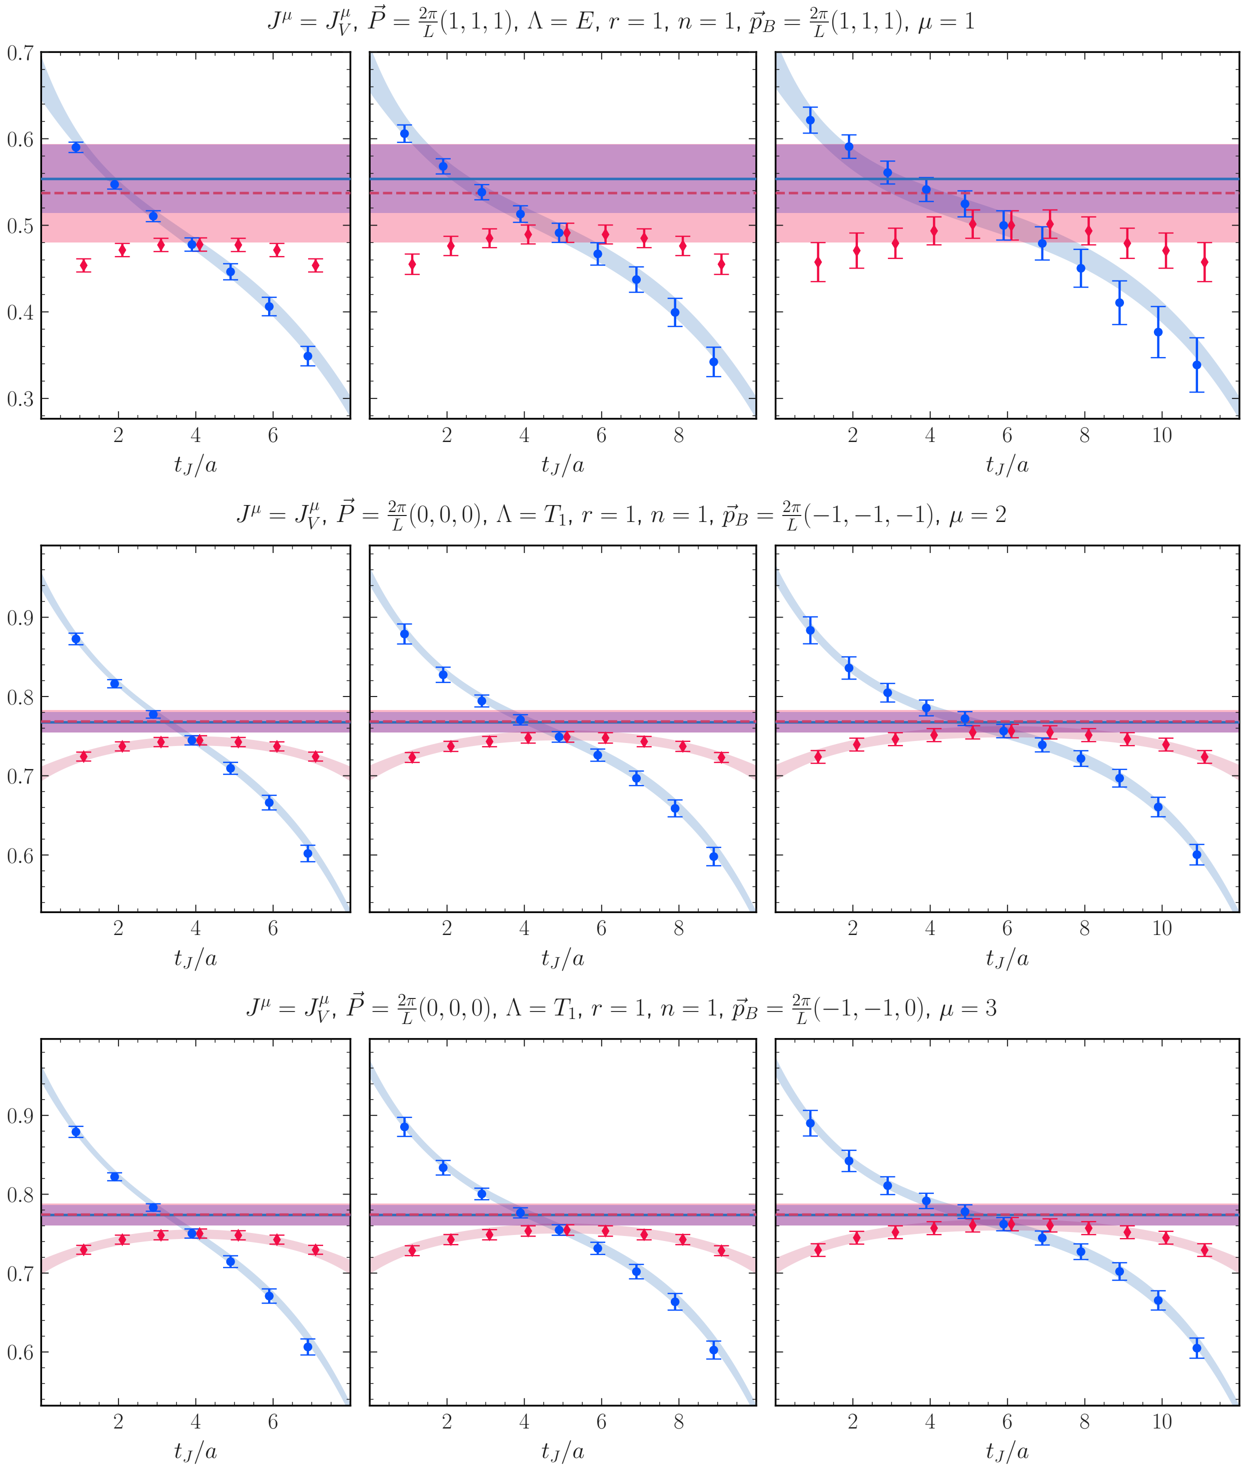

$J^\mu = J_V^\mu$, $\vec{P} = \frac{2\pi}{L}(1,1,1)$, $\Lambda = E$, $r = 1$, $n = 1$, $\vec{p}_B = \frac{2\pi}{L}(1,1,1)$, $\mu = 1$
$J^\mu = J_V^\mu$, $\vec{P} = \frac{2\pi}{L}(0,0,0)$, $\Lambda = T_1$, $r = 1$, $n = 1$, $\vec{p}_B = \frac{2\pi}{L}(-1,-1,-1)$, $\mu = 2$
$J^\mu = J_V^\mu$, $\vec{P} = \frac{2\pi}{L}(0,0,0)$, $\Lambda = T_1$, $r = 1$, $n = 1$, $\vec{p}_B = \frac{2\pi}{L}(-1,-1,0)$, $\mu = 3$
$t_J/a$

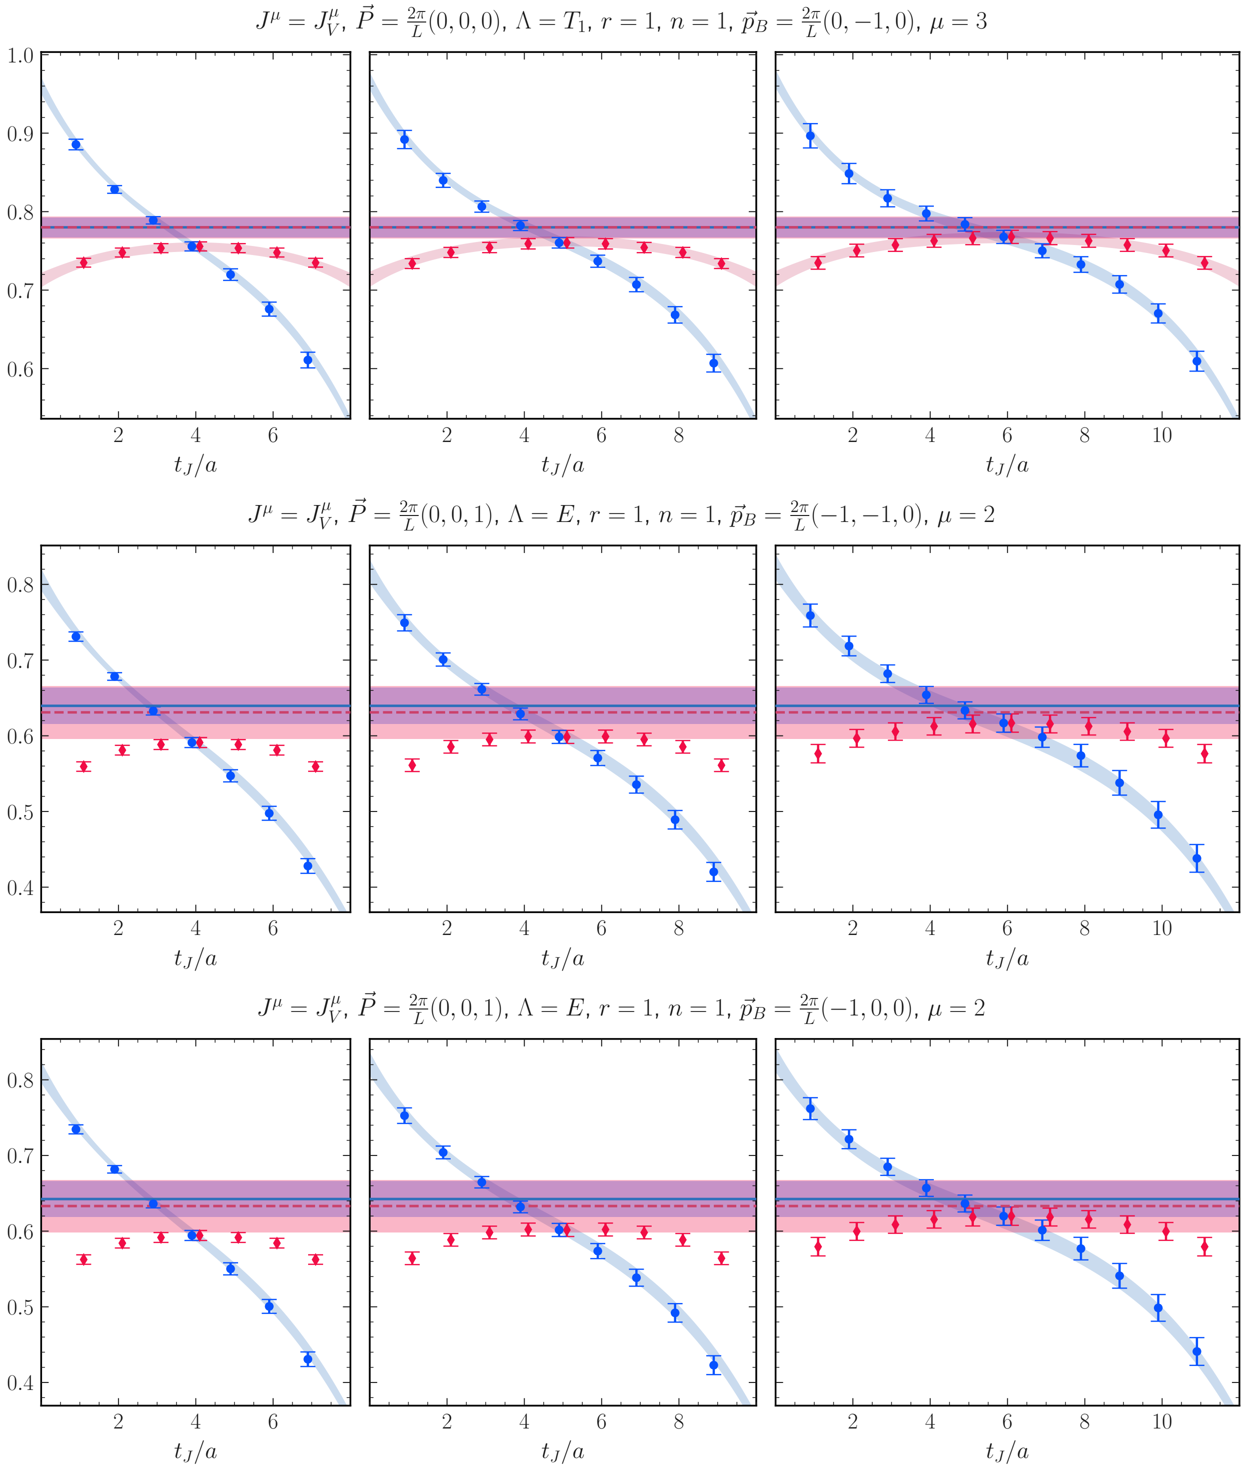

$J^\mu = J_V^\mu$, $\vec{P} = \frac{2\pi}{L}(0,0,0)$, $\Lambda = T_1$, $r = 1$, $n = 1$, $\vec{p}_B = \frac{2\pi}{L}(0,-1,0)$, $\mu = 3$
$J^\mu = J_V^\mu$, $\vec{P} = \frac{2\pi}{L}(0,0,1)$, $\Lambda = E$, $r = 1$, $n = 1$, $\vec{p}_B = \frac{2\pi}{L}(-1,-1,0)$, $\mu = 2$
$J^\mu = J_V^\mu$, $\vec{P} = \frac{2\pi}{L}(0,0,1)$, $\Lambda = E$, $r = 1$, $n = 1$, $\vec{p}_B = \frac{2\pi}{L}(-1,0,0)$, $\mu = 2$
$t_J/a$

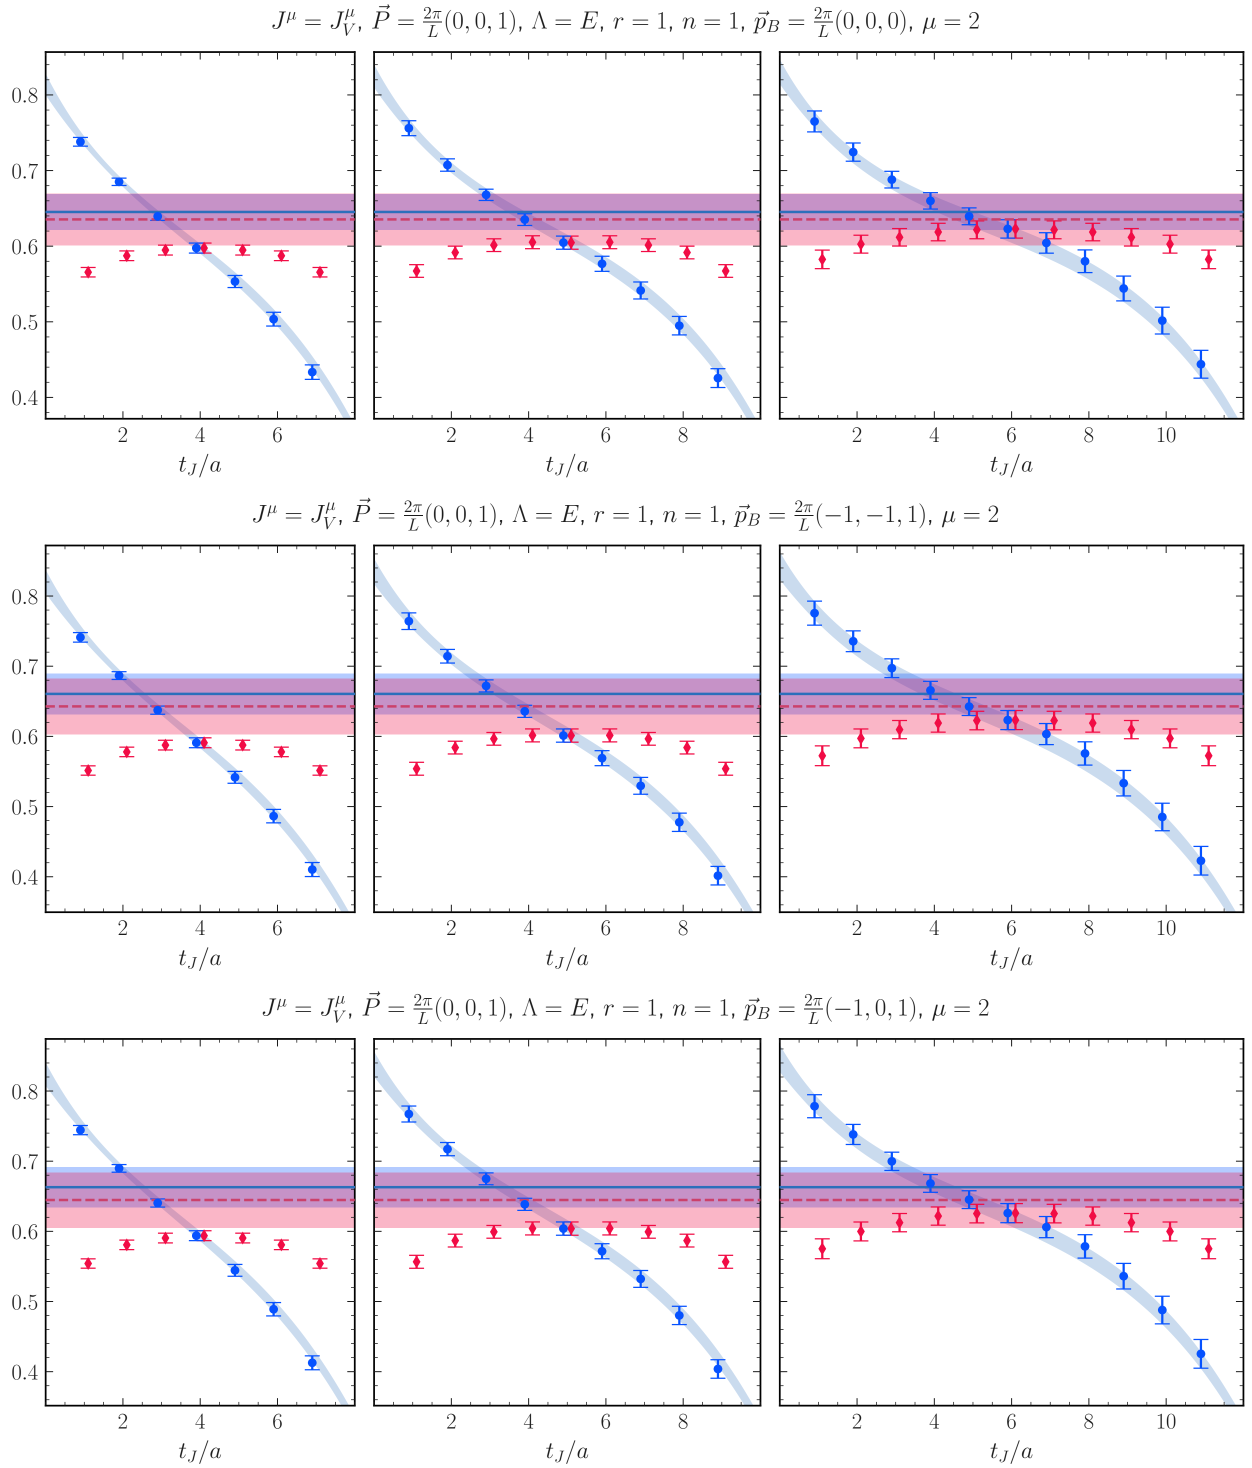
$J^\mu = J_V^\mu$, $\vec{P} = \frac{2\pi}{L}(0,0,1)$, $\Lambda = E$, $r = 1$, $n = 1$, $\vec{p}_B = \frac{2\pi}{L}(0,0,0)$, $\mu = 2$
$t_J/a$
$J^\mu = J_V^\mu$, $\vec{P} = \frac{2\pi}{L}(0,0,1)$, $\Lambda = E$, $r = 1$, $n = 1$, $\vec{p}_B = \frac{2\pi}{L}(-1,-1,1)$, $\mu = 2$
$t_J/a$
$J^\mu = J_V^\mu$, $\vec{P} = \frac{2\pi}{L}(0,0,1)$, $\Lambda = E$, $r = 1$, $n = 1$, $\vec{p}_B = \frac{2\pi}{L}(-1,0,1)$, $\mu = 2$
$t_J/a$

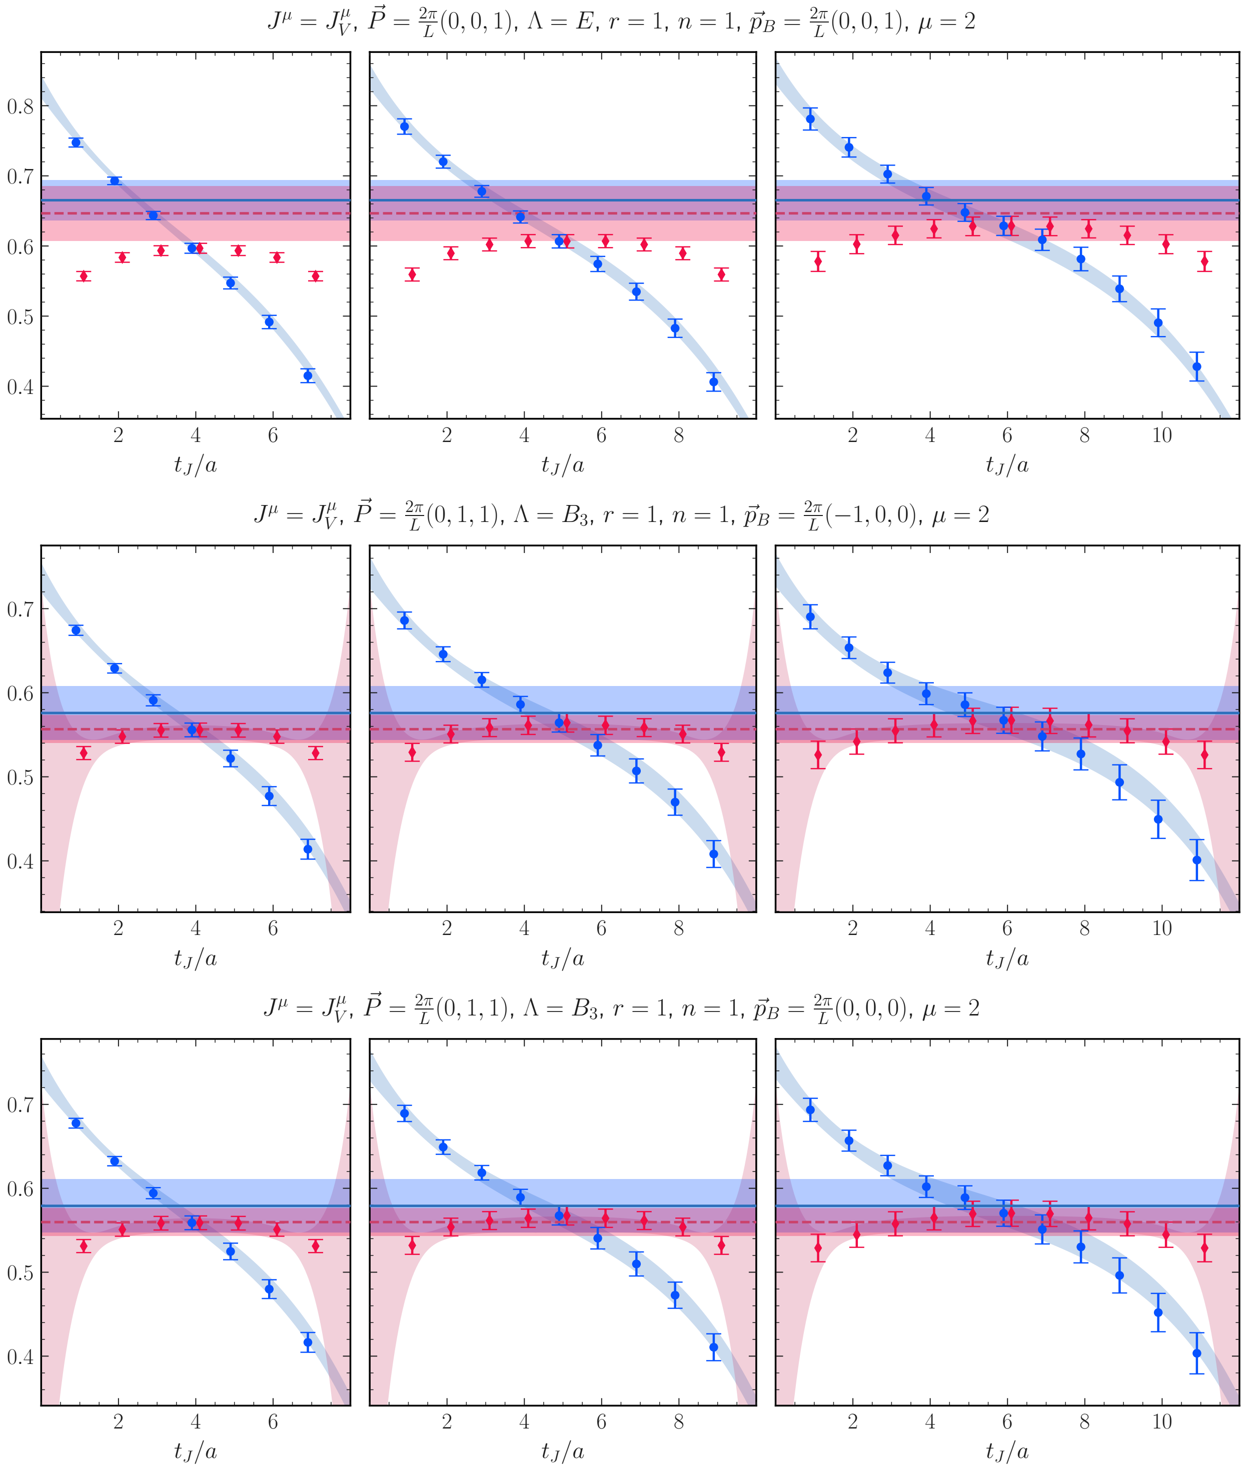
$J^\mu = J_V^\mu$, $\vec{P} = \frac{2\pi}{L}(0,0,1)$, $\Lambda = E$, $r = 1$, $n = 1$, $\vec{p}_B = \frac{2\pi}{L}(0,0,1)$, $\mu = 2$
$J^\mu = J_V^\mu$, $\vec{P} = \frac{2\pi}{L}(0,1,1)$, $\Lambda = B_3$, $r = 1$, $n = 1$, $\vec{p}_B = \frac{2\pi}{L}(-1,0,0)$, $\mu = 2$
$J^\mu = J_V^\mu$, $\vec{P} = \frac{2\pi}{L}(0,1,1)$, $\Lambda = B_3$, $r = 1$, $n = 1$, $\vec{p}_B = \frac{2\pi}{L}(0,0,0)$, $\mu = 2$
$t_J/a$

$J^{\mu} = J_V^{\mu}$, $\vec{P} = \frac{2\pi}{L}(0, 1, 1)$, $\Lambda = B_3$, $r = 1$, $n = 1$, $\vec{p}_B = \frac{2\pi}{L}(-1, 0, 1)$, $\mu = 2$

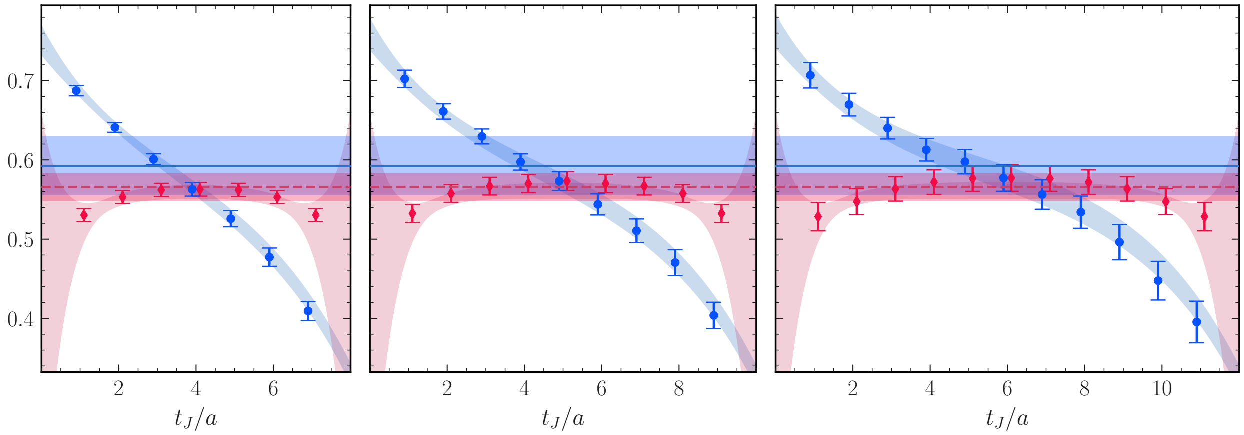


$J^{\mu} = J_V^{\mu}$, $\vec{P} = \frac{2\pi}{L}(0, 1, 1)$, $\Lambda = B_3$, $r = 1$, $n = 1$, $\vec{p}_B = \frac{2\pi}{L}(0, 0, 1)$, $\mu = 2$

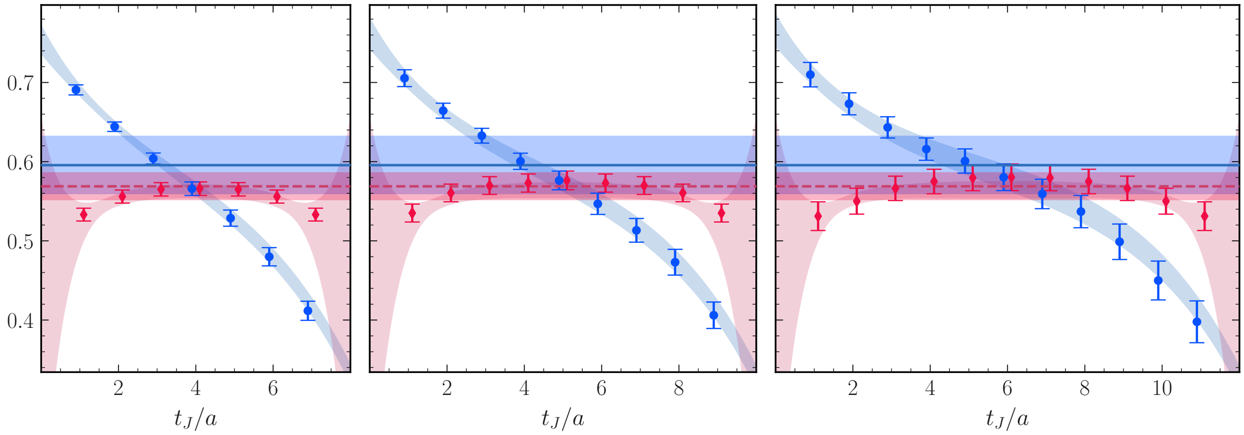


$J^{\mu} = J_V^{\mu}$, $\vec{P} = \frac{2\pi}{L}(0, 1, 1)$, $\Lambda = B_3$, $r = 1$, $n = 1$, $\vec{p}_B = \frac{2\pi}{L}(-1, 1, 1)$, $\mu = 2$

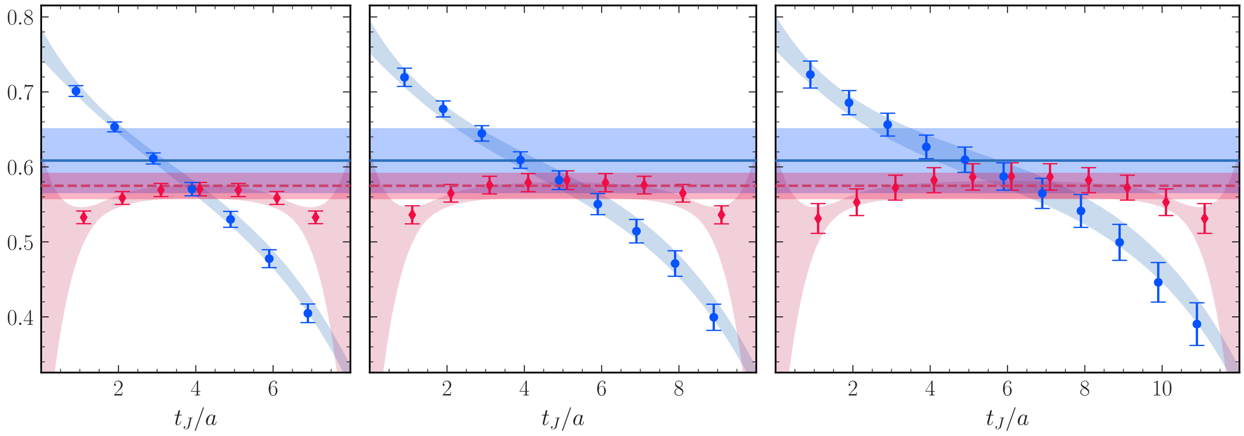

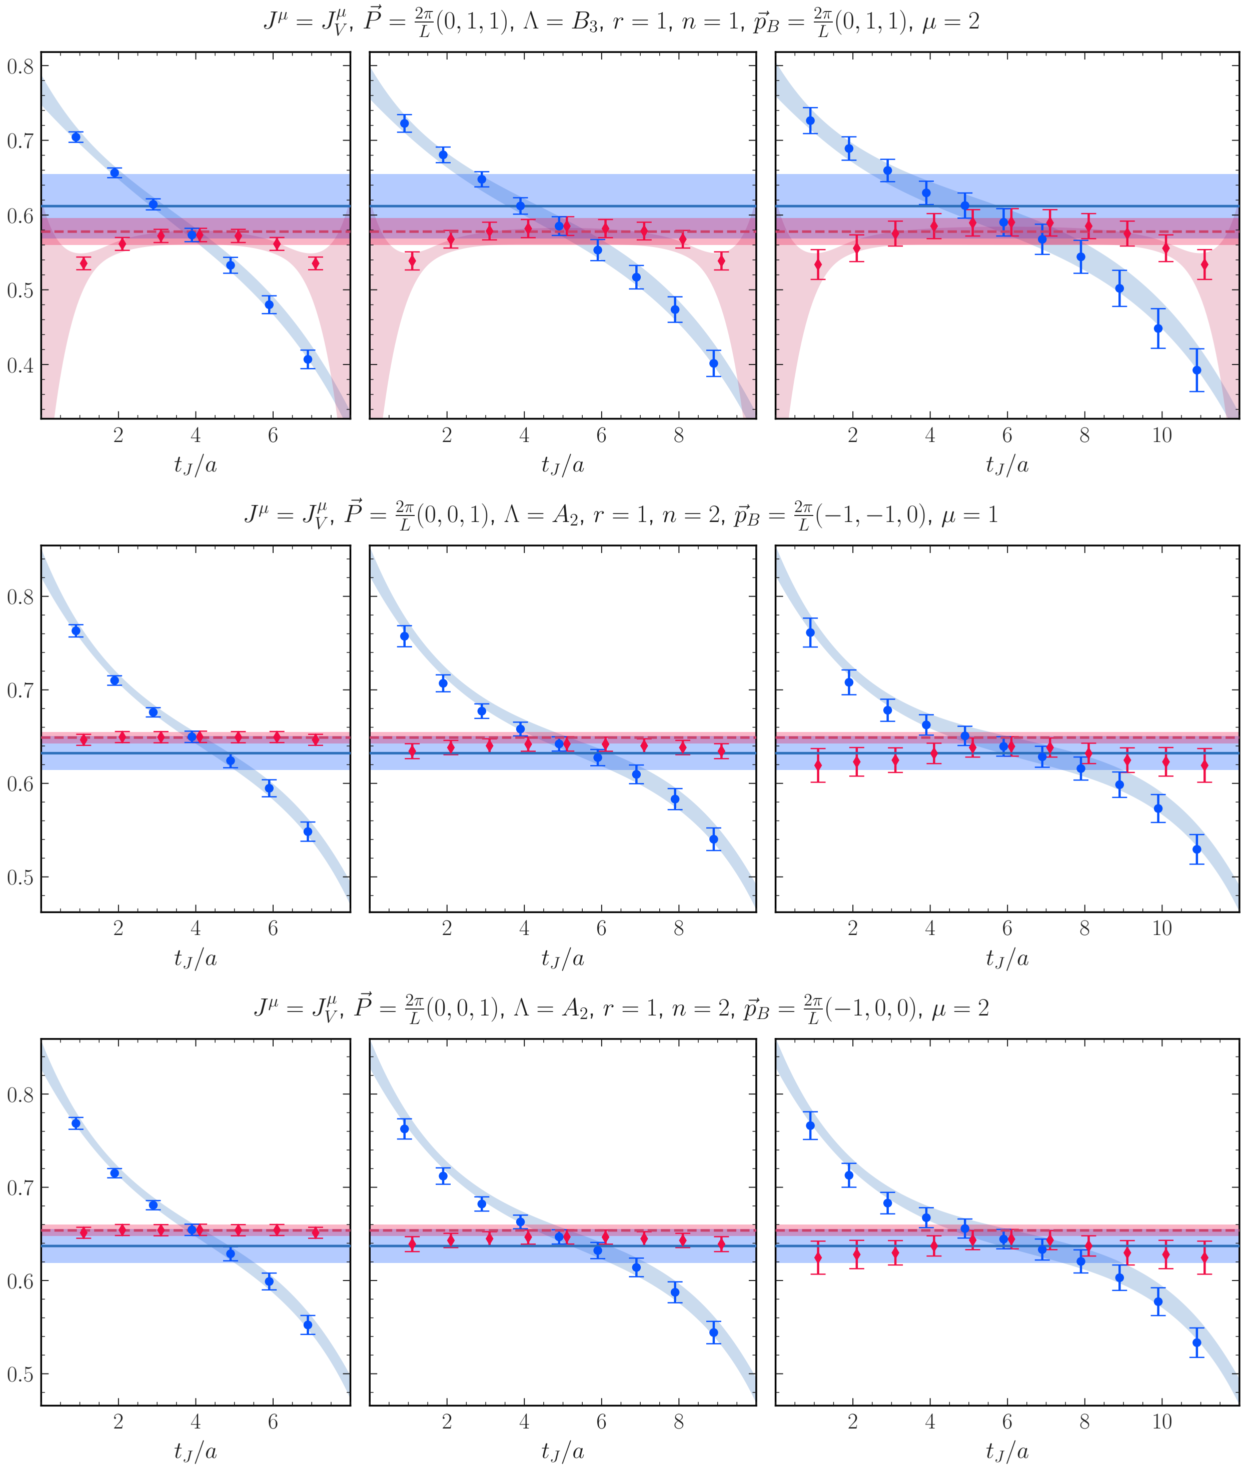

$J^\mu = J_V^\mu$, $\vec{P} = \frac{2\pi}{L}(0,1,1)$, $\Lambda = B_3$, $r = 1$, $n = 1$, $\vec{p}_B = \frac{2\pi}{L}(0,1,1)$, $\mu = 2$
$t_J/a$
$J^\mu = J_V^\mu$, $\vec{P} = \frac{2\pi}{L}(0,0,1)$, $\Lambda = A_2$, $r = 1$, $n = 2$, $\vec{p}_B = \frac{2\pi}{L}(-1,-1,0)$, $\mu = 1$
$t_J/a$
$J^\mu = J_V^\mu$, $\vec{P} = \frac{2\pi}{L}(0,0,1)$, $\Lambda = A_2$, $r = 1$, $n = 2$, $\vec{p}_B = \frac{2\pi}{L}(-1,0,0)$, $\mu = 2$
$t_J/a$

$J^\mu = J_V^\mu,\ \vec{P} = \frac{2\pi}{L}(0,0,1),\ \Lambda = A_2,\ r = 1,\ n = 2,\ \vec{p}_B = \frac{2\pi}{L}(-1,-1,1),\ \mu = 1$

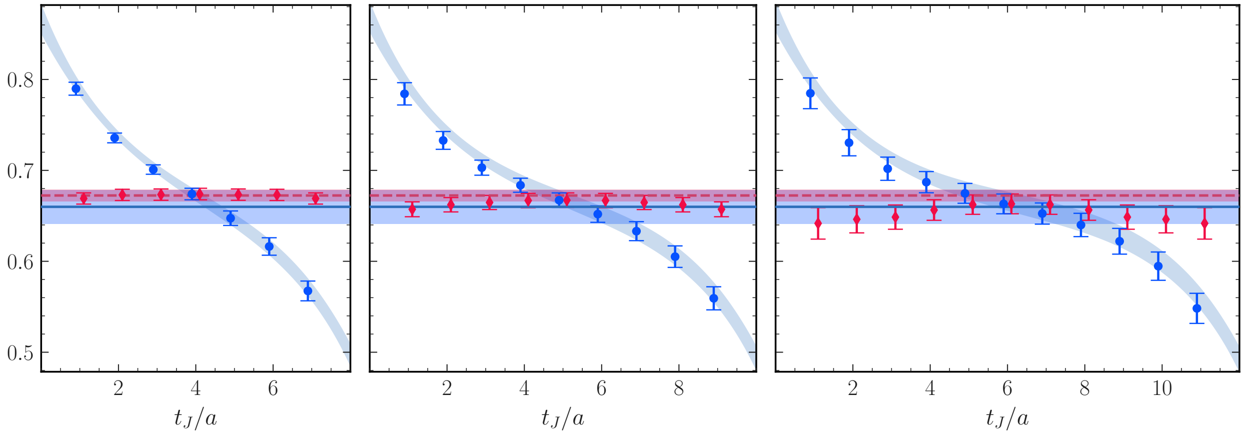


$J^\mu = J_V^\mu,\ \vec{P} = \frac{2\pi}{L}(0,0,1),\ \Lambda = A_2,\ r = 1,\ n = 2,\ \vec{p}_B = \frac{2\pi}{L}(-1,0,1),\ \mu = 2$

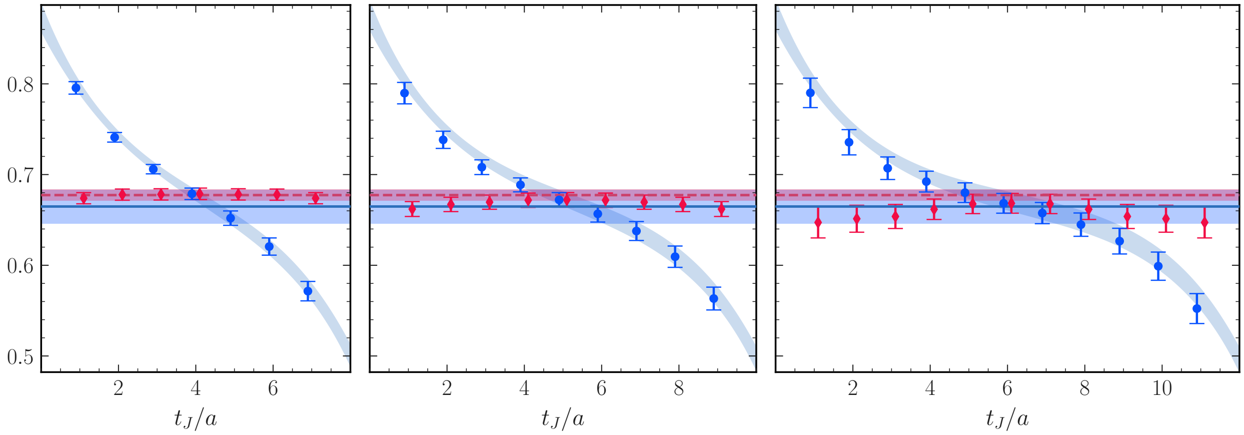


$J^\mu = J_V^\mu,\ \vec{P} = \frac{2\pi}{L}(1,1,1),\ \Lambda = A_2,\ r = 1,\ n = 2,\ \vec{p}_B = \frac{2\pi}{L}(0,0,1),\ \mu = 1$

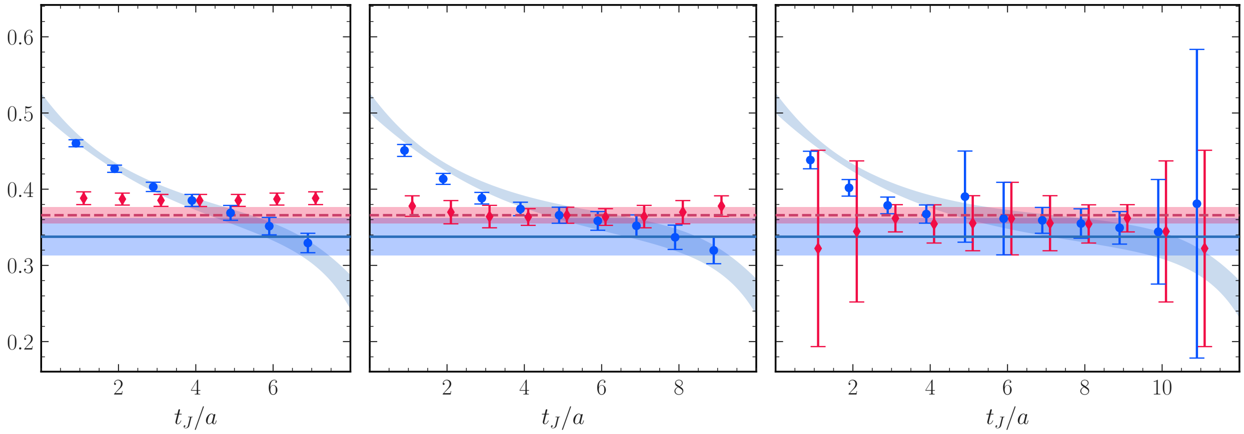

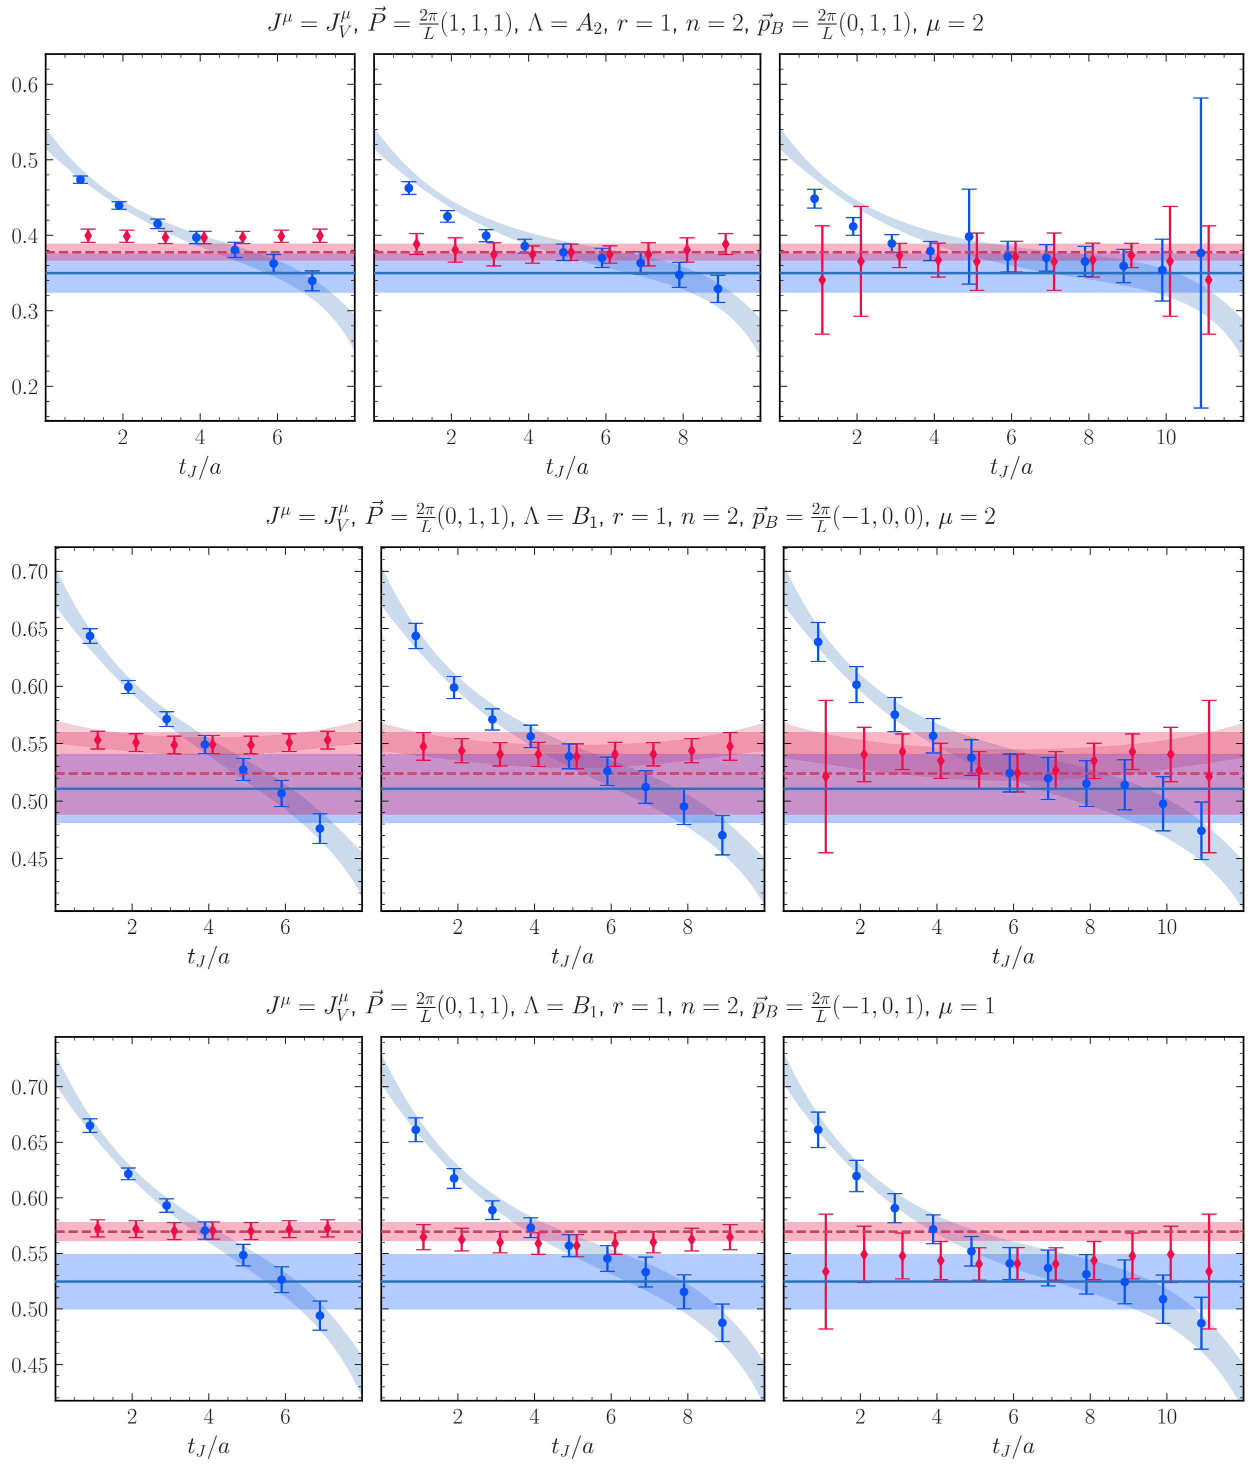

$J^\mu = J_V^\mu$, $\vec{P} = \frac{2\pi}{L}(1,1,1)$, $\Lambda = A_2$, $r = 1$, $n = 2$, $\vec{p}_B = \frac{2\pi}{L}(0,1,1)$, $\mu = 2$
0.6
0.5
0.4
0.3
0.2
2
4
6
8
10
$t_J/a$
$J^\mu = J_V^\mu$, $\vec{P} = \frac{2\pi}{L}(0,1,1)$, $\Lambda = B_1$, $r = 1$, $n = 2$, $\vec{p}_B = \frac{2\pi}{L}(-1,0,0)$, $\mu = 2$
0.70
0.65
0.60
0.55
0.50
0.45
$t_J/a$
$J^\mu = J_V^\mu$, $\vec{P} = \frac{2\pi}{L}(0,1,1)$, $\Lambda = B_1$, $r = 1$, $n = 2$, $\vec{p}_B = \frac{2\pi}{L}(-1,0,1)$, $\mu = 1$
0.70
0.65
0.60
0.55
0.50
0.45
$t_J/a$

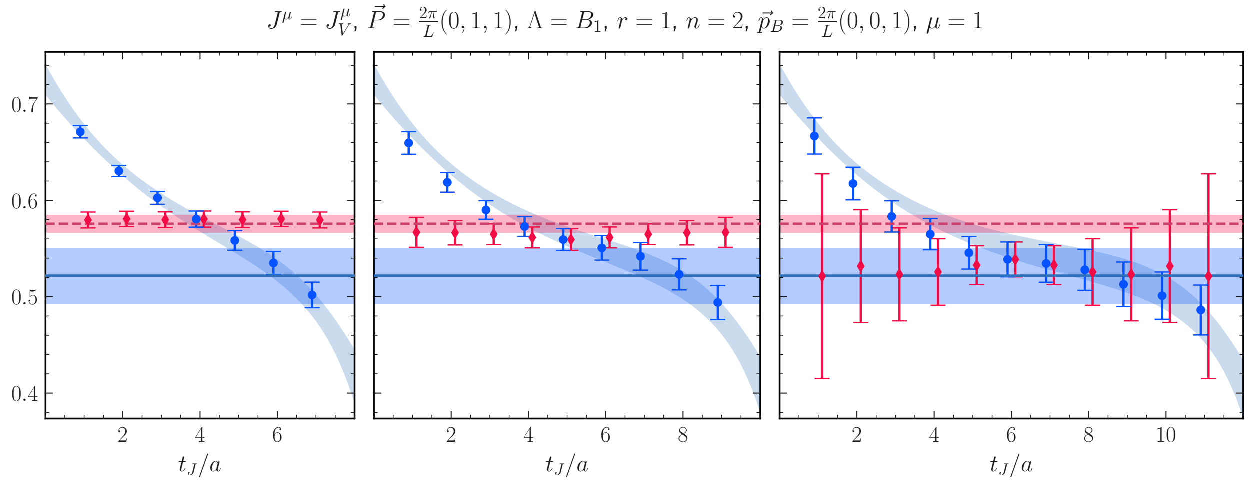
$J^\mu = J_V^\mu$, $\vec{P} = \frac{2\pi}{L}(0,1,1)$, $\Lambda = B_1$, $r = 1$, $n = 2$, $\vec{p}_B = \frac{2\pi}{L}(0,0,1)$, $\mu = 1$
$t_J/a$
$t_J/a$
$t_J/a$

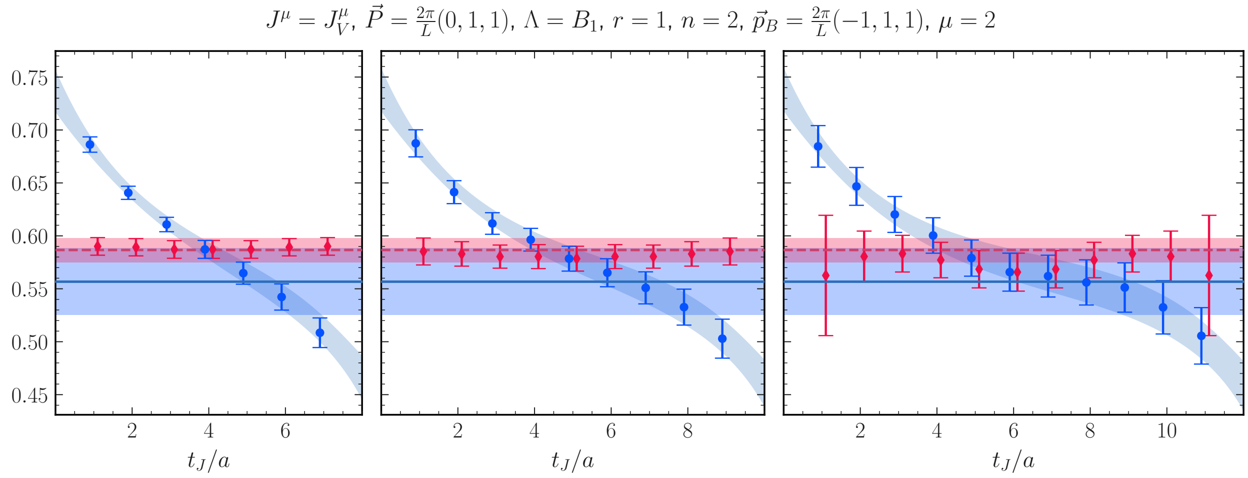
$J^\mu = J_V^\mu$, $\vec{P} = \frac{2\pi}{L}(0,1,1)$, $\Lambda = B_1$, $r = 1$, $n = 2$, $\vec{p}_B = \frac{2\pi}{L}(-1,1,1)$, $\mu = 2$
$t_J/a$
$t_J/a$
$t_J/a$

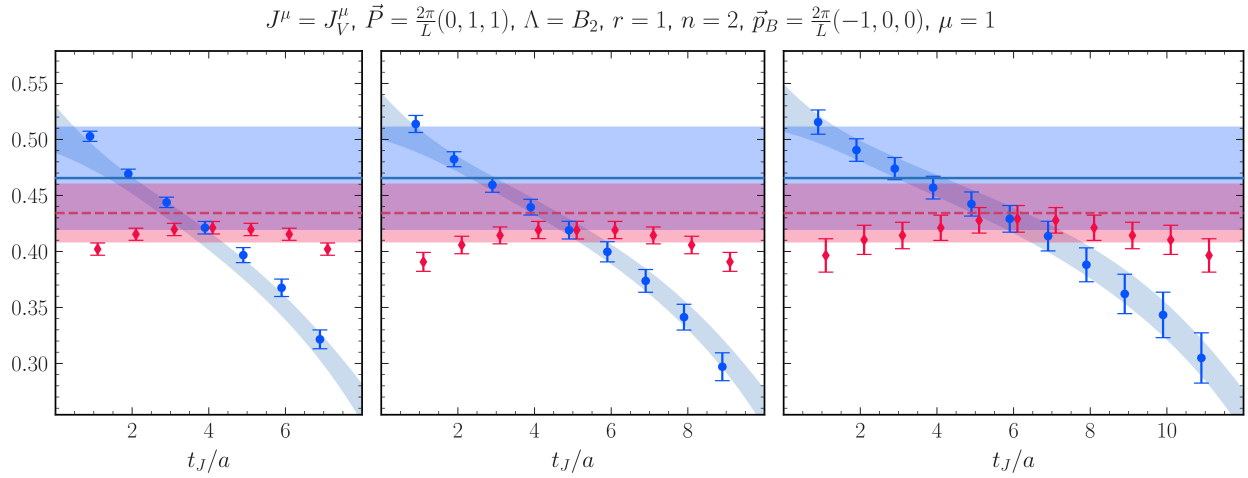
$J^\mu = J_V^\mu$, $\vec{P} = \frac{2\pi}{L}(0,1,1)$, $\Lambda = B_2$, $r = 1$, $n = 2$, $\vec{p}_B = \frac{2\pi}{L}(-1,0,0)$, $\mu = 1$
$t_J/a$
$t_J/a$
$t_J/a$

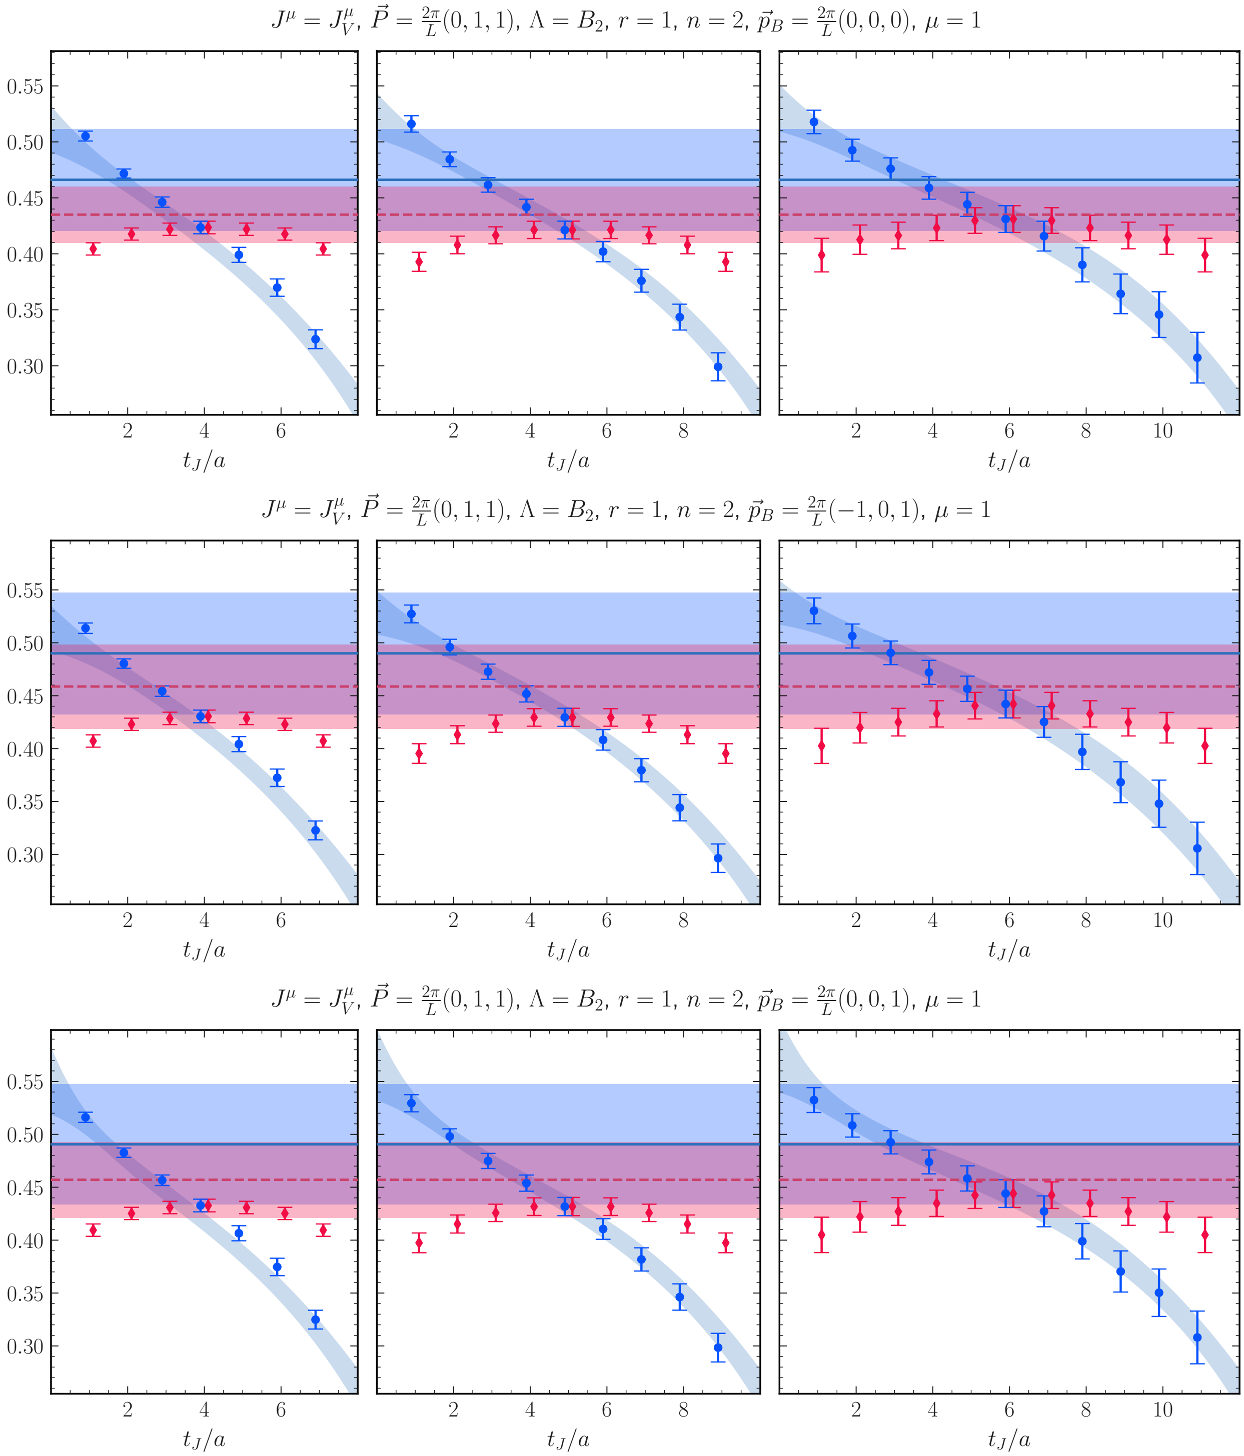
$J^\mu = J_V^\mu$, $\vec{P} = \frac{2\pi}{L}(0,1,1)$, $\Lambda = B_2$, $r = 1$, $n = 2$, $\vec{p}_B = \frac{2\pi}{L}(0,0,0)$, $\mu = 1$
$J^\mu = J_V^\mu$, $\vec{P} = \frac{2\pi}{L}(0,1,1)$, $\Lambda = B_2$, $r = 1$, $n = 2$, $\vec{p}_B = \frac{2\pi}{L}(-1,0,1)$, $\mu = 1$
$J^\mu = J_V^\mu$, $\vec{P} = \frac{2\pi}{L}(0,1,1)$, $\Lambda = B_2$, $r = 1$, $n = 2$, $\vec{p}_B = \frac{2\pi}{L}(0,0,1)$, $\mu = 1$
$t_J/a$
0.30
0.35
0.40
0.45
0.50
0.55

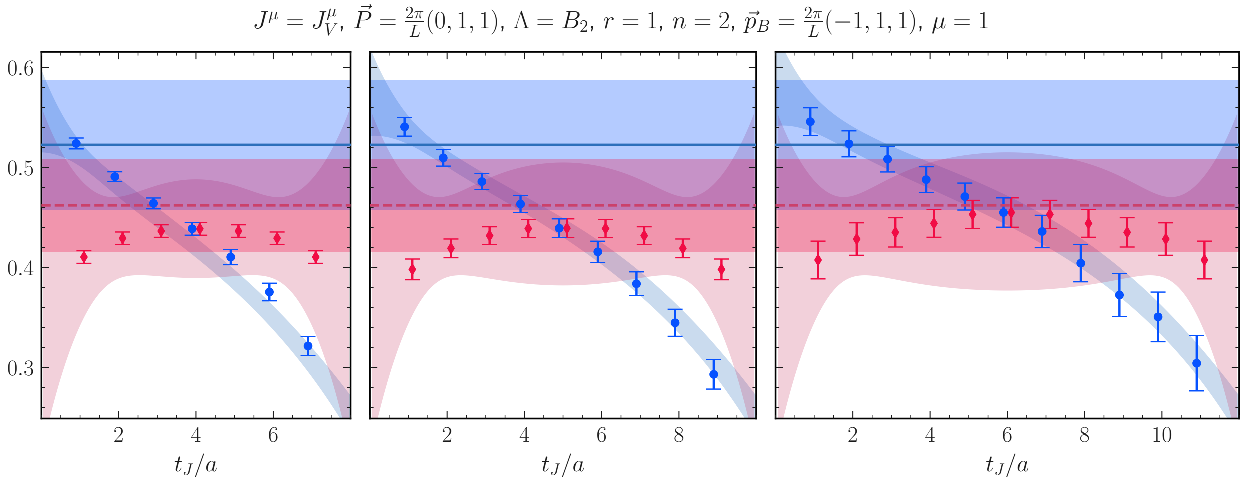
$J^\mu = J_V^\mu$, $\vec{P} = \frac{2\pi}{L}(0,1,1)$, $\Lambda = B_2$, $r = 1$, $n = 2$, $\vec{p}_B = \frac{2\pi}{L}(-1,1,1)$, $\mu = 1$
$t_J/a$
$t_J/a$
$t_J/a$

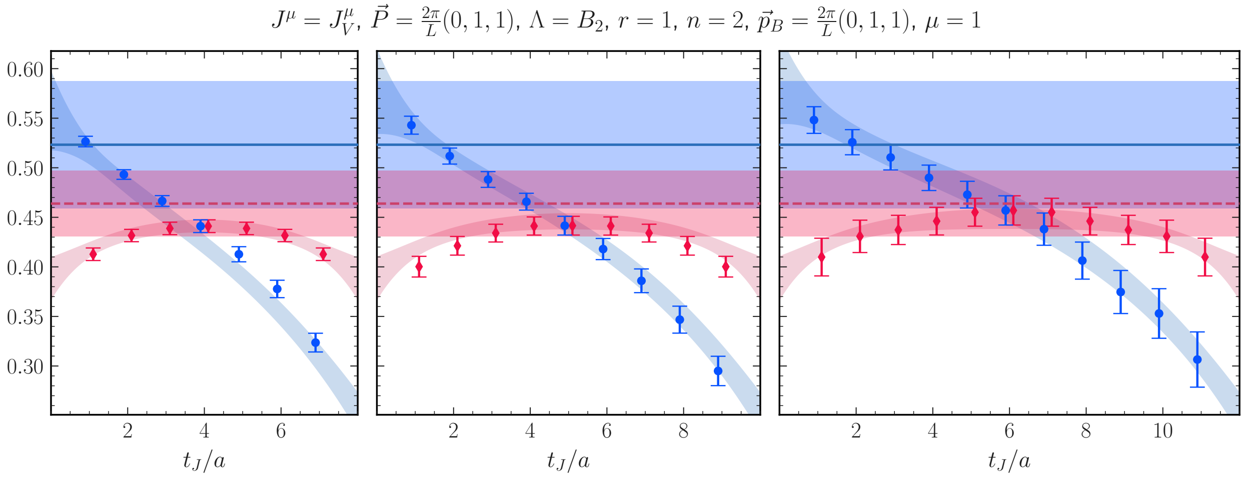
$J^\mu = J_V^\mu$, $\vec{P} = \frac{2\pi}{L}(0,1,1)$, $\Lambda = B_2$, $r = 1$, $n = 2$, $\vec{p}_B = \frac{2\pi}{L}(0,1,1)$, $\mu = 1$
$t_J/a$
$t_J/a$
$t_J/a$

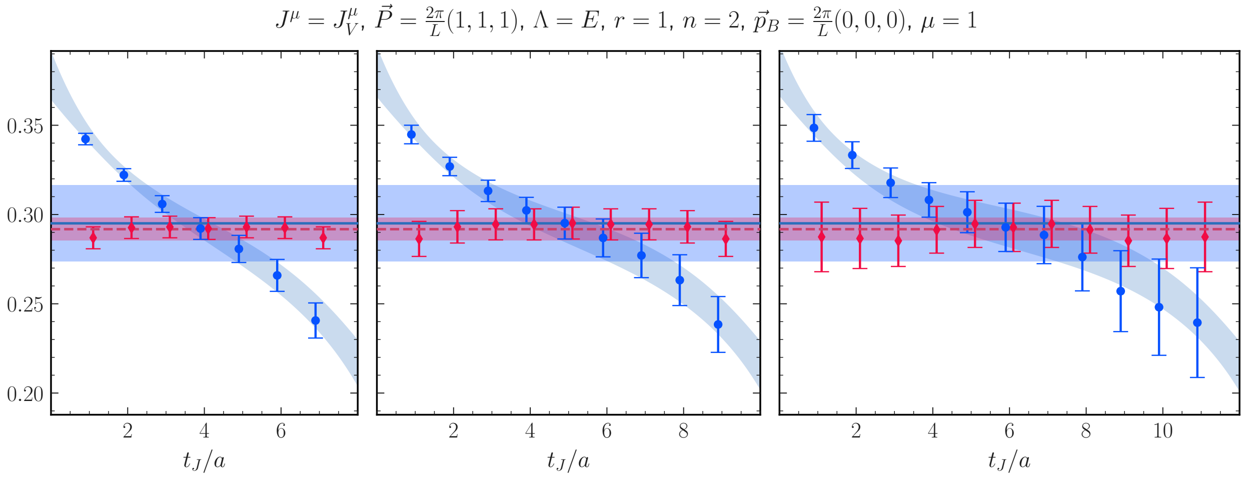
$J^\mu = J_V^\mu$, $\vec{P} = \frac{2\pi}{L}(1,1,1)$, $\Lambda = E$, $r = 1$, $n = 2$, $\vec{p}_B = \frac{2\pi}{L}(0,0,0)$, $\mu = 1$
$t_J/a$
$t_J/a$
$t_J/a$

$J^\mu = J_V^\mu$, $\vec{P} = \frac{2\pi}{L}(1,1,1)$, $\Lambda = E$, $r = 1$, $n = 2$, $\vec{p}_B = \frac{2\pi}{L}(0,0,1)$, $\mu = 1$

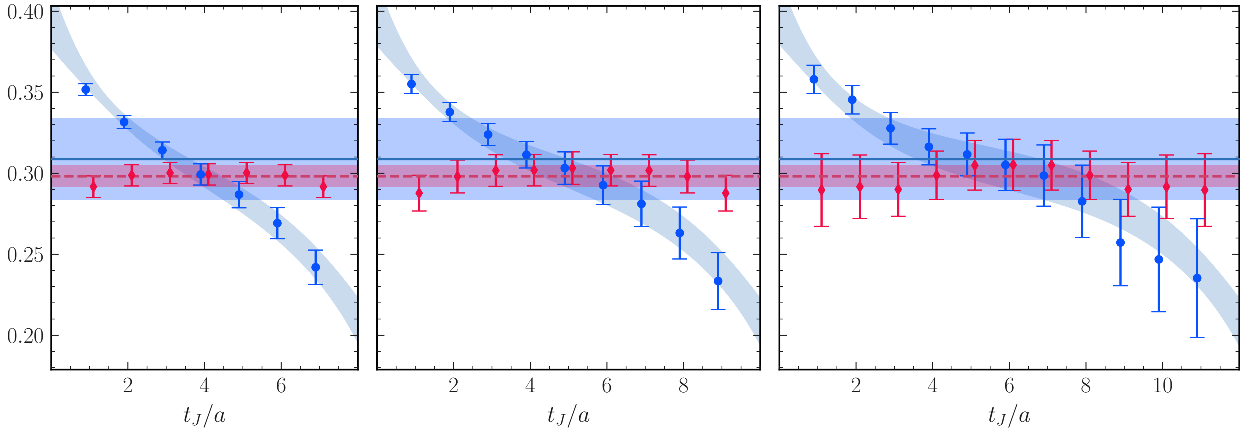


$J^\mu = J_V^\mu$, $\vec{P} = \frac{2\pi}{L}(1,1,1)$, $\Lambda = E$, $r = 1$, $n = 2$, $\vec{p}_B = \frac{2\pi}{L}(0,1,1)$, $\mu = 1$

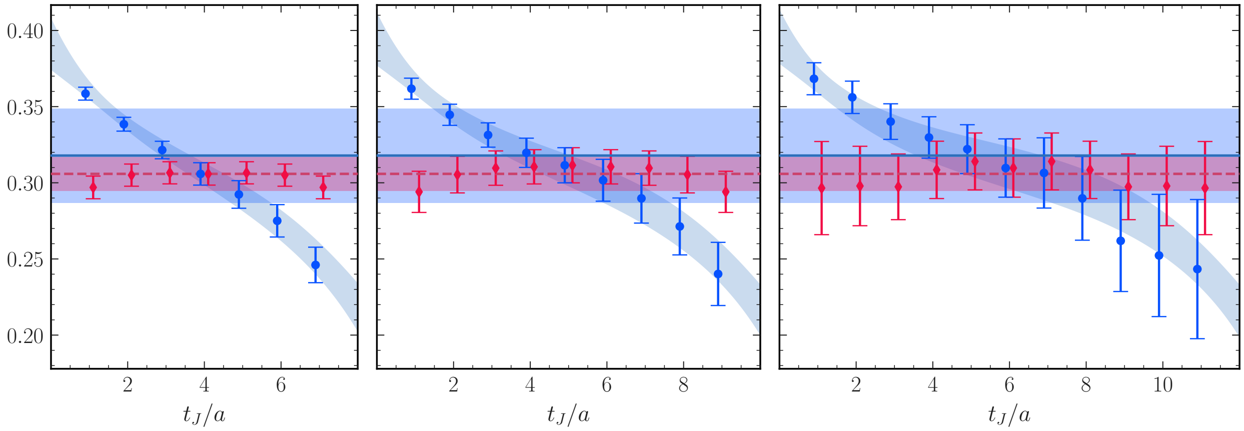


$J^\mu = J_V^\mu$, $\vec{P} = \frac{2\pi}{L}(1,1,1)$, $\Lambda = E$, $r = 1$, $n = 2$, $\vec{p}_B = \frac{2\pi}{L}(1,1,1)$, $\mu = 1$

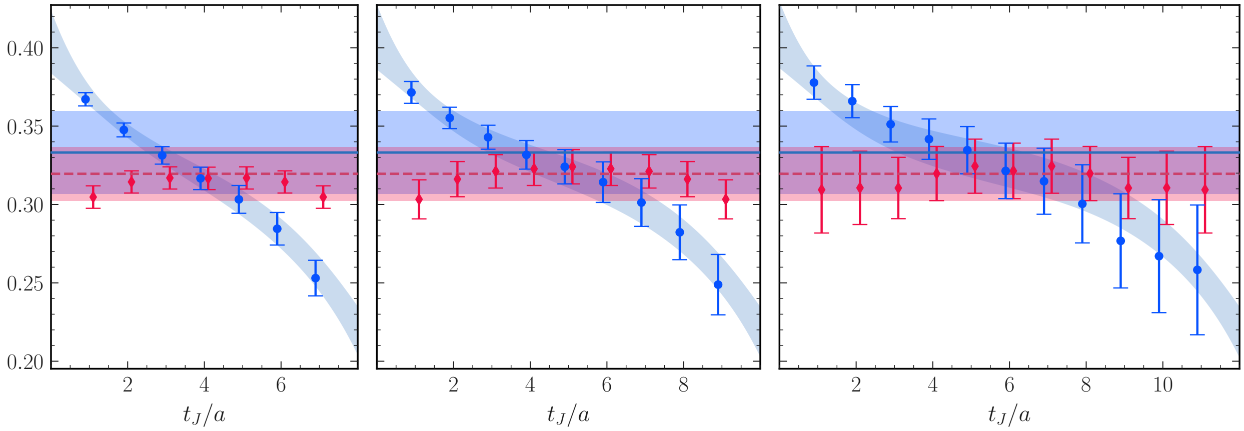

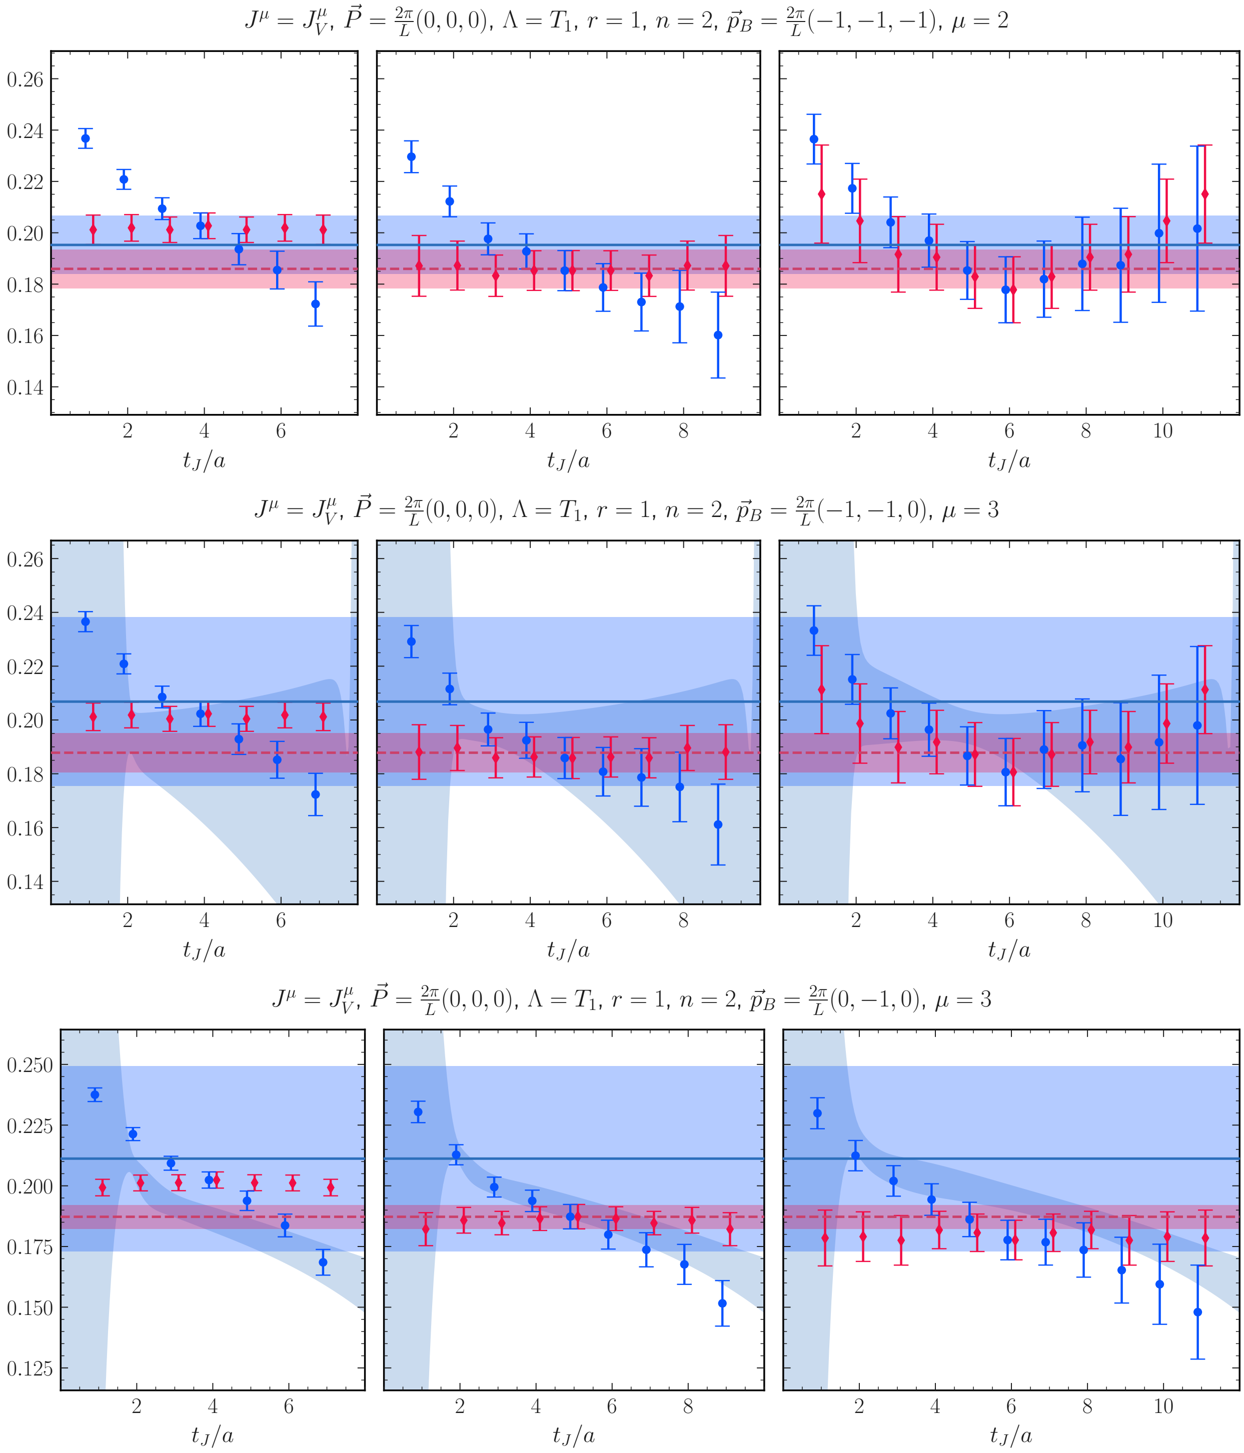
$J^\mu = J_V^\mu$, $\vec{P} = \frac{2\pi}{L}(0,0,0)$, $\Lambda = T_1$, $r = 1$, $n = 2$, $\vec{p}_B = \frac{2\pi}{L}(-1,-1,-1)$, $\mu = 2$
$J^\mu = J_V^\mu$, $\vec{P} = \frac{2\pi}{L}(0,0,0)$, $\Lambda = T_1$, $r = 1$, $n = 2$, $\vec{p}_B = \frac{2\pi}{L}(-1,-1,0)$, $\mu = 3$
$J^\mu = J_V^\mu$, $\vec{P} = \frac{2\pi}{L}(0,0,0)$, $\Lambda = T_1$, $r = 1$, $n = 2$, $\vec{p}_B = \frac{2\pi}{L}(0,-1,0)$, $\mu = 3$
$t_J/a$

$J^\mu = J_V^\mu,\ \vec{P} = \frac{2\pi}{L}(0,0,1),\ \Lambda = E,\ r = 1,\ n = 2,\ \vec{p}_B = \frac{2\pi}{L}(-1,-1,0),\ \mu = 2$

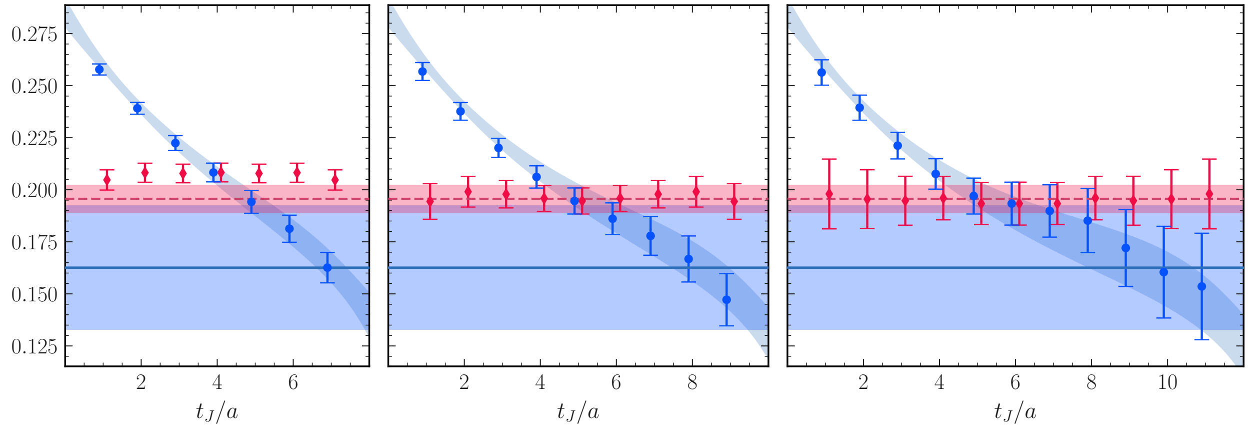


$J^\mu = J_V^\mu,\ \vec{P} = \frac{2\pi}{L}(0,0,1),\ \Lambda = E,\ r = 1,\ n = 2,\ \vec{p}_B = \frac{2\pi}{L}(-1,0,0),\ \mu = 2$

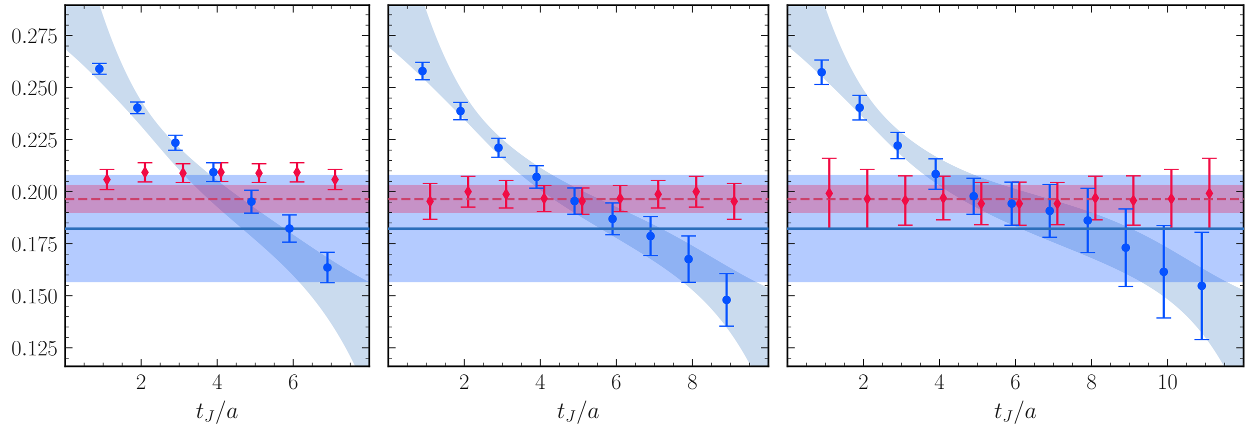


$J^\mu = J_V^\mu,\ \vec{P} = \frac{2\pi}{L}(0,0,1),\ \Lambda = E,\ r = 1,\ n = 2,\ \vec{p}_B = \frac{2\pi}{L}(0,0,0),\ \mu = 2$

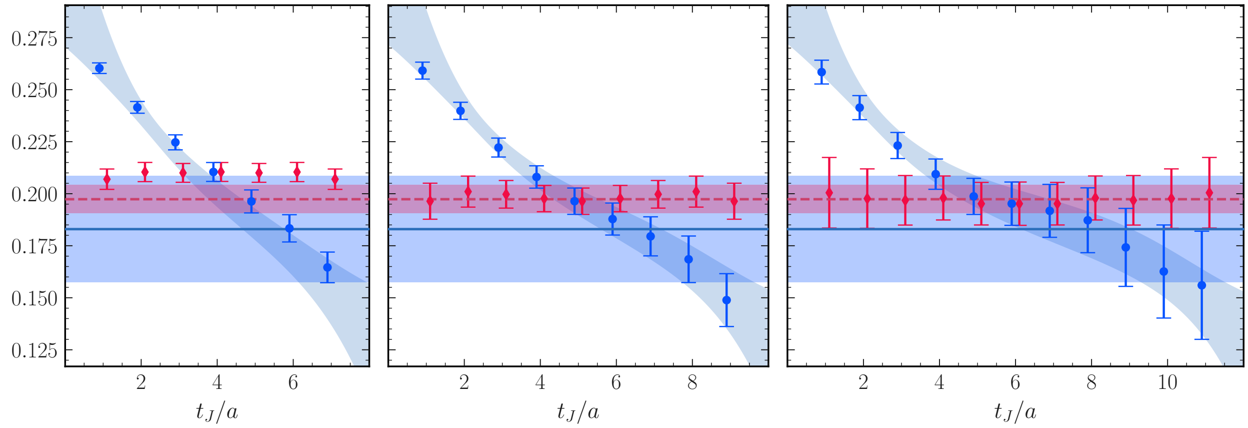

$J^\mu = J_V^\mu$, $\vec{P} = \frac{2\pi}{L}(0,0,1)$, $\Lambda = E$, $r = 1$, $n = 2$, $\vec{p}_B = \frac{2\pi}{L}(-1,-1,1)$, $\mu = 2$

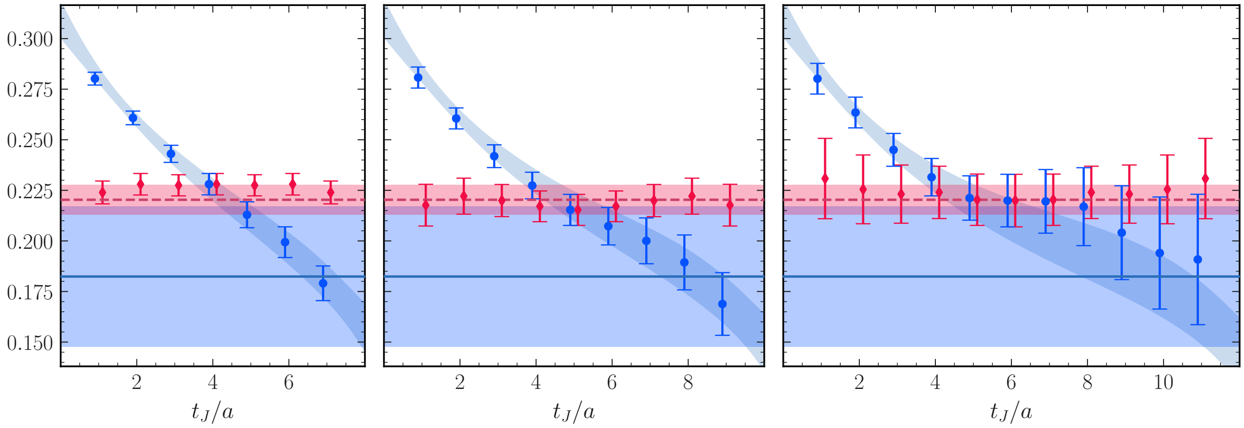


$J^\mu = J_V^\mu$, $\vec{P} = \frac{2\pi}{L}(0,0,1)$, $\Lambda = E$, $r = 1$, $n = 2$, $\vec{p}_B = \frac{2\pi}{L}(-1,0,1)$, $\mu = 2$

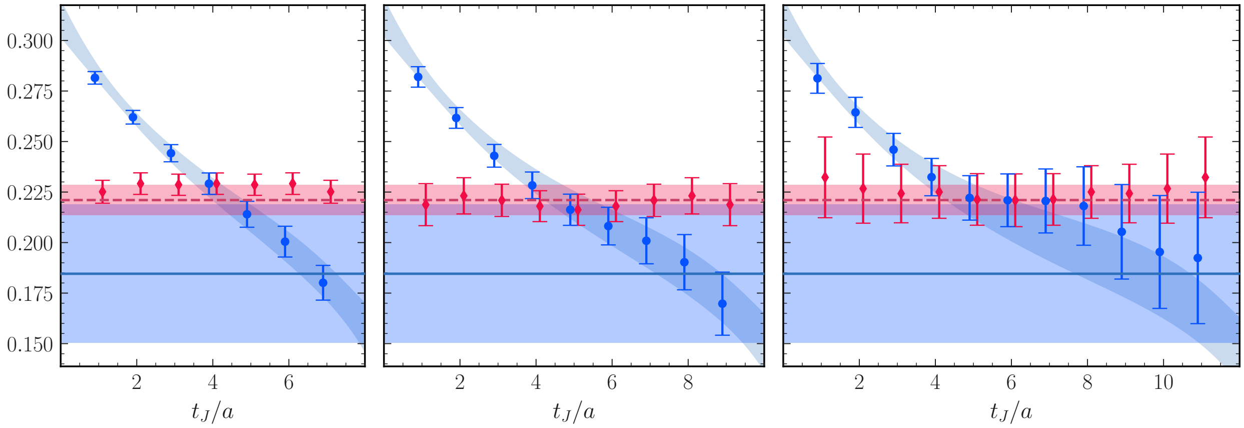


$J^\mu = J_V^\mu$, $\vec{P} = \frac{2\pi}{L}(0,0,1)$, $\Lambda = E$, $r = 1$, $n = 2$, $\vec{p}_B = \frac{2\pi}{L}(0,0,1)$, $\mu = 2$

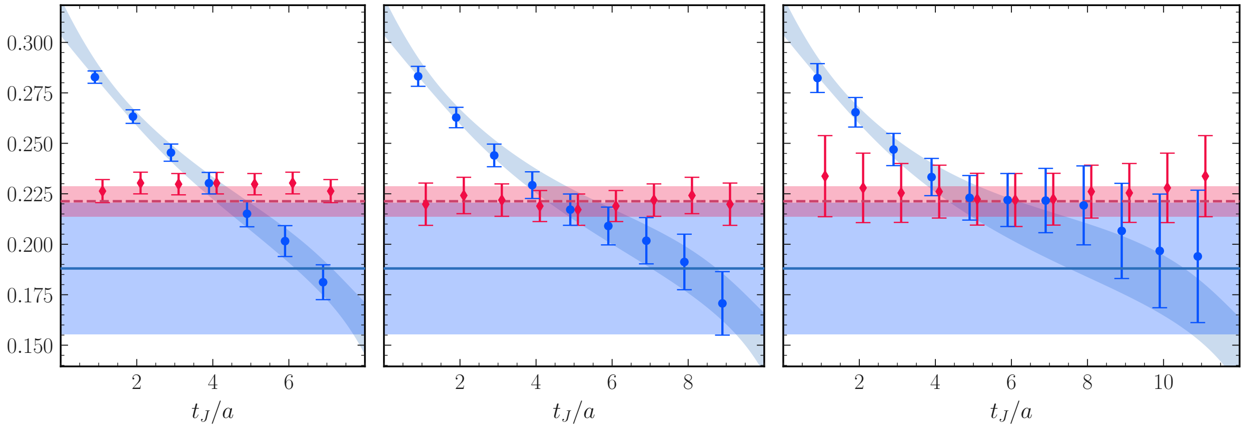

## V. PLOTS OF THE FITS FOR THE AXIAL-CURRENT MATRIX ELEMENTS

The axial-current matrix elements come with three form factors and thus cannot be simply factored; here we show the lattice-determined matrix elements with the kinematical factors included. For the description of the figure content see Sec. IV.

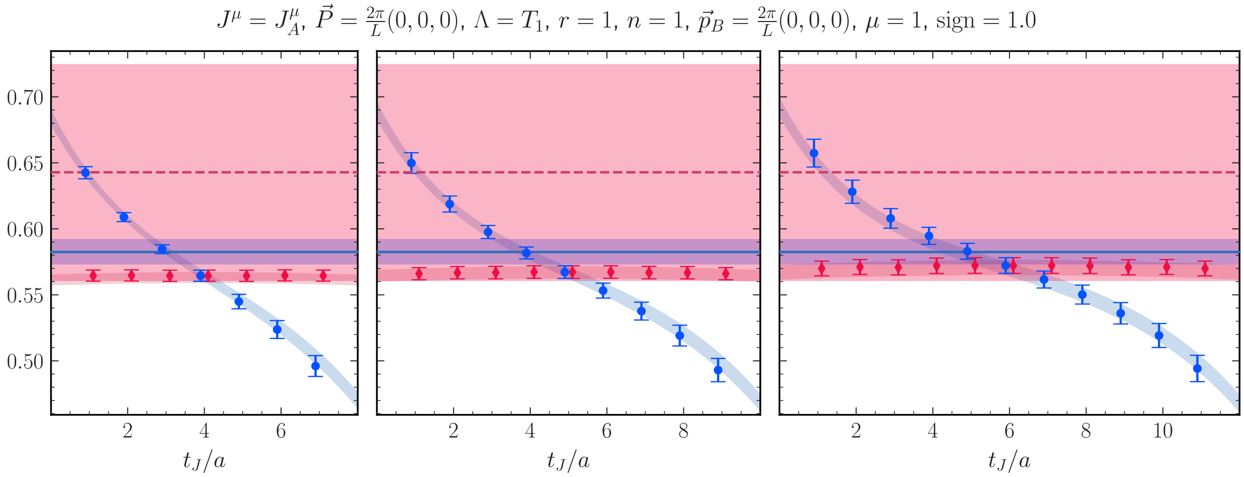

$J^\mu = J_A^\mu$, $\vec{P} = \frac{2\pi}{L}(0,0,0)$, $\Lambda = T_1$, $r = 1$, $n = 1$, $\vec{p}_B = \frac{2\pi}{L}(0,0,0)$, $\mu = 1$, sign $= 1.0$
0.70
0.65
0.60
0.55
0.50
$t_J/a$


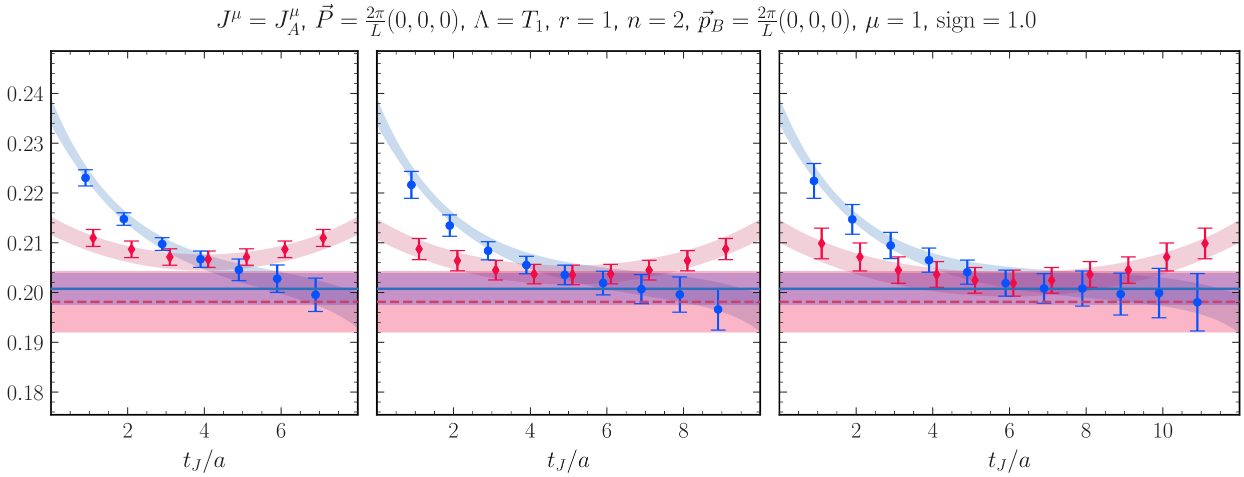

$J^\mu = J_A^\mu$, $\vec{P} = \frac{2\pi}{L}(0,0,0)$, $\Lambda = T_1$, $r = 1$, $n = 2$, $\vec{p}_B = \frac{2\pi}{L}(0,0,0)$, $\mu = 1$, sign $= 1.0$
0.24
0.23
0.22
0.21
0.20
0.19
0.18
$t_J/a$


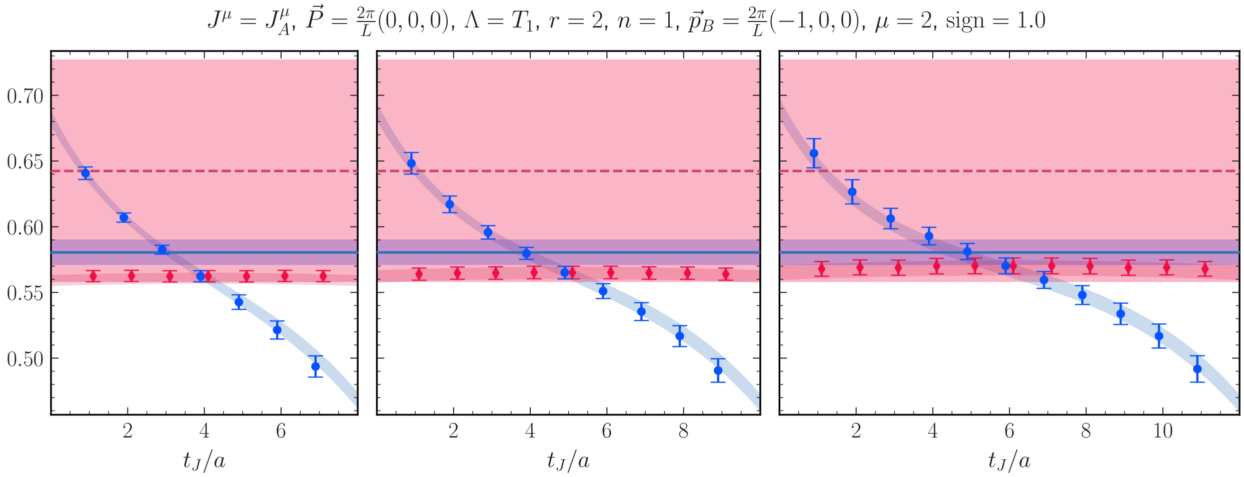

$J^\mu = J_A^\mu$, $\vec{P} = \frac{2\pi}{L}(0,0,0)$, $\Lambda = T_1$, $r = 2$, $n = 1$, $\vec{p}_B = \frac{2\pi}{L}(-1,0,0)$, $\mu = 2$, sign $= 1.0$
0.70
0.65
0.60
0.55
0.50
$t_J/a$

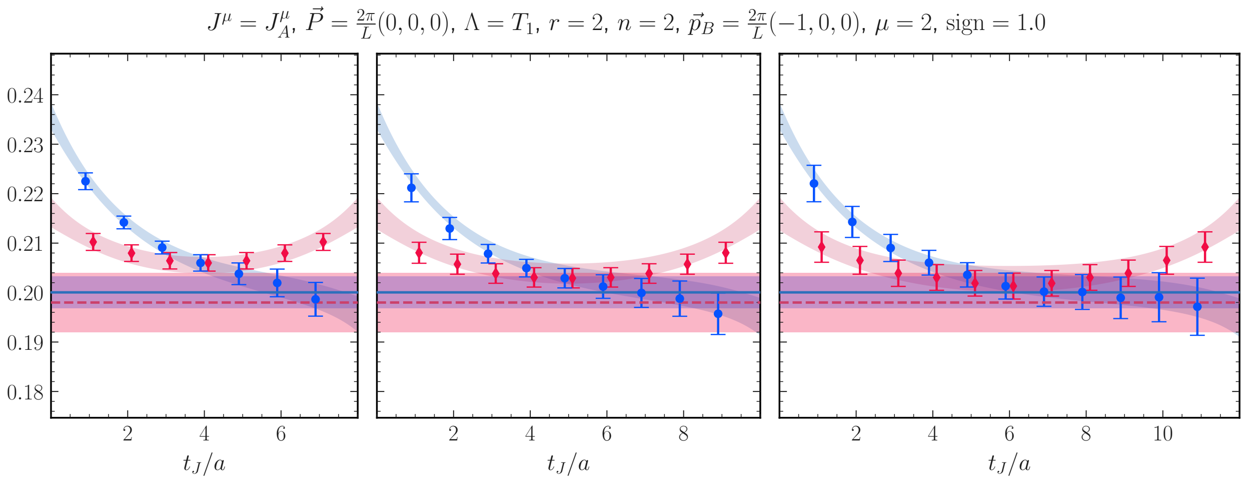
$J^\mu = J_A^\mu$, $\vec{P} = \frac{2\pi}{L}(0,0,0)$, $\Lambda = T_1$, $r = 2$, $n = 2$, $\vec{p}_B = \frac{2\pi}{L}(-1,0,0)$, $\mu = 2$, sign = 1.0
$t_J/a$

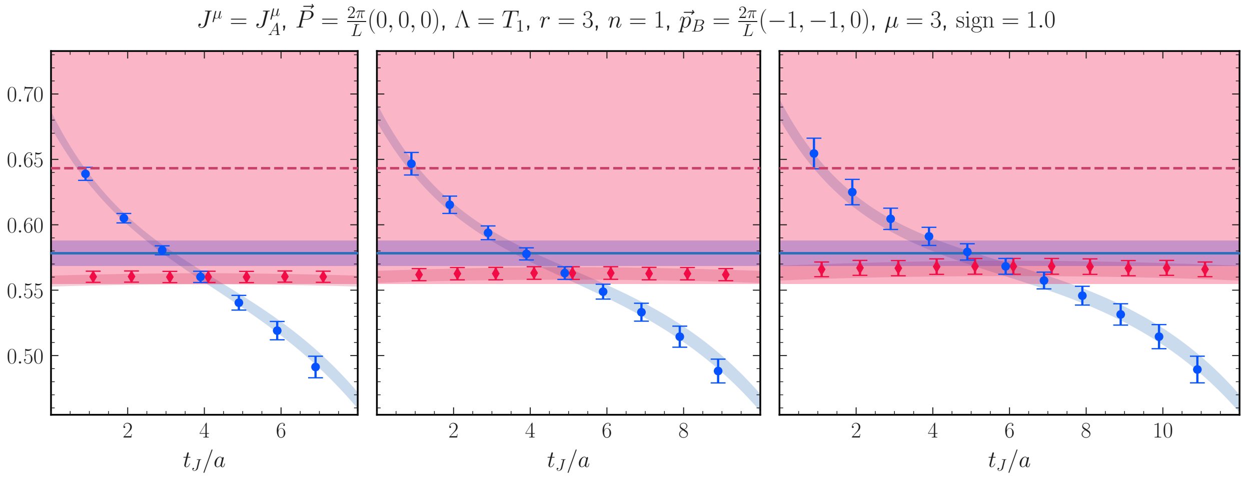
$J^\mu = J_A^\mu$, $\vec{P} = \frac{2\pi}{L}(0,0,0)$, $\Lambda = T_1$, $r = 3$, $n = 1$, $\vec{p}_B = \frac{2\pi}{L}(-1,-1,0)$, $\mu = 3$, sign = 1.0
$t_J/a$

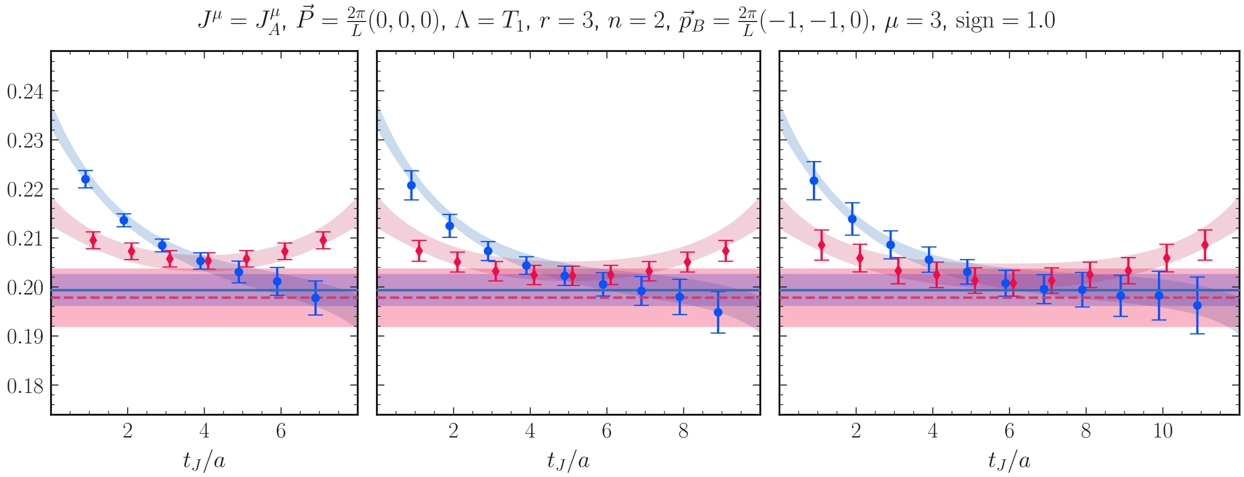
$J^\mu = J_A^\mu$, $\vec{P} = \frac{2\pi}{L}(0,0,0)$, $\Lambda = T_1$, $r = 3$, $n = 2$, $\vec{p}_B = \frac{2\pi}{L}(-1,-1,0)$, $\mu = 3$, sign = 1.0
$t_J/a$

$J^\mu = J_A^\mu$, $\vec{P} = \frac{2\pi}{L}(0,0,1)$, $\Lambda = A_2$, $r = 1$, $n = 1$, $\vec{p}_B = \frac{2\pi}{L}(-1,-1,0)$, $\mu = 0$, sign $= -1.0$

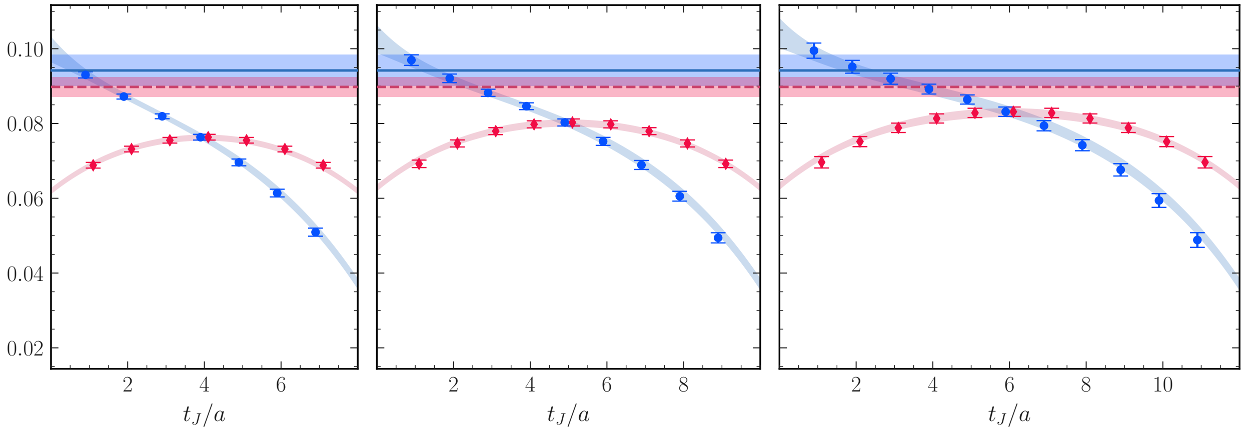


$J^\mu = J_A^\mu$, $\vec{P} = \frac{2\pi}{L}(0,0,1)$, $\Lambda = A_2$, $r = 1$, $n = 1$, $\vec{p}_B = \frac{2\pi}{L}(-1,-1,0)$, $\mu = 3$, sign $= 1.0$

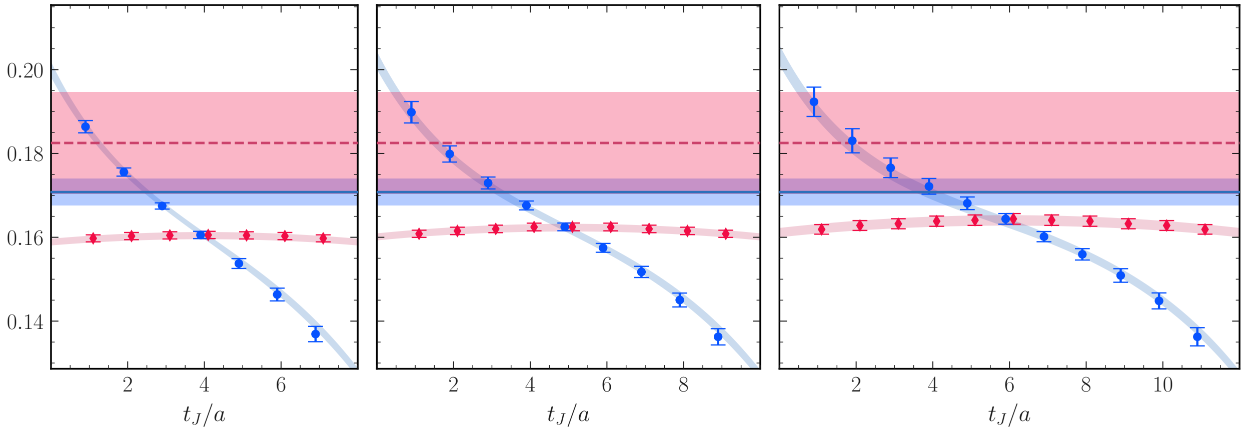


$J^\mu = J_A^\mu$, $\vec{P} = \frac{2\pi}{L}(0,0,1)$, $\Lambda = A_2$, $r = 1$, $n = 1$, $\vec{p}_B = \frac{2\pi}{L}(-1,-1,1)$, $\mu = 0$, sign $= -1.0$

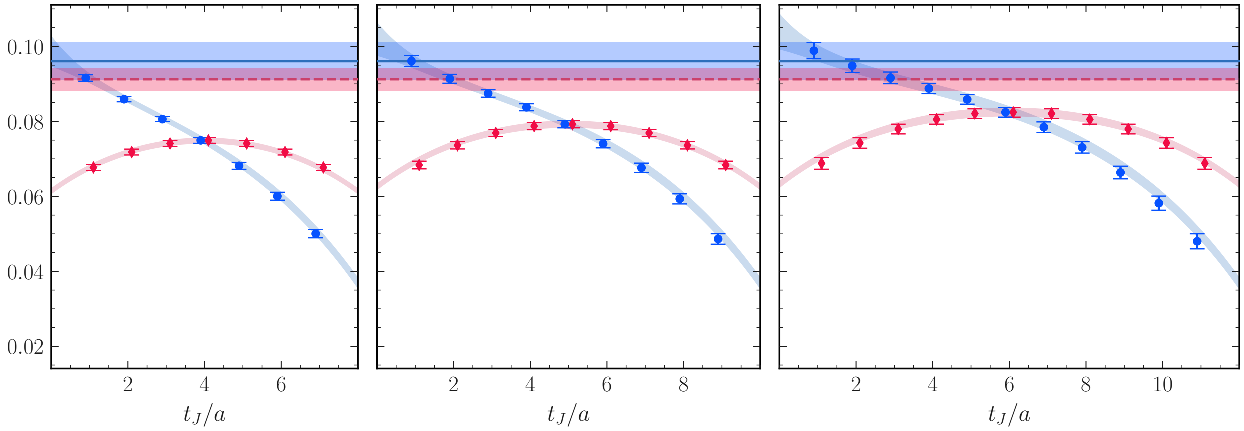

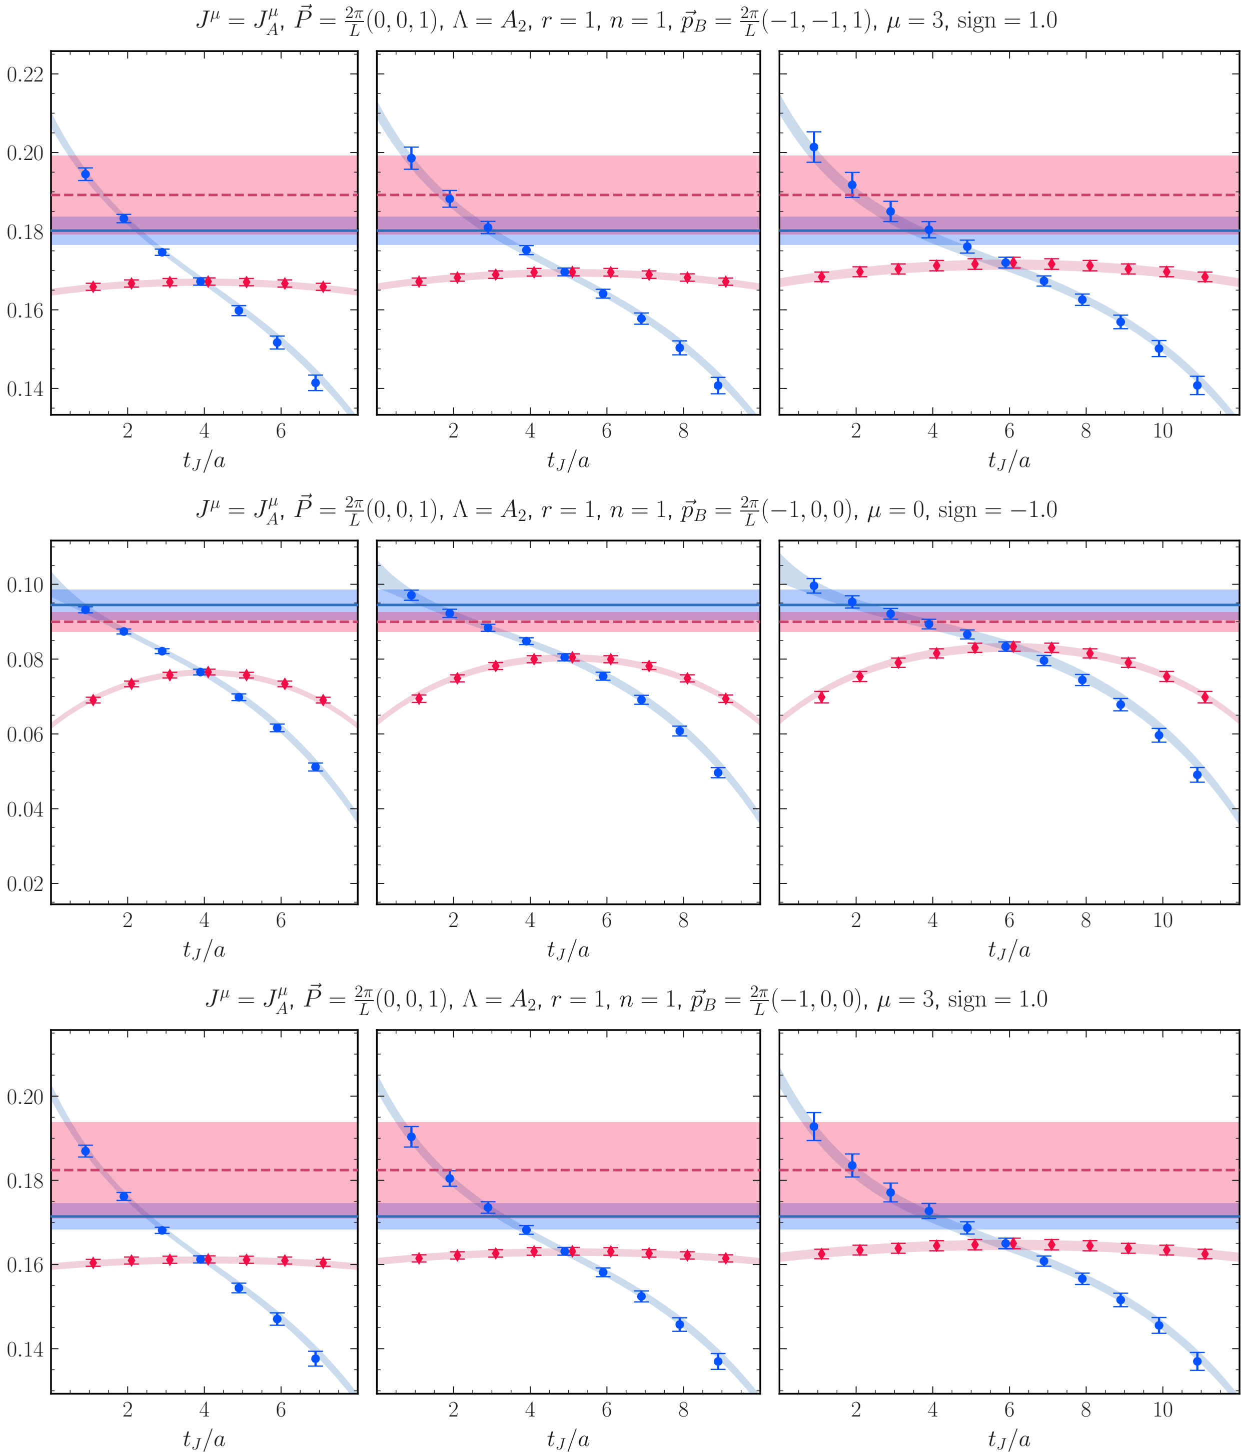

$J^\mu = J_A^\mu$, $\vec{P} = \frac{2\pi}{L}(0,0,1)$, $\Lambda = A_2$, $r = 1$, $n = 1$, $\vec{p}_B = \frac{2\pi}{L}(-1,-1,1)$, $\mu = 3$, sign $= 1.0$
$J^\mu = J_A^\mu$, $\vec{P} = \frac{2\pi}{L}(0,0,1)$, $\Lambda = A_2$, $r = 1$, $n = 1$, $\vec{p}_B = \frac{2\pi}{L}(-1,0,0)$, $\mu = 0$, sign $= -1.0$
$J^\mu = J_A^\mu$, $\vec{P} = \frac{2\pi}{L}(0,0,1)$, $\Lambda = A_2$, $r = 1$, $n = 1$, $\vec{p}_B = \frac{2\pi}{L}(-1,0,0)$, $\mu = 3$, sign $= 1.0$
$t_J/a$

$J^\mu = J_A^\mu$, $\vec{P} = \frac{2\pi}{L}(0,0,1)$, $\Lambda = A_2$, $r = 1$, $n = 1$, $\vec{p}_B = \frac{2\pi}{L}(-1,0,1)$, $\mu = 0$, sign $= -1.0$

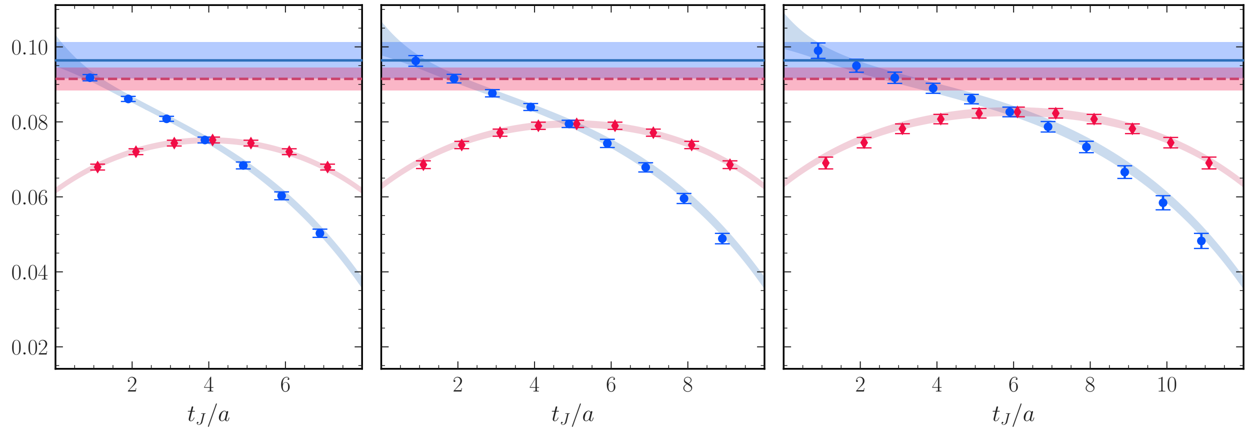


$J^\mu = J_A^\mu$, $\vec{P} = \frac{2\pi}{L}(0,0,1)$, $\Lambda = A_2$, $r = 1$, $n = 1$, $\vec{p}_B = \frac{2\pi}{L}(-1,0,1)$, $\mu = 3$, sign $= 1.0$

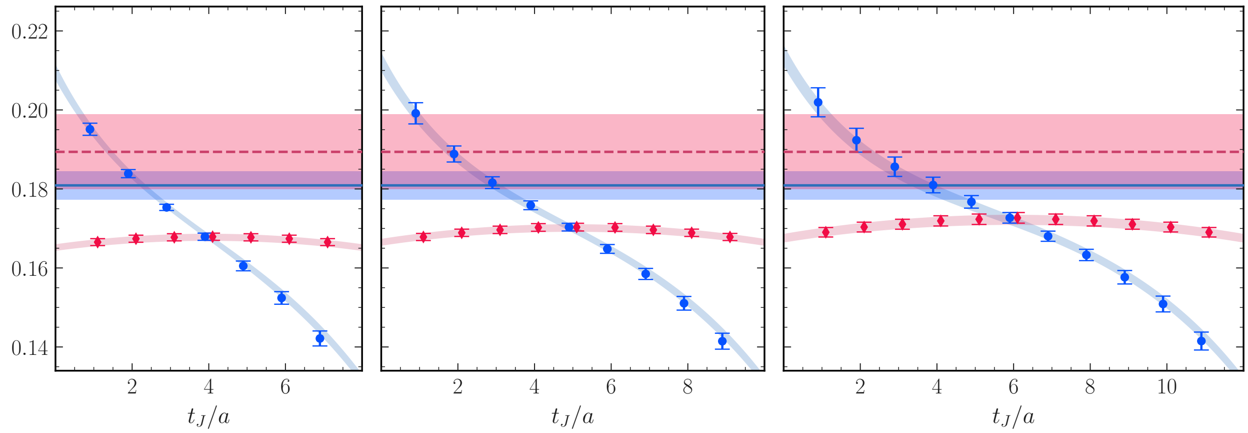


$J^\mu = J_A^\mu$, $\vec{P} = \frac{2\pi}{L}(0,0,1)$, $\Lambda = A_2$, $r = 1$, $n = 1$, $\vec{p}_B = \frac{2\pi}{L}(0,0,0)$, $\mu = 0$, sign $= -1.0$

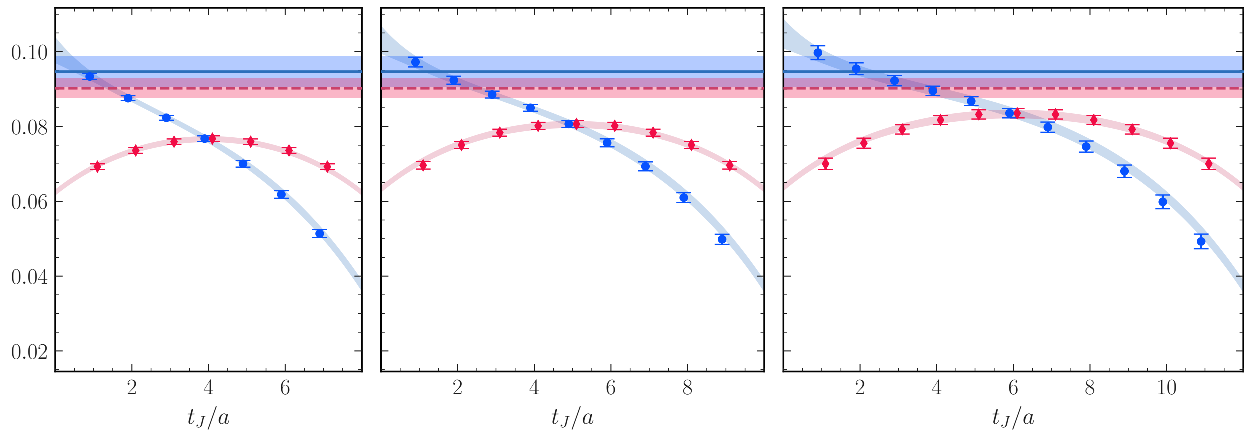

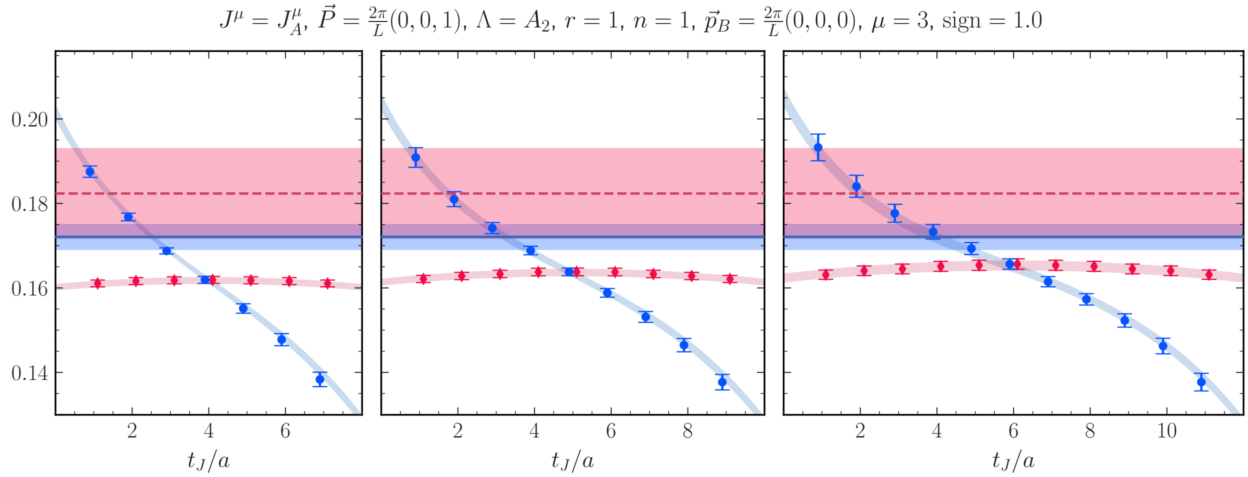
$J^\mu = J_A^\mu$, $\vec{P} = \frac{2\pi}{L}(0,0,1)$, $\Lambda = A_2$, $r = 1$, $n = 1$, $\vec{p}_B = \frac{2\pi}{L}(0,0,0)$, $\mu = 3$, sign = 1.0
0.20
0.18
0.16
0.14
2 4 6
2 4 6 8
2 4 6 8 10
$t_J/a$
$t_J/a$
$t_J/a$

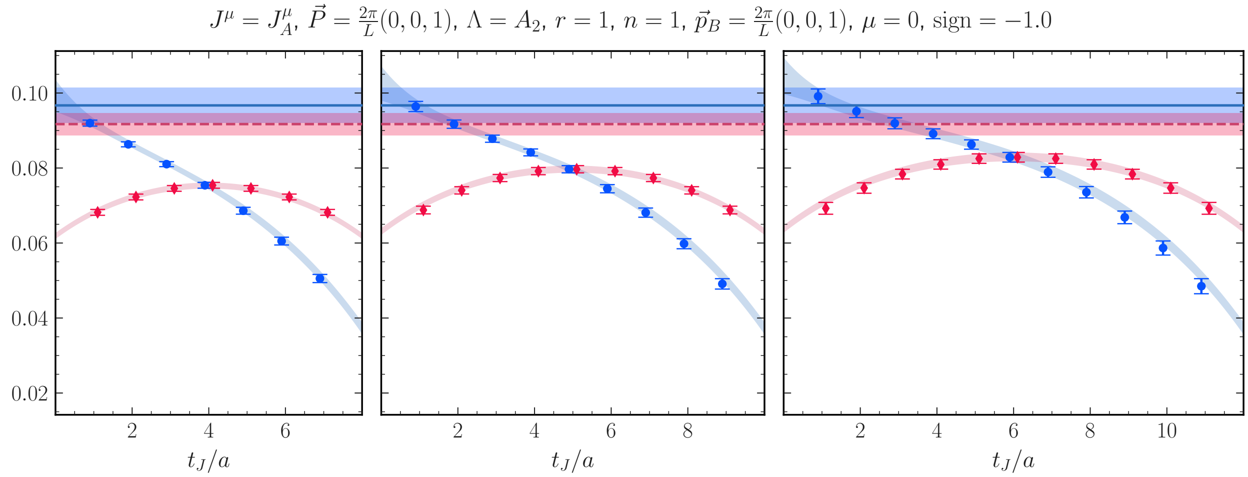
$J^\mu = J_A^\mu$, $\vec{P} = \frac{2\pi}{L}(0,0,1)$, $\Lambda = A_2$, $r = 1$, $n = 1$, $\vec{p}_B = \frac{2\pi}{L}(0,0,1)$, $\mu = 0$, sign = −1.0
0.10
0.08
0.06
0.04
0.02
2 4 6
2 4 6 8
2 4 6 8 10
$t_J/a$
$t_J/a$
$t_J/a$

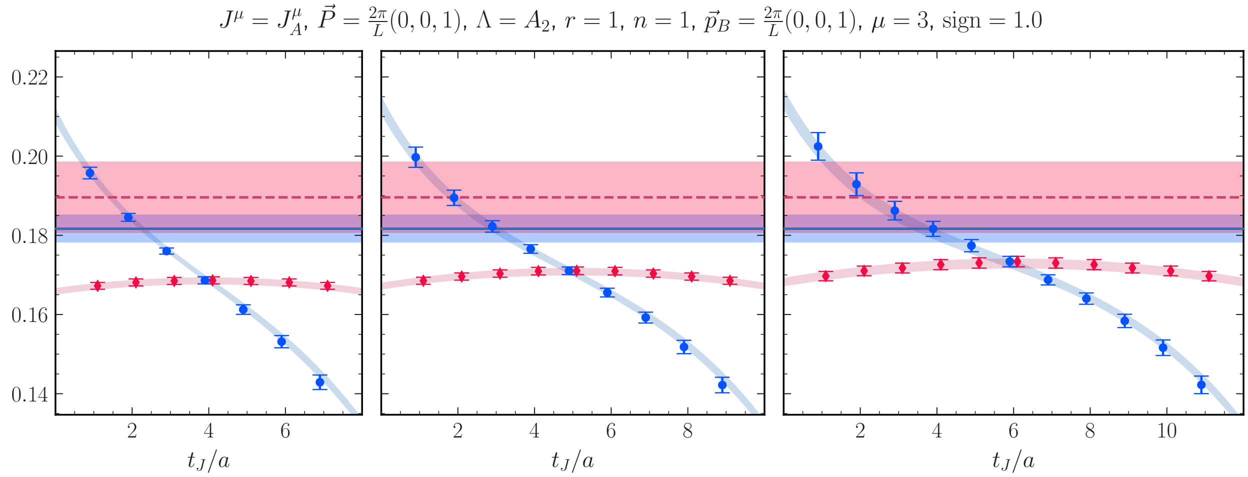
$J^\mu = J_A^\mu$, $\vec{P} = \frac{2\pi}{L}(0,0,1)$, $\Lambda = A_2$, $r = 1$, $n = 1$, $\vec{p}_B = \frac{2\pi}{L}(0,0,1)$, $\mu = 3$, sign = 1.0
0.22
0.20
0.18
0.16
0.14
2 4 6
2 4 6 8
2 4 6 8 10
$t_J/a$
$t_J/a$
$t_J/a$

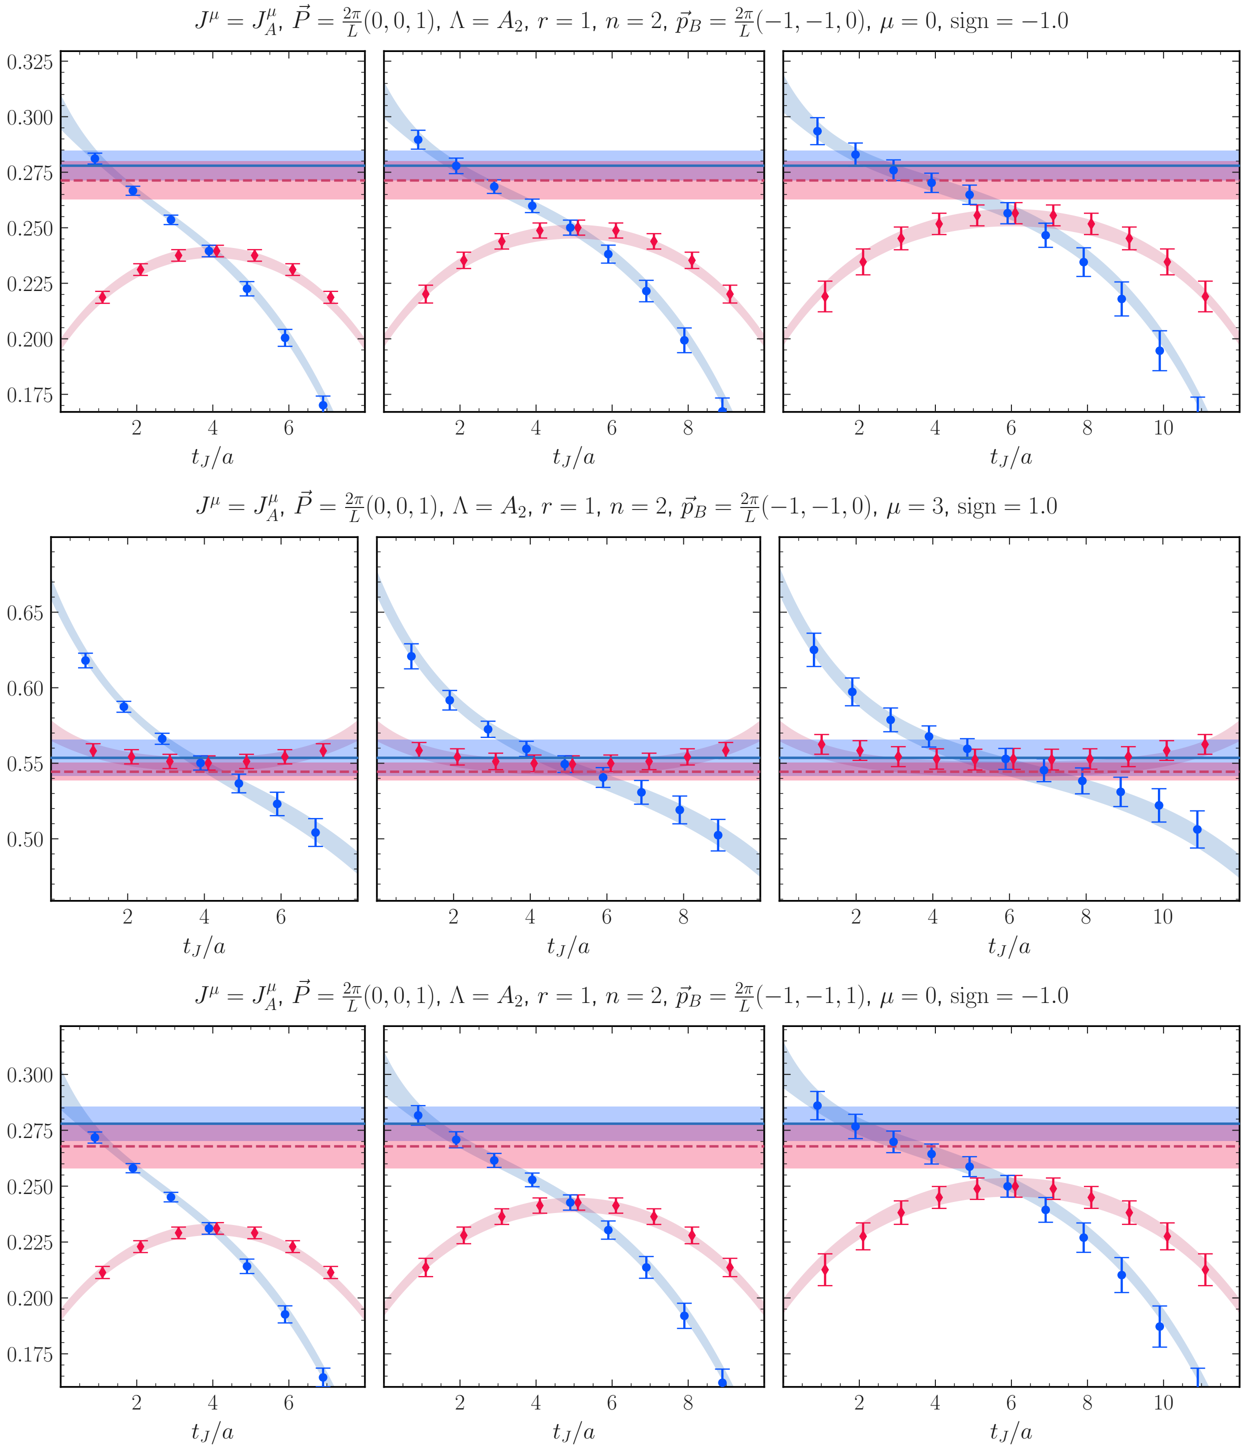

$J^\mu = J^\mu_A$, $\vec{P} = \frac{2\pi}{L}(0,0,1)$, $\Lambda = A_2$, $r = 1$, $n = 2$, $\vec{p}_B = \frac{2\pi}{L}(-1,-1,0)$, $\mu = 0$, sign $= -1.0$
$t_J/a$
$J^\mu = J^\mu_A$, $\vec{P} = \frac{2\pi}{L}(0,0,1)$, $\Lambda = A_2$, $r = 1$, $n = 2$, $\vec{p}_B = \frac{2\pi}{L}(-1,-1,0)$, $\mu = 3$, sign $= 1.0$
$t_J/a$
$J^\mu = J^\mu_A$, $\vec{P} = \frac{2\pi}{L}(0,0,1)$, $\Lambda = A_2$, $r = 1$, $n = 2$, $\vec{p}_B = \frac{2\pi}{L}(-1,-1,1)$, $\mu = 0$, sign $= -1.0$
$t_J/a$

$J^\mu = J^\mu_A$, $\vec{P} = \frac{2\pi}{L}(0,0,1)$, $\Lambda = A_2$, $r = 1$, $n = 2$, $\vec{p}_B = \frac{2\pi}{L}(-1,-1,1)$, $\mu = 3$, sign $= 1.0$

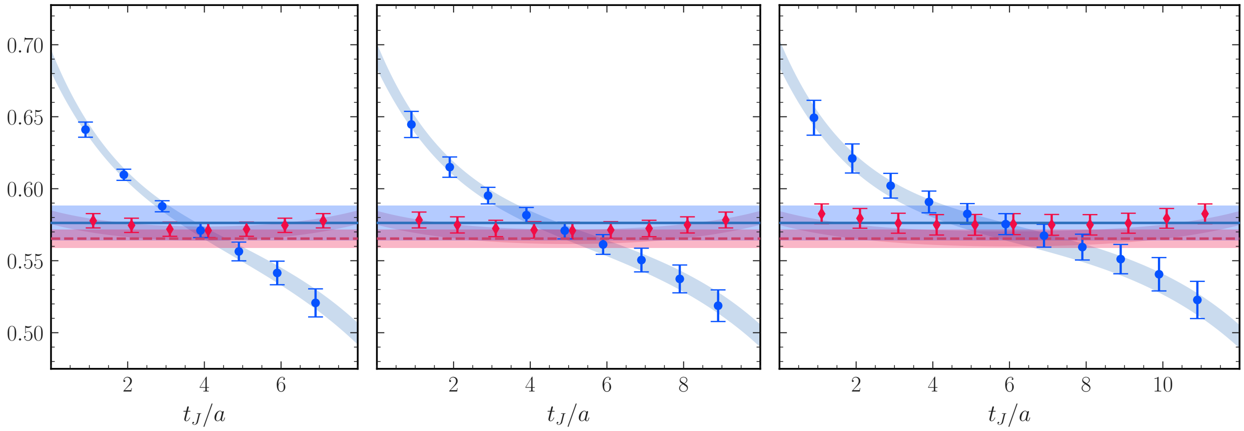


$J^\mu = J^\mu_A$, $\vec{P} = \frac{2\pi}{L}(0,0,1)$, $\Lambda = A_2$, $r = 1$, $n = 2$, $\vec{p}_B = \frac{2\pi}{L}(-1,0,0)$, $\mu = 0$, sign $= -1.0$

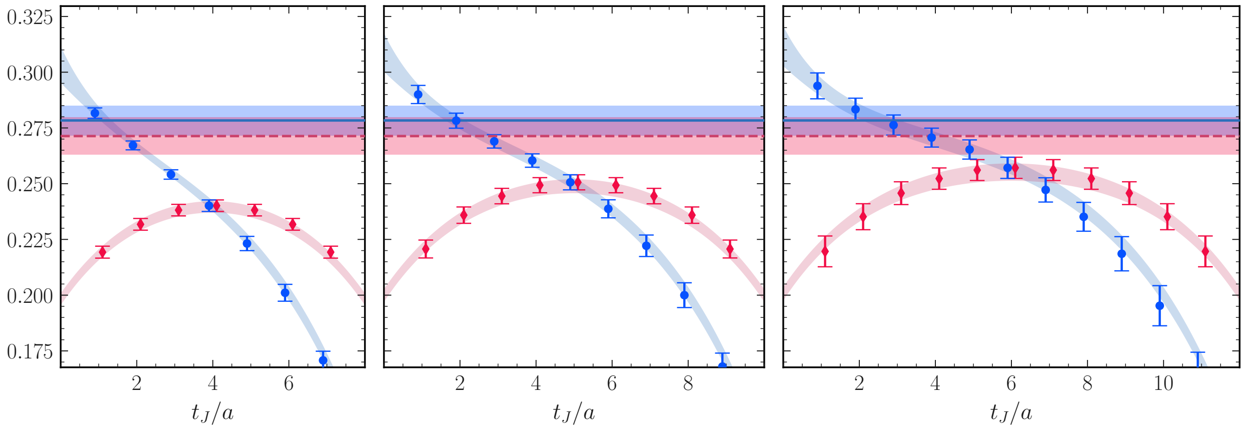


$J^\mu = J^\mu_A$, $\vec{P} = \frac{2\pi}{L}(0,0,1)$, $\Lambda = A_2$, $r = 1$, $n = 2$, $\vec{p}_B = \frac{2\pi}{L}(-1,0,0)$, $\mu = 3$, sign $= 1.0$

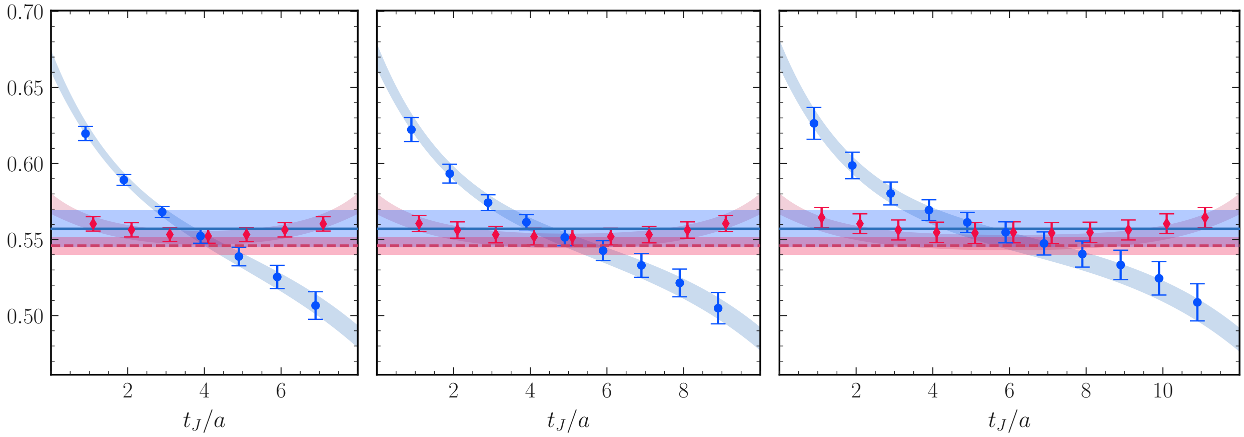

$J^\mu = J_A^\mu$, $\vec{P} = \frac{2\pi}{L}(0,0,1)$, $\Lambda = A_2$, $r = 1$, $n = 2$, $\vec{p}_B = \frac{2\pi}{L}(-1,0,1)$, $\mu = 0$, sign $= -1.0$

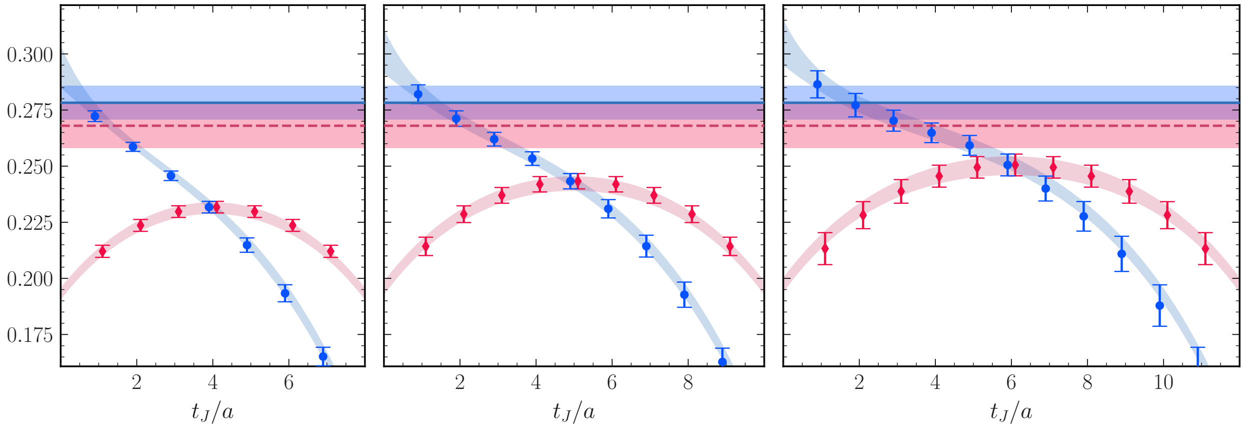


$J^\mu = J_A^\mu$, $\vec{P} = \frac{2\pi}{L}(0,0,1)$, $\Lambda = A_2$, $r = 1$, $n = 2$, $\vec{p}_B = \frac{2\pi}{L}(-1,0,1)$, $\mu = 3$, sign $= 1.0$

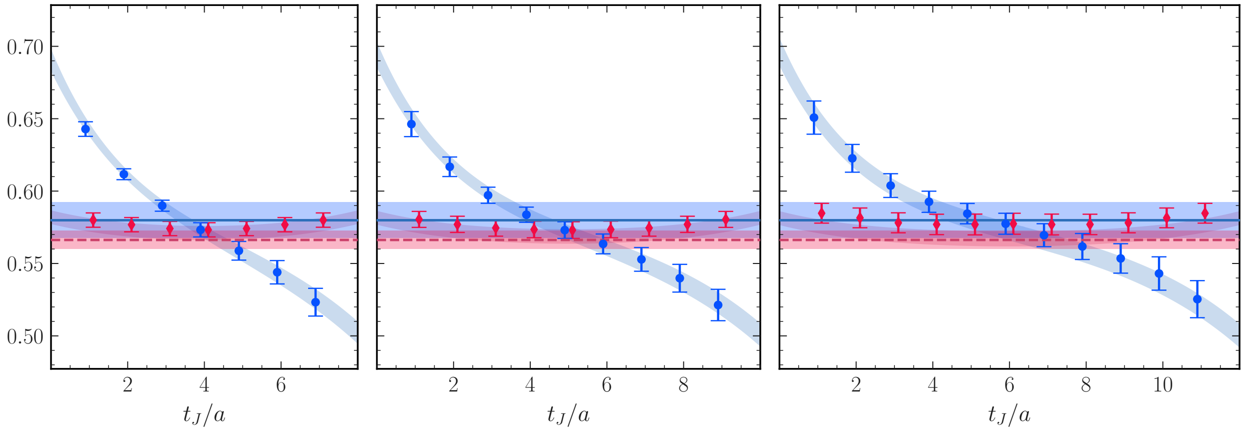


$J^\mu = J_A^\mu$, $\vec{P} = \frac{2\pi}{L}(0,0,1)$, $\Lambda = A_2$, $r = 1$, $n = 2$, $\vec{p}_B = \frac{2\pi}{L}(0,0,0)$, $\mu = 0$, sign $= -1.0$

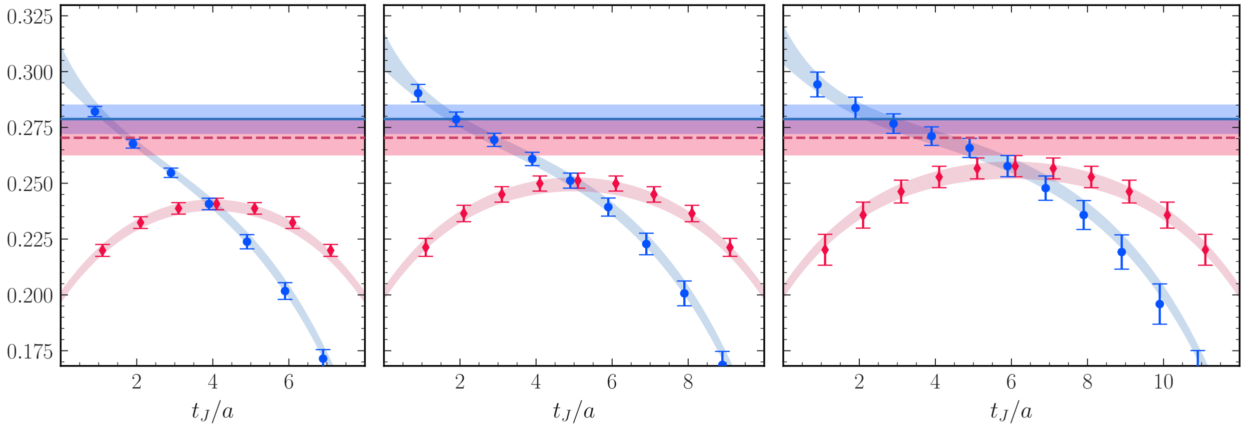

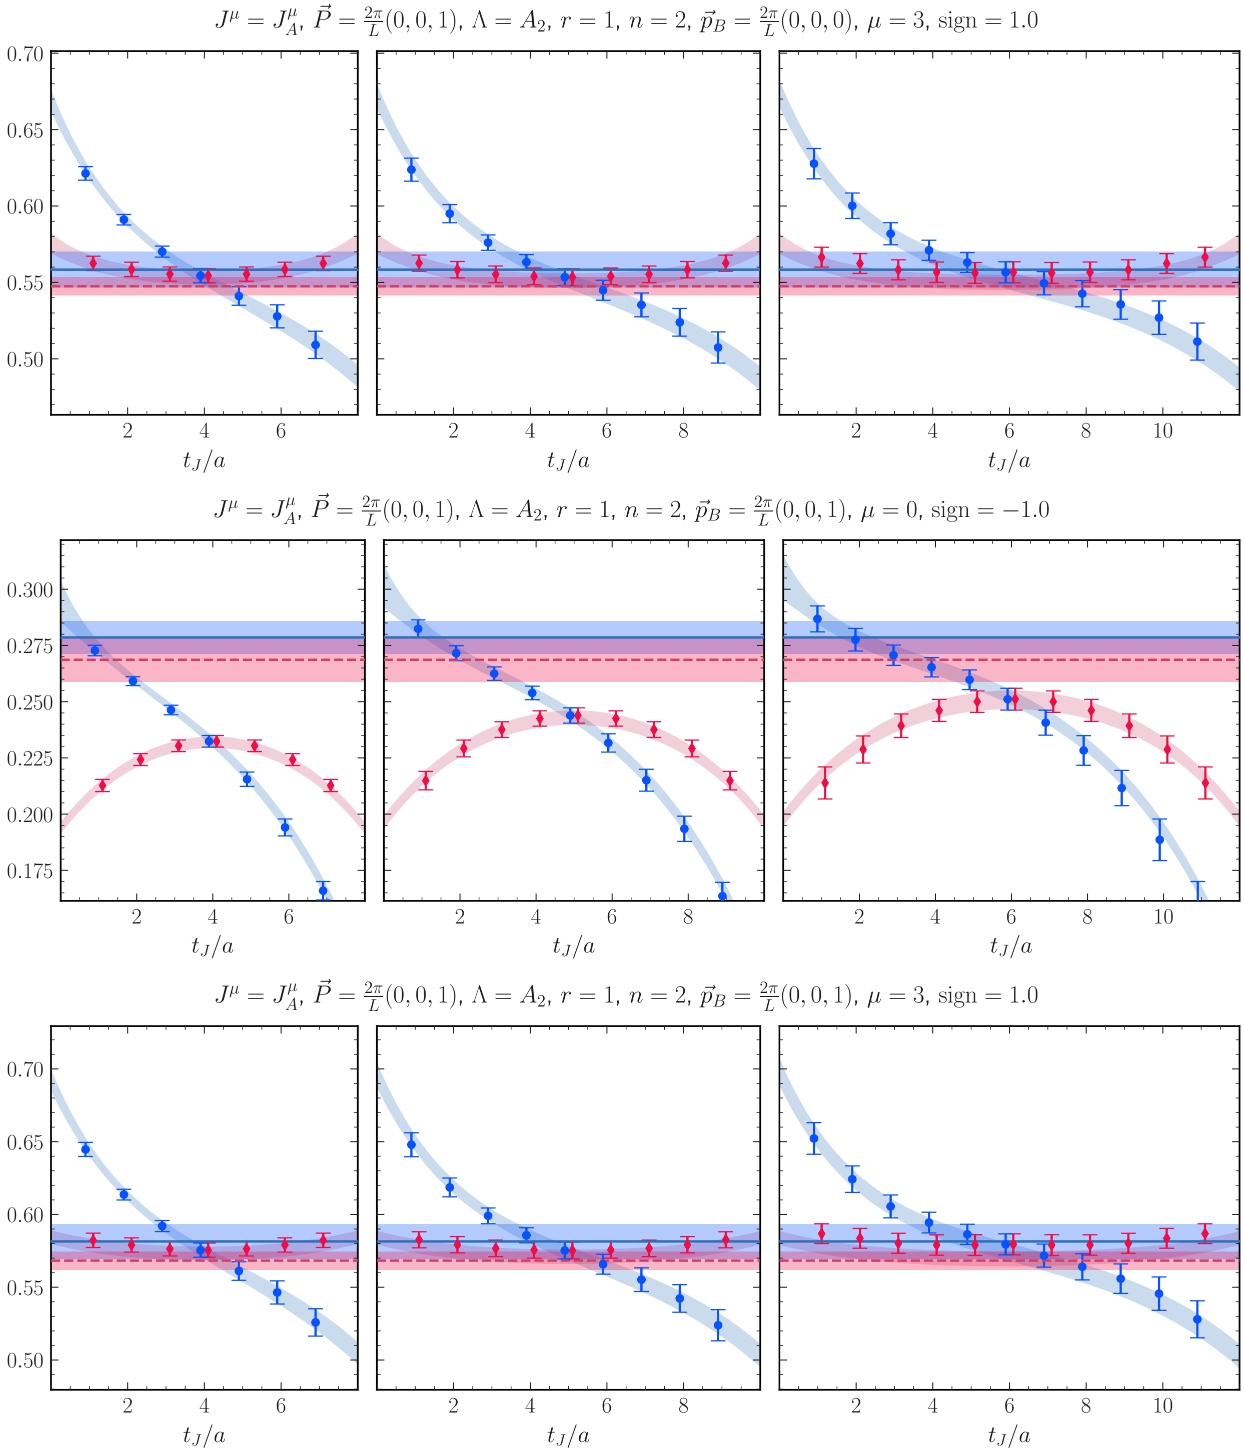

$J^\mu = J_A^\mu$, $\vec{P} = \frac{2\pi}{L}(0,0,1)$, $\Lambda = A_2$, $r = 1$, $n = 2$, $\vec{p}_B = \frac{2\pi}{L}(0,0,0)$, $\mu = 3$, sign $= 1.0$
$t_J/a$
$J^\mu = J_A^\mu$, $\vec{P} = \frac{2\pi}{L}(0,0,1)$, $\Lambda = A_2$, $r = 1$, $n = 2$, $\vec{p}_B = \frac{2\pi}{L}(0,0,1)$, $\mu = 0$, sign $= -1.0$
$t_J/a$
$J^\mu = J_A^\mu$, $\vec{P} = \frac{2\pi}{L}(0,0,1)$, $\Lambda = A_2$, $r = 1$, $n = 2$, $\vec{p}_B = \frac{2\pi}{L}(0,0,1)$, $\mu = 3$, sign $= 1.0$
$t_J/a$

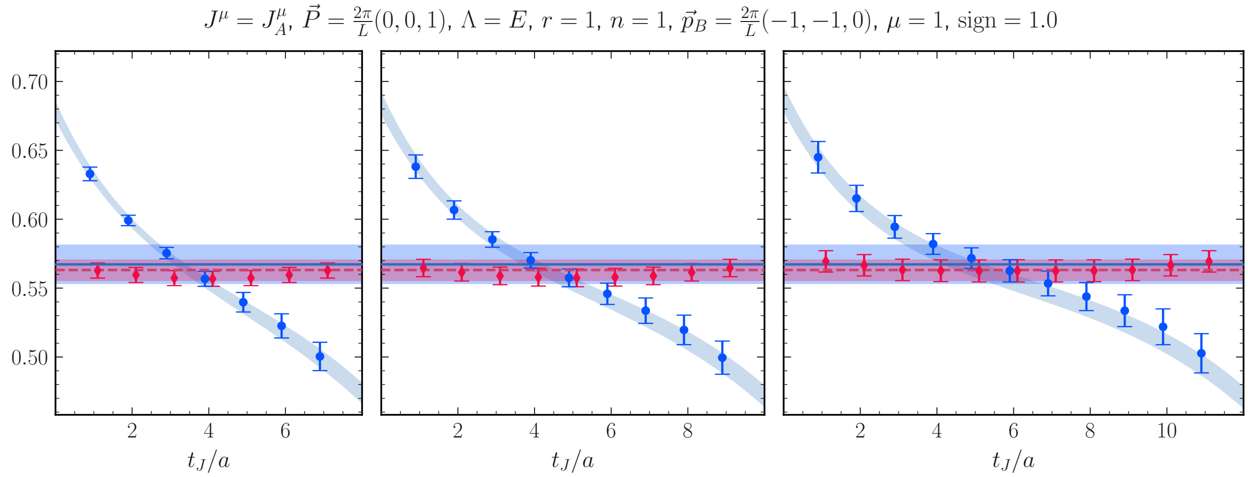
$J^\mu = J^\mu_A$, $\vec{P} = \frac{2\pi}{L}(0,0,1)$, $\Lambda = E$, $r = 1$, $n = 1$, $\vec{p}_B = \frac{2\pi}{L}(-1,-1,0)$, $\mu = 1$, sign = 1.0
0.70
0.65
0.60
0.55
0.50
2 4 6
2 4 6 8
2 4 6 8 10
$t_J/a$

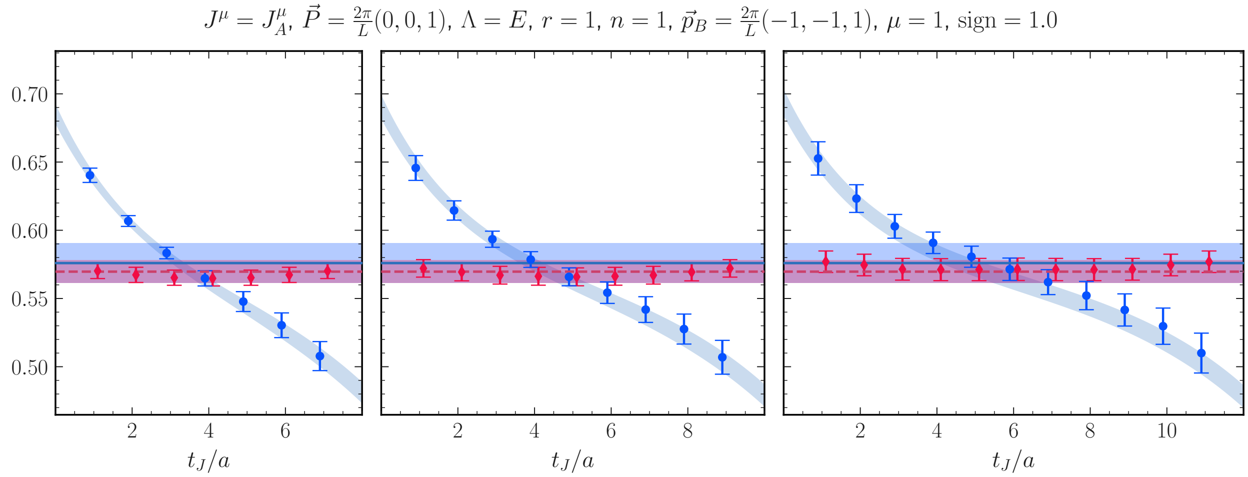
$J^\mu = J^\mu_A$, $\vec{P} = \frac{2\pi}{L}(0,0,1)$, $\Lambda = E$, $r = 1$, $n = 1$, $\vec{p}_B = \frac{2\pi}{L}(-1,-1,1)$, $\mu = 1$, sign = 1.0
0.70
0.65
0.60
0.55
0.50
2 4 6
2 4 6 8
2 4 6 8 10
$t_J/a$

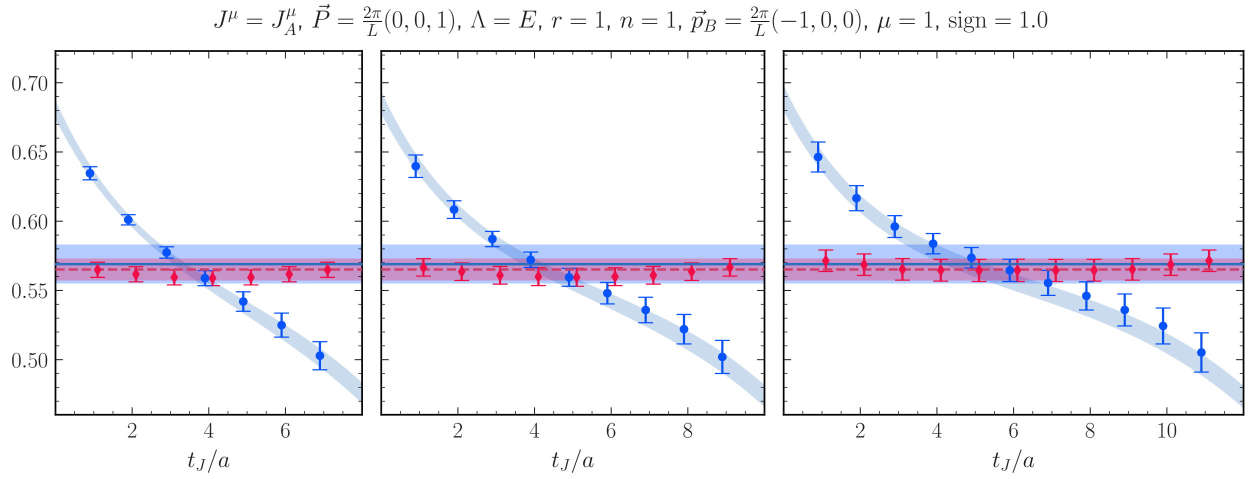
$J^\mu = J^\mu_A$, $\vec{P} = \frac{2\pi}{L}(0,0,1)$, $\Lambda = E$, $r = 1$, $n = 1$, $\vec{p}_B = \frac{2\pi}{L}(-1,0,0)$, $\mu = 1$, sign = 1.0
0.70
0.65
0.60
0.55
0.50
2 4 6
2 4 6 8
2 4 6 8 10
$t_J/a$

$J^\mu = J_A^\mu$, $\vec{P} = \frac{2\pi}{L}(0,0,1)$, $\Lambda = E$, $r = 1$, $n = 1$, $\vec{p}_B = \frac{2\pi}{L}(-1,0,1)$, $\mu = 1$, sign = 1.0

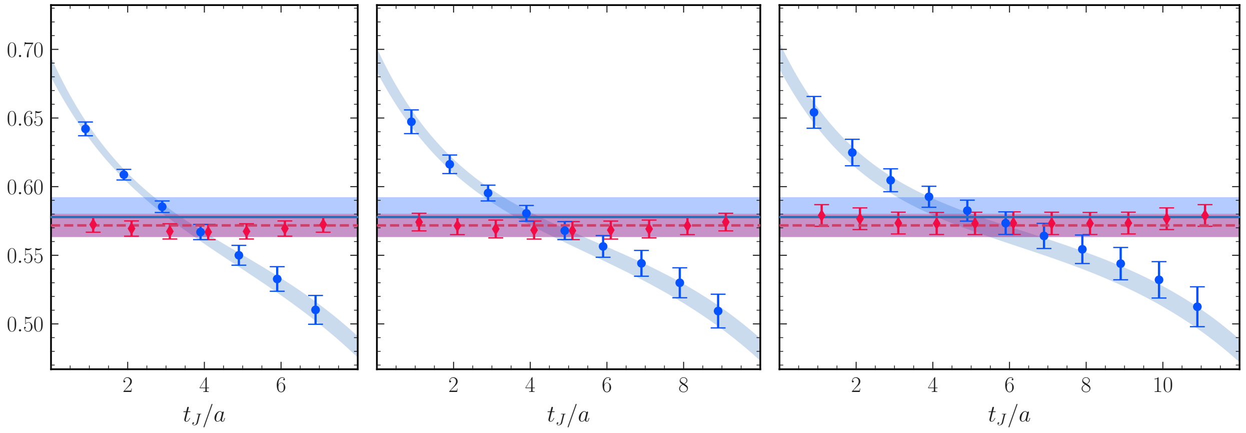


$J^\mu = J_A^\mu$, $\vec{P} = \frac{2\pi}{L}(0,0,1)$, $\Lambda = E$, $r = 1$, $n = 1$, $\vec{p}_B = \frac{2\pi}{L}(0,0,0)$, $\mu = 1$, sign = 1.0

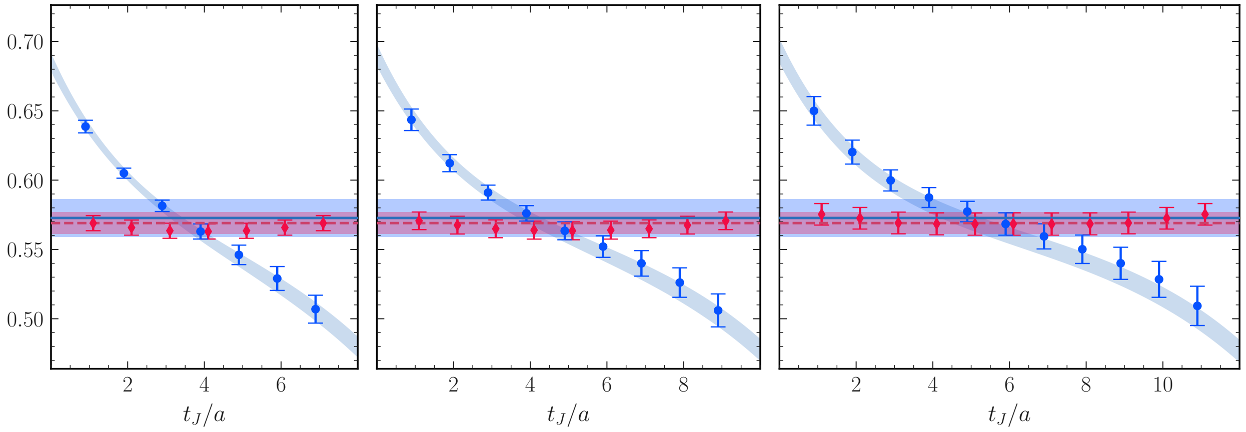


$J^\mu = J_A^\mu$, $\vec{P} = \frac{2\pi}{L}(0,0,1)$, $\Lambda = E$, $r = 1$, $n = 1$, $\vec{p}_B = \frac{2\pi}{L}(0,0,1)$, $\mu = 1$, sign = 1.0

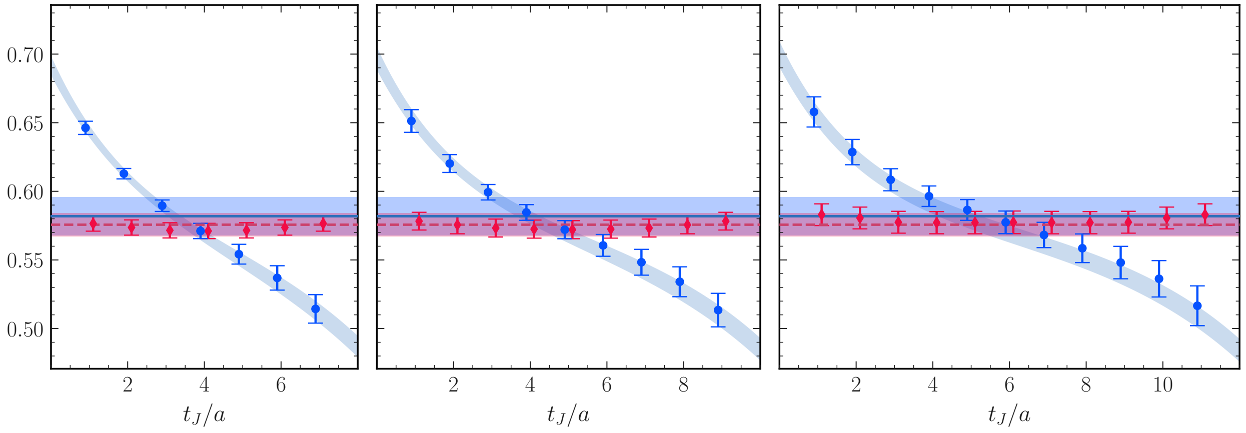

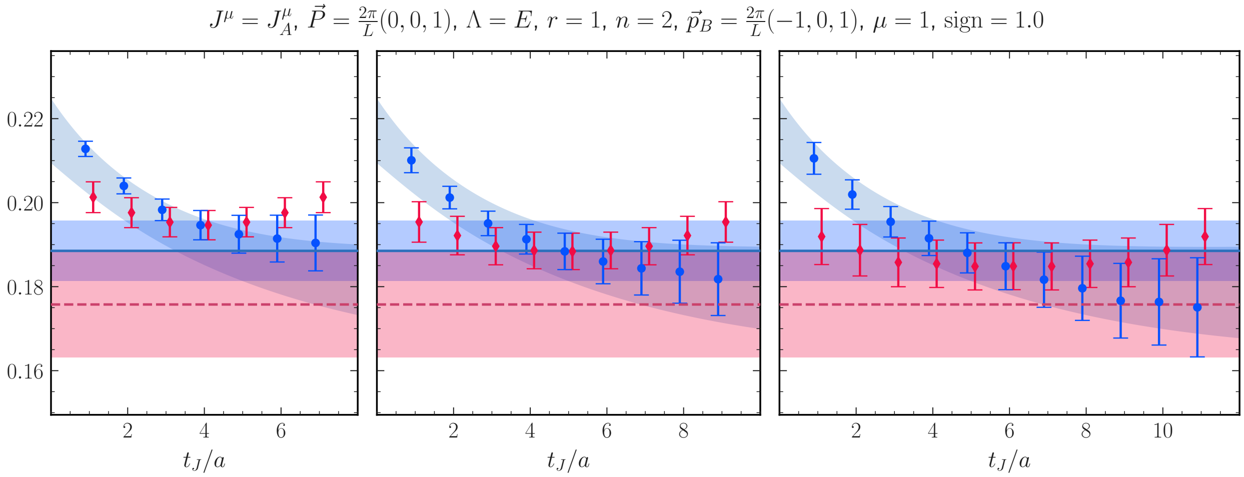
$J^\mu = J^\mu_A$, $\vec{P} = \frac{2\pi}{L}(0,0,1)$, $\Lambda = E$, $r = 1$, $n = 2$, $\vec{p}_B = \frac{2\pi}{L}(-1,0,1)$, $\mu = 1$, sign = 1.0
0.22
0.20
0.18
0.16
$t_J/a$
$t_J/a$
$t_J/a$

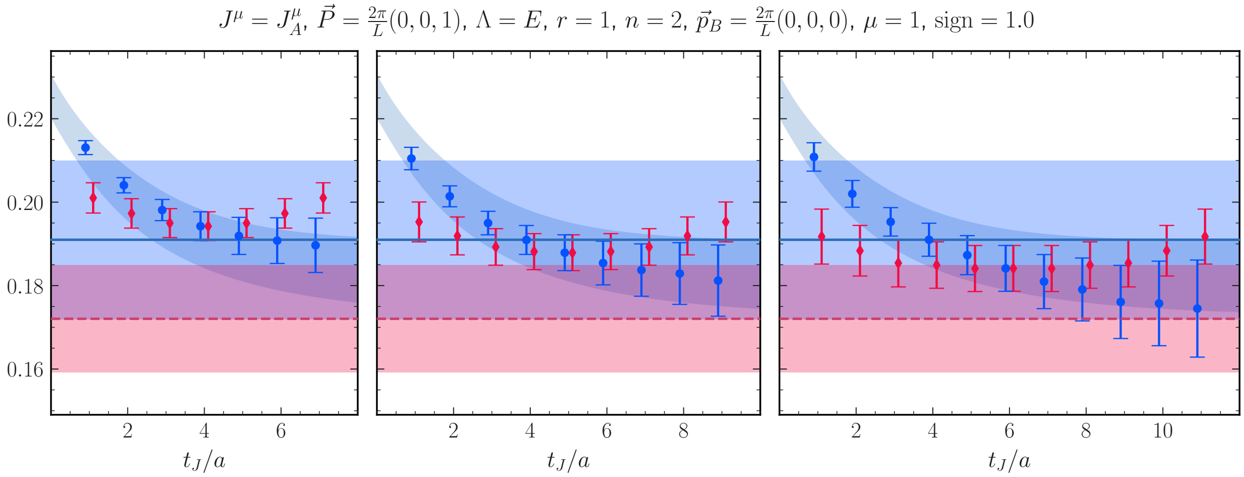
$J^\mu = J^\mu_A$, $\vec{P} = \frac{2\pi}{L}(0,0,1)$, $\Lambda = E$, $r = 1$, $n = 2$, $\vec{p}_B = \frac{2\pi}{L}(0,0,0)$, $\mu = 1$, sign = 1.0
0.22
0.20
0.18
0.16
$t_J/a$
$t_J/a$
$t_J/a$

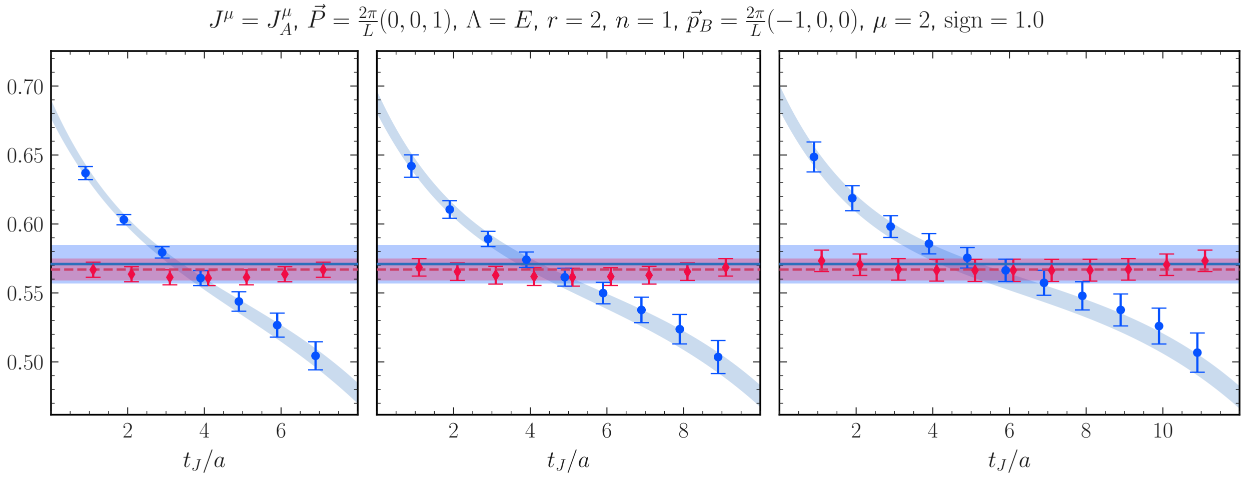
$J^\mu = J^\mu_A$, $\vec{P} = \frac{2\pi}{L}(0,0,1)$, $\Lambda = E$, $r = 2$, $n = 1$, $\vec{p}_B = \frac{2\pi}{L}(-1,0,0)$, $\mu = 2$, sign = 1.0
0.70
0.65
0.60
0.55
0.50
$t_J/a$
$t_J/a$
$t_J/a$

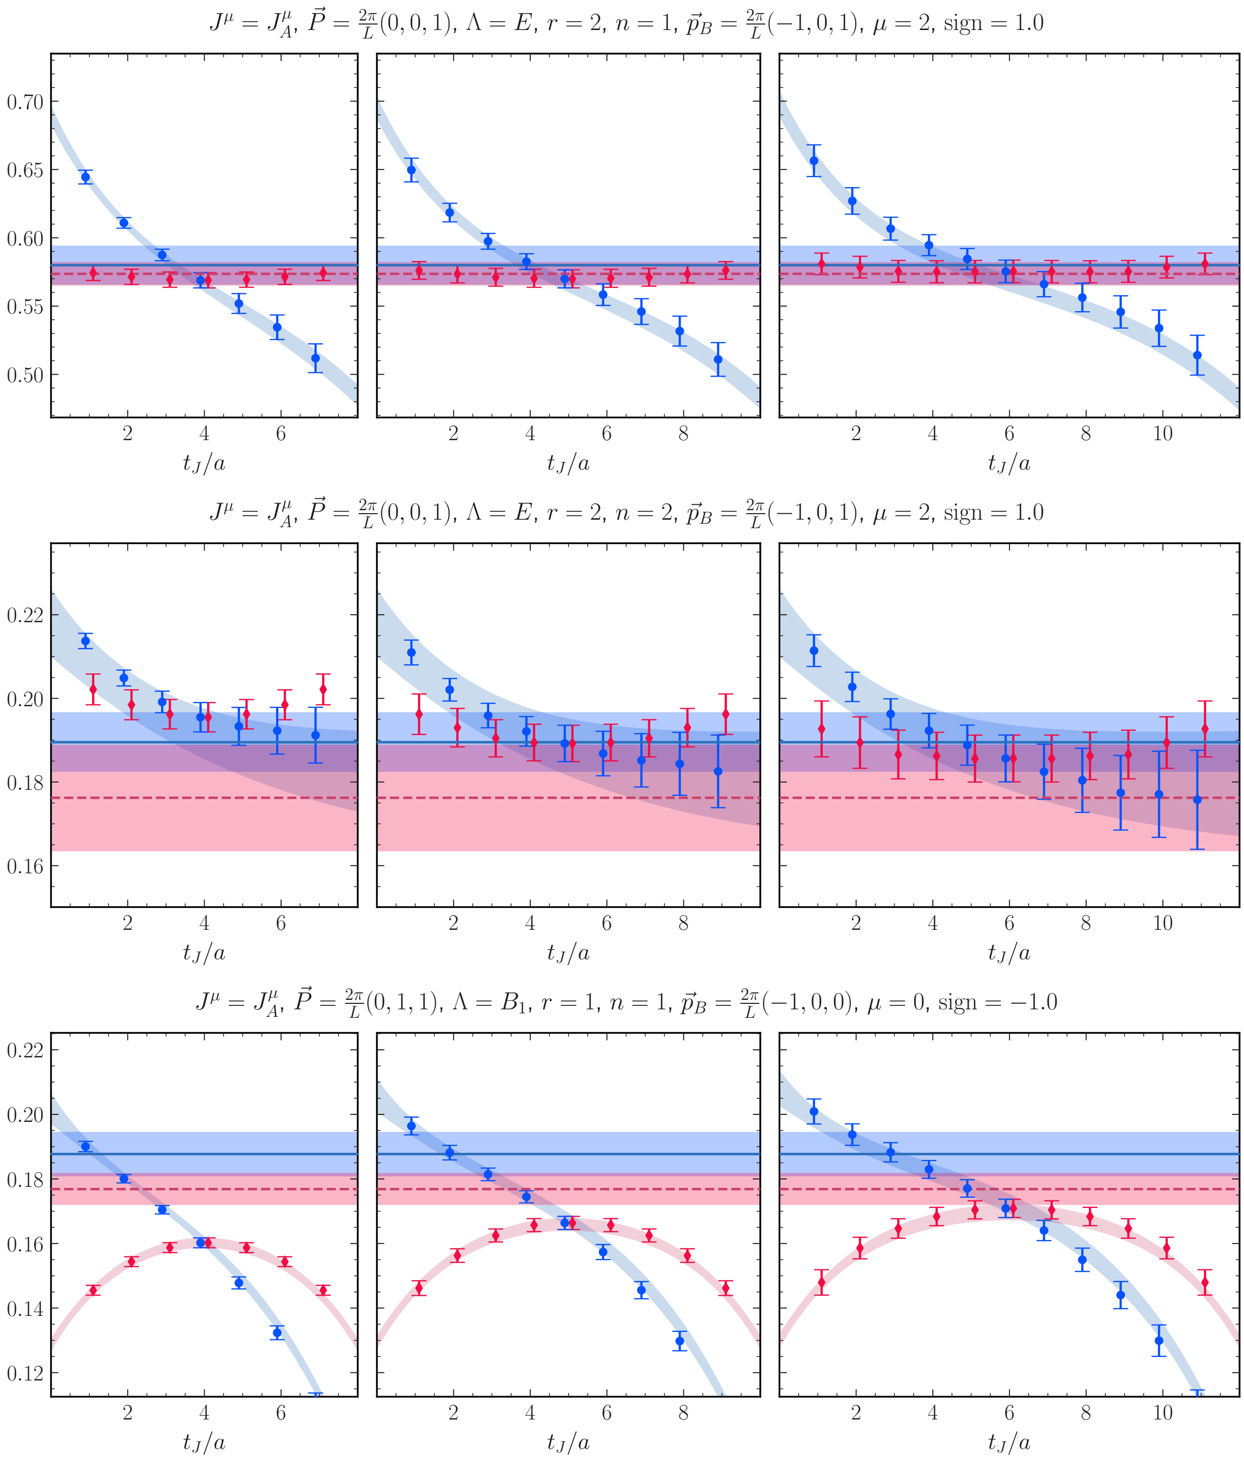

$J^\mu = J^\mu_A$, $\vec{P} = \frac{2\pi}{L}(0,0,1)$, $\Lambda = E$, $r = 2$, $n = 1$, $\vec{p}_B = \frac{2\pi}{L}(-1,0,1)$, $\mu = 2$, sign = 1.0
$J^\mu = J^\mu_A$, $\vec{P} = \frac{2\pi}{L}(0,0,1)$, $\Lambda = E$, $r = 2$, $n = 2$, $\vec{p}_B = \frac{2\pi}{L}(-1,0,1)$, $\mu = 2$, sign = 1.0
$J^\mu = J^\mu_A$, $\vec{P} = \frac{2\pi}{L}(0,1,1)$, $\Lambda = B_1$, $r = 1$, $n = 1$, $\vec{p}_B = \frac{2\pi}{L}(-1,0,0)$, $\mu = 0$, sign = −1.0
$t_J/a$

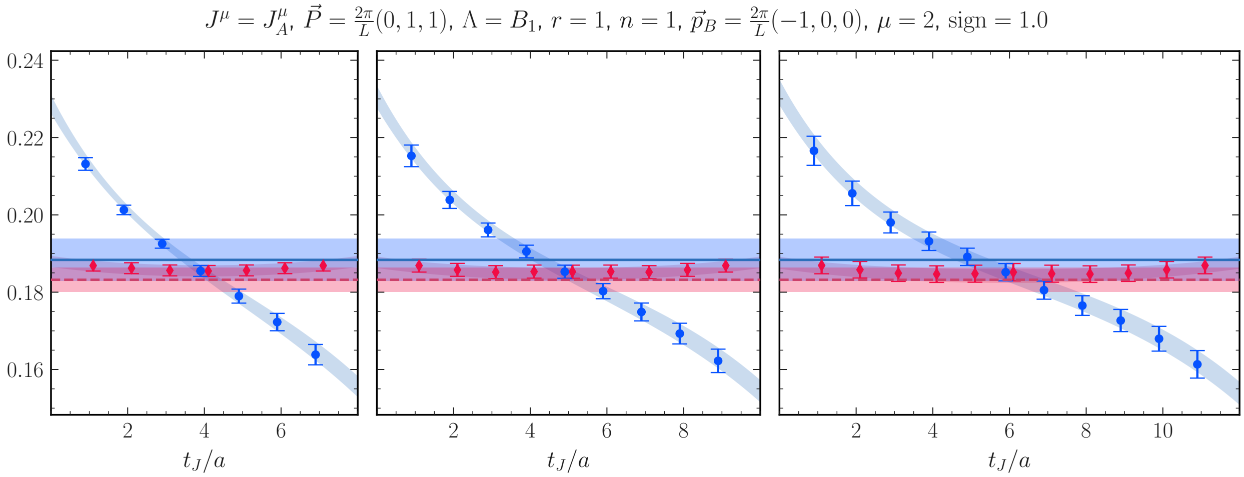
$J^\mu = J_A^\mu$, $\vec{P} = \frac{2\pi}{L}(0,1,1)$, $\Lambda = B_1$, $r = 1$, $n = 1$, $\vec{p}_B = \frac{2\pi}{L}(-1,0,0)$, $\mu = 2$, sign = 1.0
0.24
0.22
0.20
0.18
0.16
$t_J/a$
$t_J/a$
$t_J/a$

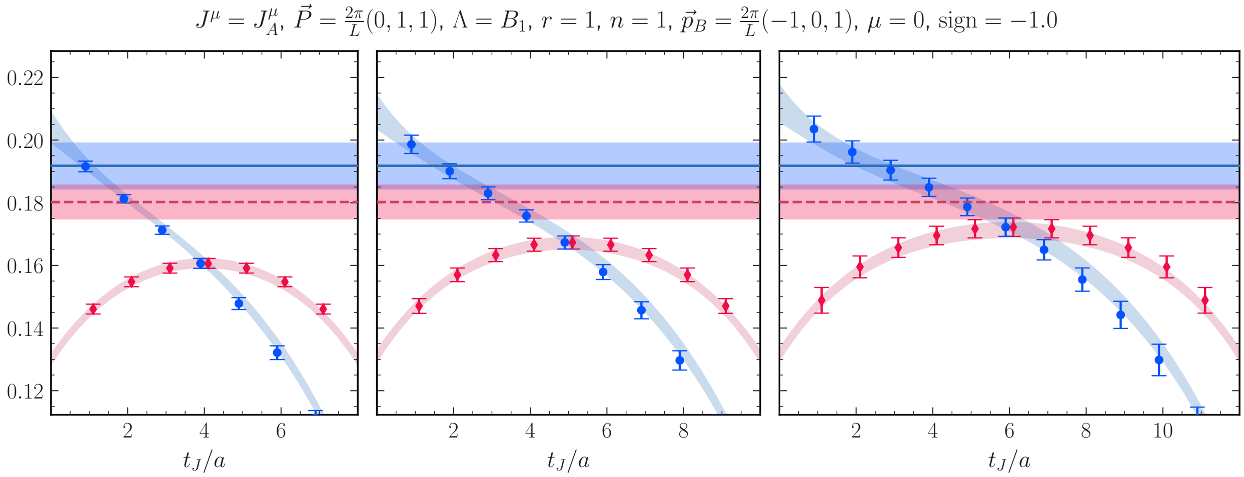
$J^\mu = J_A^\mu$, $\vec{P} = \frac{2\pi}{L}(0,1,1)$, $\Lambda = B_1$, $r = 1$, $n = 1$, $\vec{p}_B = \frac{2\pi}{L}(-1,0,1)$, $\mu = 0$, sign = −1.0
0.22
0.20
0.18
0.16
0.14
0.12
$t_J/a$
$t_J/a$
$t_J/a$

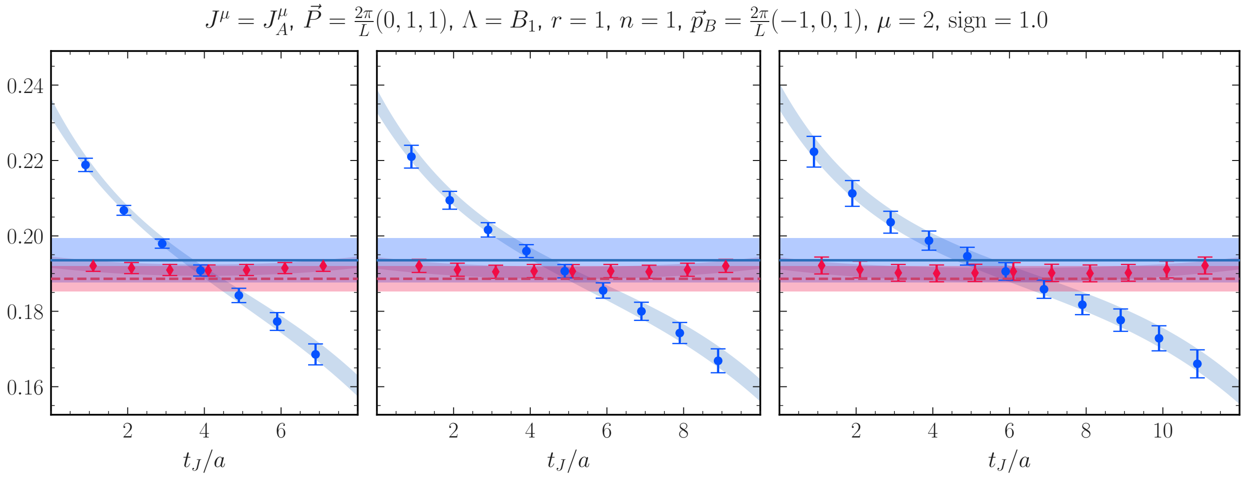
$J^\mu = J_A^\mu$, $\vec{P} = \frac{2\pi}{L}(0,1,1)$, $\Lambda = B_1$, $r = 1$, $n = 1$, $\vec{p}_B = \frac{2\pi}{L}(-1,0,1)$, $\mu = 2$, sign = 1.0
0.24
0.22
0.20
0.18
0.16
$t_J/a$
$t_J/a$
$t_J/a$

$J^\mu = J^\mu_A$, $\vec{P} = \frac{2\pi}{L}(0,1,1)$, $\Lambda = B_1$, $r = 1$, $n = 1$, $\vec{p}_B = \frac{2\pi}{L}(-1,0,1)$, $\mu = 3$, sign $= 1.0$

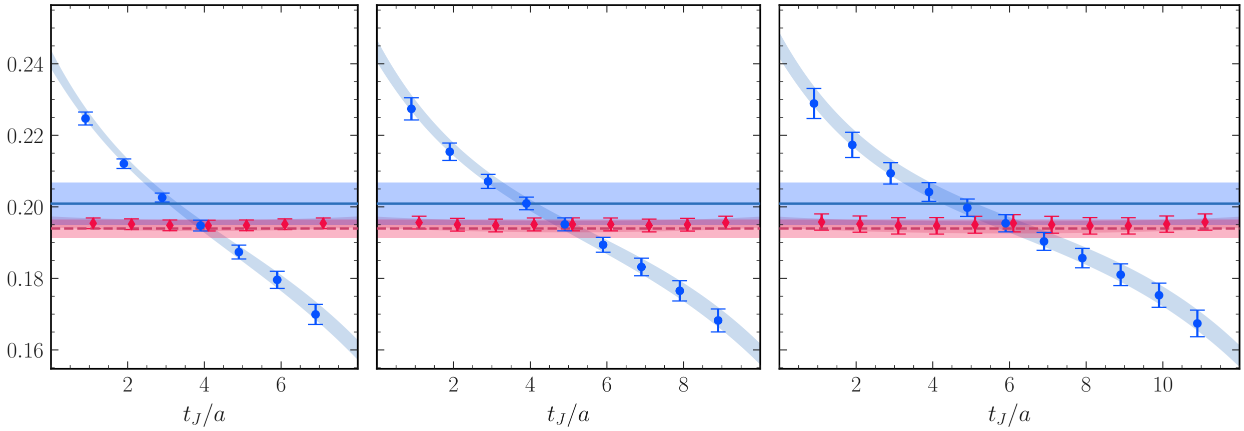


$J^\mu = J^\mu_A$, $\vec{P} = \frac{2\pi}{L}(0,1,1)$, $\Lambda = B_1$, $r = 1$, $n = 1$, $\vec{p}_B = \frac{2\pi}{L}(-1,1,1)$, $\mu = 0$, sign $= -1.0$

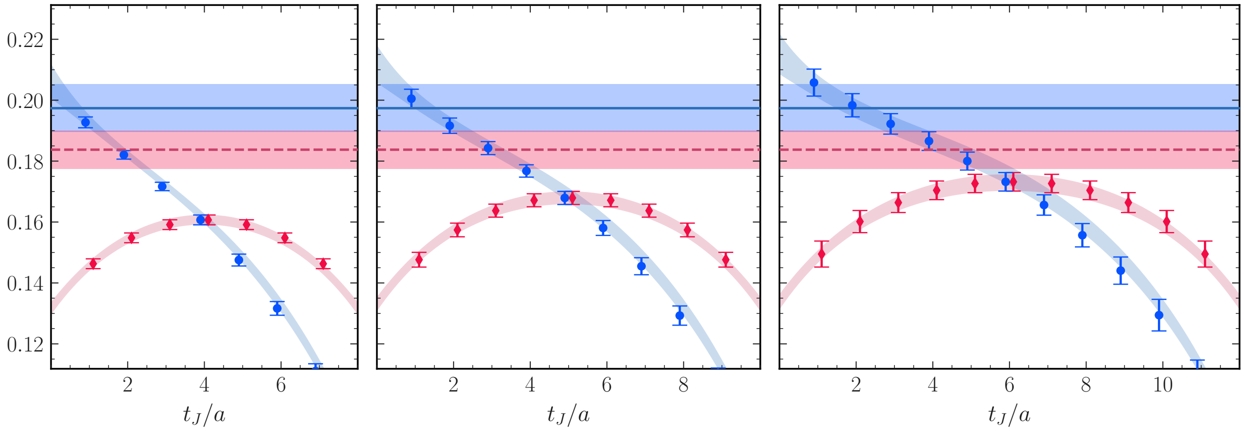


$J^\mu = J^\mu_A$, $\vec{P} = \frac{2\pi}{L}(0,1,1)$, $\Lambda = B_1$, $r = 1$, $n = 1$, $\vec{p}_B = \frac{2\pi}{L}(-1,1,1)$, $\mu = 2$, sign $= 1.0$

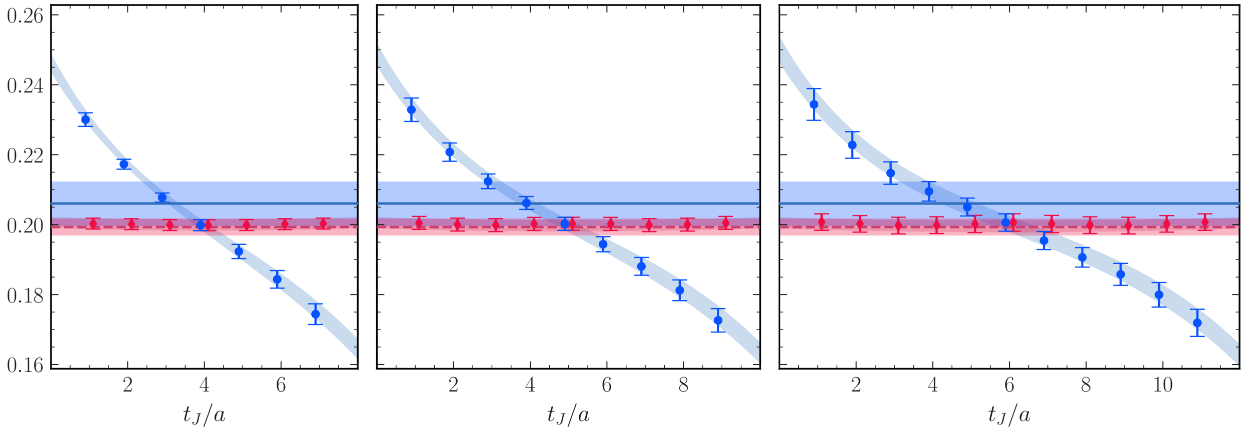

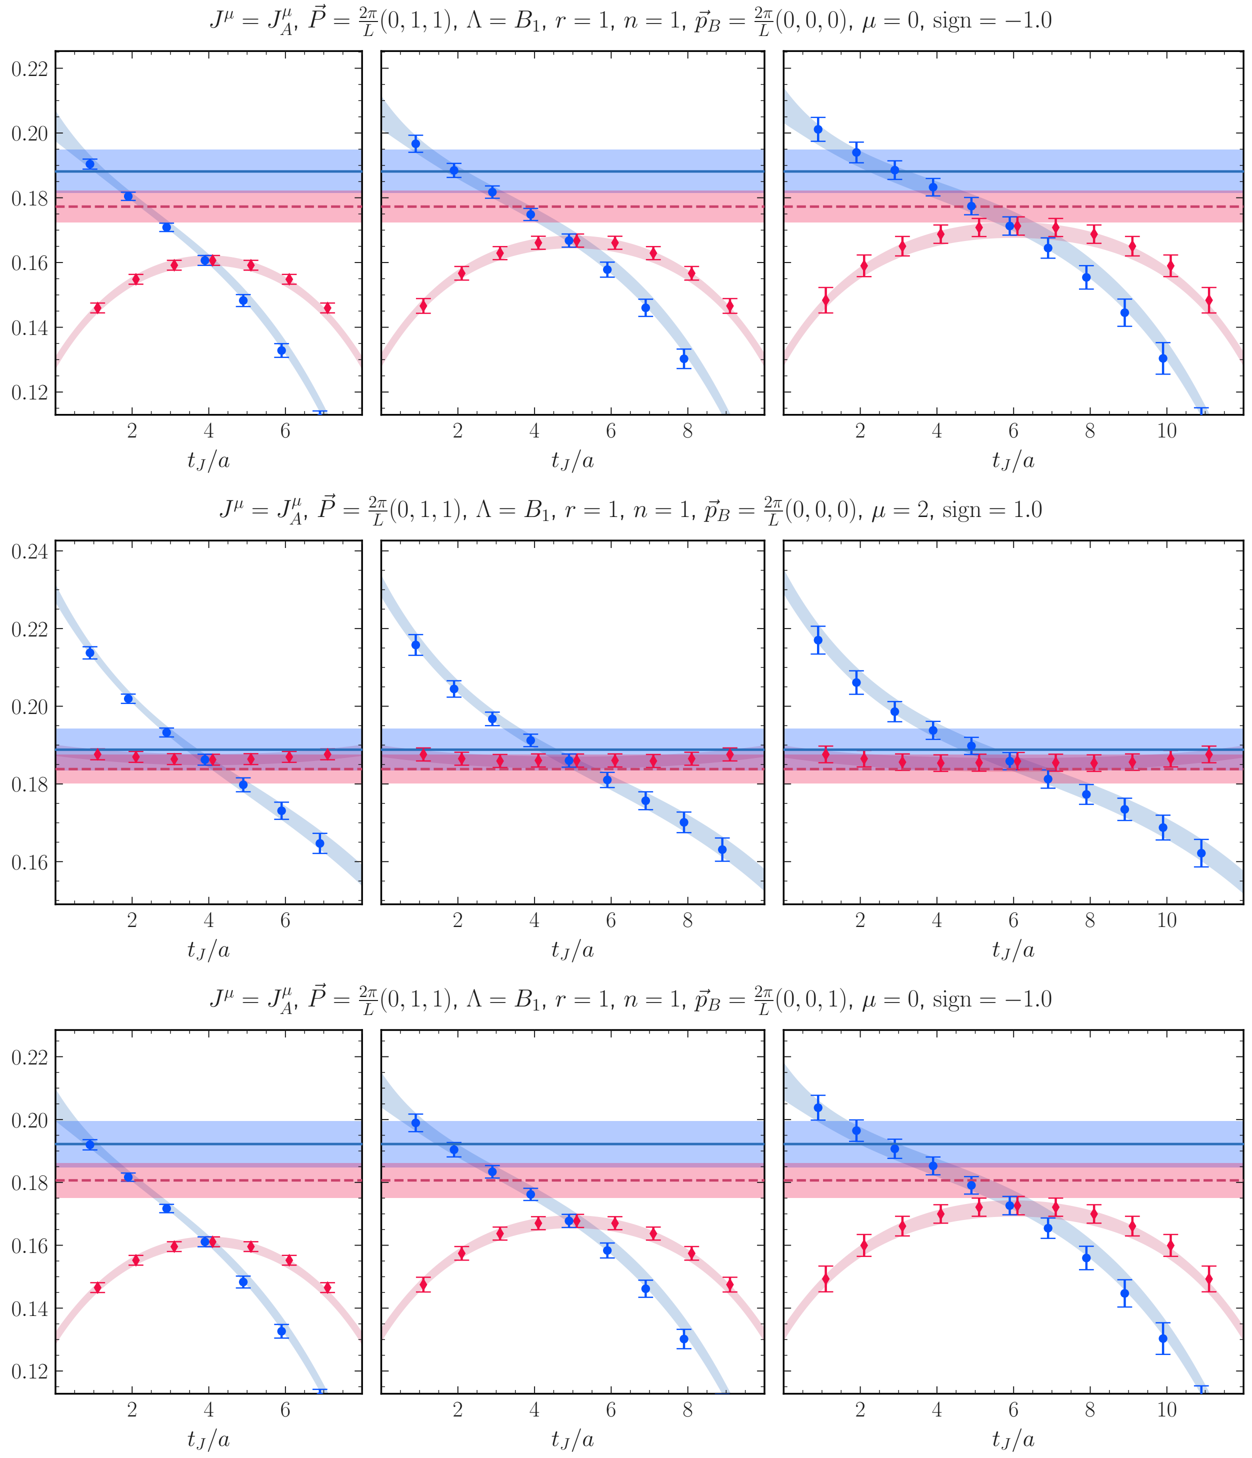
$J^\mu = J^\mu_A$, $\vec{P} = \frac{2\pi}{L}(0,1,1)$, $\Lambda = B_1$, $r = 1$, $n = 1$, $\vec{p}_B = \frac{2\pi}{L}(0,0,0)$, $\mu = 0$, sign $= -1.0$
0.22
0.20
0.18
0.16
0.14
0.12
2
4
6
8
10
$t_J/a$
$J^\mu = J^\mu_A$, $\vec{P} = \frac{2\pi}{L}(0,1,1)$, $\Lambda = B_1$, $r = 1$, $n = 1$, $\vec{p}_B = \frac{2\pi}{L}(0,0,0)$, $\mu = 2$, sign $= 1.0$
0.24
0.22
0.20
0.18
0.16
$t_J/a$
$J^\mu = J^\mu_A$, $\vec{P} = \frac{2\pi}{L}(0,1,1)$, $\Lambda = B_1$, $r = 1$, $n = 1$, $\vec{p}_B = \frac{2\pi}{L}(0,0,1)$, $\mu = 0$, sign $= -1.0$
$t_J/a$

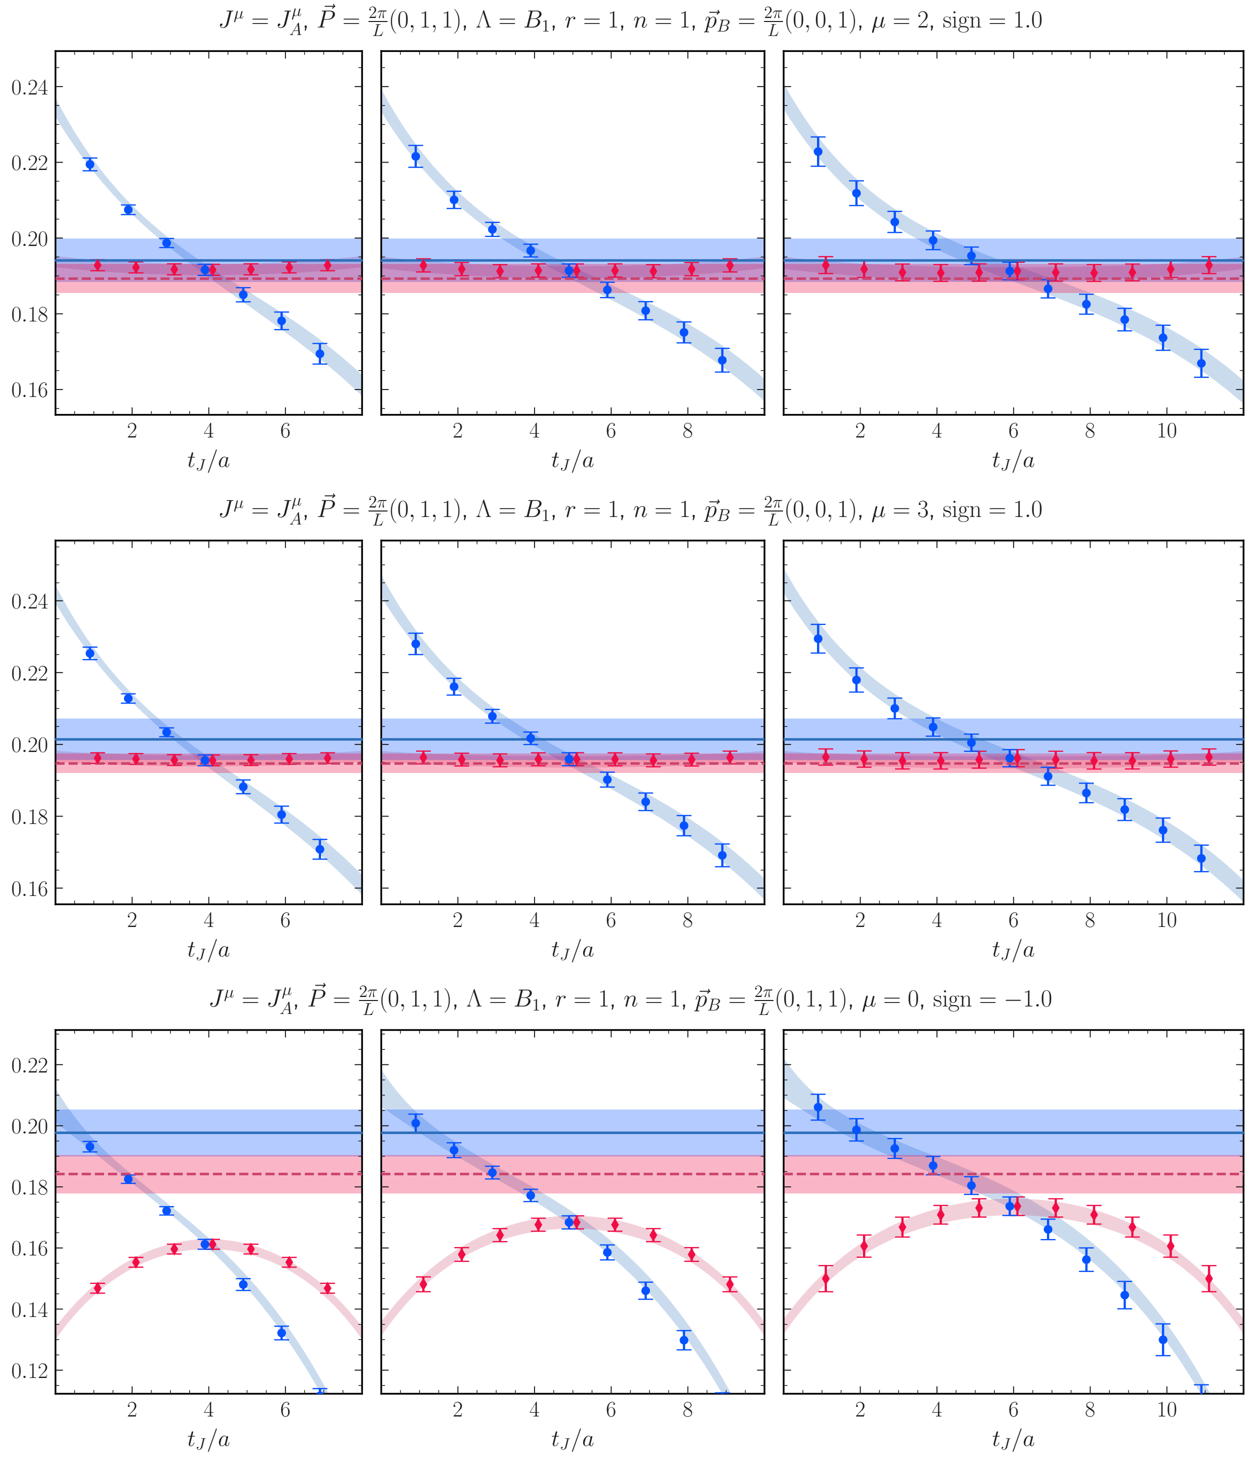

$J^\mu = J_A^\mu$, $\vec{P} = \frac{2\pi}{L}(0,1,1)$, $\Lambda = B_1$, $r = 1$, $n = 1$, $\vec{p}_B = \frac{2\pi}{L}(0,0,1)$, $\mu = 2$, sign $= 1.0$
$t_J/a$
$J^\mu = J_A^\mu$, $\vec{P} = \frac{2\pi}{L}(0,1,1)$, $\Lambda = B_1$, $r = 1$, $n = 1$, $\vec{p}_B = \frac{2\pi}{L}(0,0,1)$, $\mu = 3$, sign $= 1.0$
$t_J/a$
$J^\mu = J_A^\mu$, $\vec{P} = \frac{2\pi}{L}(0,1,1)$, $\Lambda = B_1$, $r = 1$, $n = 1$, $\vec{p}_B = \frac{2\pi}{L}(0,1,1)$, $\mu = 0$, sign $= -1.0$
$t_J/a$

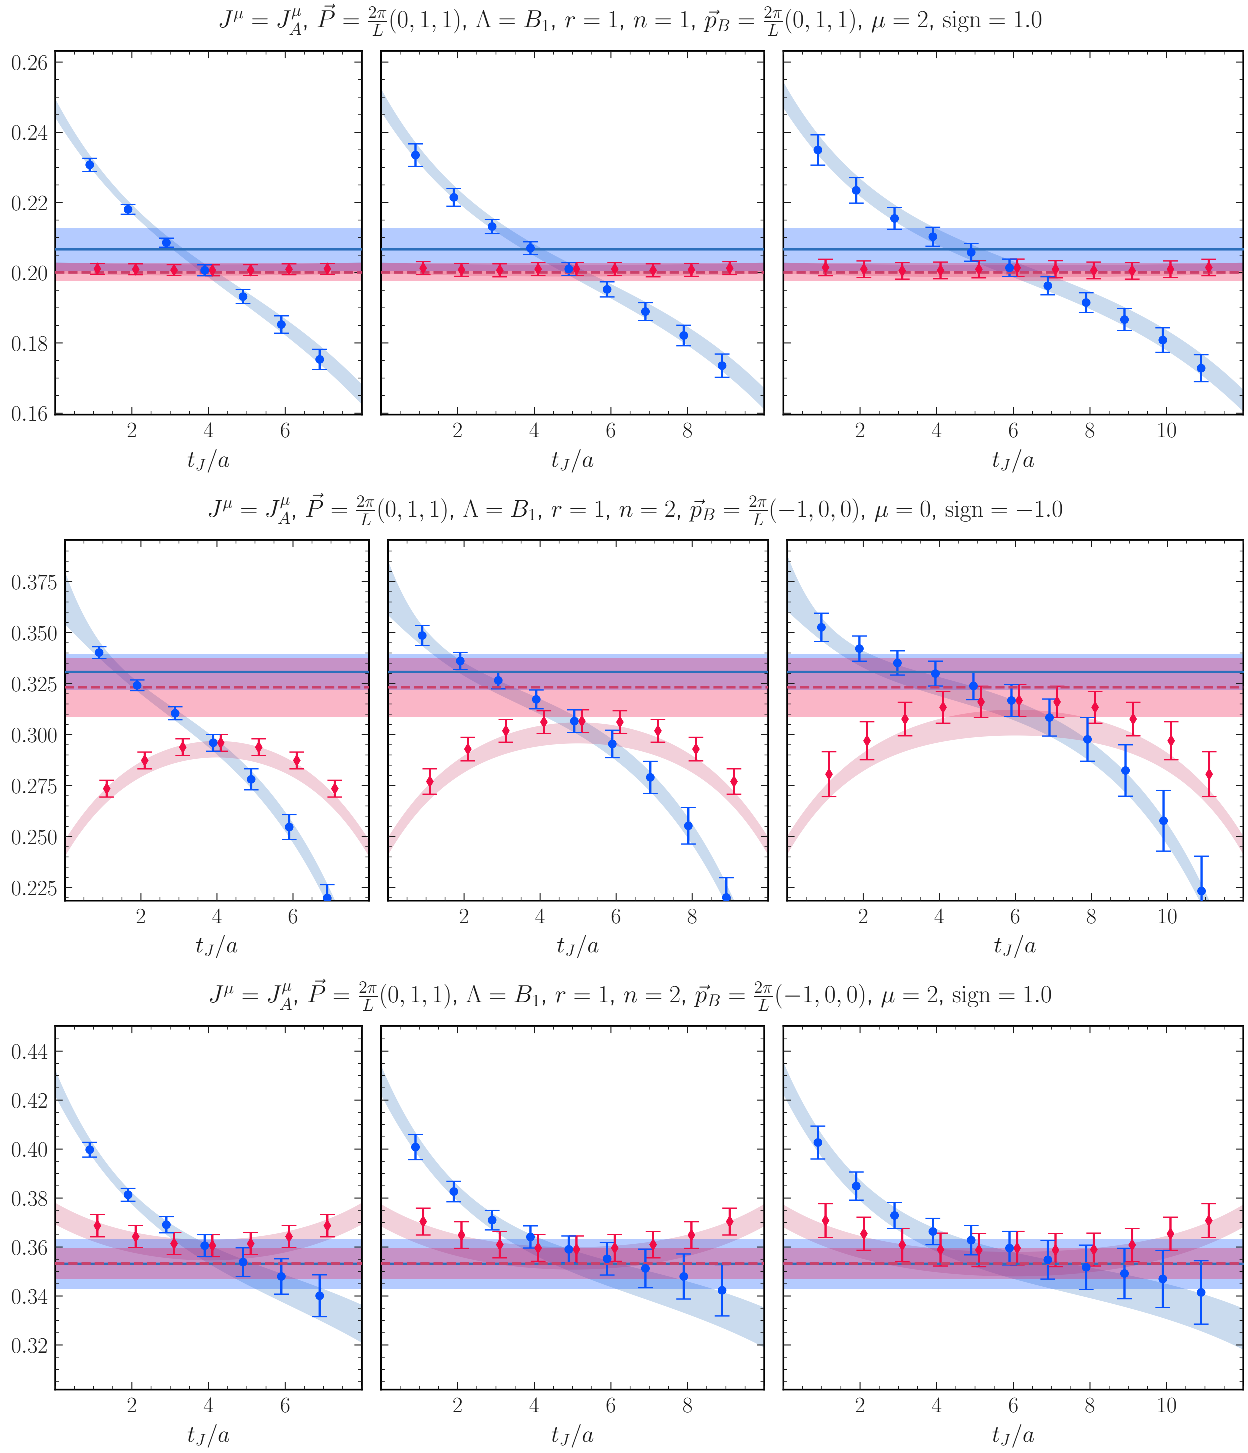

$J^\mu = J_A^\mu$, $\vec{P} = \frac{2\pi}{L}(0,1,1)$, $\Lambda = B_1$, $r = 1$, $n = 1$, $\vec{p}_B = \frac{2\pi}{L}(0,1,1)$, $\mu = 2$, sign = 1.0
0.26
0.24
0.22
0.20
0.18
0.16
2 4 6
2 4 6 8
2 4 6 8 10
$t_J/a$
$J^\mu = J_A^\mu$, $\vec{P} = \frac{2\pi}{L}(0,1,1)$, $\Lambda = B_1$, $r = 1$, $n = 2$, $\vec{p}_B = \frac{2\pi}{L}(-1,0,0)$, $\mu = 0$, sign = −1.0
0.375
0.350
0.325
0.300
0.275
0.250
0.225
$t_J/a$
$J^\mu = J_A^\mu$, $\vec{P} = \frac{2\pi}{L}(0,1,1)$, $\Lambda = B_1$, $r = 1$, $n = 2$, $\vec{p}_B = \frac{2\pi}{L}(-1,0,0)$, $\mu = 2$, sign = 1.0
0.44
0.42
0.40
0.38
0.36
0.34
0.32
$t_J/a$

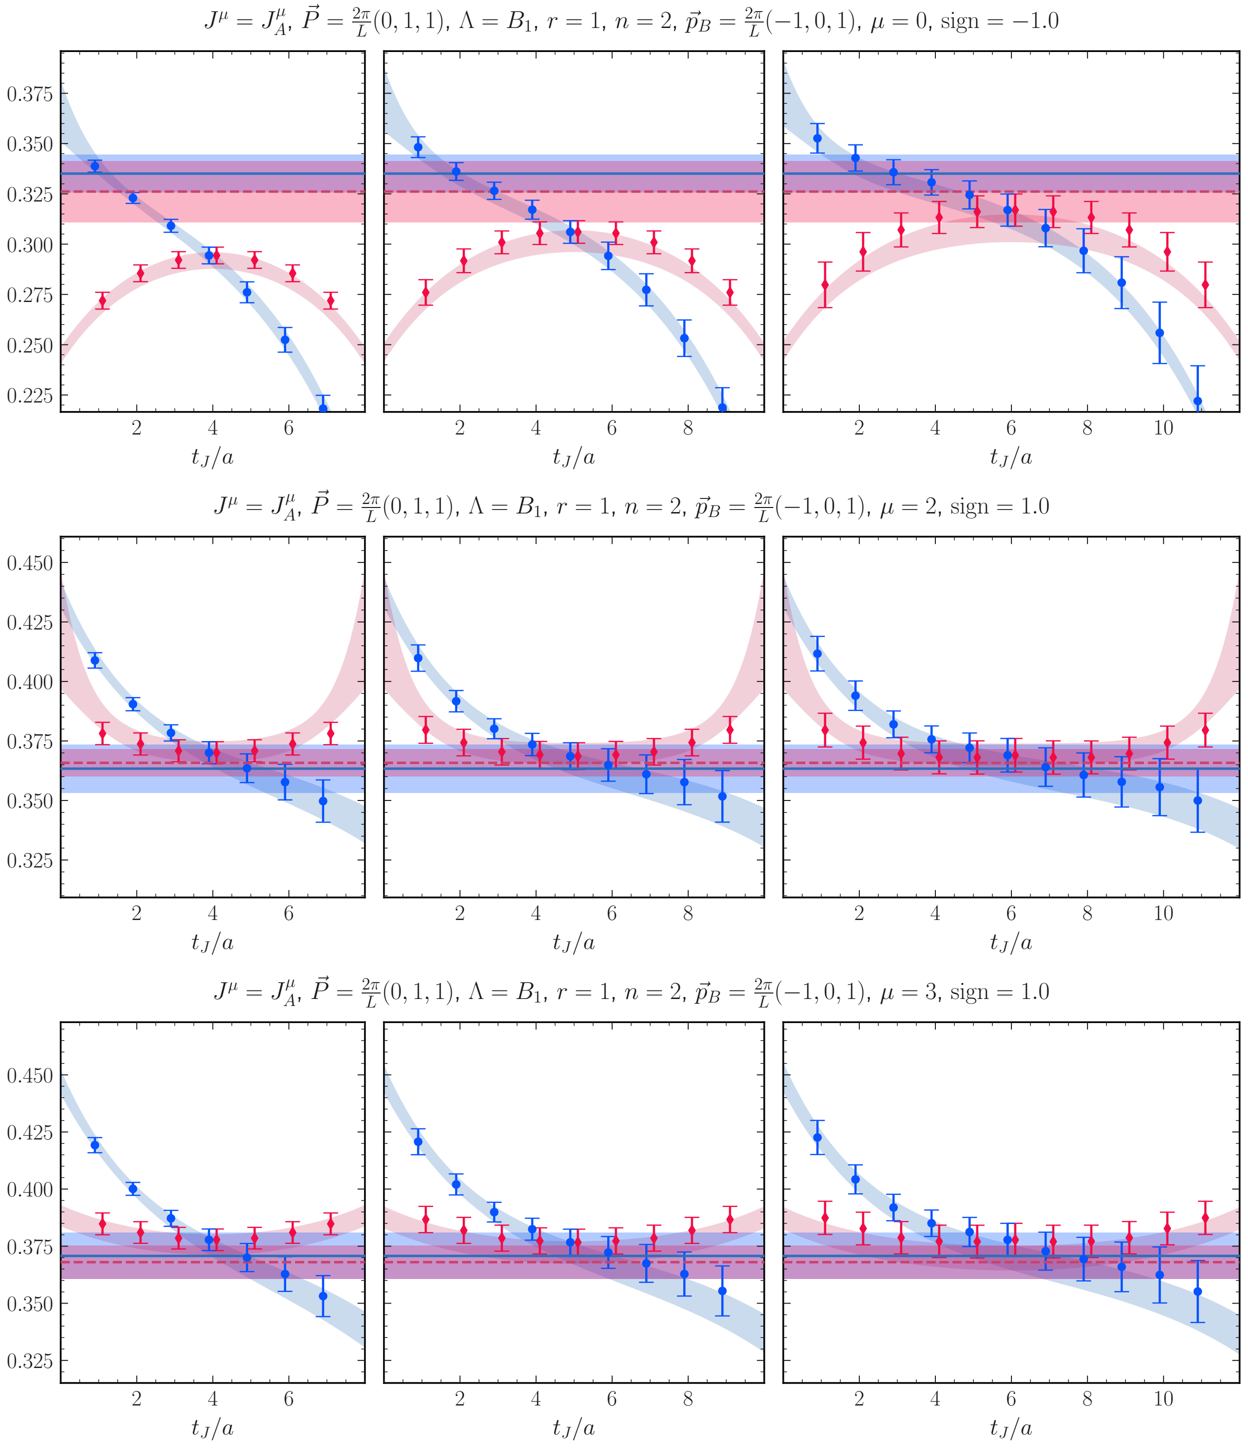

$J^\mu = J_A^\mu$, $\vec{P} = \frac{2\pi}{L}(0,1,1)$, $\Lambda = B_1$, $r = 1$, $n = 2$, $\vec{p}_B = \frac{2\pi}{L}(-1,0,1)$, $\mu = 0$, sign $= -1.0$
0.375
0.350
0.325
0.300
0.275
0.250
0.225
$t_J/a$
$J^\mu = J_A^\mu$, $\vec{P} = \frac{2\pi}{L}(0,1,1)$, $\Lambda = B_1$, $r = 1$, $n = 2$, $\vec{p}_B = \frac{2\pi}{L}(-1,0,1)$, $\mu = 2$, sign $= 1.0$
0.450
0.425
0.400
0.375
0.350
0.325
$t_J/a$
$J^\mu = J_A^\mu$, $\vec{P} = \frac{2\pi}{L}(0,1,1)$, $\Lambda = B_1$, $r = 1$, $n = 2$, $\vec{p}_B = \frac{2\pi}{L}(-1,0,1)$, $\mu = 3$, sign $= 1.0$
0.450
0.425
0.400
0.375
0.350
0.325
$t_J/a$

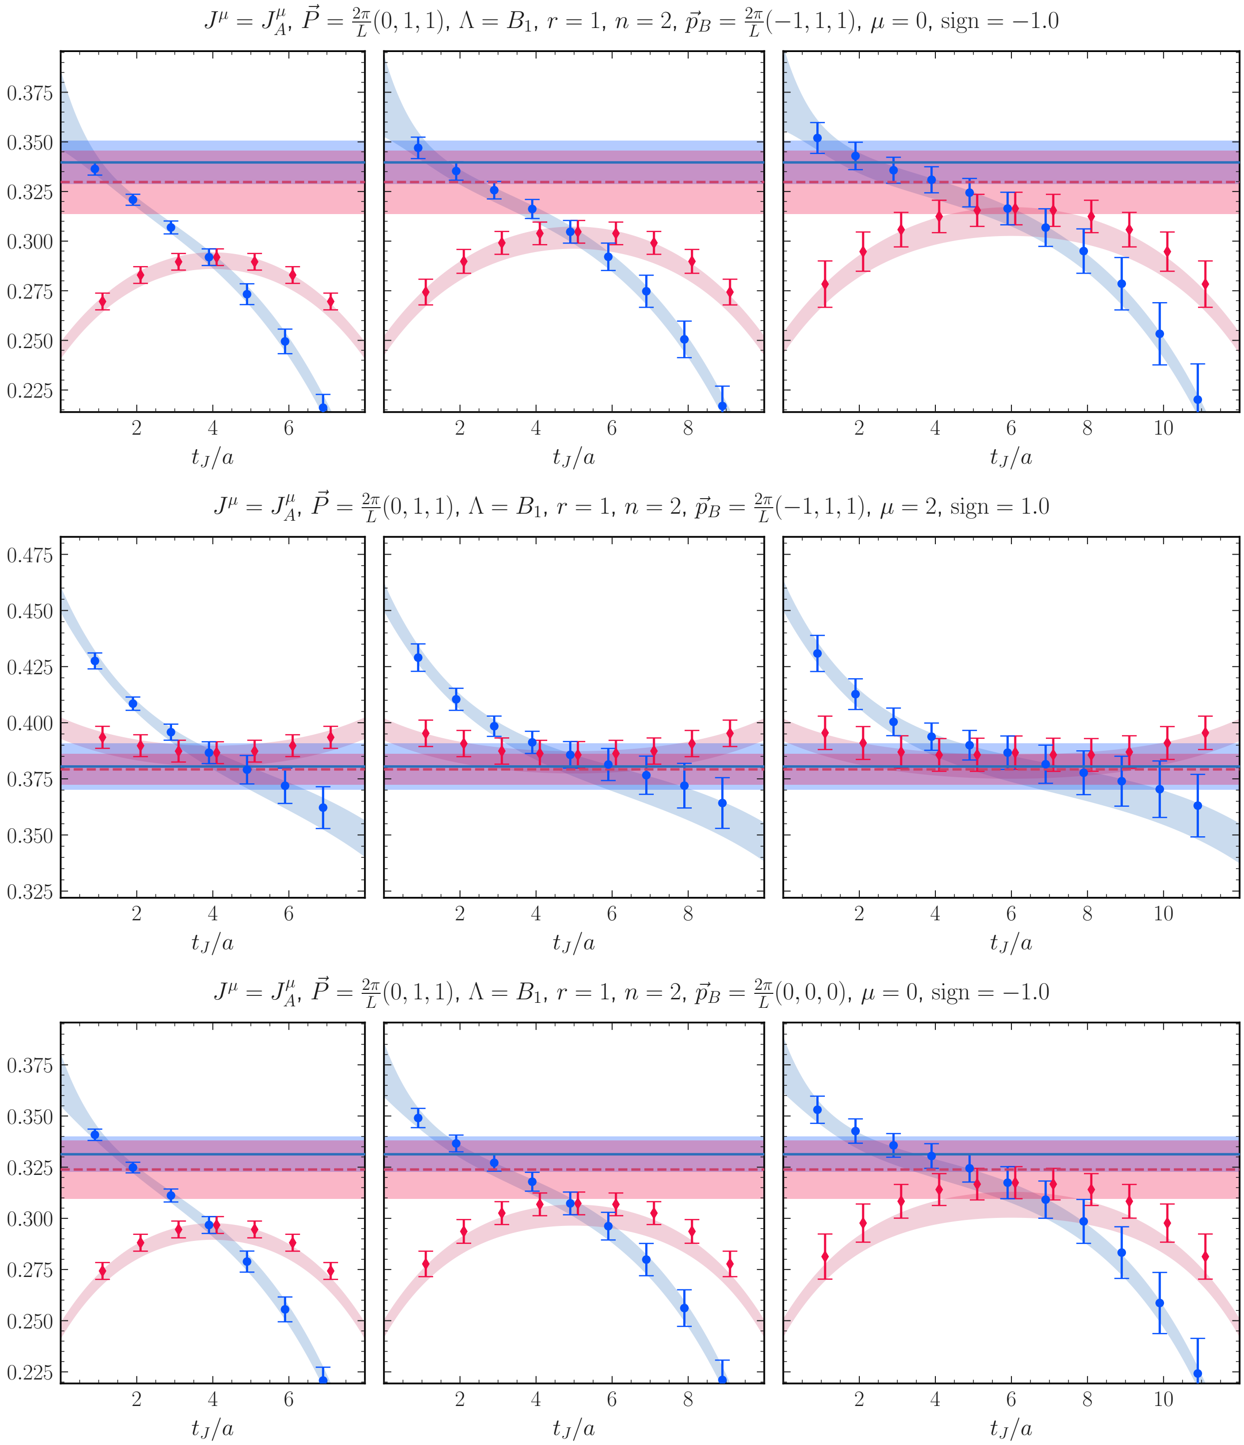

$J^{\mu} = J^{\mu}_{A}$, $\vec{P} = \frac{2\pi}{L}(0,1,1)$, $\Lambda = B_1$, $r = 1$, $n = 2$, $\vec{p}_B = \frac{2\pi}{L}(-1,1,1)$, $\mu = 0$, sign $= -1.0$
$J^{\mu} = J^{\mu}_{A}$, $\vec{P} = \frac{2\pi}{L}(0,1,1)$, $\Lambda = B_1$, $r = 1$, $n = 2$, $\vec{p}_B = \frac{2\pi}{L}(-1,1,1)$, $\mu = 2$, sign $= 1.0$
$J^{\mu} = J^{\mu}_{A}$, $\vec{P} = \frac{2\pi}{L}(0,1,1)$, $\Lambda = B_1$, $r = 1$, $n = 2$, $\vec{p}_B = \frac{2\pi}{L}(0,0,0)$, $\mu = 0$, sign $= -1.0$
$t_J/a$

$J^{\mu} = J_A^{\mu}$, $\vec{P} = \frac{2\pi}{L}(0,1,1)$, $\Lambda = B_1$, $r = 1$, $n = 2$, $\vec{p}_B = \frac{2\pi}{L}(0,0,0)$, $\mu = 2$, sign $= 1.0$

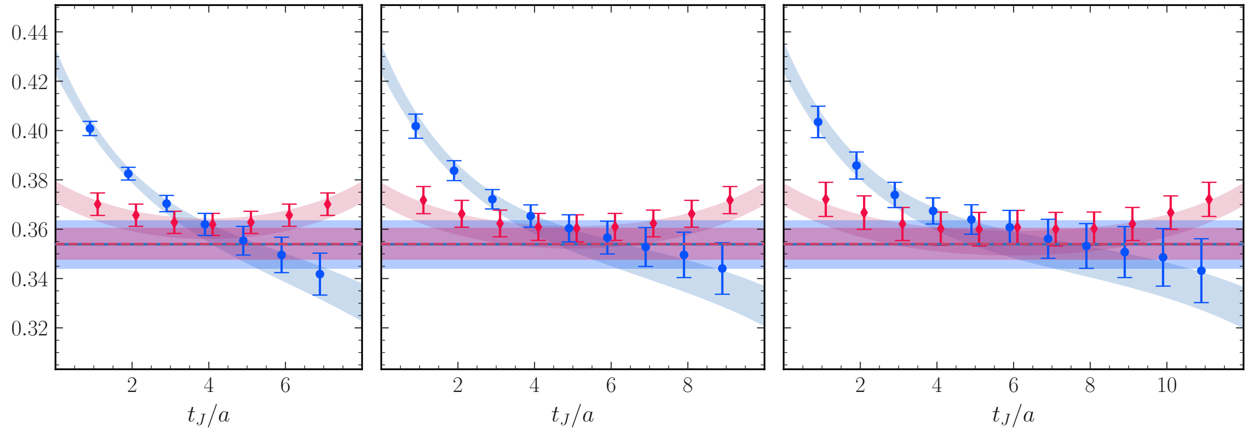


$J^{\mu} = J_A^{\mu}$, $\vec{P} = \frac{2\pi}{L}(0,1,1)$, $\Lambda = B_1$, $r = 1$, $n = 2$, $\vec{p}_B = \frac{2\pi}{L}(0,0,1)$, $\mu = 0$, sign $= -1.0$

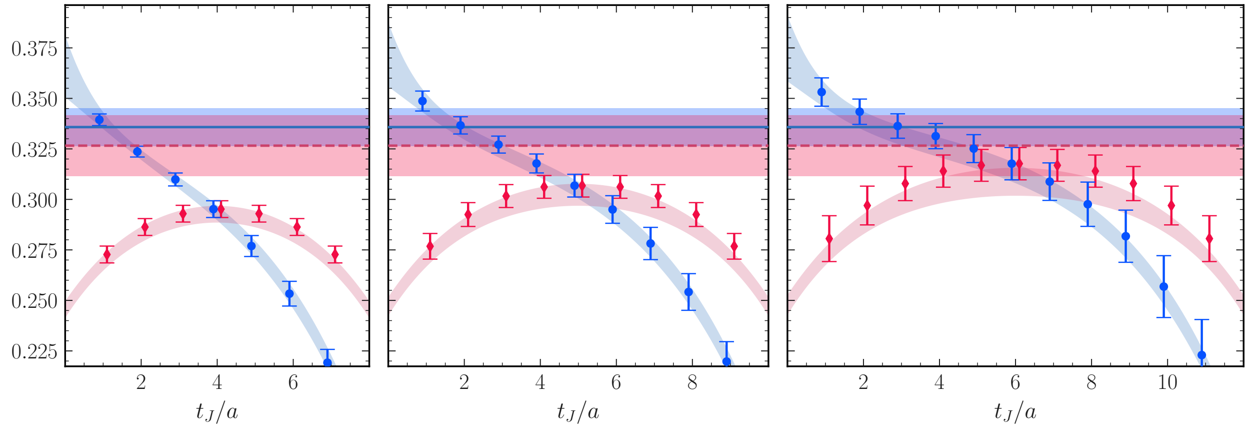


$J^{\mu} = J_A^{\mu}$, $\vec{P} = \frac{2\pi}{L}(0,1,1)$, $\Lambda = B_1$, $r = 1$, $n = 2$, $\vec{p}_B = \frac{2\pi}{L}(0,0,1)$, $\mu = 2$, sign $= 1.0$

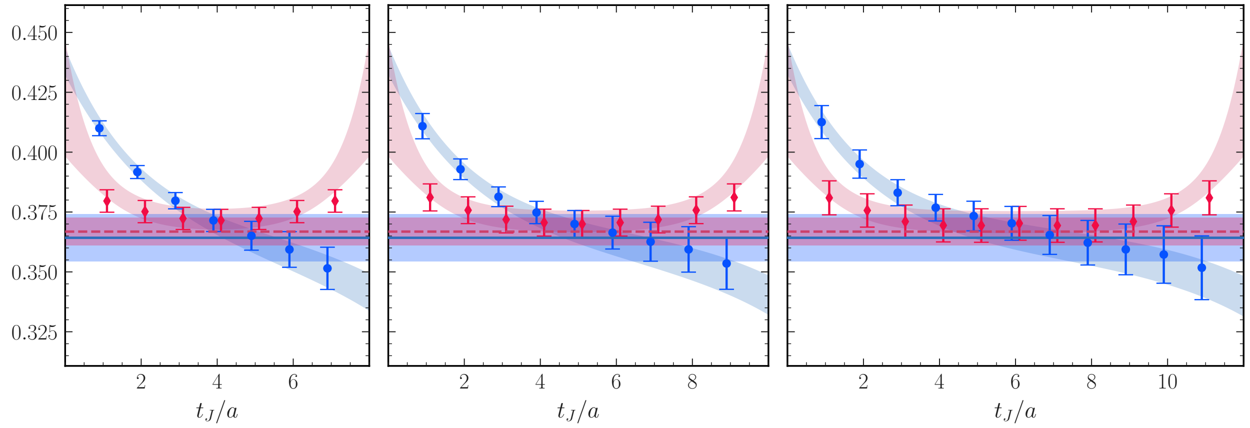

$J^\mu = J_A^\mu$, $\vec{P} = \frac{2\pi}{L}(0,1,1)$, $\Lambda = B_1$, $r = 1$, $n = 2$, $\vec{p}_B = \frac{2\pi}{L}(0,0,1)$, $\mu = 3$, sign = 1.0

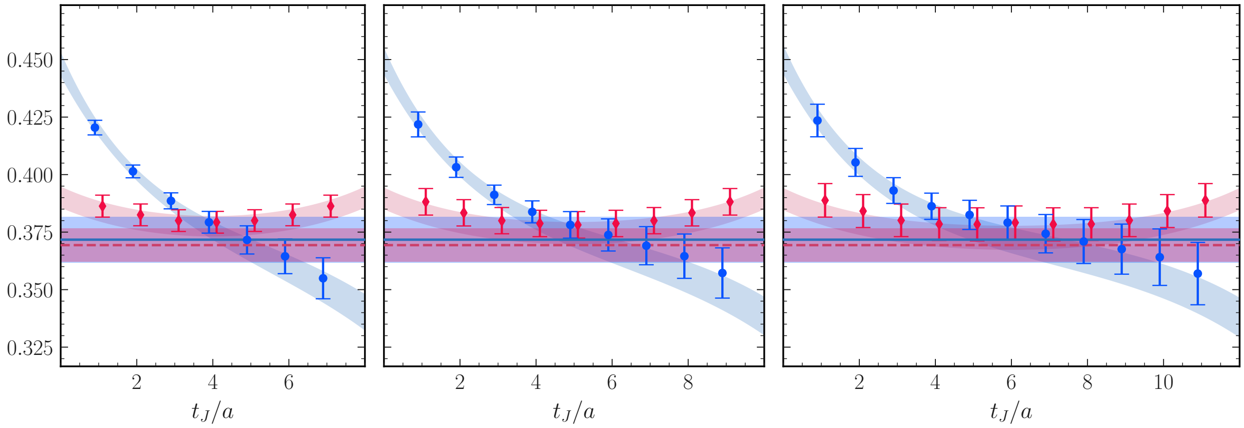


$J^\mu = J_A^\mu$, $\vec{P} = \frac{2\pi}{L}(0,1,1)$, $\Lambda = B_1$, $r = 1$, $n = 2$, $\vec{p}_B = \frac{2\pi}{L}(0,1,1)$, $\mu = 0$, sign = −1.0

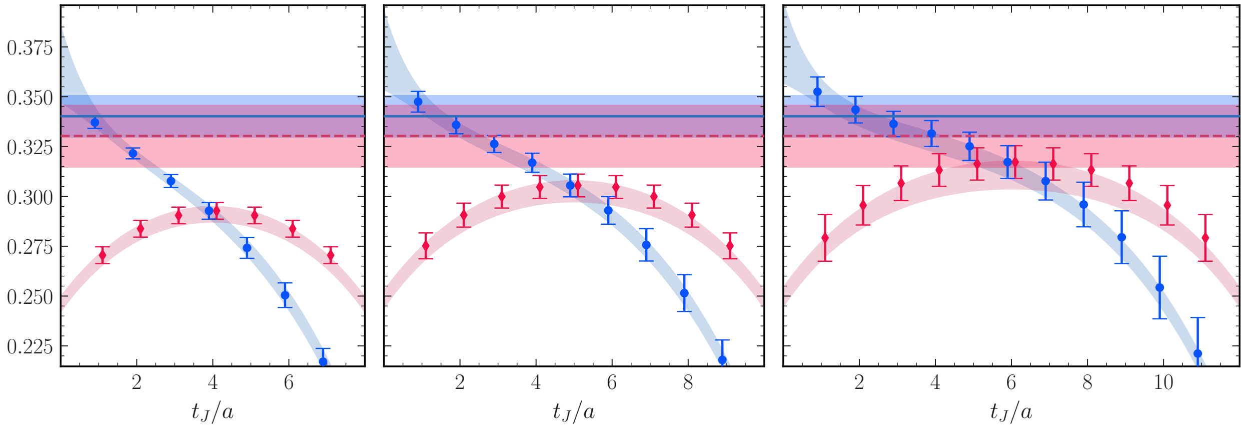


$J^\mu = J_A^\mu$, $\vec{P} = \frac{2\pi}{L}(0,1,1)$, $\Lambda = B_1$, $r = 1$, $n = 2$, $\vec{p}_B = \frac{2\pi}{L}(0,1,1)$, $\mu = 2$, sign = 1.0

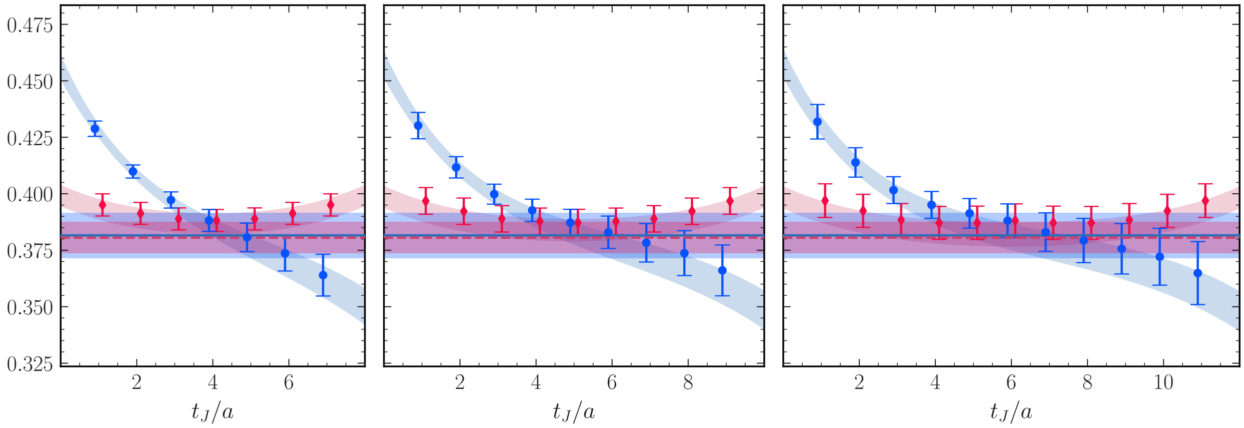

$J^\mu = J_A^\mu$, $\vec{P} = \frac{2\pi}{L}(0,1,1)$, $\Lambda = B_2$, $r = 1$, $n = 1$, $\vec{p}_B = \frac{2\pi}{L}(-1,0,0)$, $\mu = 2$, sign $= 1.0$

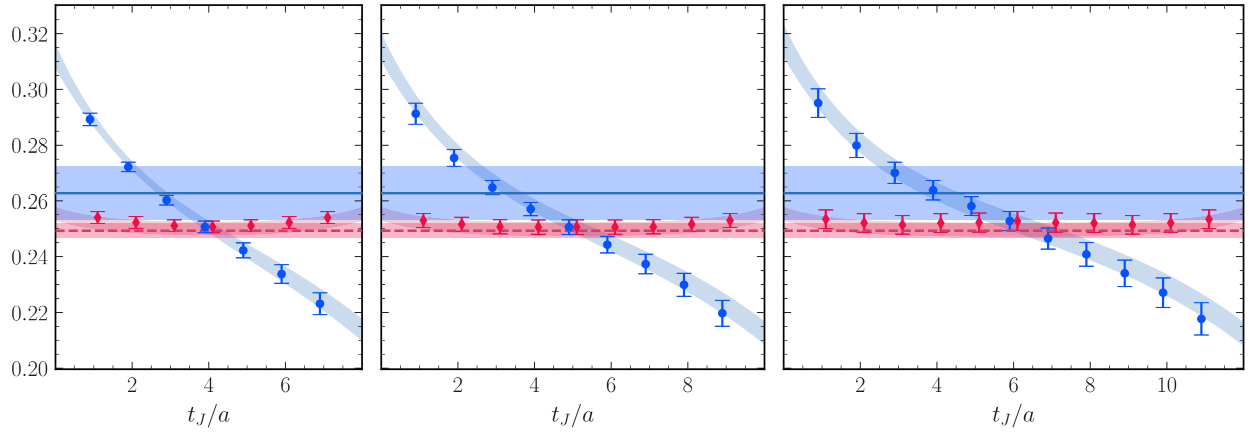


$J^\mu = J_A^\mu$, $\vec{P} = \frac{2\pi}{L}(0,1,1)$, $\Lambda = B_2$, $r = 1$, $n = 1$, $\vec{p}_B = \frac{2\pi}{L}(-1,0,0)$, $\mu = 3$, sign $= -1.0$

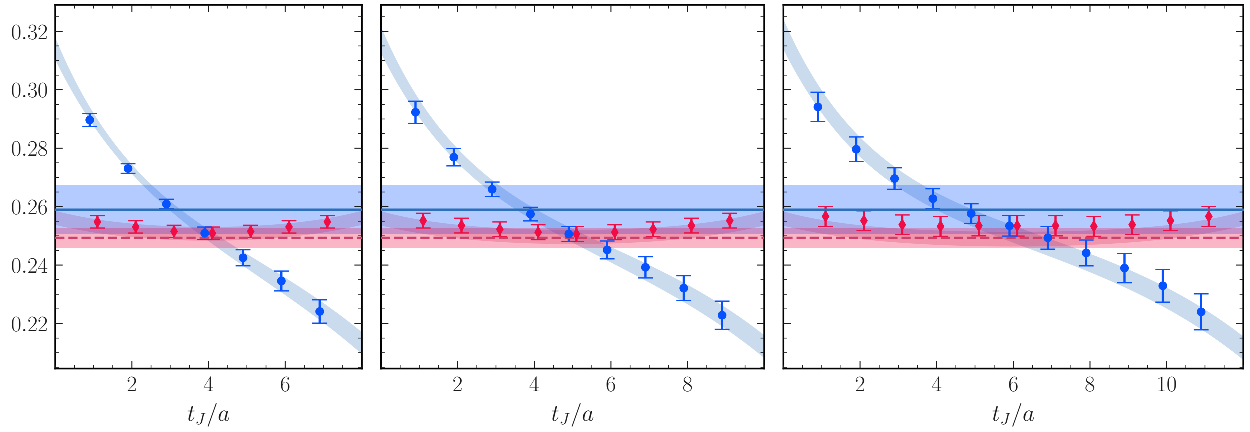


$J^\mu = J_A^\mu$, $\vec{P} = \frac{2\pi}{L}(0,1,1)$, $\Lambda = B_2$, $r = 1$, $n = 1$, $\vec{p}_B = \frac{2\pi}{L}(-1,0,1)$, $\mu = 2$, sign $= 1.0$

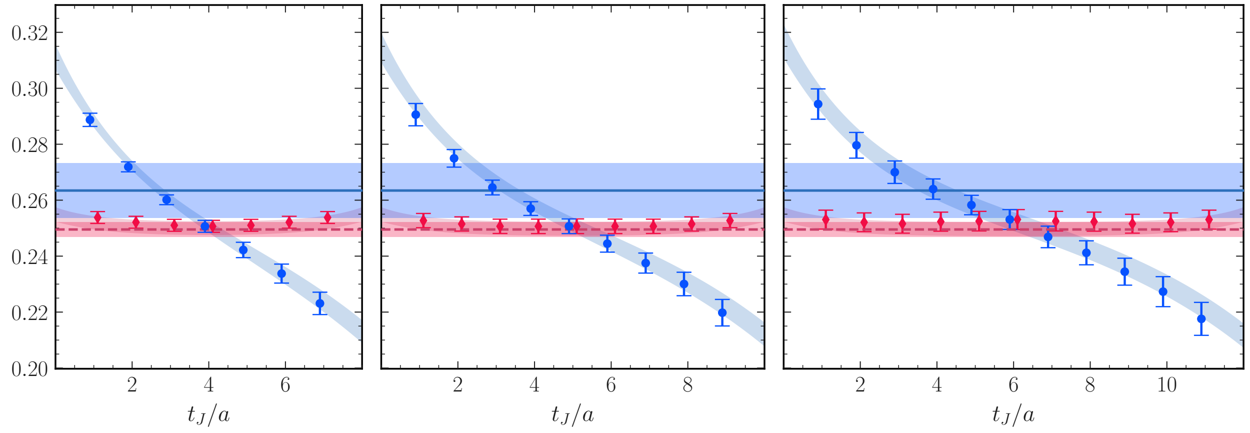

$J^\mu = J^\mu_A$, $\vec{P} = \frac{2\pi}{L}(0,1,1)$, $\Lambda = B_2$, $r = 1$, $n = 1$, $\vec{p}_B = \frac{2\pi}{L}(-1,0,1)$, $\mu = 3$, sign $= -1.0$

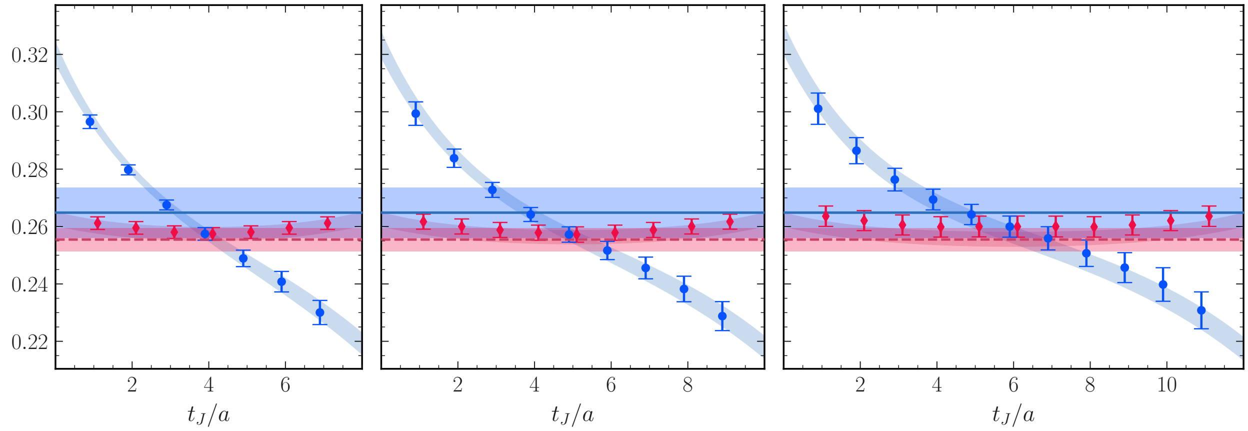


$J^\mu = J^\mu_A$, $\vec{P} = \frac{2\pi}{L}(0,1,1)$, $\Lambda = B_2$, $r = 1$, $n = 1$, $\vec{p}_B = \frac{2\pi}{L}(-1,1,0)$, $\mu = 2$, sign $= 1.0$

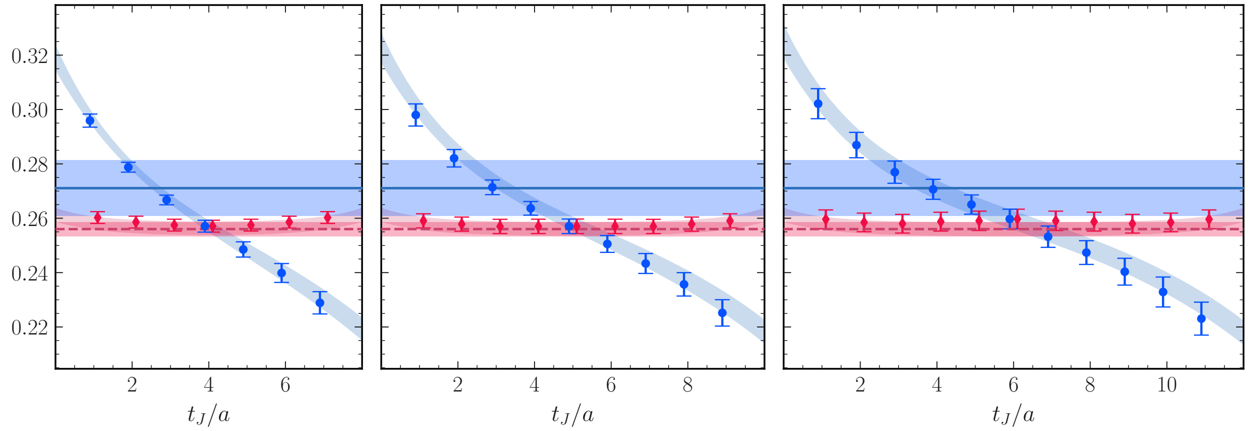


$J^\mu = J^\mu_A$, $\vec{P} = \frac{2\pi}{L}(0,1,1)$, $\Lambda = B_2$, $r = 1$, $n = 1$, $\vec{p}_B = \frac{2\pi}{L}(-1,1,0)$, $\mu = 3$, sign $= -1.0$

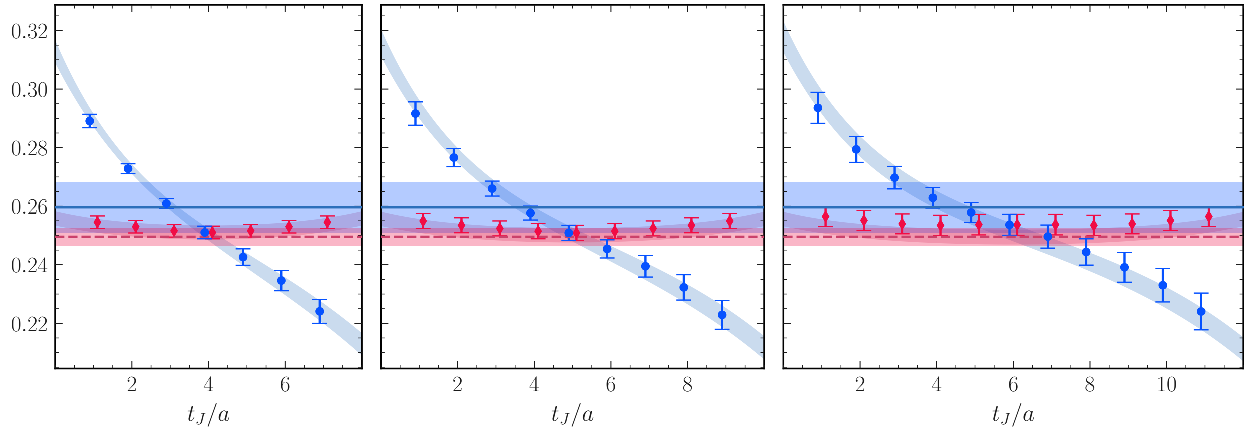

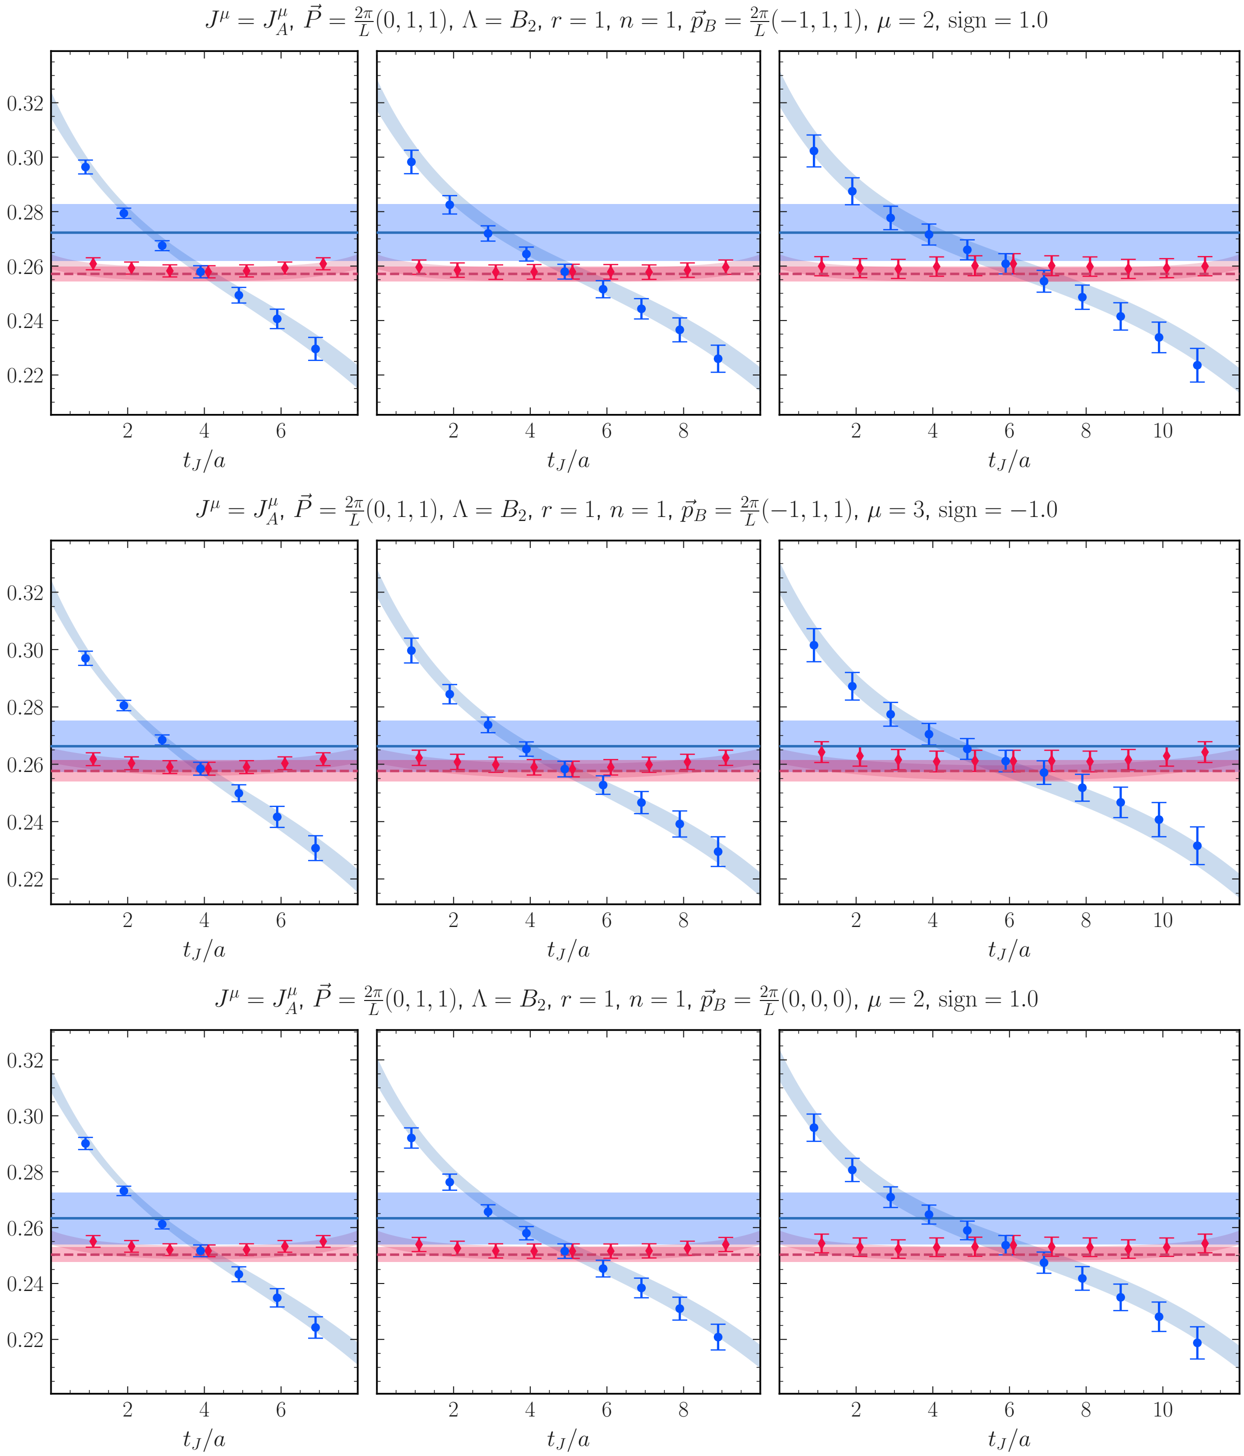
$J^\mu = J^\mu_A$, $\vec{P} = \frac{2\pi}{L}(0,1,1)$, $\Lambda = B_2$, $r = 1$, $n = 1$, $\vec{p}_B = \frac{2\pi}{L}(-1,1,1)$, $\mu = 2$, sign = 1.0
$J^\mu = J^\mu_A$, $\vec{P} = \frac{2\pi}{L}(0,1,1)$, $\Lambda = B_2$, $r = 1$, $n = 1$, $\vec{p}_B = \frac{2\pi}{L}(-1,1,1)$, $\mu = 3$, sign = −1.0
$J^\mu = J^\mu_A$, $\vec{P} = \frac{2\pi}{L}(0,1,1)$, $\Lambda = B_2$, $r = 1$, $n = 1$, $\vec{p}_B = \frac{2\pi}{L}(0,0,0)$, $\mu = 2$, sign = 1.0
0.22
0.24
0.26
0.28
0.30
0.32
2
4
6
8
10
$t_J/a$

$J^\mu = J_A^\mu$, $\vec{P} = \frac{2\pi}{L}(0,1,1)$, $\Lambda = B_2$, $r = 1$, $n = 1$, $\vec{p}_B = \frac{2\pi}{L}(0,0,0)$, $\mu = 3$, sign $= -1.0$

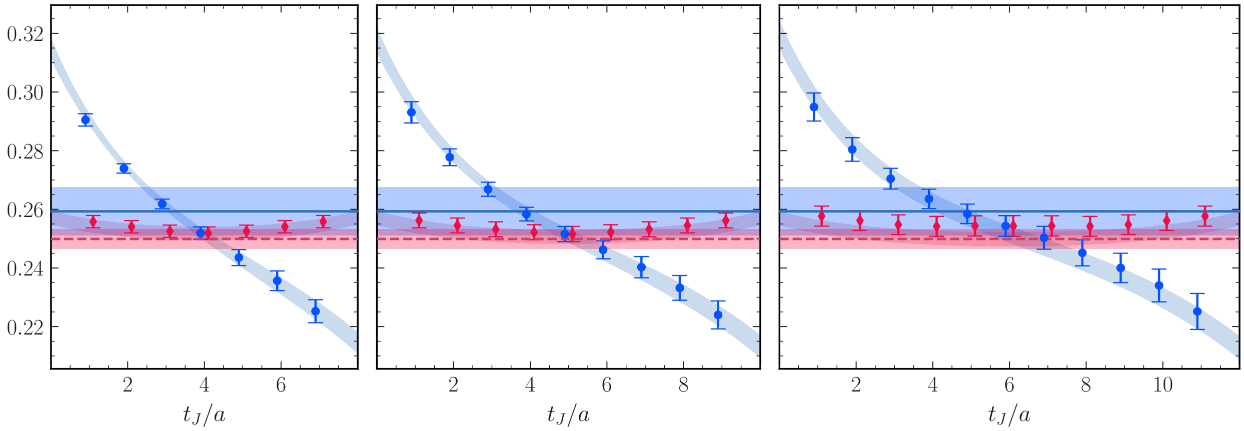


$J^\mu = J_A^\mu$, $\vec{P} = \frac{2\pi}{L}(0,1,1)$, $\Lambda = B_2$, $r = 1$, $n = 1$, $\vec{p}_B = \frac{2\pi}{L}(0,0,1)$, $\mu = 2$, sign $= 1.0$

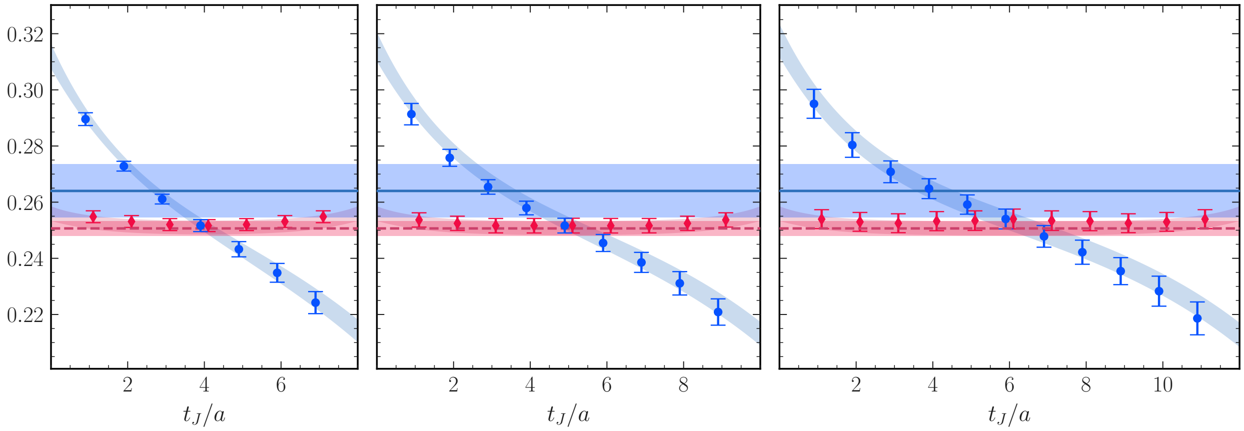


$J^\mu = J_A^\mu$, $\vec{P} = \frac{2\pi}{L}(0,1,1)$, $\Lambda = B_2$, $r = 1$, $n = 1$, $\vec{p}_B = \frac{2\pi}{L}(0,0,1)$, $\mu = 3$, sign $= -1.0$

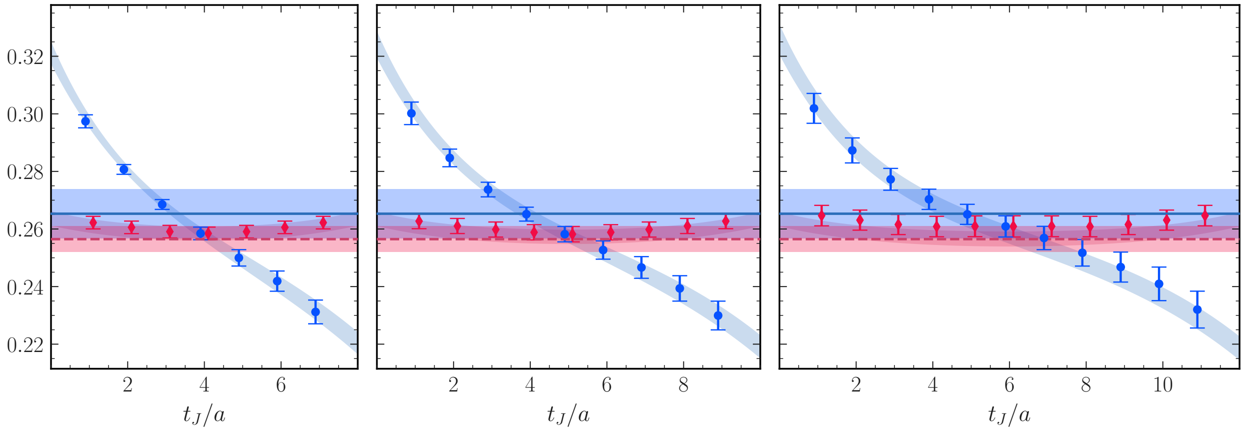

$J^\mu = J_A^\mu$, $\vec{P} = \frac{2\pi}{L}(0,1,1)$, $\Lambda = B_2$, $r = 1$, $n = 1$, $\vec{p}_B = \frac{2\pi}{L}(0,1,0)$, $\mu = 2$, sign $= 1.0$

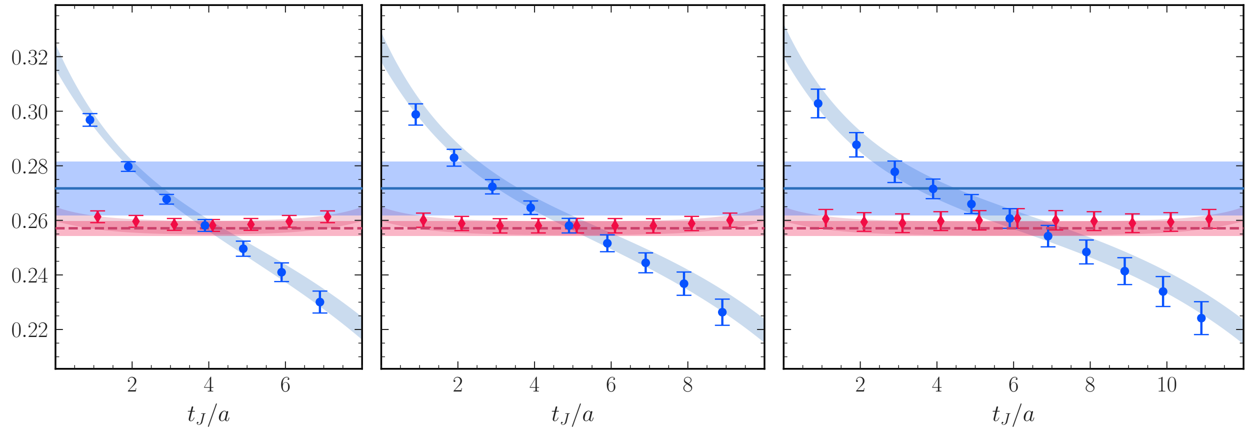


$J^\mu = J_A^\mu$, $\vec{P} = \frac{2\pi}{L}(0,1,1)$, $\Lambda = B_2$, $r = 1$, $n = 1$, $\vec{p}_B = \frac{2\pi}{L}(0,1,0)$, $\mu = 3$, sign $= -1.0$

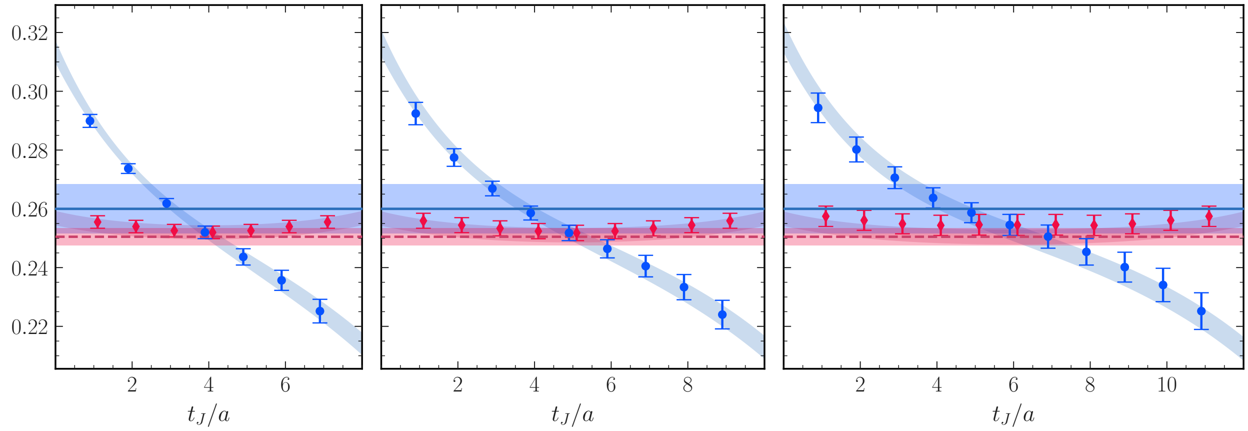


$J^\mu = J_A^\mu$, $\vec{P} = \frac{2\pi}{L}(0,1,1)$, $\Lambda = B_2$, $r = 1$, $n = 1$, $\vec{p}_B = \frac{2\pi}{L}(0,1,1)$, $\mu = 2$, sign $= 1.0$

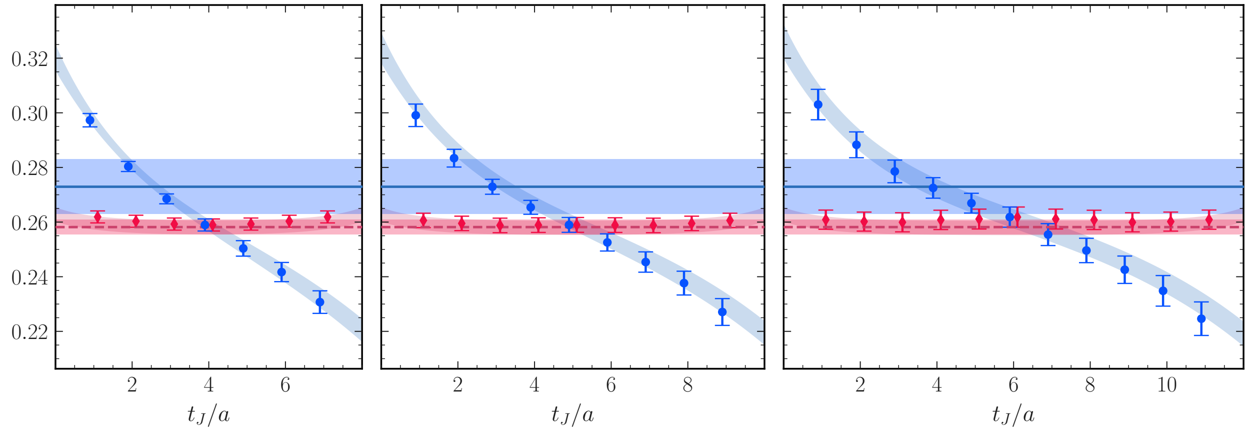

$J^\mu = J_A^\mu$, $\vec{P} = \frac{2\pi}{L}(0,1,1)$, $\Lambda = B_2$, $r = 1$, $n = 1$, $\vec{p}_B = \frac{2\pi}{L}(0,1,1)$, $\mu = 3$, sign $= -1.0$

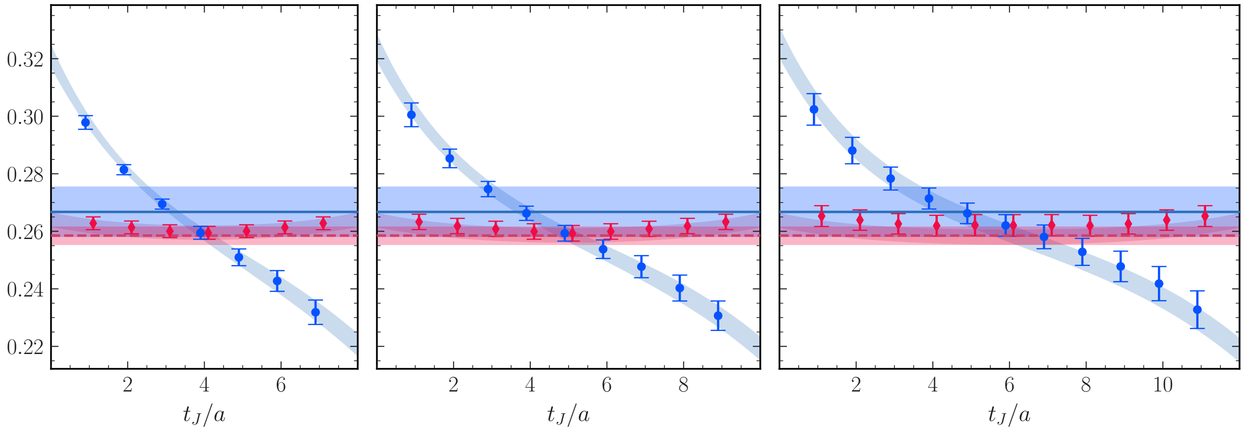


$J^\mu = J_A^\mu$, $\vec{P} = \frac{2\pi}{L}(0,1,1)$, $\Lambda = B_2$, $r = 1$, $n = 2$, $\vec{p}_B = \frac{2\pi}{L}(-1,0,0)$, $\mu = 2$, sign $= 1.0$

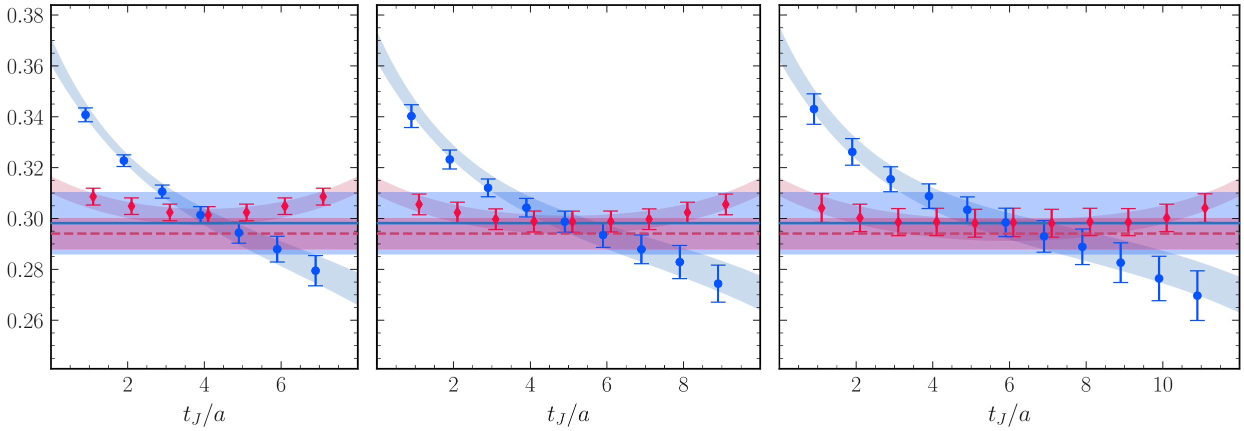


$J^\mu = J_A^\mu$, $\vec{P} = \frac{2\pi}{L}(0,1,1)$, $\Lambda = B_2$, $r = 1$, $n = 2$, $\vec{p}_B = \frac{2\pi}{L}(-1,0,0)$, $\mu = 3$, sign $= -1.0$

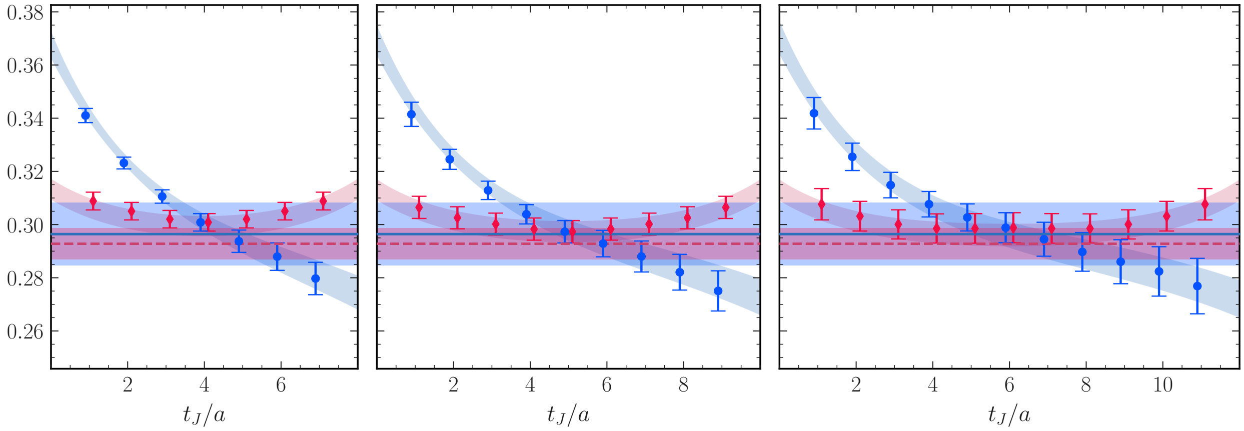

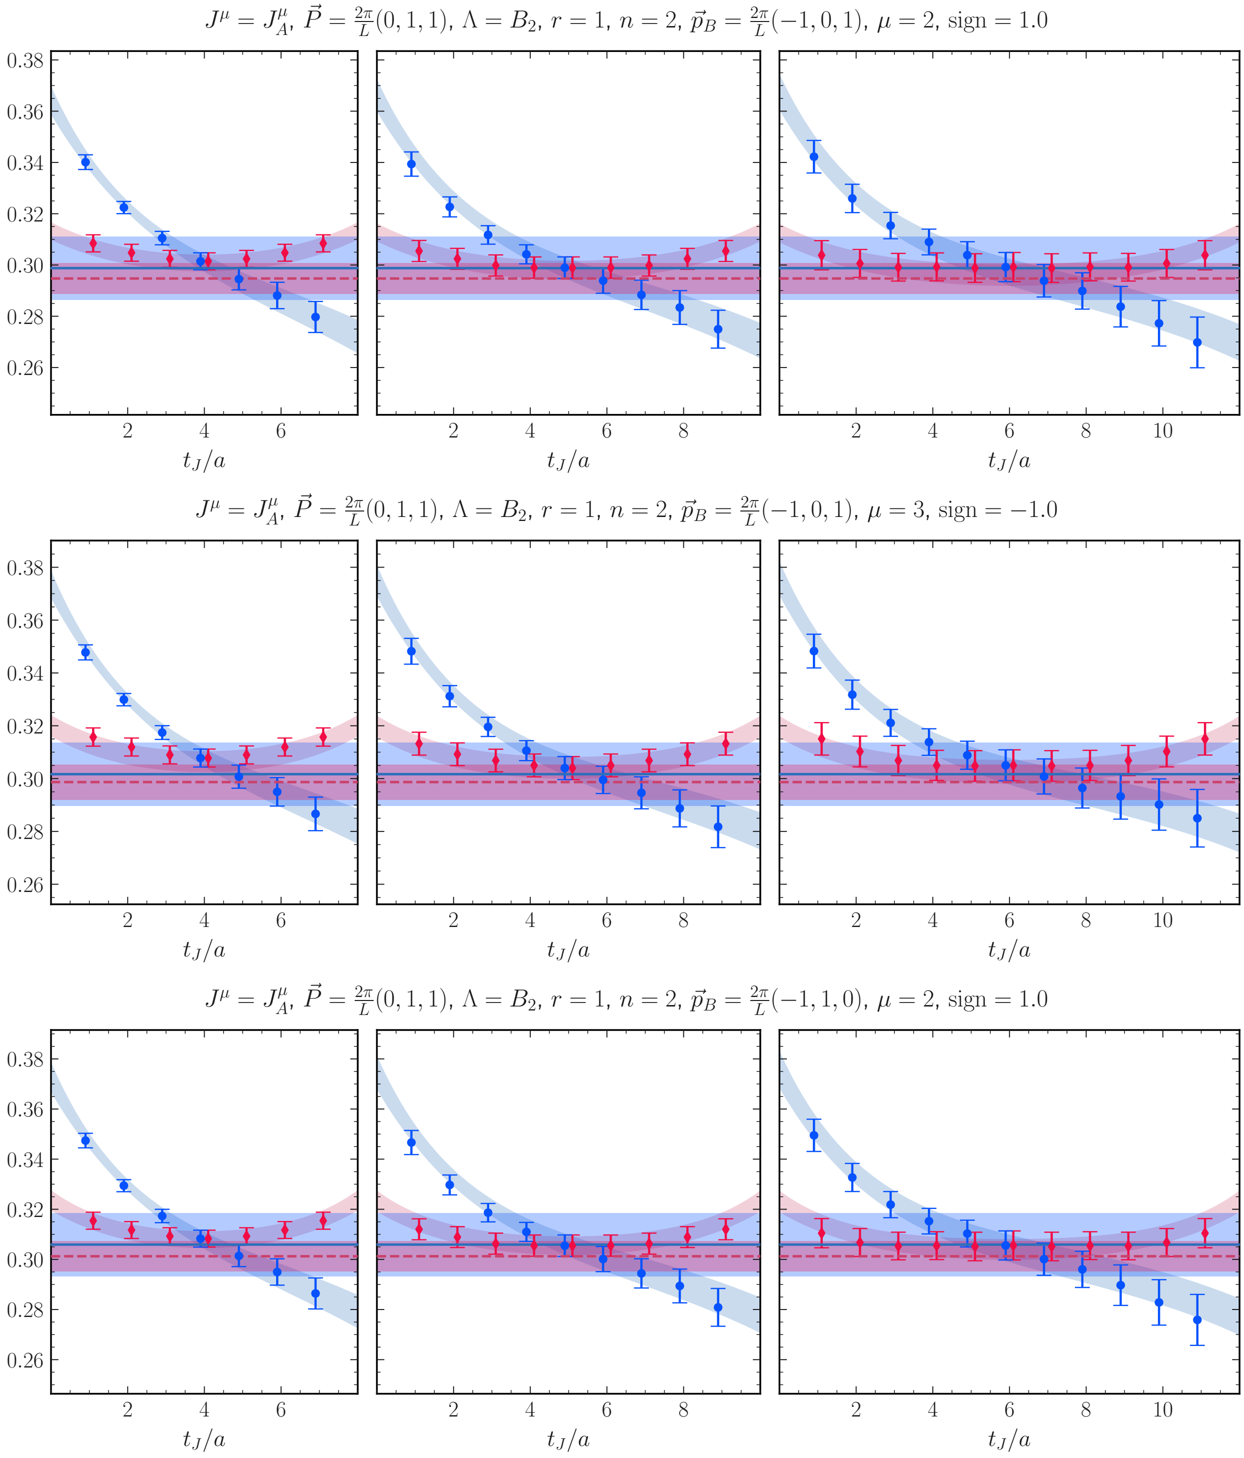
$J^\mu = J_A^\mu$, $\vec{P} = \frac{2\pi}{L}(0,1,1)$, $\Lambda = B_2$, $r = 1$, $n = 2$, $\vec{p}_B = \frac{2\pi}{L}(-1,0,1)$, $\mu = 2$, sign $= 1.0$
$J^\mu = J_A^\mu$, $\vec{P} = \frac{2\pi}{L}(0,1,1)$, $\Lambda = B_2$, $r = 1$, $n = 2$, $\vec{p}_B = \frac{2\pi}{L}(-1,0,1)$, $\mu = 3$, sign $= -1.0$
$J^\mu = J_A^\mu$, $\vec{P} = \frac{2\pi}{L}(0,1,1)$, $\Lambda = B_2$, $r = 1$, $n = 2$, $\vec{p}_B = \frac{2\pi}{L}(-1,1,0)$, $\mu = 2$, sign $= 1.0$
$t_J/a$
0.26
0.28
0.30
0.32
0.34
0.36
0.38

$J^\mu = J_A^\mu$, $\vec{P} = \frac{2\pi}{L}(0,1,1)$, $\Lambda = B_2$, $r = 1$, $n = 2$, $\vec{p}_B = \frac{2\pi}{L}(-1,1,0)$, $\mu = 3$, sign $= -1.0$

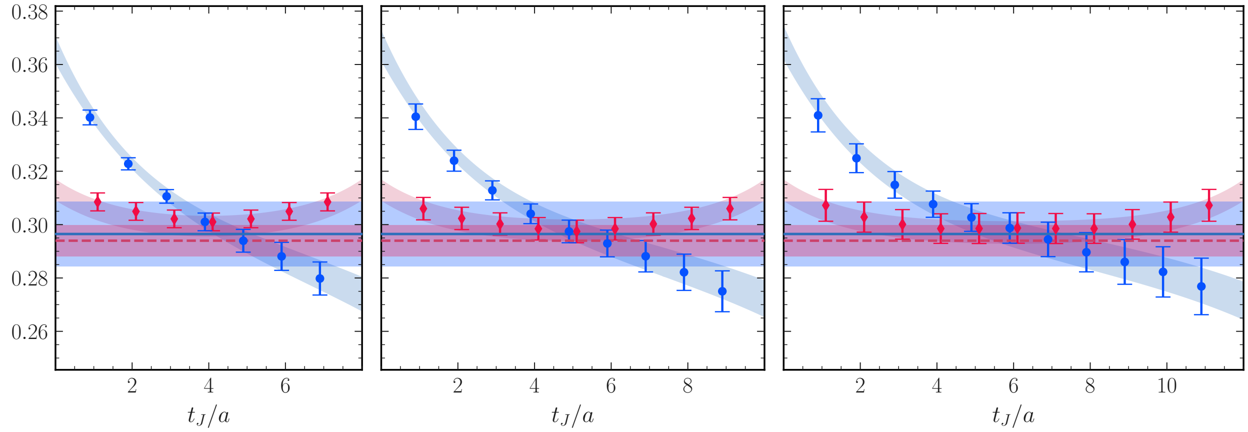


$J^\mu = J_A^\mu$, $\vec{P} = \frac{2\pi}{L}(0,1,1)$, $\Lambda = B_2$, $r = 1$, $n = 2$, $\vec{p}_B = \frac{2\pi}{L}(-1,1,1)$, $\mu = 2$, sign $= 1.0$

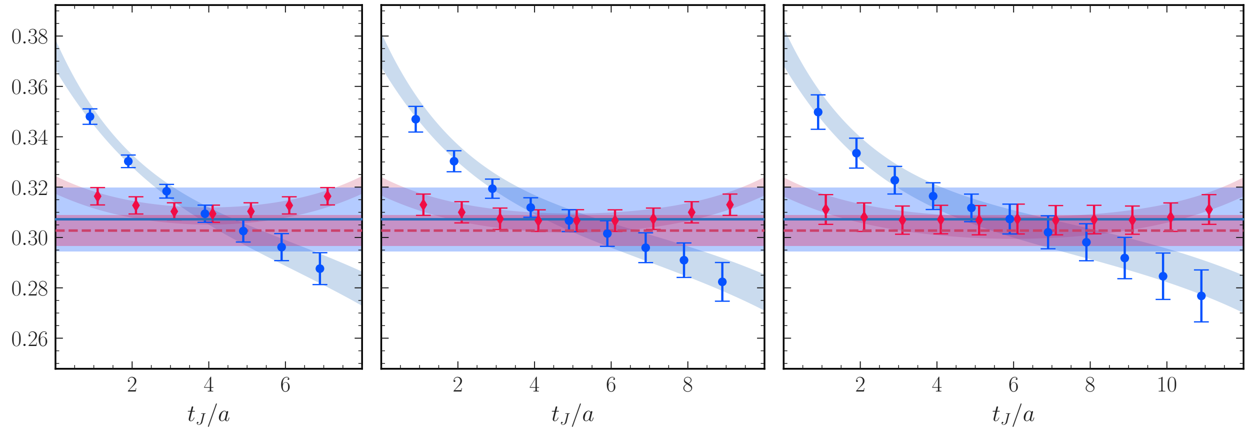


$J^\mu = J_A^\mu$, $\vec{P} = \frac{2\pi}{L}(0,1,1)$, $\Lambda = B_2$, $r = 1$, $n = 2$, $\vec{p}_B = \frac{2\pi}{L}(-1,1,1)$, $\mu = 3$, sign $= -1.0$

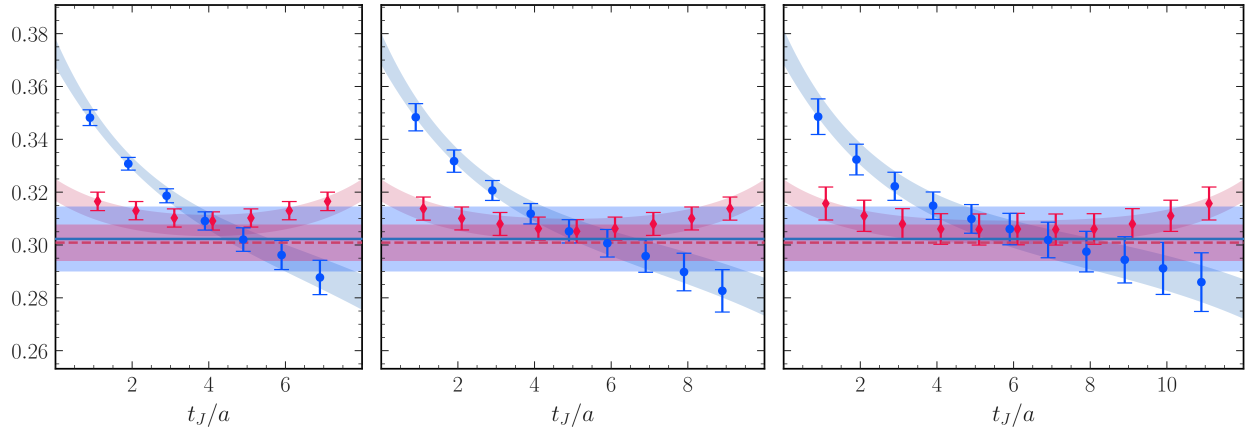

$J^\mu = J_A^\mu$, $\vec{P} = \frac{2\pi}{L}(0,1,1)$, $\Lambda = B_2$, $r = 1$, $n = 2$, $\vec{p}_B = \frac{2\pi}{L}(0,0,0)$, $\mu = 2$, sign $= 1.0$

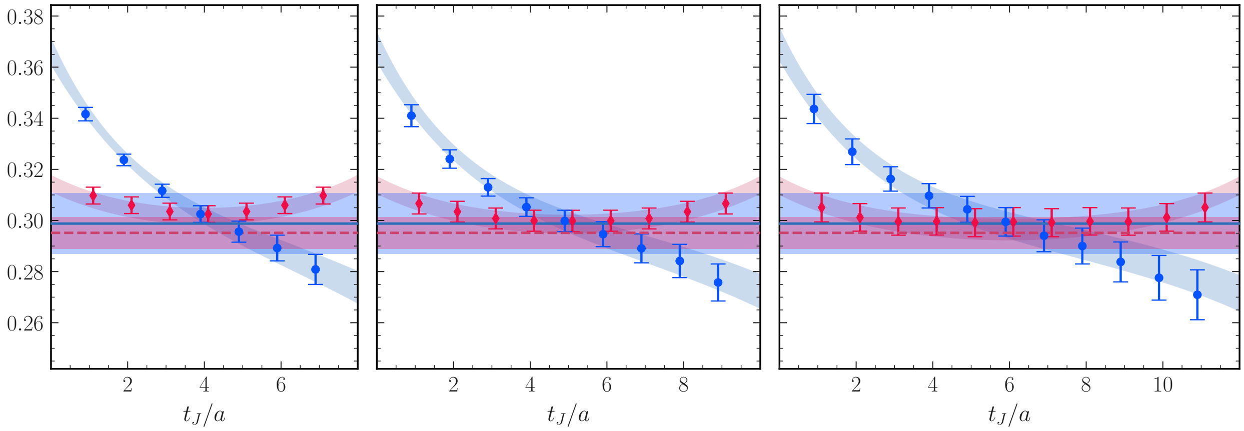


$J^\mu = J_A^\mu$, $\vec{P} = \frac{2\pi}{L}(0,1,1)$, $\Lambda = B_2$, $r = 1$, $n = 2$, $\vec{p}_B = \frac{2\pi}{L}(0,0,0)$, $\mu = 3$, sign $= -1.0$

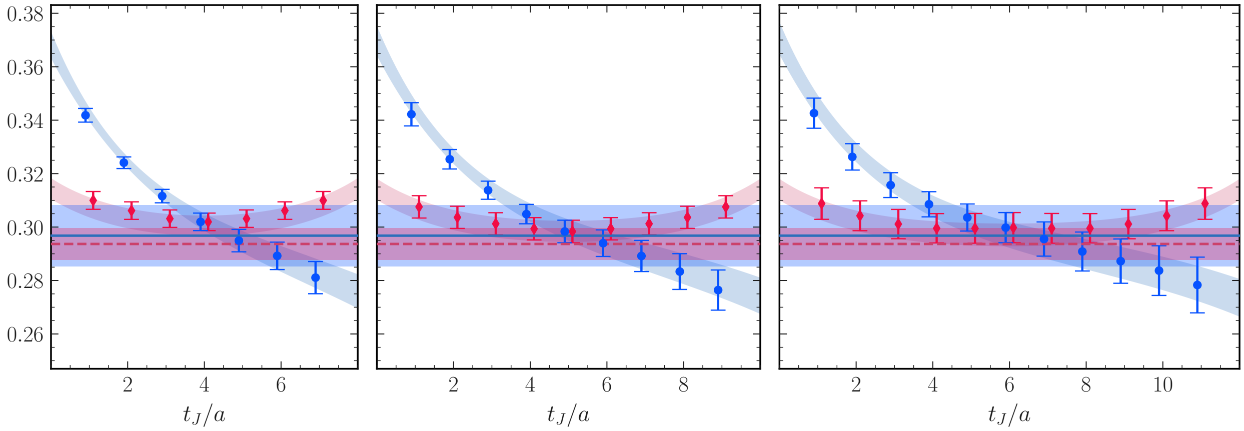


$J^\mu = J_A^\mu$, $\vec{P} = \frac{2\pi}{L}(0,1,1)$, $\Lambda = B_2$, $r = 1$, $n = 2$, $\vec{p}_B = \frac{2\pi}{L}(0,0,1)$, $\mu = 2$, sign $= 1.0$

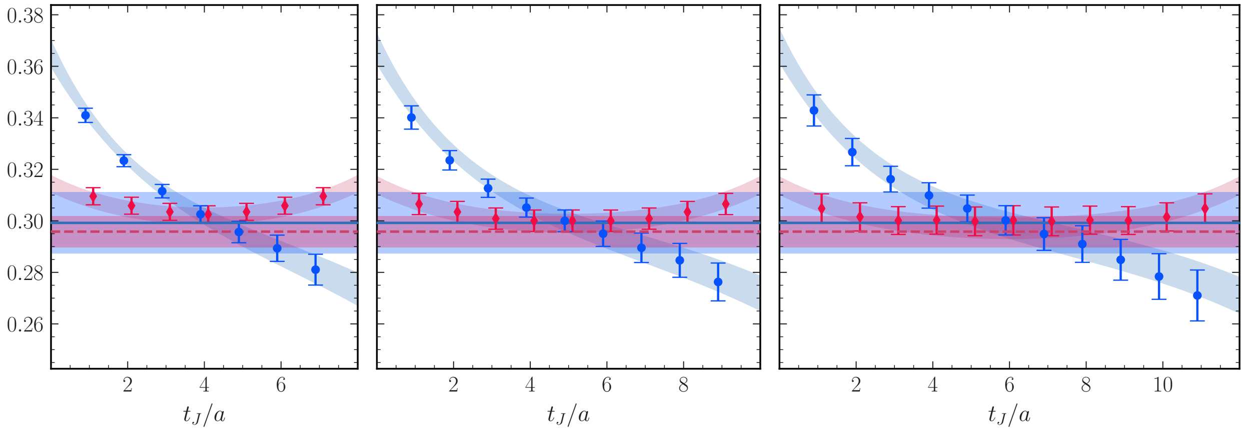

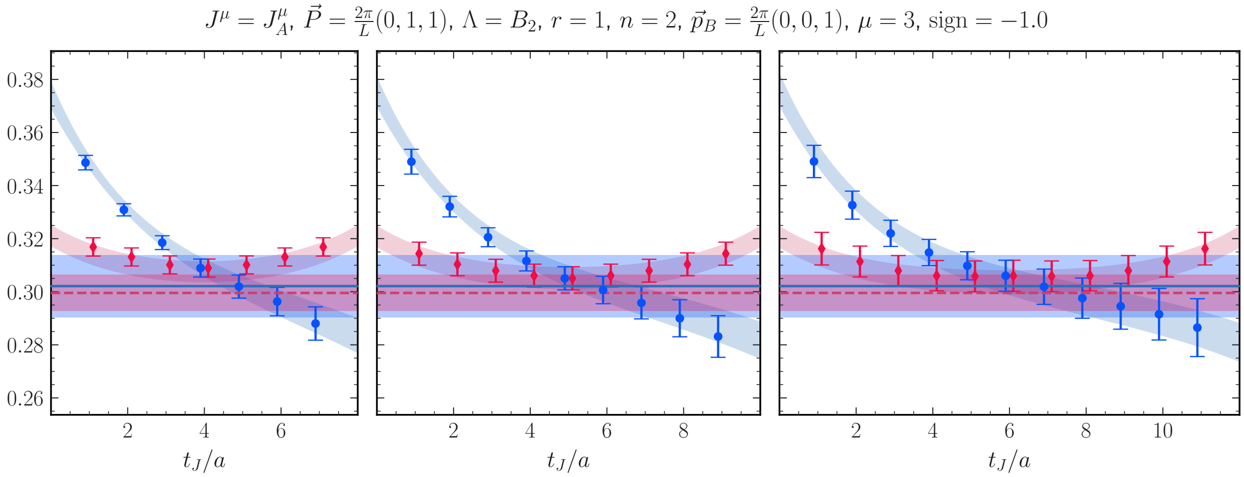
$J^\mu = J^\mu_A$, $\vec{P} = \frac{2\pi}{L}(0,1,1)$, $\Lambda = B_2$, $r = 1$, $n = 2$, $\vec{p}_B = \frac{2\pi}{L}(0,0,1)$, $\mu = 3$, sign $= -1.0$
0.38
0.36
0.34
0.32
0.30
0.28
0.26
$t_J/a$
$t_J/a$
$t_J/a$

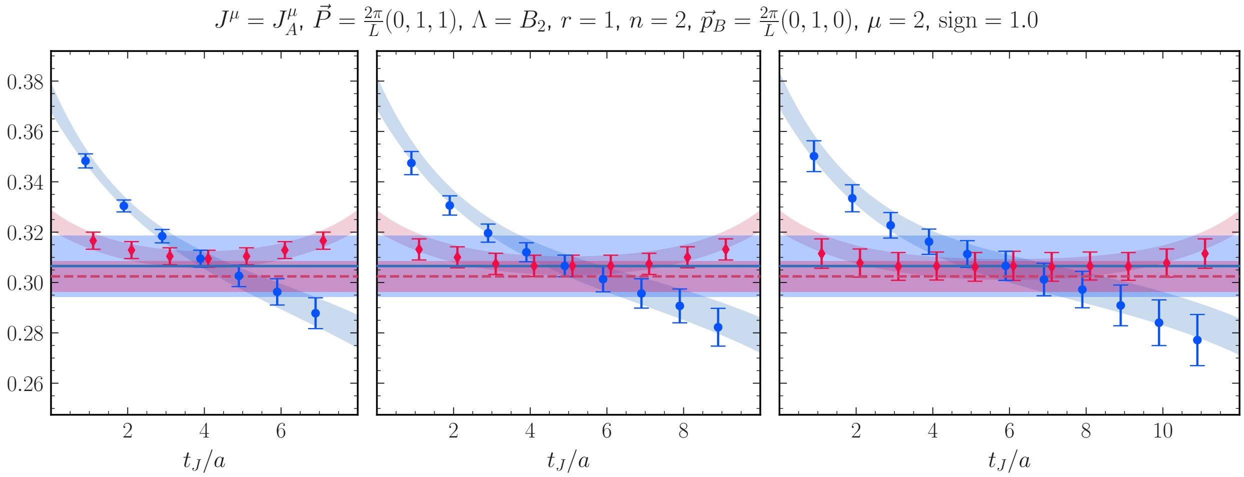
$J^\mu = J^\mu_A$, $\vec{P} = \frac{2\pi}{L}(0,1,1)$, $\Lambda = B_2$, $r = 1$, $n = 2$, $\vec{p}_B = \frac{2\pi}{L}(0,1,0)$, $\mu = 2$, sign $= 1.0$
0.38
0.36
0.34
0.32
0.30
0.28
0.26
$t_J/a$
$t_J/a$
$t_J/a$

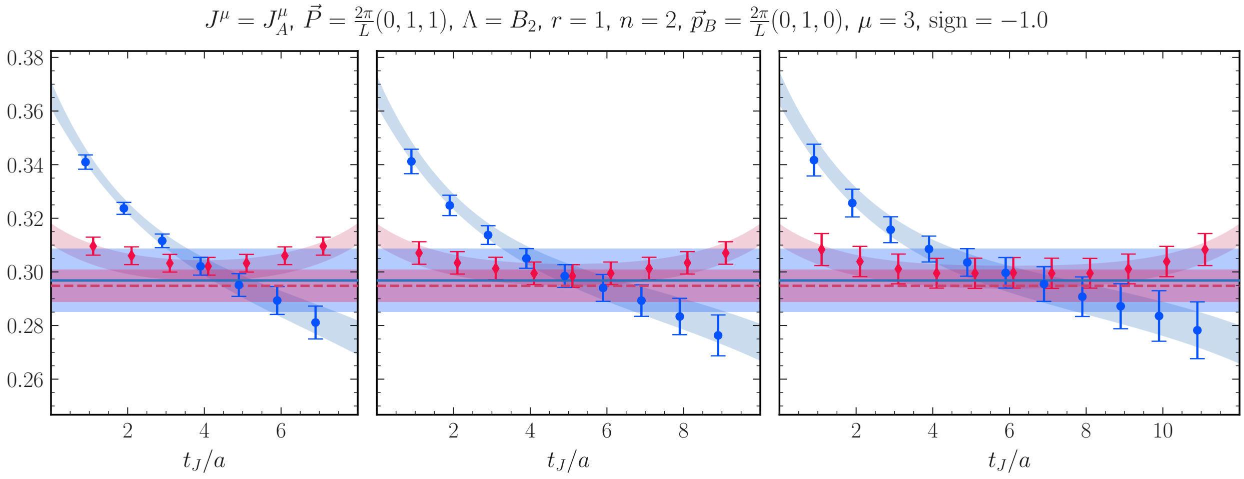
$J^\mu = J^\mu_A$, $\vec{P} = \frac{2\pi}{L}(0,1,1)$, $\Lambda = B_2$, $r = 1$, $n = 2$, $\vec{p}_B = \frac{2\pi}{L}(0,1,0)$, $\mu = 3$, sign $= -1.0$
0.38
0.36
0.34
0.32
0.30
0.28
0.26
$t_J/a$
$t_J/a$
$t_J/a$

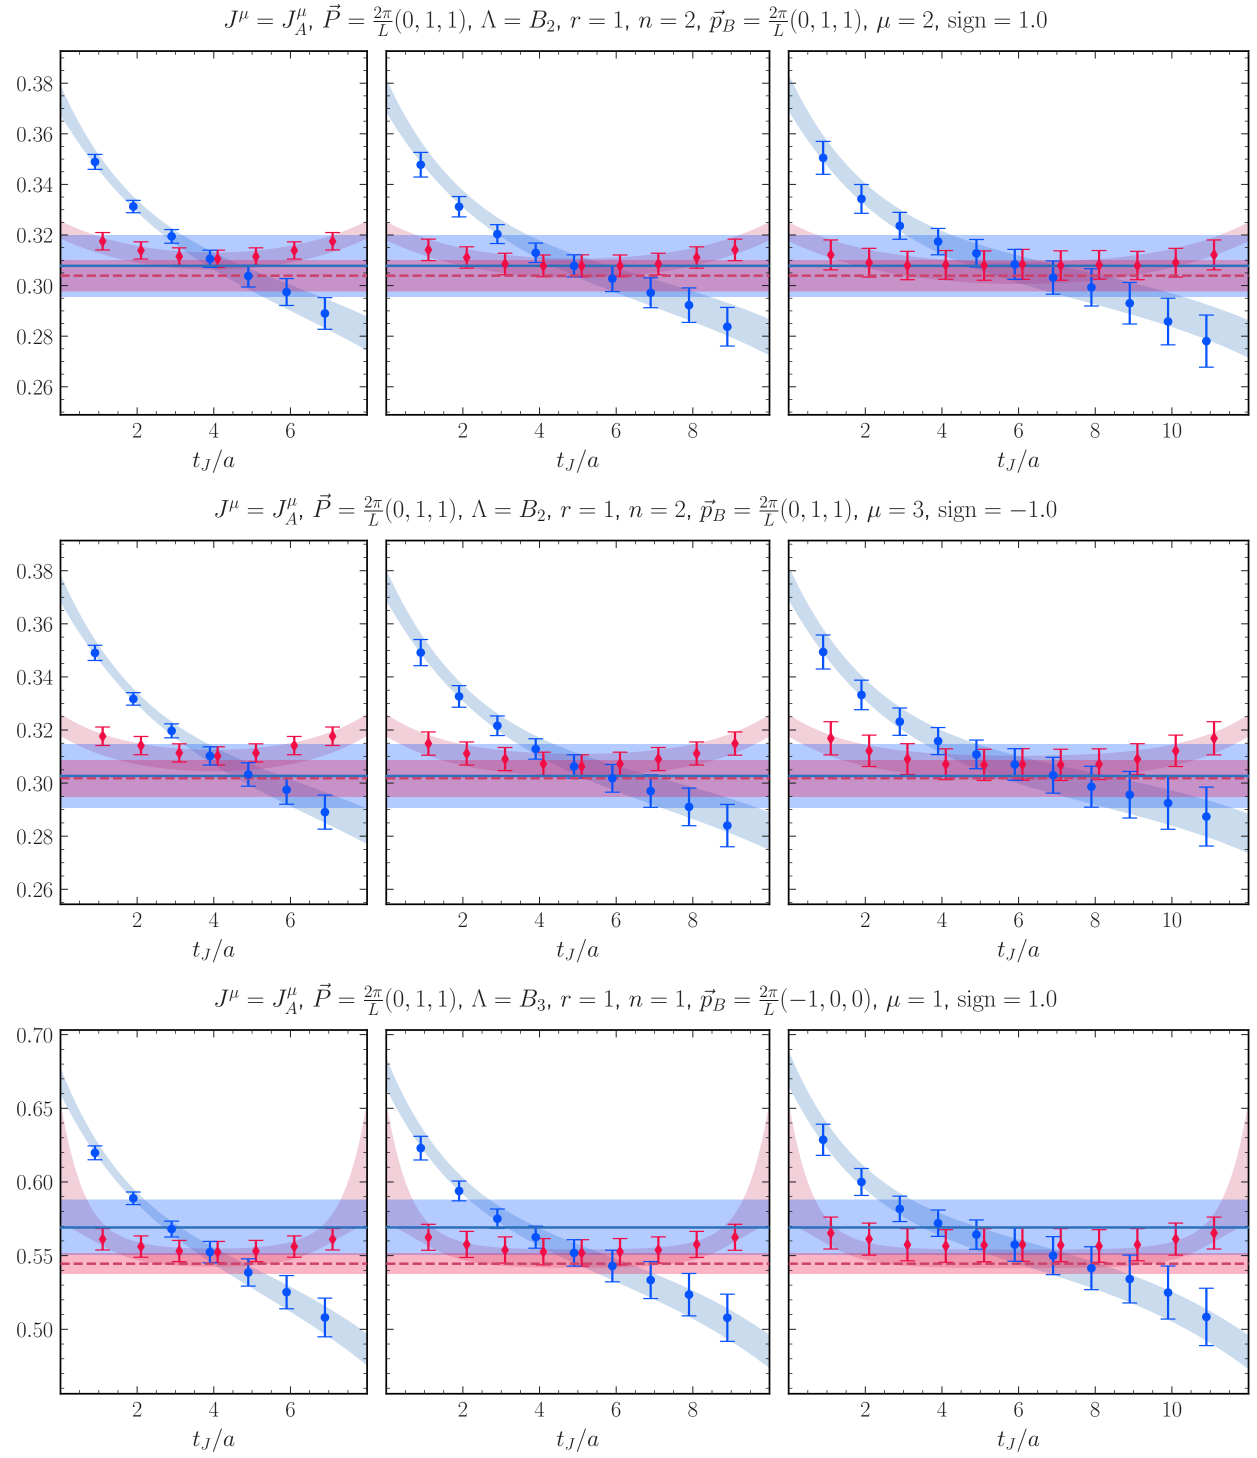
$J^\mu = J^\mu_A$, $\vec{P} = \frac{2\pi}{L}(0,1,1)$, $\Lambda = B_2$, $r = 1$, $n = 2$, $\vec{p}_B = \frac{2\pi}{L}(0,1,1)$, $\mu = 2$, sign = 1.0
$J^\mu = J^\mu_A$, $\vec{P} = \frac{2\pi}{L}(0,1,1)$, $\Lambda = B_2$, $r = 1$, $n = 2$, $\vec{p}_B = \frac{2\pi}{L}(0,1,1)$, $\mu = 3$, sign = −1.0
$J^\mu = J^\mu_A$, $\vec{P} = \frac{2\pi}{L}(0,1,1)$, $\Lambda = B_3$, $r = 1$, $n = 1$, $\vec{p}_B = \frac{2\pi}{L}(-1,0,0)$, $\mu = 1$, sign = 1.0
$t_J/a$

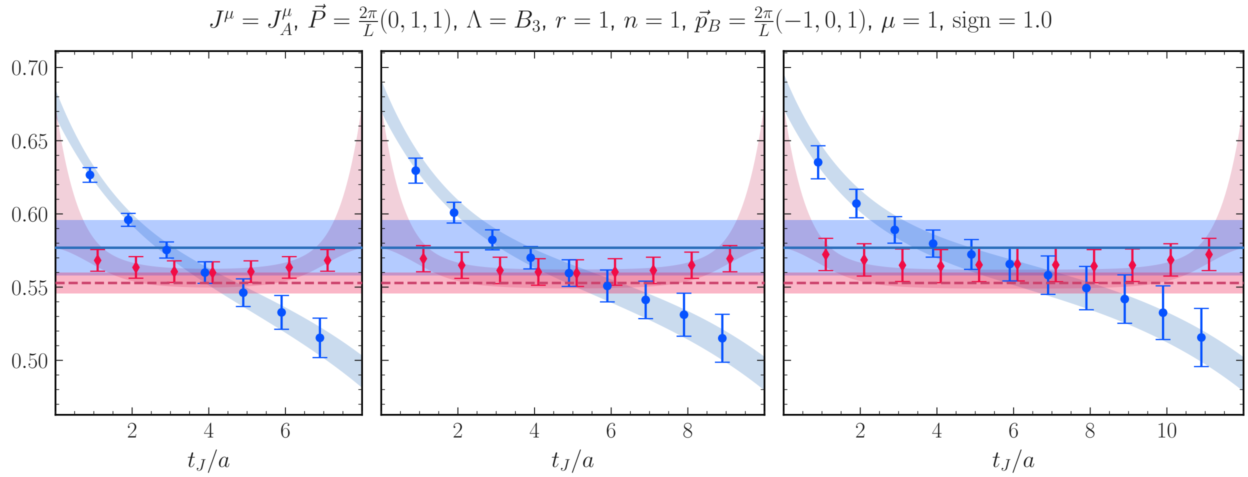
$J^\mu = J^\mu_A$, $\vec{P} = \frac{2\pi}{L}(0,1,1)$, $\Lambda = B_3$, $r = 1$, $n = 1$, $\vec{p}_B = \frac{2\pi}{L}(-1,0,1)$, $\mu = 1$, sign = 1.0
0.70
0.65
0.60
0.55
0.50
2 4 6
2 4 6 8
2 4 6 8 10
$t_J/a$
$t_J/a$
$t_J/a$

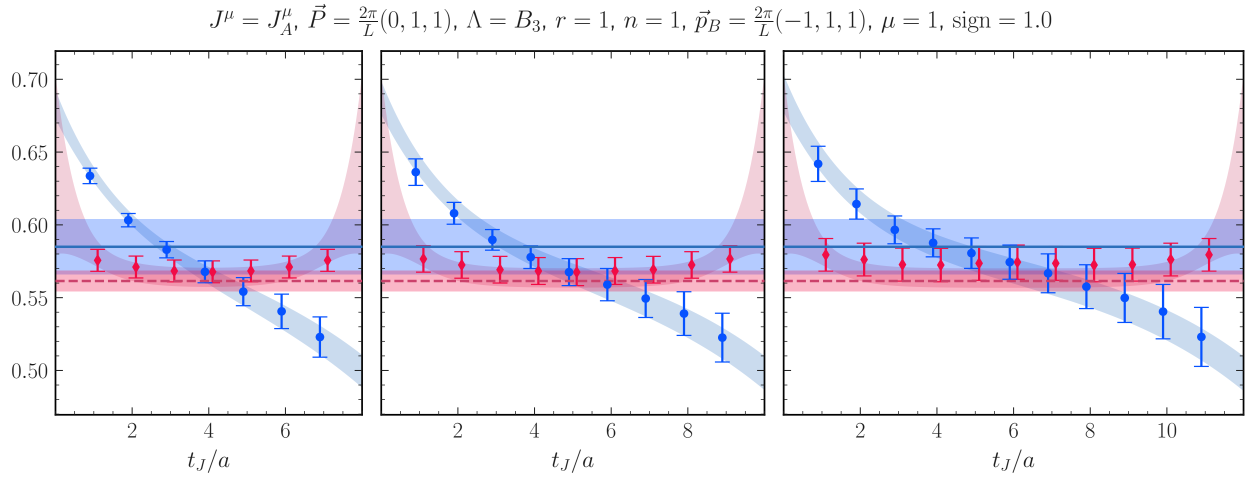
$J^\mu = J^\mu_A$, $\vec{P} = \frac{2\pi}{L}(0,1,1)$, $\Lambda = B_3$, $r = 1$, $n = 1$, $\vec{p}_B = \frac{2\pi}{L}(-1,1,1)$, $\mu = 1$, sign = 1.0
0.70
0.65
0.60
0.55
0.50
2 4 6
2 4 6 8
2 4 6 8 10
$t_J/a$
$t_J/a$
$t_J/a$

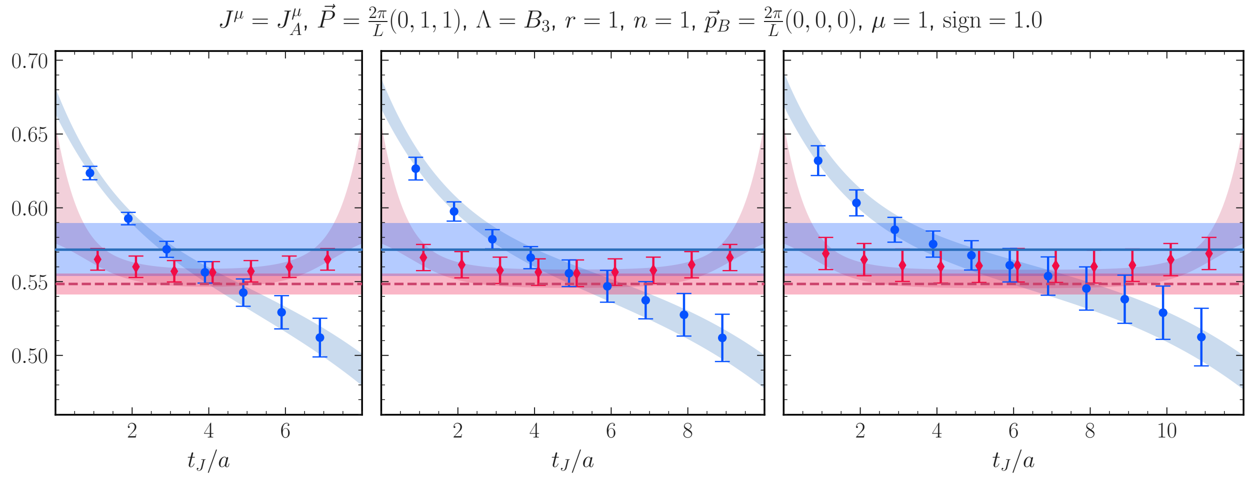
$J^\mu = J^\mu_A$, $\vec{P} = \frac{2\pi}{L}(0,1,1)$, $\Lambda = B_3$, $r = 1$, $n = 1$, $\vec{p}_B = \frac{2\pi}{L}(0,0,0)$, $\mu = 1$, sign = 1.0
0.70
0.65
0.60
0.55
0.50
2 4 6
2 4 6 8
2 4 6 8 10
$t_J/a$
$t_J/a$
$t_J/a$

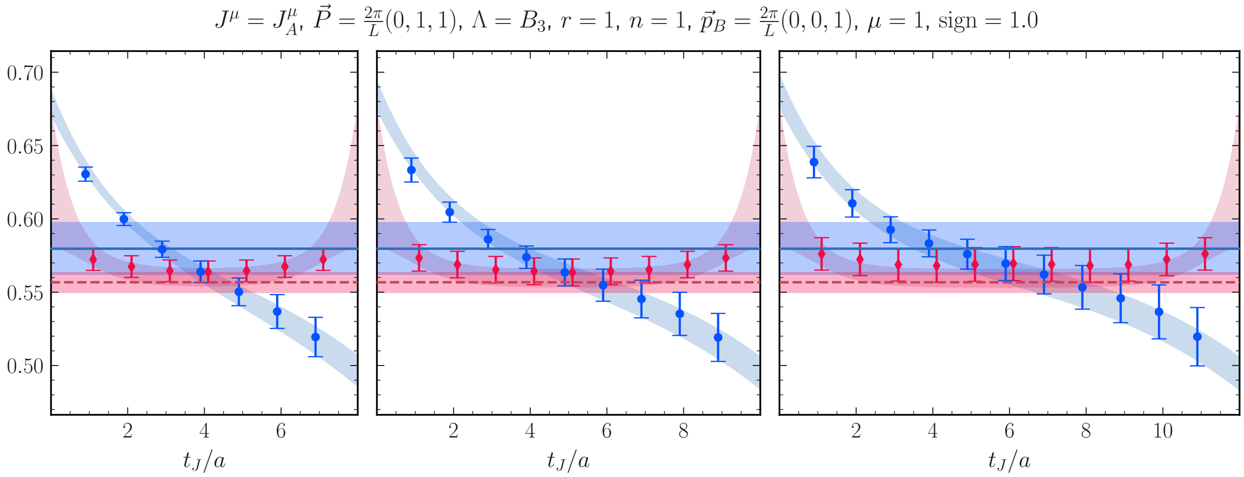
$J^\mu = J_A^\mu$, $\vec{P} = \frac{2\pi}{L}(0,1,1)$, $\Lambda = B_3$, $r = 1$, $n = 1$, $\vec{p}_B = \frac{2\pi}{L}(0,0,1)$, $\mu = 1$, sign = 1.0
0.70
0.65
0.60
0.55
0.50
$t_J/a$
$t_J/a$
$t_J/a$

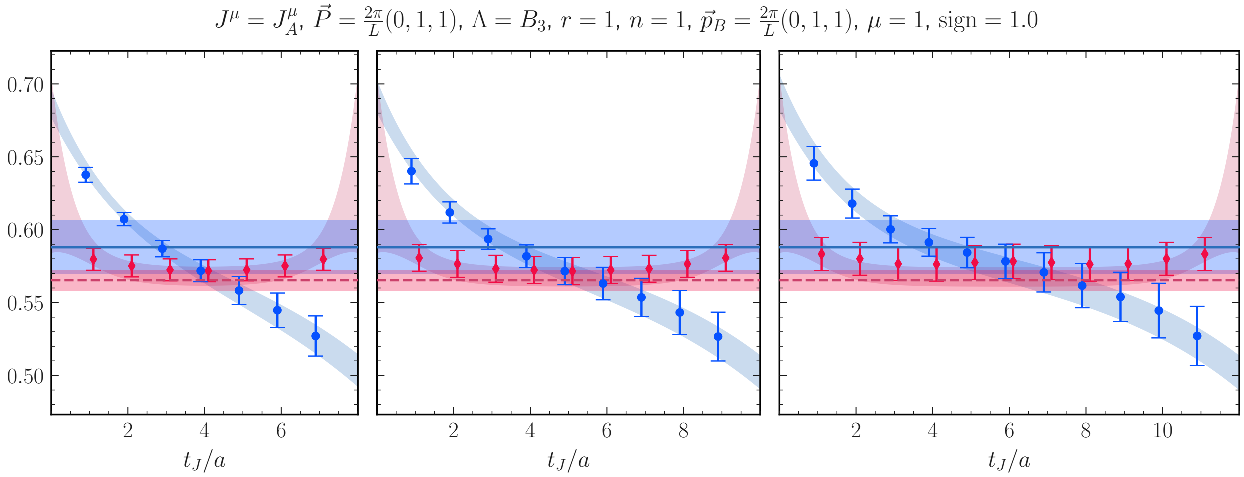
$J^\mu = J_A^\mu$, $\vec{P} = \frac{2\pi}{L}(0,1,1)$, $\Lambda = B_3$, $r = 1$, $n = 1$, $\vec{p}_B = \frac{2\pi}{L}(0,1,1)$, $\mu = 1$, sign = 1.0
0.70
0.65
0.60
0.55
0.50
$t_J/a$
$t_J/a$
$t_J/a$

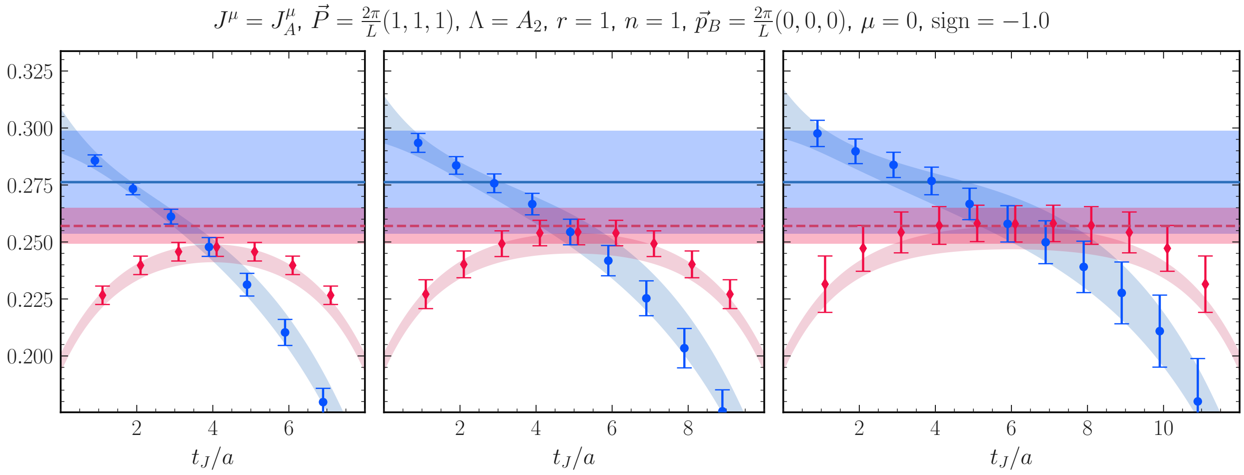
$J^\mu = J_A^\mu$, $\vec{P} = \frac{2\pi}{L}(1,1,1)$, $\Lambda = A_2$, $r = 1$, $n = 1$, $\vec{p}_B = \frac{2\pi}{L}(0,0,0)$, $\mu = 0$, sign = −1.0
0.325
0.300
0.275
0.250
0.225
0.200
$t_J/a$
$t_J/a$
$t_J/a$

$J^\mu = J_A^\mu$, $\vec{P} = \frac{2\pi}{L}(1,1,1)$, $\Lambda = A_2$, $r = 1$, $n = 1$, $\vec{p}_B = \frac{2\pi}{L}(0,0,1)$, $\mu = 0$, sign $= -1.0$

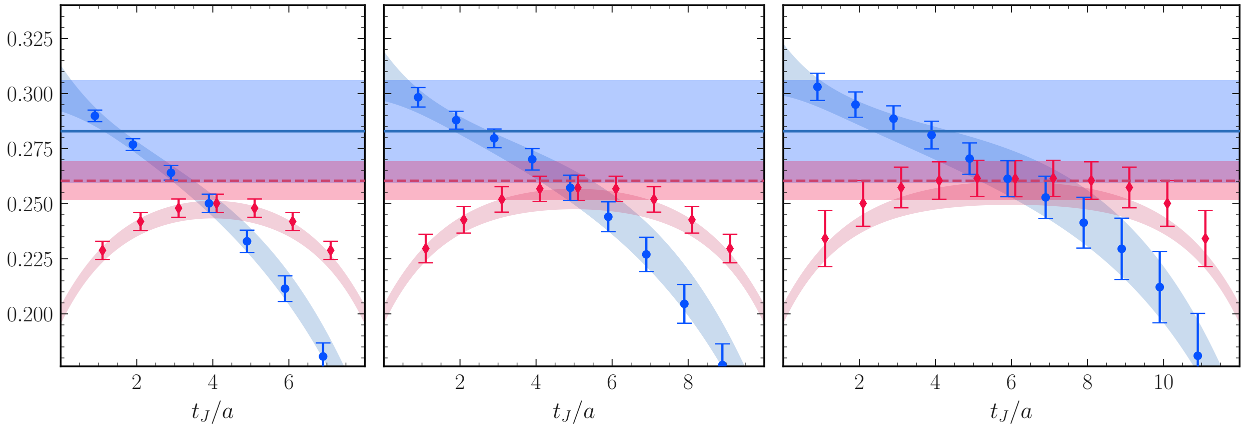


$J^\mu = J_A^\mu$, $\vec{P} = \frac{2\pi}{L}(1,1,1)$, $\Lambda = A_2$, $r = 1$, $n = 1$, $\vec{p}_B = \frac{2\pi}{L}(0,0,1)$, $\mu = 3$, sign $= 1.0$

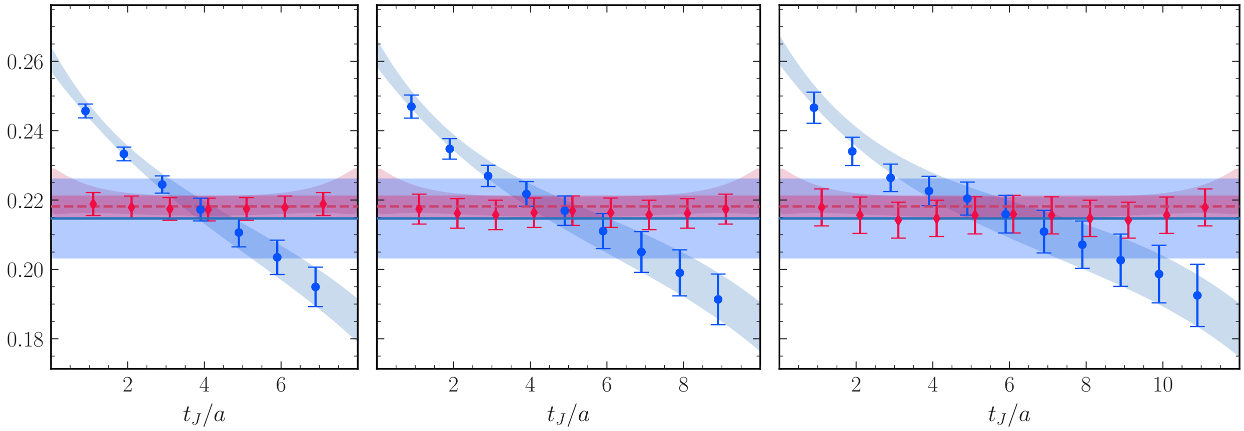


$J^\mu = J_A^\mu$, $\vec{P} = \frac{2\pi}{L}(1,1,1)$, $\Lambda = A_2$, $r = 1$, $n = 1$, $\vec{p}_B = \frac{2\pi}{L}(0,1,1)$, $\mu = 0$, sign $= -1.0$

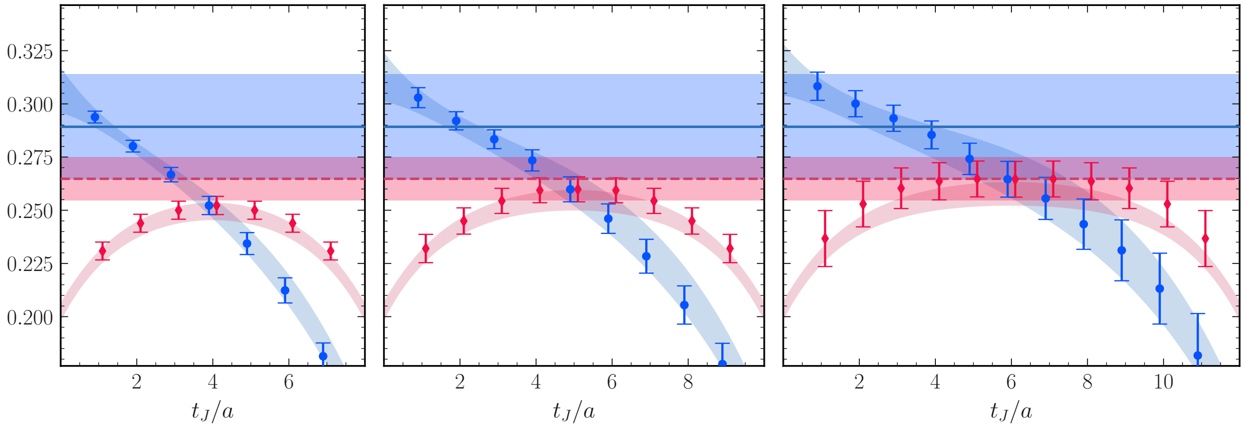

$J^{\mu} = J^{\mu}_{A}$, $\vec{P} = \frac{2\pi}{L}(1,1,1)$, $\Lambda = A_2$, $r = 1$, $n = 1$, $\vec{p}_B = \frac{2\pi}{L}(0,1,1)$, $\mu = 1$, sign $= 1.0$

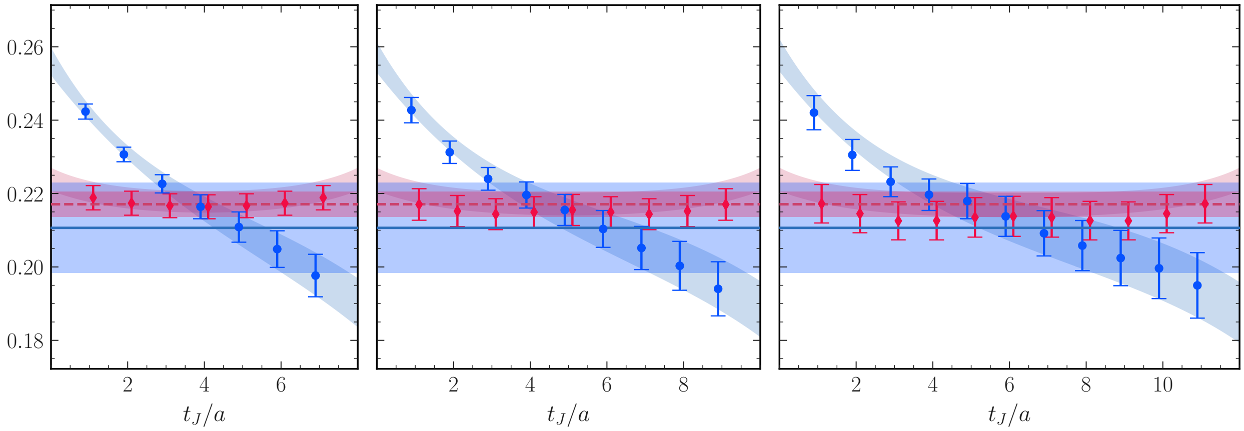


$J^{\mu} = J^{\mu}_{A}$, $\vec{P} = \frac{2\pi}{L}(1,1,1)$, $\Lambda = A_2$, $r = 1$, $n = 1$, $\vec{p}_B = \frac{2\pi}{L}(0,1,1)$, $\mu = 2$, sign $= 1.0$

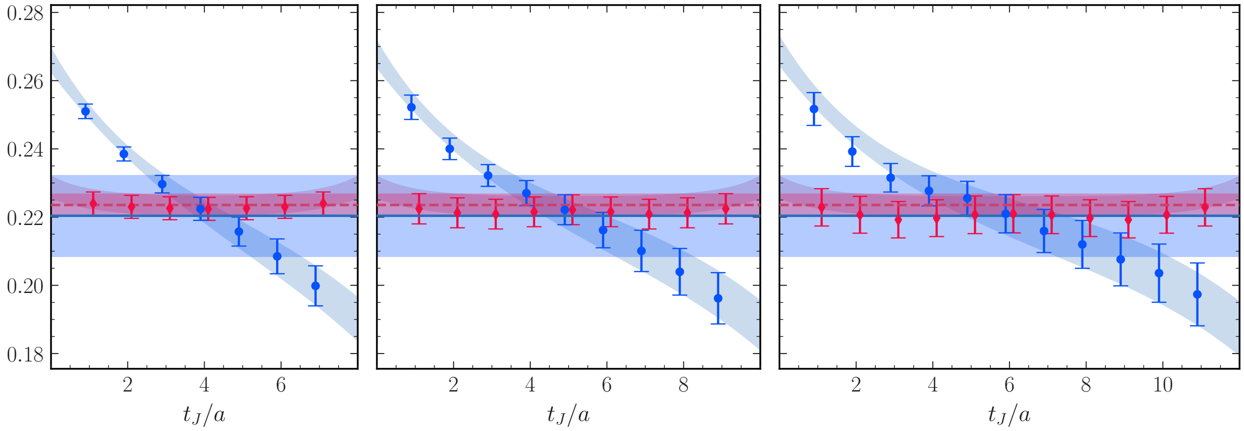


$J^{\mu} = J^{\mu}_{A}$, $\vec{P} = \frac{2\pi}{L}(1,1,1)$, $\Lambda = A_2$, $r = 1$, $n = 1$, $\vec{p}_B = \frac{2\pi}{L}(1,1,1)$, $\mu = 0$, sign $= -1.0$

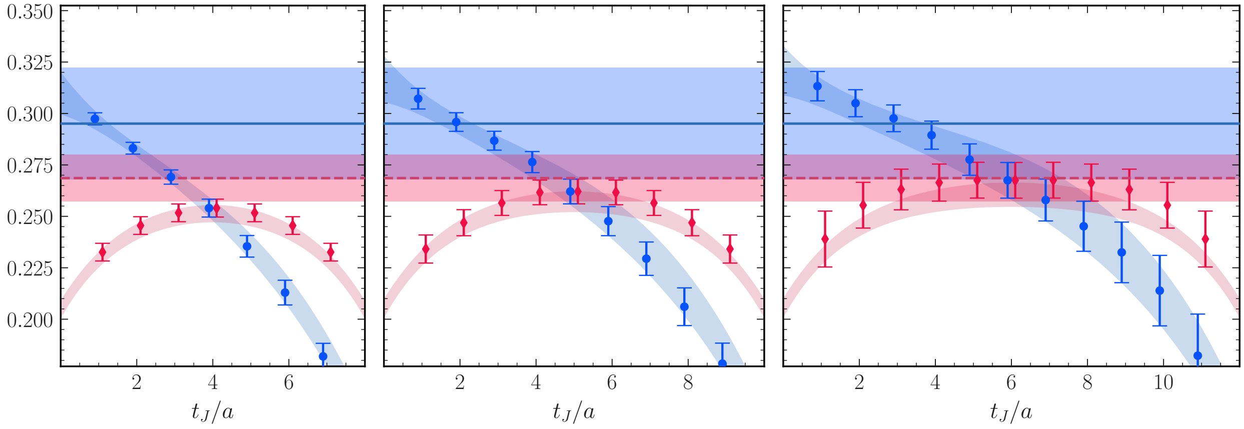

$J^\mu = J^\mu_A$, $\vec{P} = \frac{2\pi}{L}(1,1,1)$, $\Lambda = A_2$, $r = 1$, $n = 2$, $\vec{p}_B = \frac{2\pi}{L}(0,0,0)$, $\mu = 0$, sign $= -1.0$

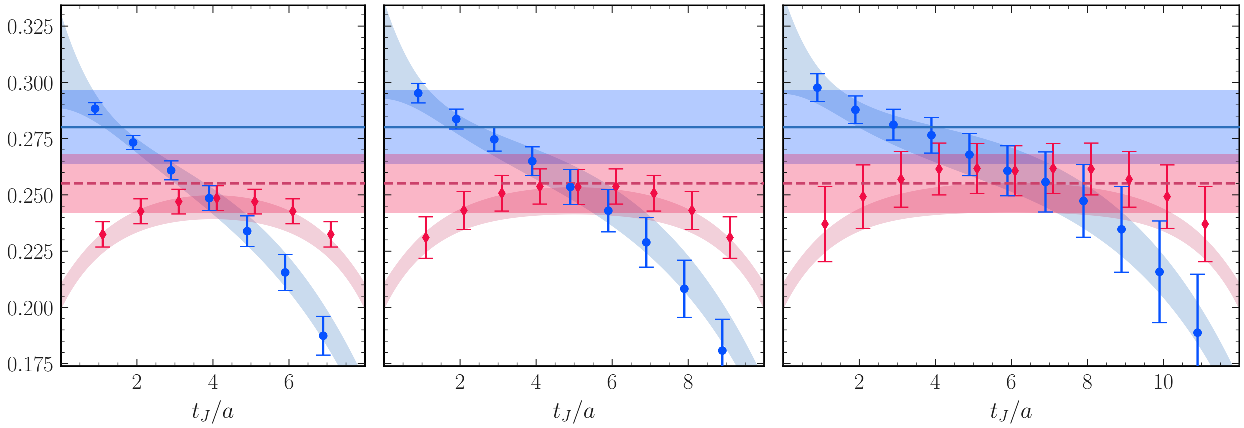


$J^\mu = J^\mu_A$, $\vec{P} = \frac{2\pi}{L}(1,1,1)$, $\Lambda = A_2$, $r = 1$, $n = 2$, $\vec{p}_B = \frac{2\pi}{L}(0,0,0)$, $\mu = 1$, sign $= 1.0$

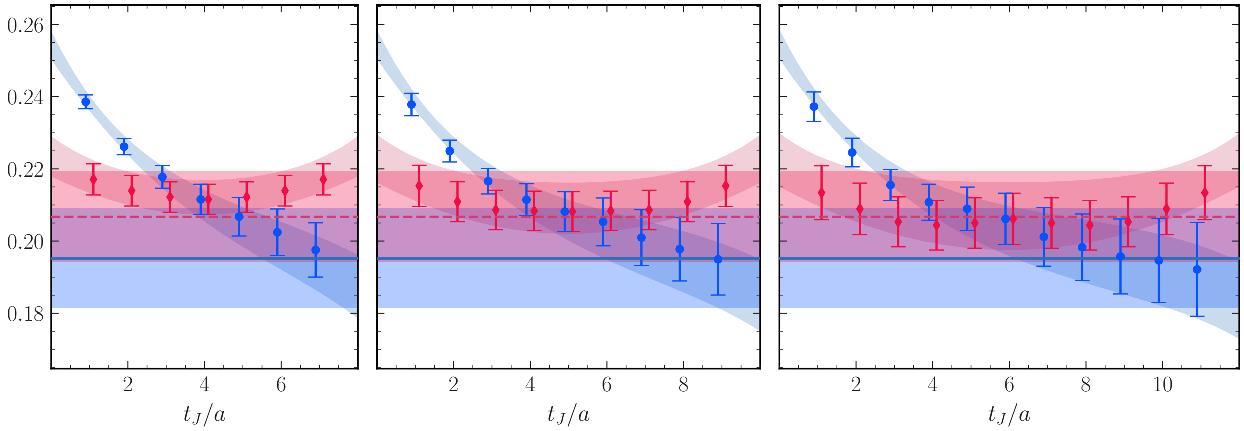


$J^\mu = J^\mu_A$, $\vec{P} = \frac{2\pi}{L}(1,1,1)$, $\Lambda = A_2$, $r = 1$, $n = 2$, $\vec{p}_B = \frac{2\pi}{L}(0,0,1)$, $\mu = 0$, sign $= -1.0$

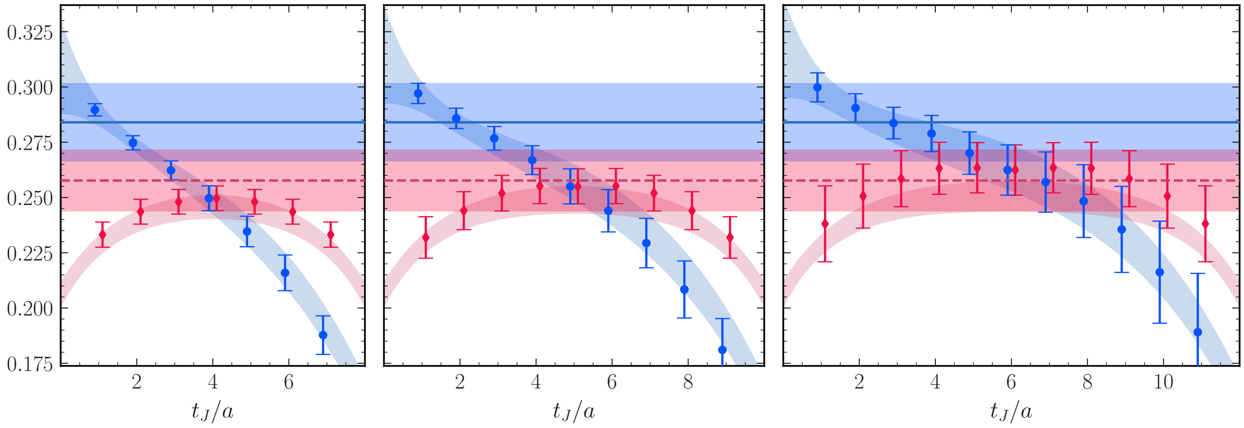

$J^\mu = J_A^\mu$, $\vec{P} = \frac{2\pi}{L}(1,1,1)$, $\Lambda = A_2$, $r = 1$, $n = 2$, $\vec{p}_B = \frac{2\pi}{L}(0,0,1)$, $\mu = 1$, sign $= 1.0$

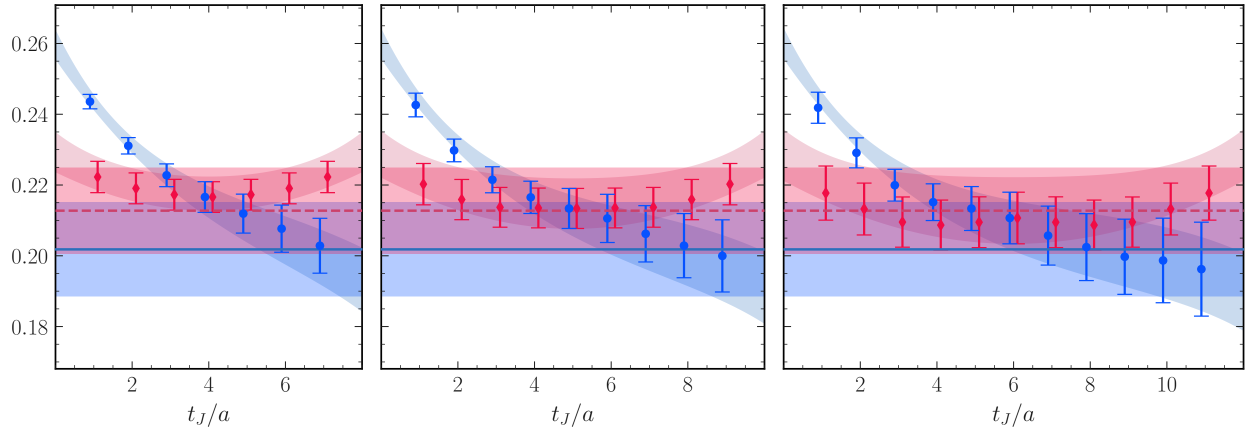


$J^\mu = J_A^\mu$, $\vec{P} = \frac{2\pi}{L}(1,1,1)$, $\Lambda = A_2$, $r = 1$, $n = 2$, $\vec{p}_B = \frac{2\pi}{L}(0,0,1)$, $\mu = 3$, sign $= 1.0$

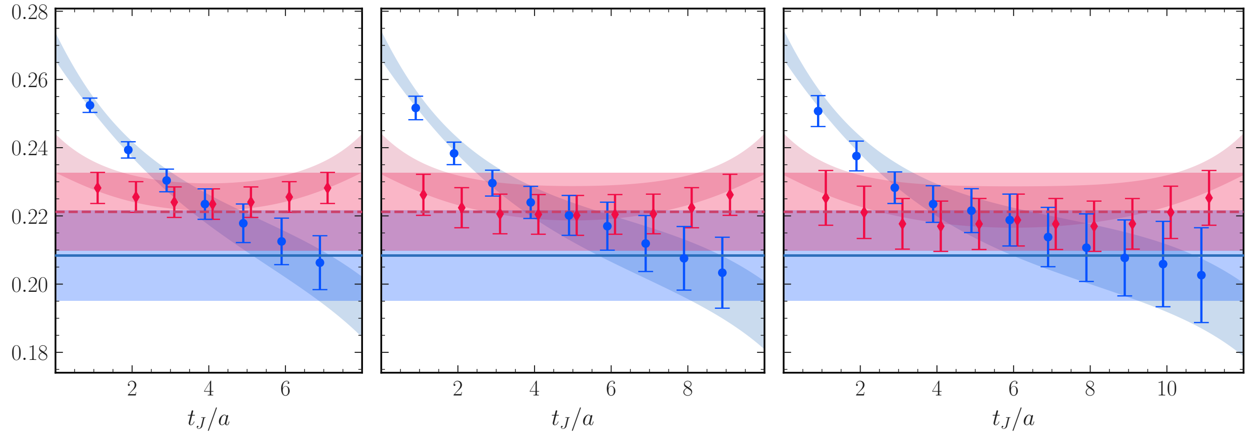


$J^\mu = J_A^\mu$, $\vec{P} = \frac{2\pi}{L}(1,1,1)$, $\Lambda = A_2$, $r = 1$, $n = 2$, $\vec{p}_B = \frac{2\pi}{L}(0,1,1)$, $\mu = 0$, sign $= -1.0$

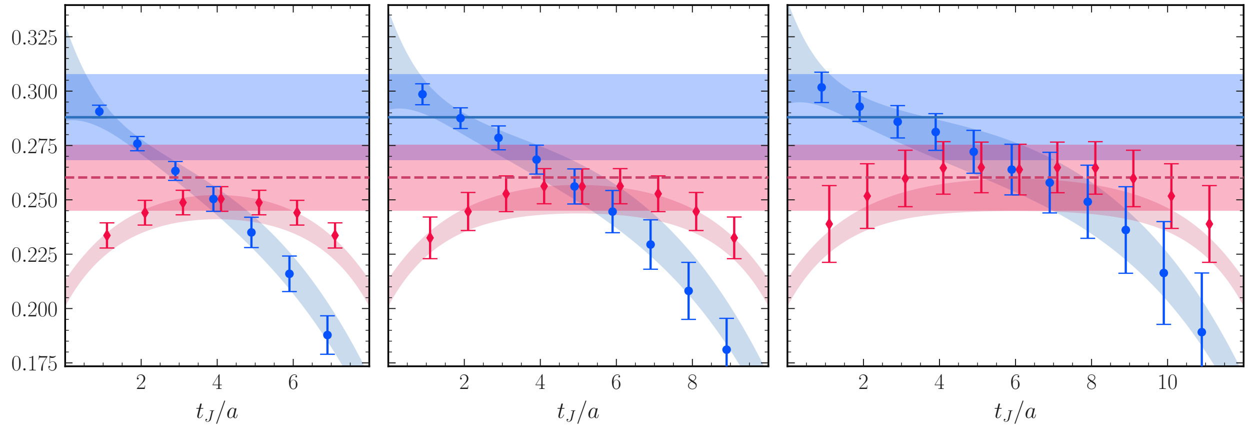

$J^\mu = J_A^\mu$, $\vec{P} = \frac{2\pi}{L}(1,1,1)$, $\Lambda = A_2$, $r = 1$, $n = 2$, $\vec{p}_B = \frac{2\pi}{L}(0,1,1)$, $\mu = 1$, sign $= 1.0$

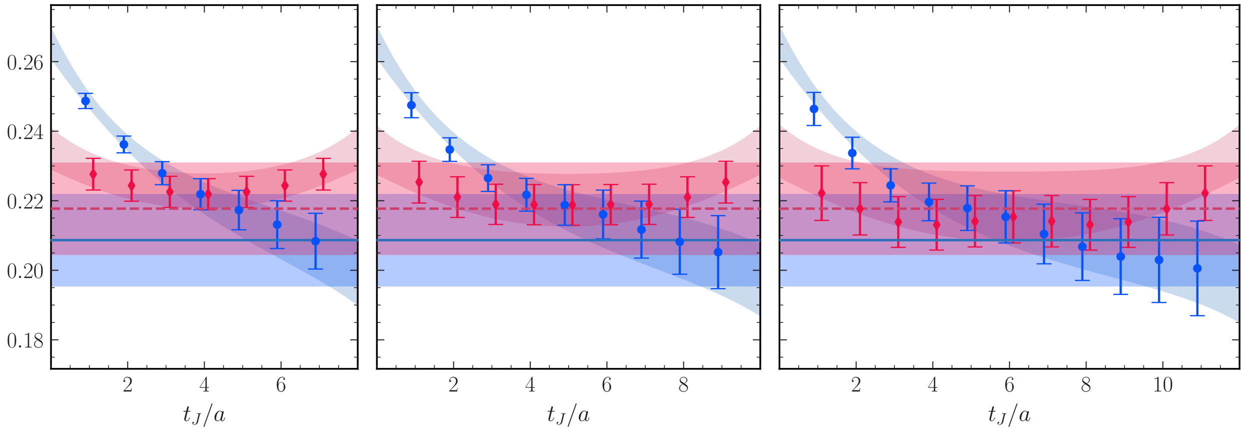


$J^\mu = J_A^\mu$, $\vec{P} = \frac{2\pi}{L}(1,1,1)$, $\Lambda = A_2$, $r = 1$, $n = 2$, $\vec{p}_B = \frac{2\pi}{L}(0,1,1)$, $\mu = 2$, sign $= 1.0$

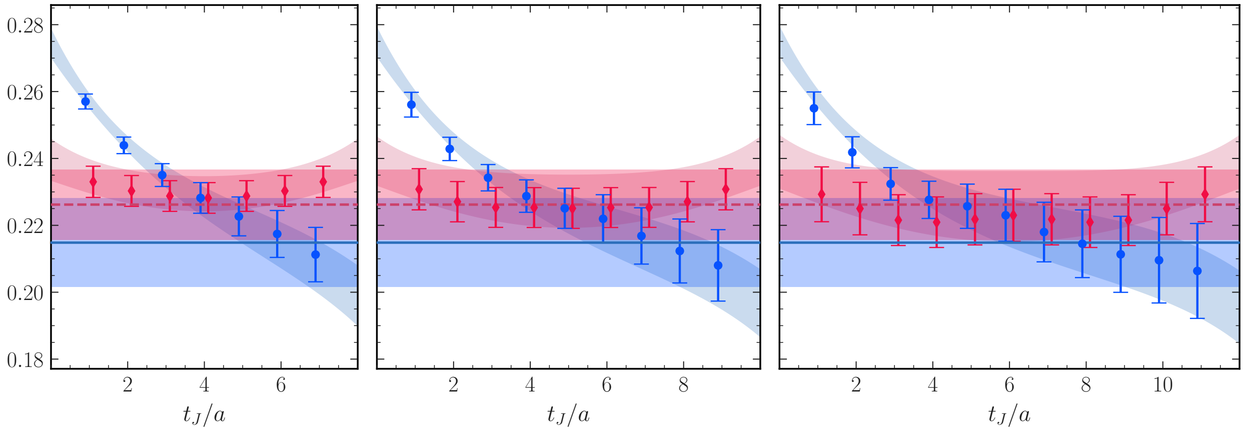


$J^\mu = J_A^\mu$, $\vec{P} = \frac{2\pi}{L}(1,1,1)$, $\Lambda = A_2$, $r = 1$, $n = 2$, $\vec{p}_B = \frac{2\pi}{L}(1,1,1)$, $\mu = 0$, sign $= -1.0$

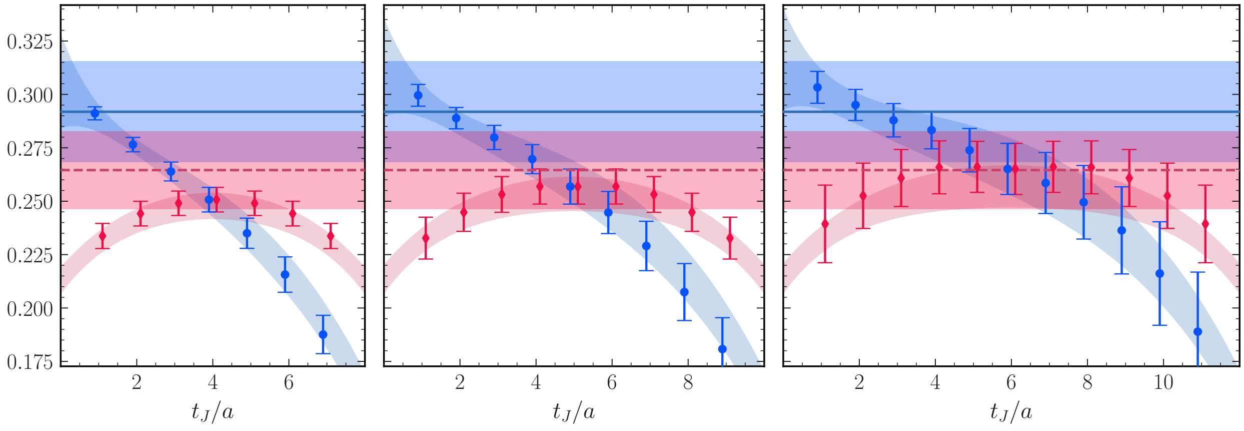

$J^\mu = J^\mu_A$, $\vec{P} = \frac{2\pi}{L}(1,1,1)$, $\Lambda = E$, $r = 1$, $n = 1$, $\vec{p}_B = \frac{2\pi}{L}(0,0,0)$, $\mu = 1$, sign $= 1.0$

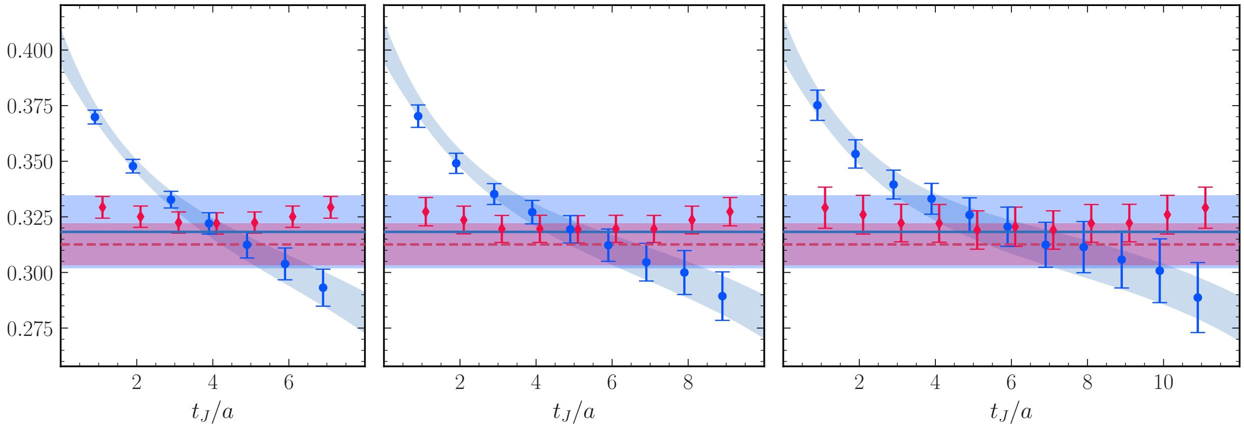


$J^\mu = J^\mu_A$, $\vec{P} = \frac{2\pi}{L}(1,1,1)$, $\Lambda = E$, $r = 1$, $n = 1$, $\vec{p}_B = \frac{2\pi}{L}(0,0,0)$, $\mu = 2$, sign $= -1.0$

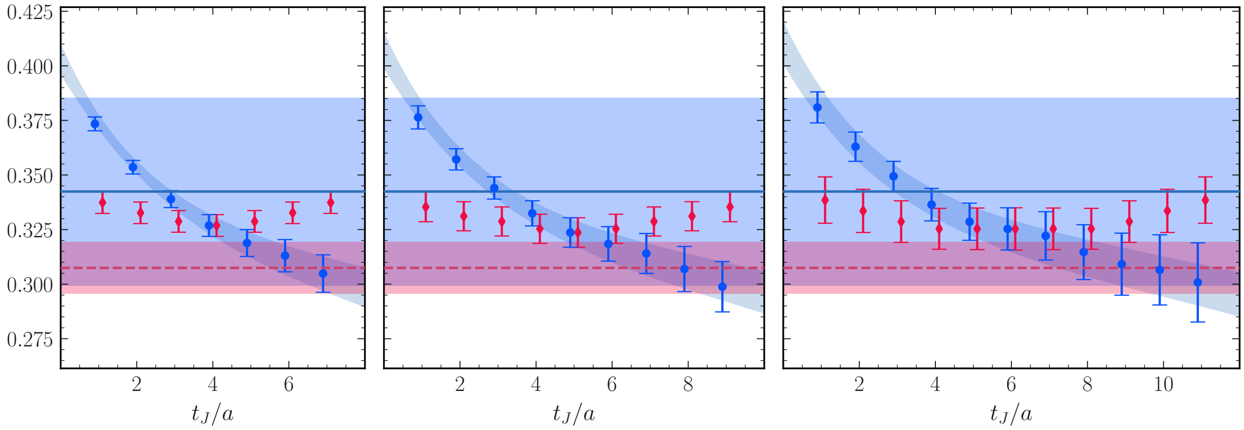


$J^\mu = J^\mu_A$, $\vec{P} = \frac{2\pi}{L}(1,1,1)$, $\Lambda = E$, $r = 1$, $n = 1$, $\vec{p}_B = \frac{2\pi}{L}(0,0,1)$, $\mu = 1$, sign $= 1.0$

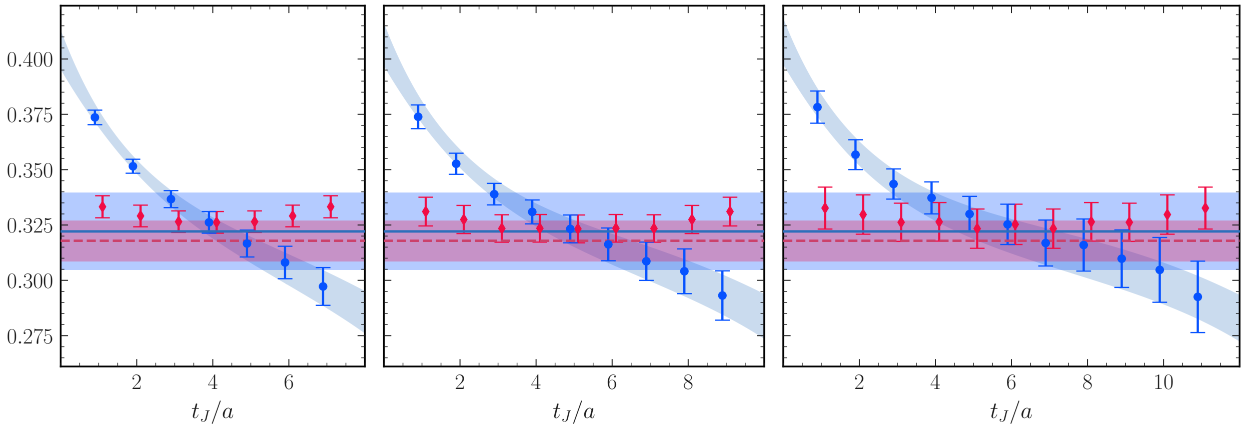

$J^{\mu} = J^{\mu}_{A}$, $\vec{P} = \frac{2\pi}{L}(1,1,1)$, $\Lambda = E$, $r = 1$, $n = 1$, $\vec{p}_B = \frac{2\pi}{L}(0,0,1)$, $\mu = 2$, sign $= -1.0$

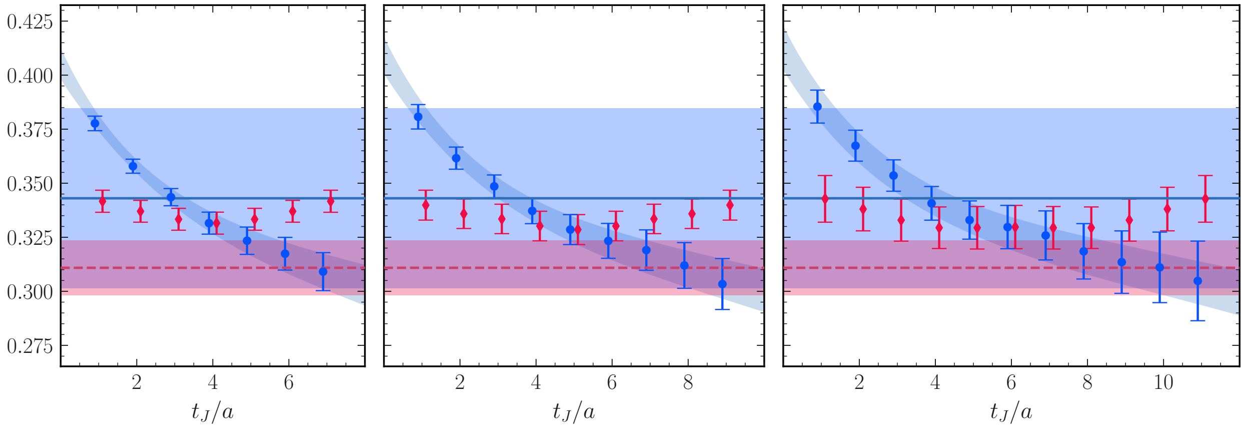


$J^{\mu} = J^{\mu}_{A}$, $\vec{P} = \frac{2\pi}{L}(1,1,1)$, $\Lambda = E$, $r = 1$, $n = 1$, $\vec{p}_B = \frac{2\pi}{L}(0,1,0)$, $\mu = 1$, sign $= 1.0$

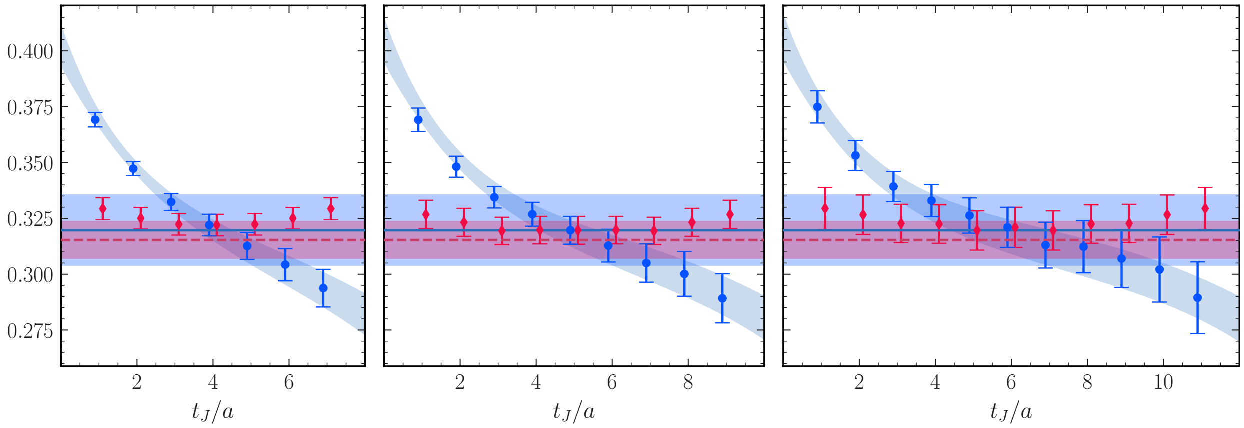


$J^{\mu} = J^{\mu}_{A}$, $\vec{P} = \frac{2\pi}{L}(1,1,1)$, $\Lambda = E$, $r = 1$, $n = 1$, $\vec{p}_B = \frac{2\pi}{L}(0,1,0)$, $\mu = 2$, sign $= -1.0$

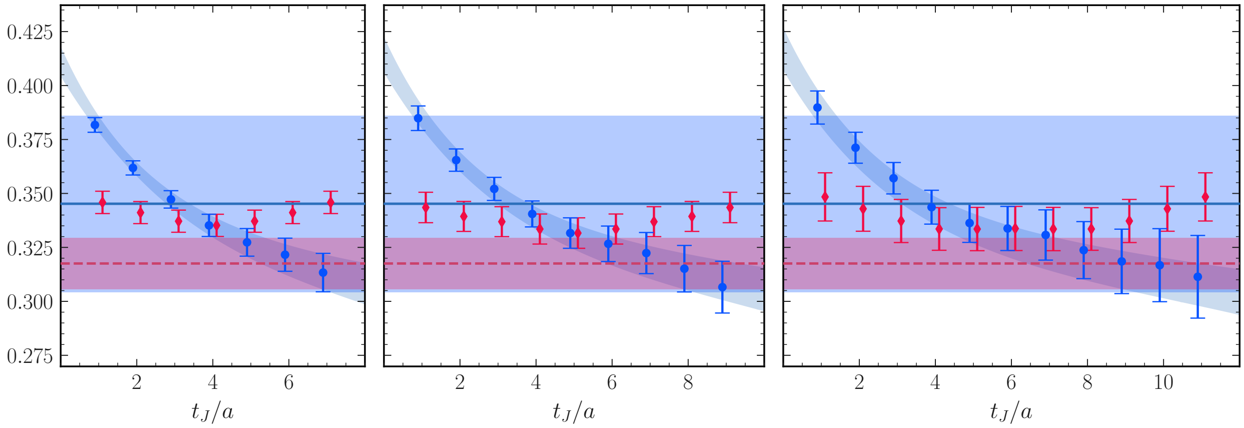

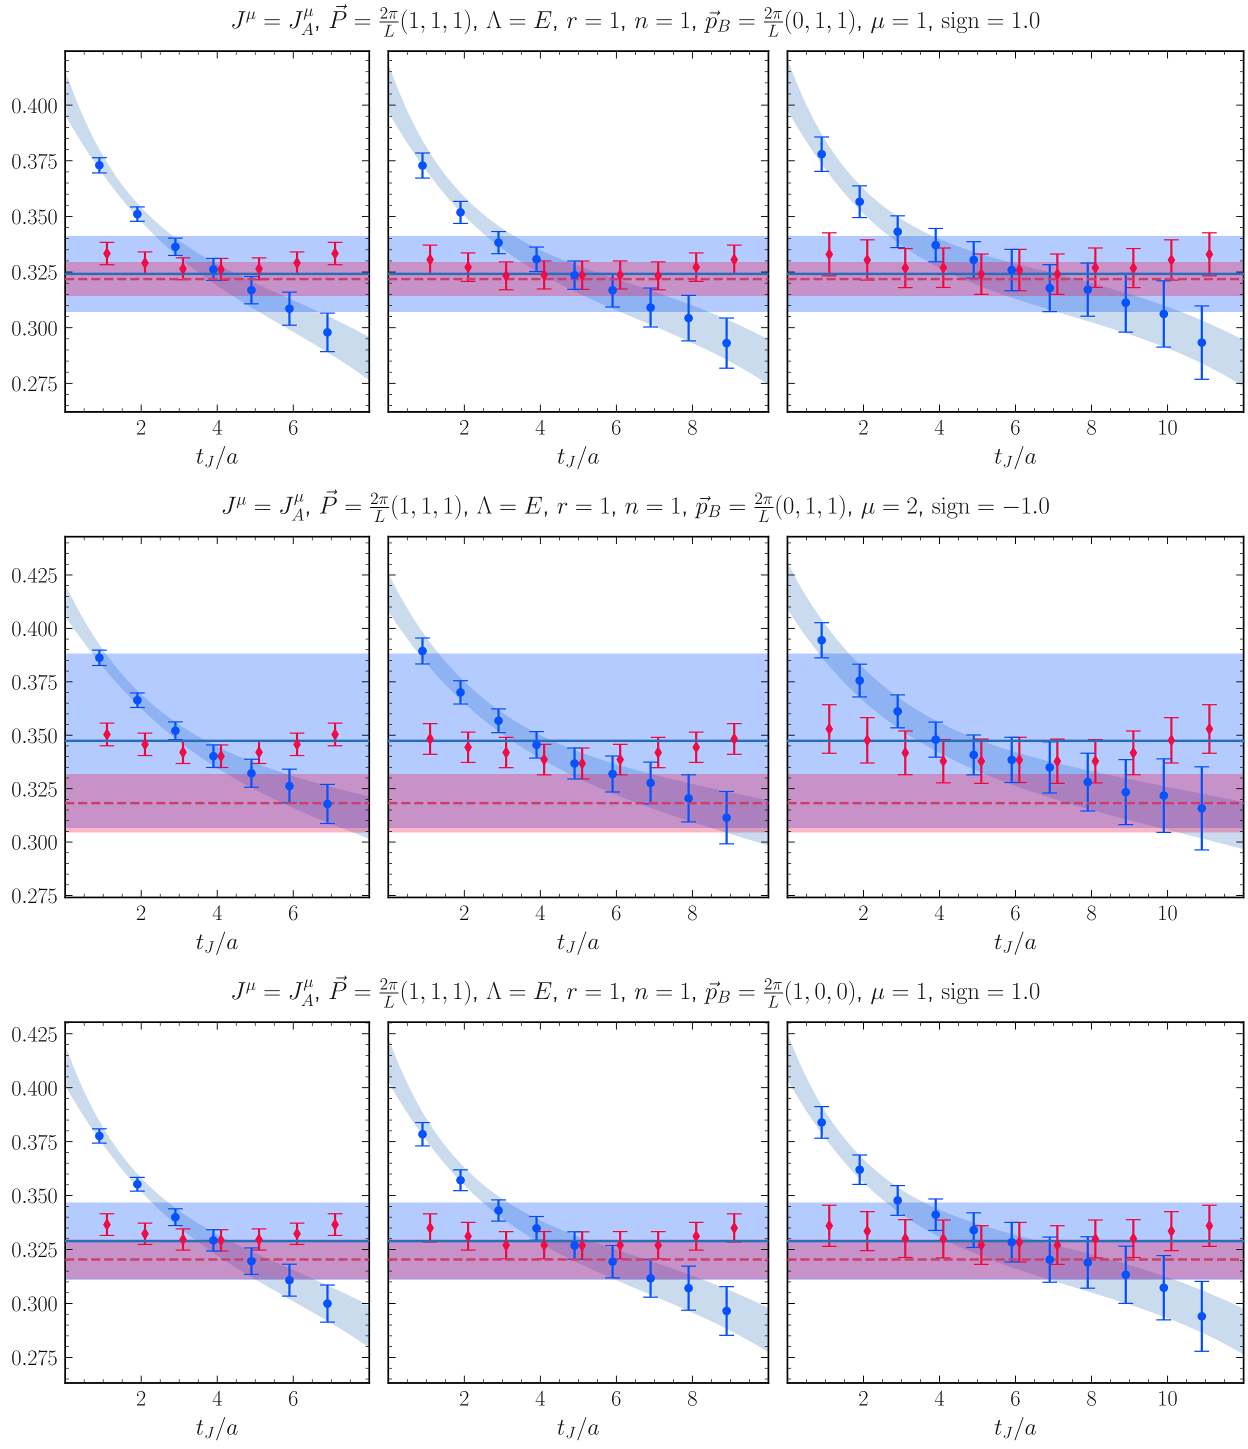

$J^\mu = J^\mu_A$, $\vec{P} = \frac{2\pi}{L}(1,1,1)$, $\Lambda = E$, $r = 1$, $n = 1$, $\vec{p}_B = \frac{2\pi}{L}(0,1,1)$, $\mu = 1$, sign = 1.0
0.400
0.375
0.350
0.325
0.300
0.275
2
4
6
8
10
$t_J/a$
$J^\mu = J^\mu_A$, $\vec{P} = \frac{2\pi}{L}(1,1,1)$, $\Lambda = E$, $r = 1$, $n = 1$, $\vec{p}_B = \frac{2\pi}{L}(0,1,1)$, $\mu = 2$, sign = −1.0
0.425
$J^\mu = J^\mu_A$, $\vec{P} = \frac{2\pi}{L}(1,1,1)$, $\Lambda = E$, $r = 1$, $n = 1$, $\vec{p}_B = \frac{2\pi}{L}(1,0,0)$, $\mu = 1$, sign = 1.0

$J^\mu = J_A^\mu$, $\vec{P} = \frac{2\pi}{L}(1,1,1)$, $\Lambda = E$, $r = 1$, $n = 1$, $\vec{p}_B = \frac{2\pi}{L}(1,0,0)$, $\mu = 2$, sign $= -1.0$

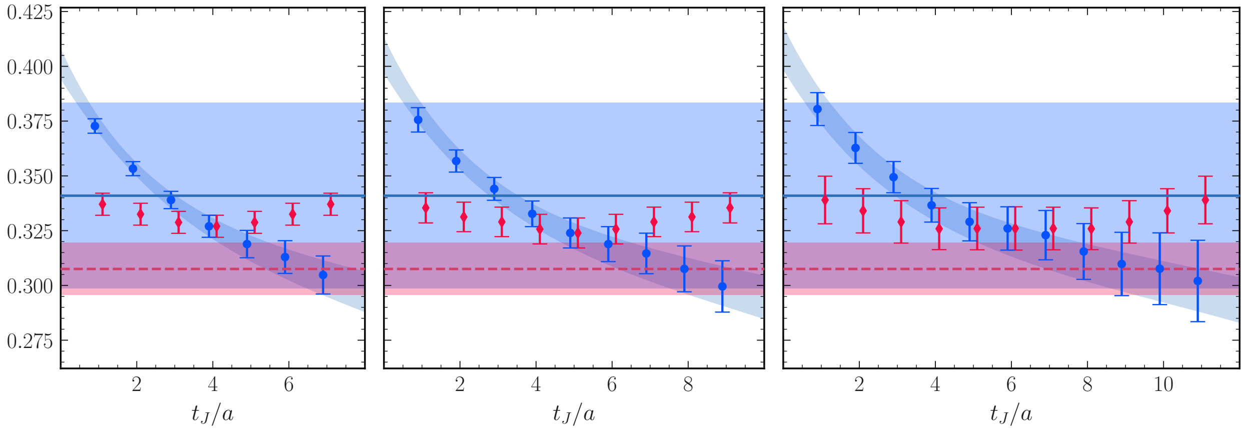


$J^\mu = J_A^\mu$, $\vec{P} = \frac{2\pi}{L}(1,1,1)$, $\Lambda = E$, $r = 1$, $n = 1$, $\vec{p}_B = \frac{2\pi}{L}(1,0,1)$, $\mu = 1$, sign $= 1.0$

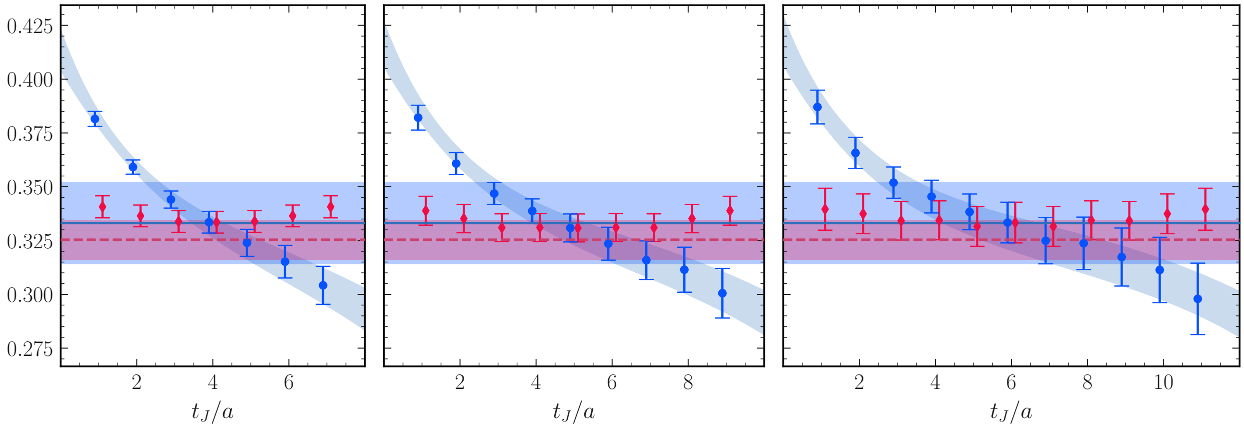


$J^\mu = J_A^\mu$, $\vec{P} = \frac{2\pi}{L}(1,1,1)$, $\Lambda = E$, $r = 1$, $n = 1$, $\vec{p}_B = \frac{2\pi}{L}(1,0,1)$, $\mu = 2$, sign $= -1.0$

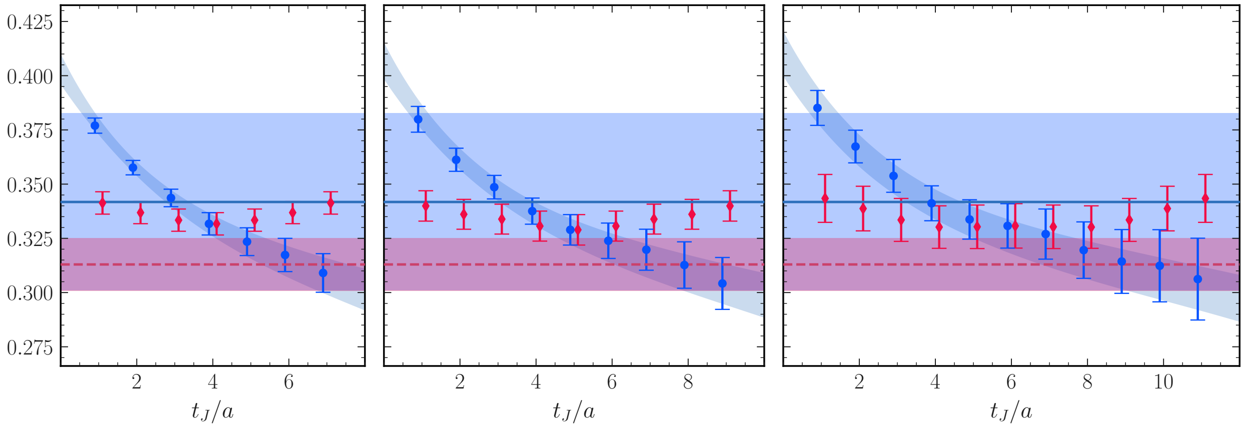

$J^\mu = J_A^\mu$, $\vec{P} = \frac{2\pi}{L}(1,1,1)$, $\Lambda = E$, $r = 1$, $n = 1$, $\vec{p}_B = \frac{2\pi}{L}(1,1,0)$, $\mu = 1$, sign $= 1.0$

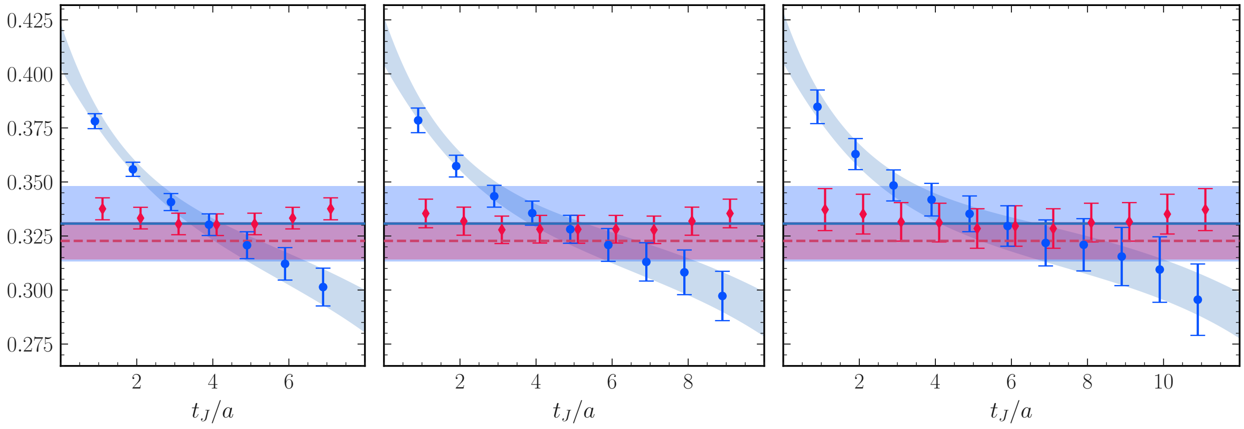


$J^\mu = J_A^\mu$, $\vec{P} = \frac{2\pi}{L}(1,1,1)$, $\Lambda = E$, $r = 1$, $n = 1$, $\vec{p}_B = \frac{2\pi}{L}(1,1,0)$, $\mu = 2$, sign $= -1.0$

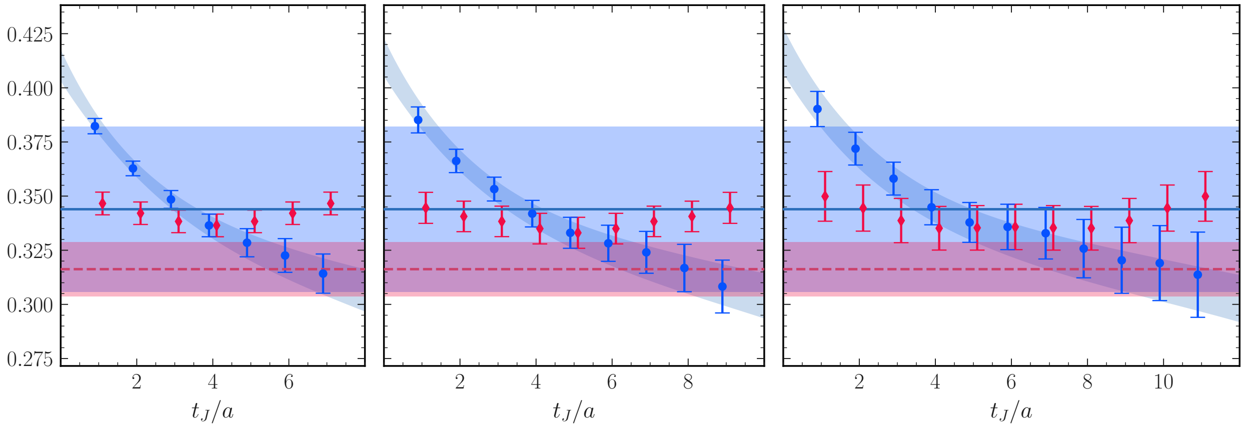


$J^\mu = J_A^\mu$, $\vec{P} = \frac{2\pi}{L}(1,1,1)$, $\Lambda = E$, $r = 1$, $n = 1$, $\vec{p}_B = \frac{2\pi}{L}(1,1,1)$, $\mu = 1$, sign $= 1.0$

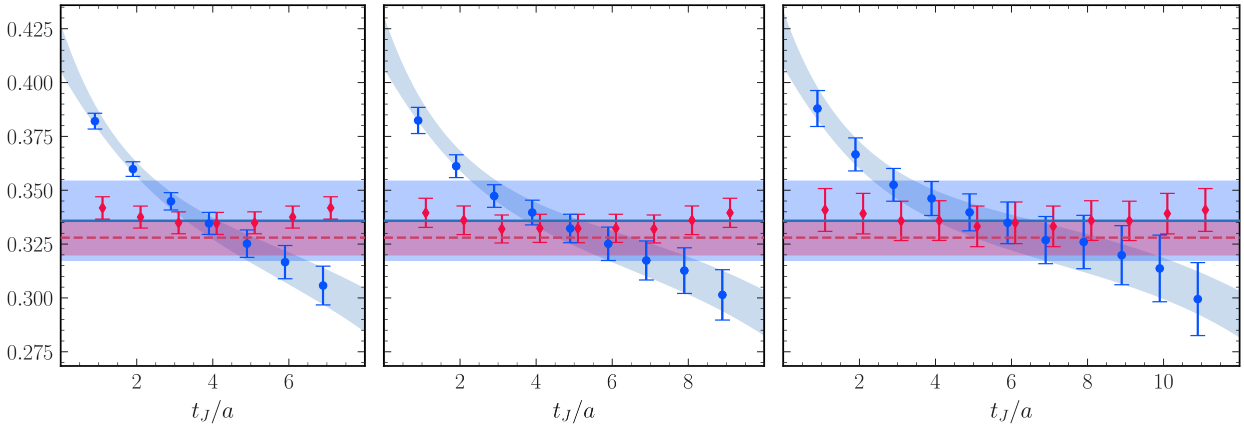

$J^\mu = J_A^\mu,\ \vec{P} = \frac{2\pi}{L}(1,1,1),\ \Lambda = E,\ r = 1,\ n = 1,\ \vec{p}_B = \frac{2\pi}{L}(1,1,1),\ \mu = 2,\ \text{sign} = -1.0$

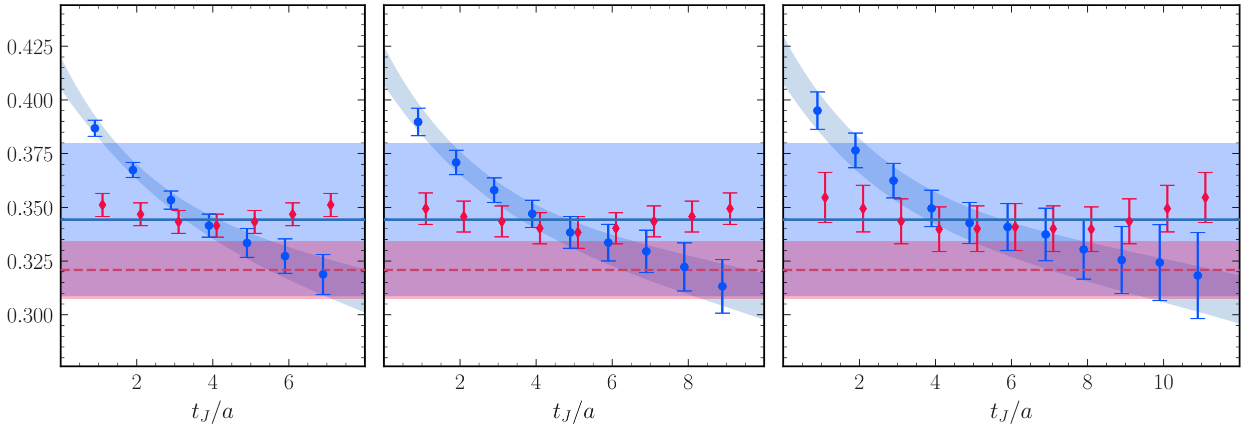


$J^\mu = J_A^\mu,\ \vec{P} = \frac{2\pi}{L}(1,1,1),\ \Lambda = E,\ r = 1,\ n = 2,\ \vec{p}_B = \frac{2\pi}{L}(0,0,0),\ \mu = 1,\ \text{sign} = 1.0$

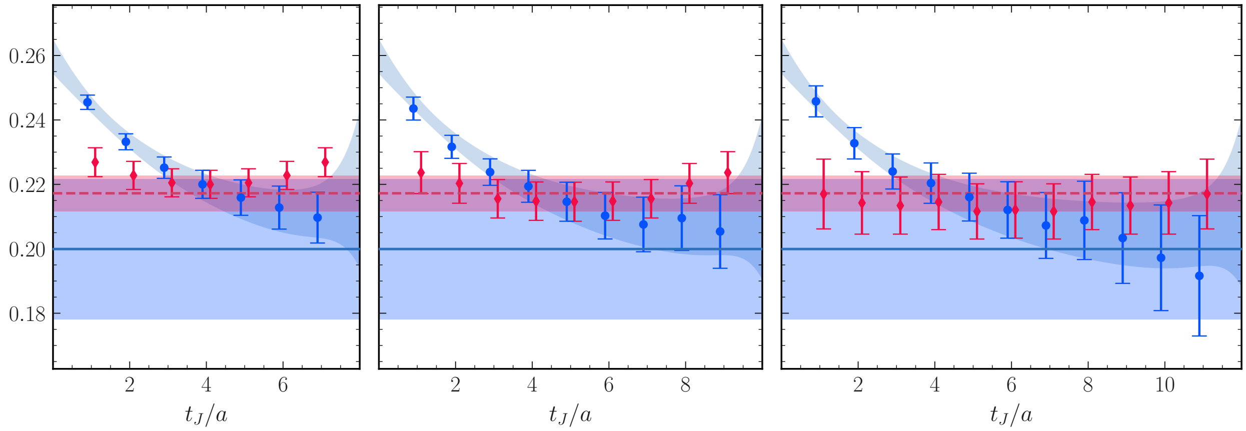


$J^\mu = J_A^\mu,\ \vec{P} = \frac{2\pi}{L}(1,1,1),\ \Lambda = E,\ r = 1,\ n = 2,\ \vec{p}_B = \frac{2\pi}{L}(0,0,0),\ \mu = 2,\ \text{sign} = -1.0$

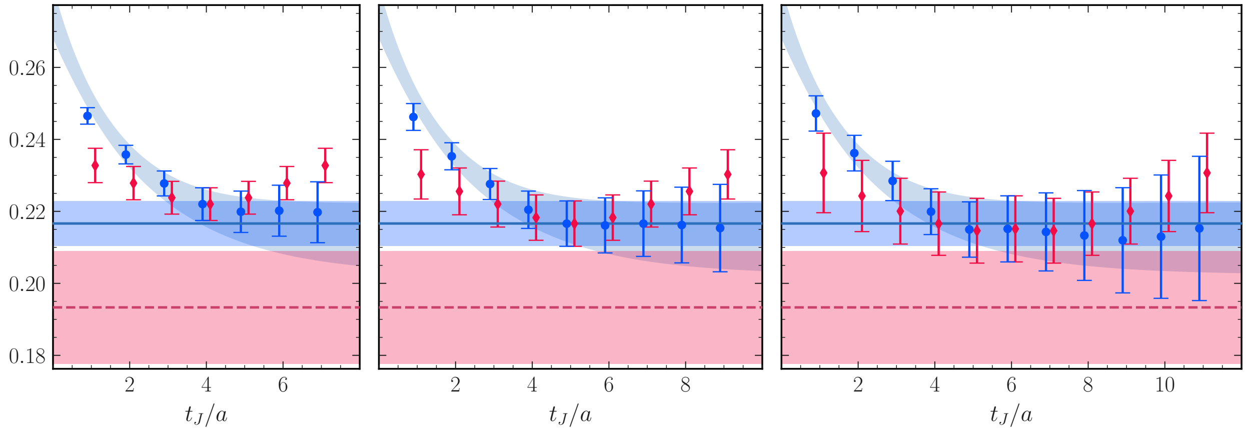

$J^\mu = J_A^\mu$, $\vec{P} = \frac{2\pi}{L}(1,1,1)$, $\Lambda = E$, $r = 1$, $n = 2$, $\vec{p}_B = \frac{2\pi}{L}(0,0,1)$, $\mu = 1$, sign $= 1.0$

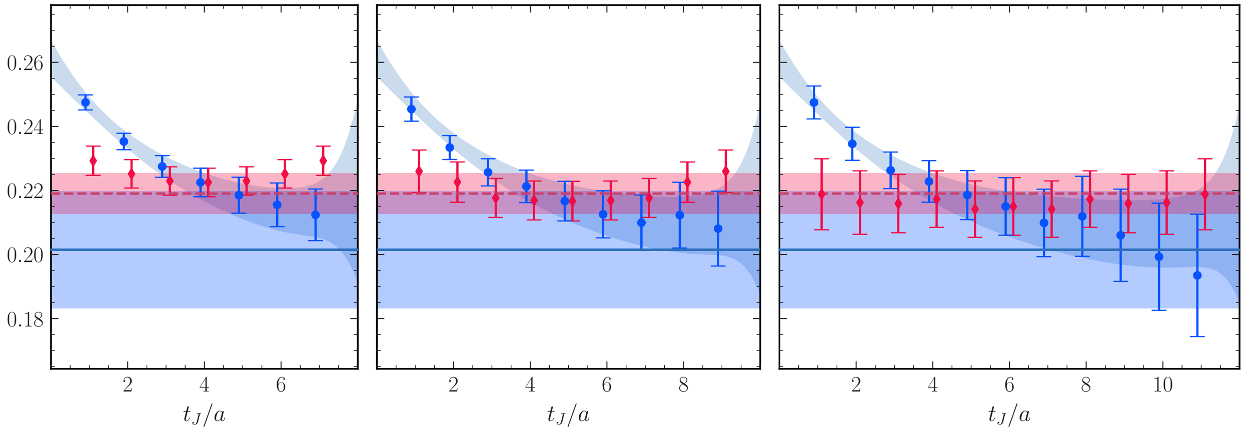


$J^\mu = J_A^\mu$, $\vec{P} = \frac{2\pi}{L}(1,1,1)$, $\Lambda = E$, $r = 1$, $n = 2$, $\vec{p}_B = \frac{2\pi}{L}(0,0,1)$, $\mu = 2$, sign $= -1.0$

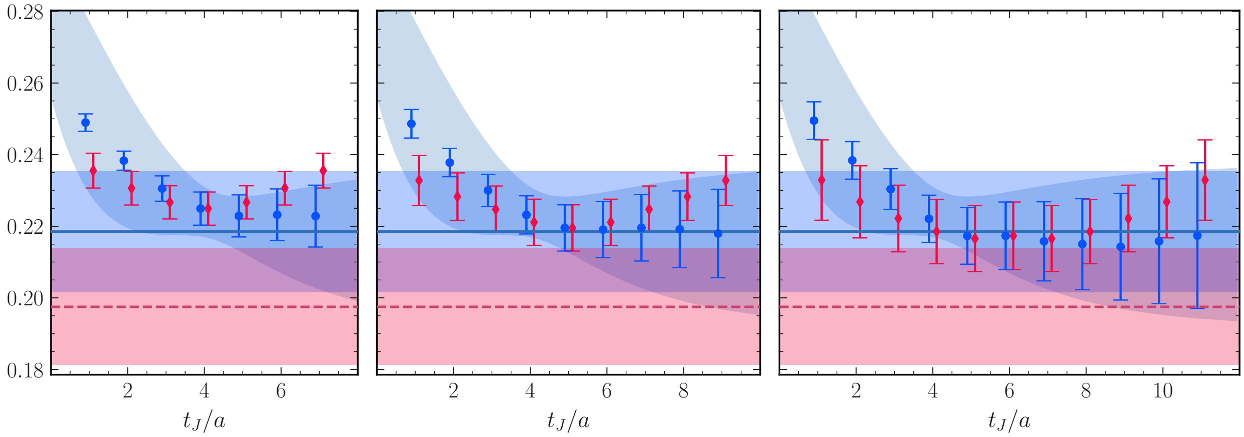


$J^\mu = J_A^\mu$, $\vec{P} = \frac{2\pi}{L}(1,1,1)$, $\Lambda = E$, $r = 1$, $n = 2$, $\vec{p}_B = \frac{2\pi}{L}(0,1,0)$, $\mu = 1$, sign $= 1.0$

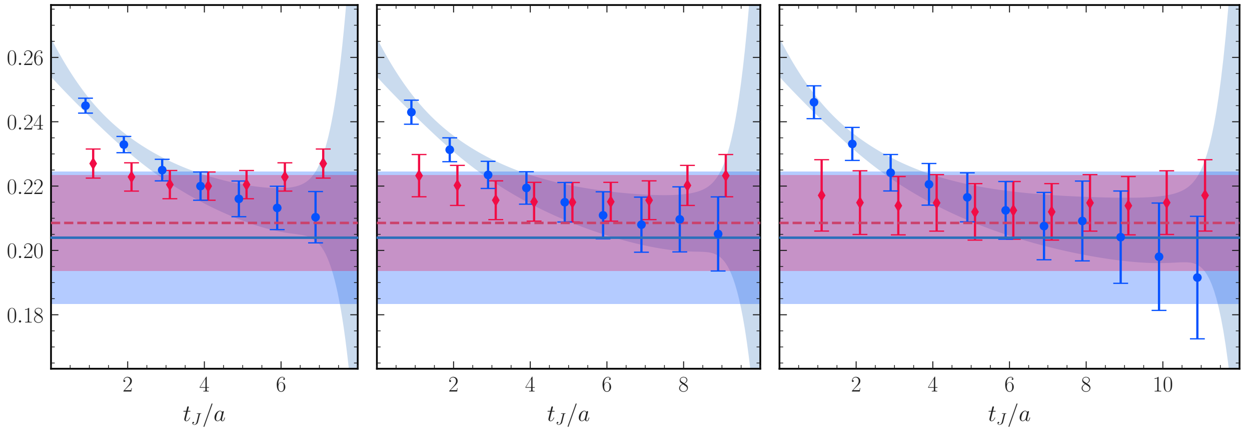

$J^\mu = J_A^\mu$, $\vec{P} = \frac{2\pi}{L}(1,1,1)$, $\Lambda = E$, $r = 1$, $n = 2$, $\vec{p}_B = \frac{2\pi}{L}(0,1,0)$, $\mu = 2$, sign $= -1.0$

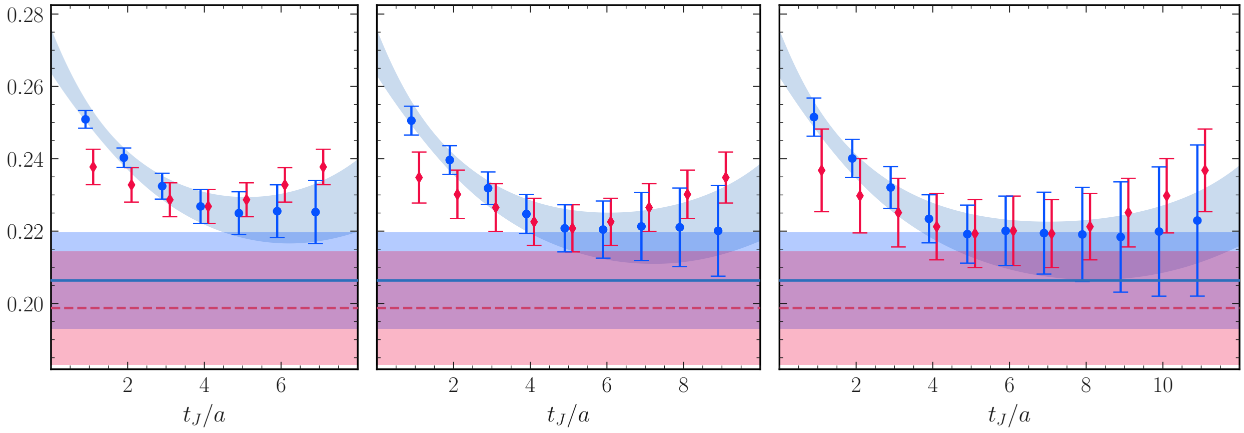


$J^\mu = J_A^\mu$, $\vec{P} = \frac{2\pi}{L}(1,1,1)$, $\Lambda = E$, $r = 1$, $n = 2$, $\vec{p}_B = \frac{2\pi}{L}(0,1,1)$, $\mu = 1$, sign $= 1.0$

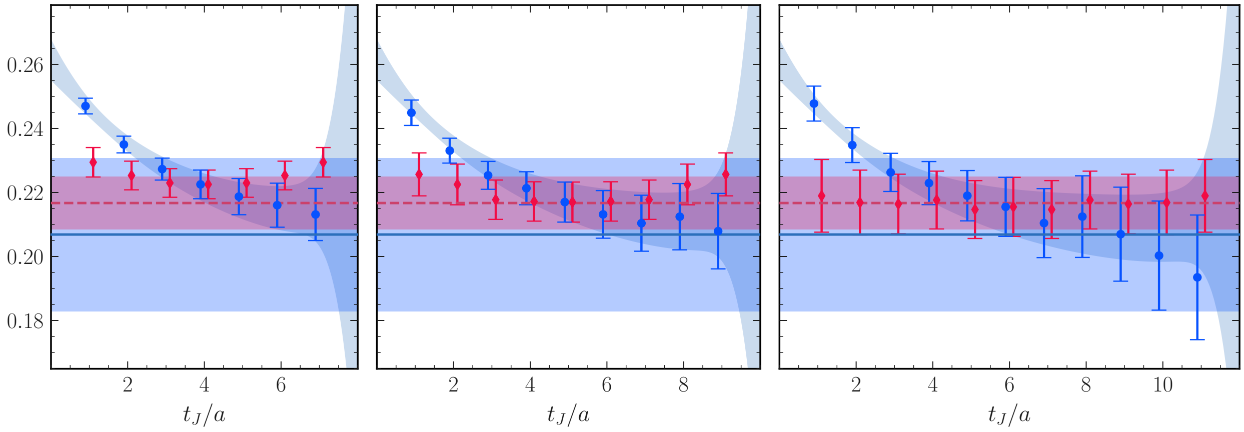


$J^\mu = J_A^\mu$, $\vec{P} = \frac{2\pi}{L}(1,1,1)$, $\Lambda = E$, $r = 1$, $n = 2$, $\vec{p}_B = \frac{2\pi}{L}(0,1,1)$, $\mu = 2$, sign $= -1.0$

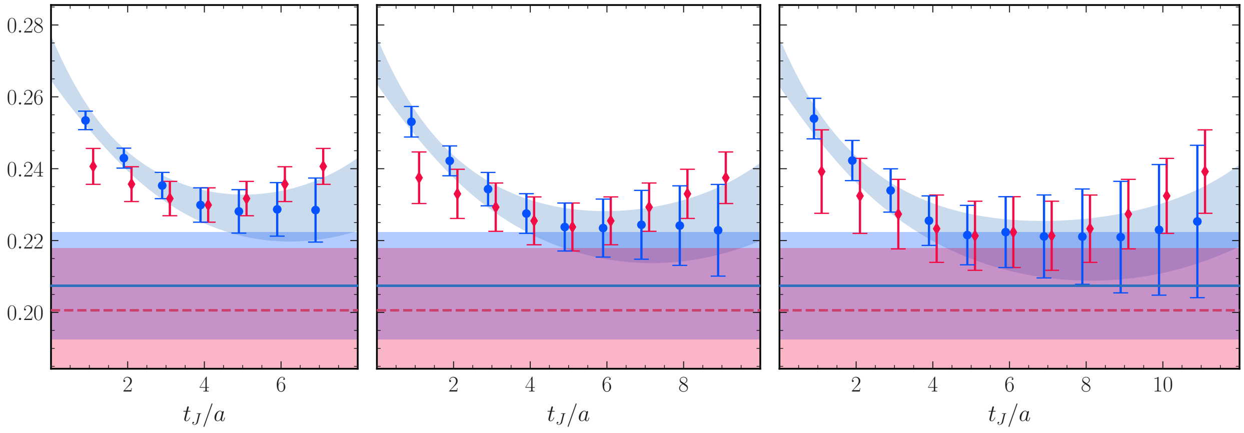

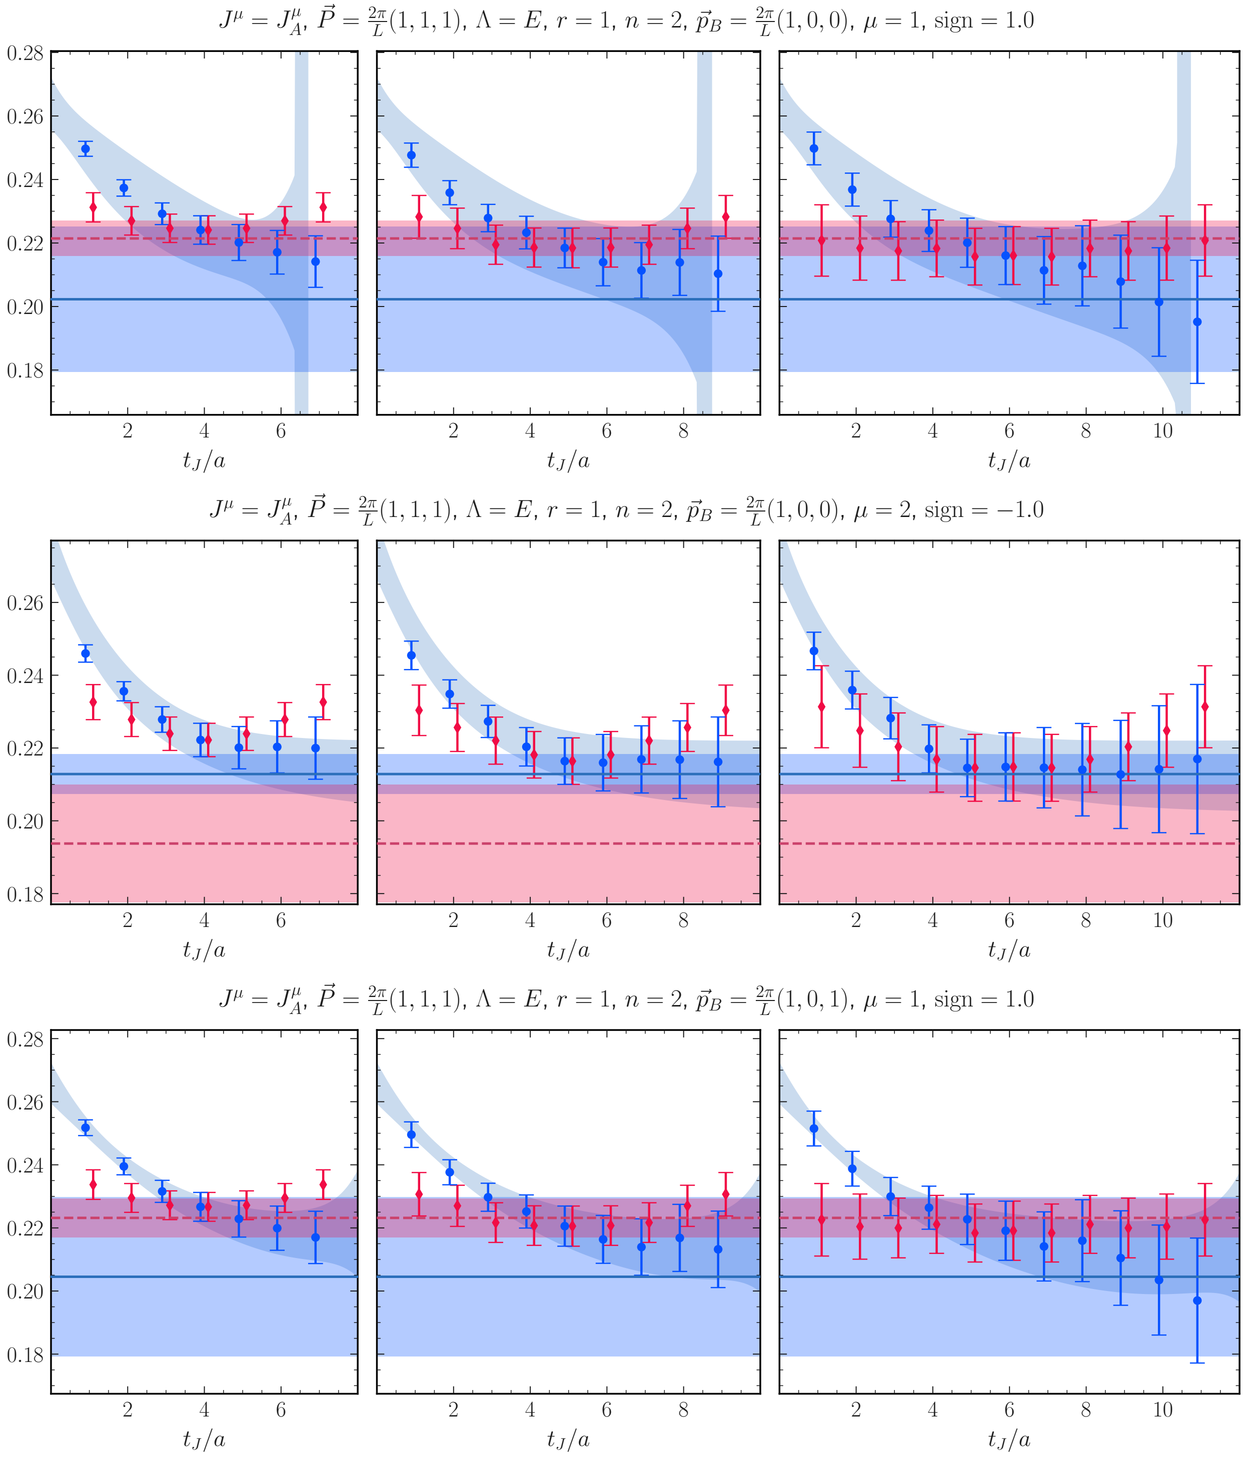
$J^\mu = J^\mu_A$, $\vec{P} = \frac{2\pi}{L}(1,1,1)$, $\Lambda = E$, $r = 1$, $n = 2$, $\vec{p}_B = \frac{2\pi}{L}(1,0,0)$, $\mu = 1$, sign = 1.0
$J^\mu = J^\mu_A$, $\vec{P} = \frac{2\pi}{L}(1,1,1)$, $\Lambda = E$, $r = 1$, $n = 2$, $\vec{p}_B = \frac{2\pi}{L}(1,0,0)$, $\mu = 2$, sign = −1.0
$J^\mu = J^\mu_A$, $\vec{P} = \frac{2\pi}{L}(1,1,1)$, $\Lambda = E$, $r = 1$, $n = 2$, $\vec{p}_B = \frac{2\pi}{L}(1,0,1)$, $\mu = 1$, sign = 1.0
$t_J/a$

$J^\mu = J^\mu_A$, $\vec{P} = \frac{2\pi}{L}(1,1,1)$, $\Lambda = E$, $r = 1$, $n = 2$, $\vec{p}_B = \frac{2\pi}{L}(1,0,1)$, $\mu = 2$, sign $= -1.0$

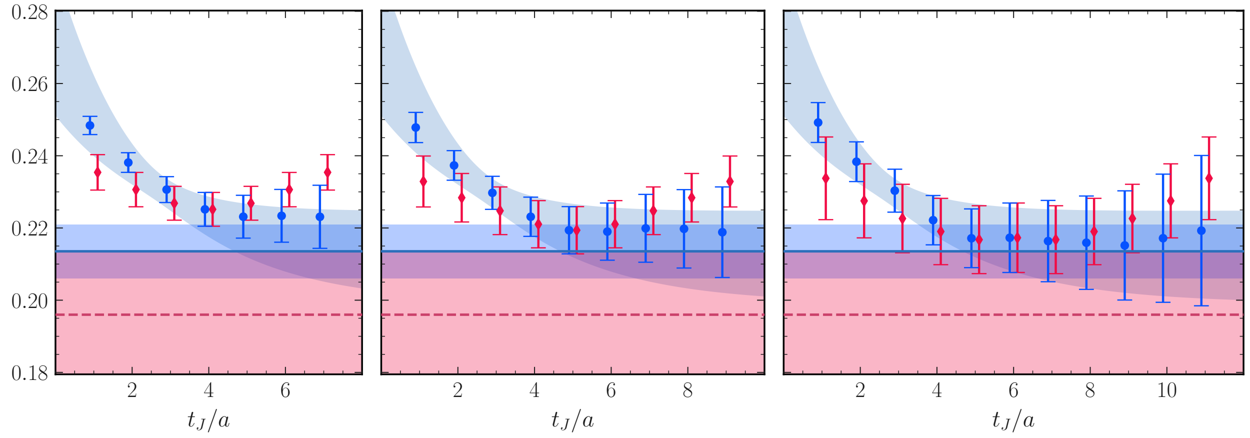


$J^\mu = J^\mu_A$, $\vec{P} = \frac{2\pi}{L}(1,1,1)$, $\Lambda = E$, $r = 1$, $n = 2$, $\vec{p}_B = \frac{2\pi}{L}(1,1,0)$, $\mu = 1$, sign $= 1.0$

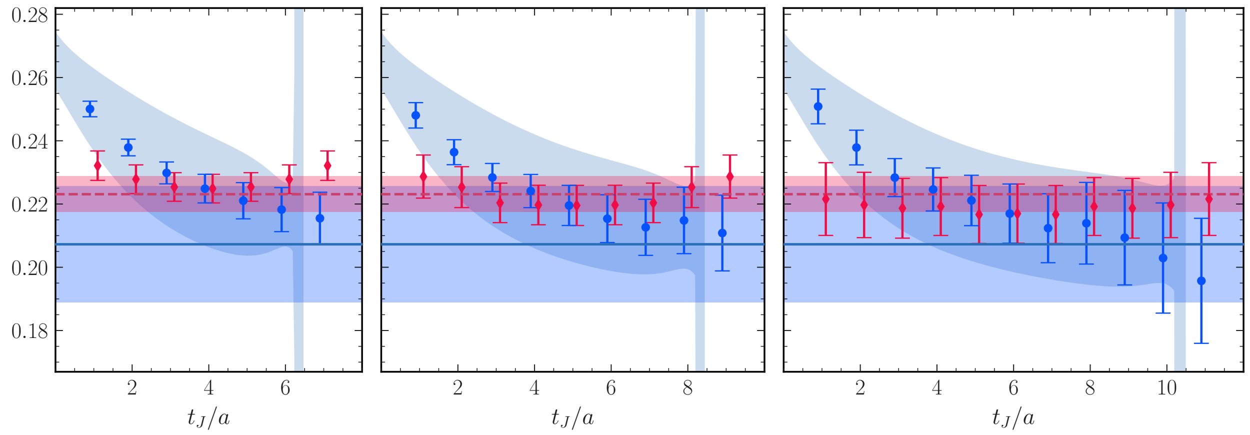


$J^\mu = J^\mu_A$, $\vec{P} = \frac{2\pi}{L}(1,1,1)$, $\Lambda = E$, $r = 1$, $n = 2$, $\vec{p}_B = \frac{2\pi}{L}(1,1,0)$, $\mu = 2$, sign $= -1.0$

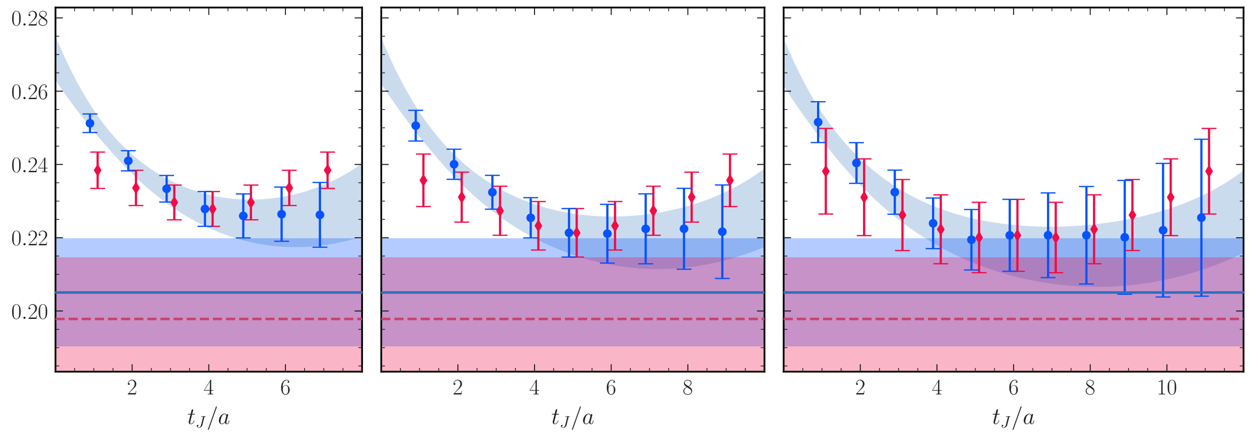

$J^\mu = J_A^\mu$, $\vec{P} = \frac{2\pi}{L}(1,1,1)$, $\Lambda = E$, $r = 1$, $n = 2$, $\vec{p}_B = \frac{2\pi}{L}(1,1,1)$, $\mu = 1$, sign $= 1.0$

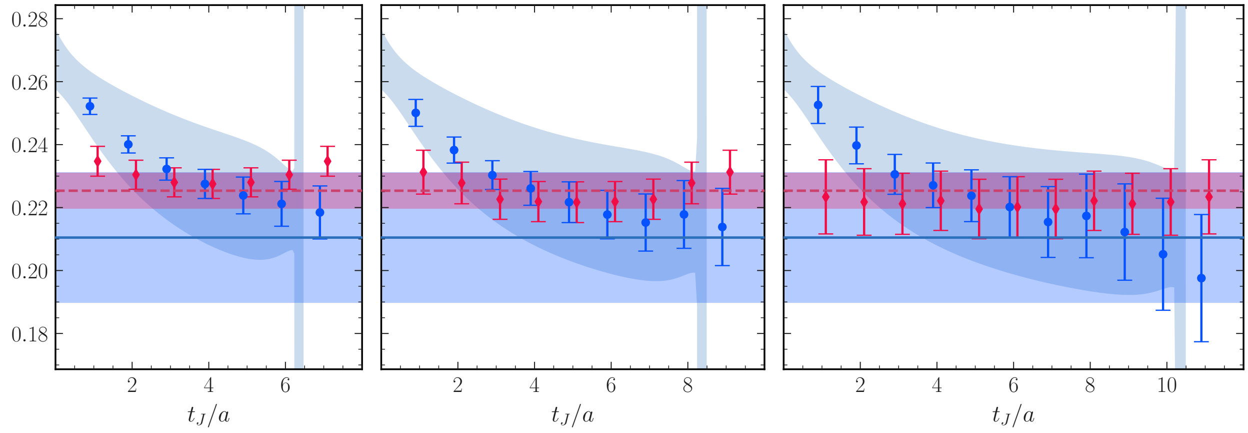


$J^\mu = J_A^\mu$, $\vec{P} = \frac{2\pi}{L}(1,1,1)$, $\Lambda = E$, $r = 1$, $n = 2$, $\vec{p}_B = \frac{2\pi}{L}(1,1,1)$, $\mu = 2$, sign $= -1.0$

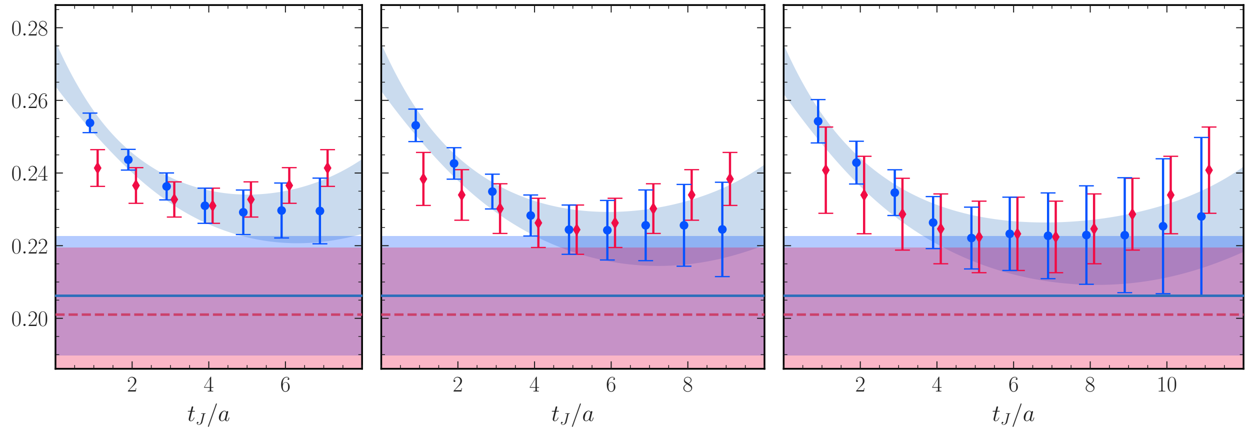


$J^\mu = J_A^\mu$, $\vec{P} = \frac{2\pi}{L}(1,1,1)$, $\Lambda = E$, $r = 2$, $n = 1$, $\vec{p}_B = \frac{2\pi}{L}(0,0,0)$, $\mu = 1$, sign $= 1.0$

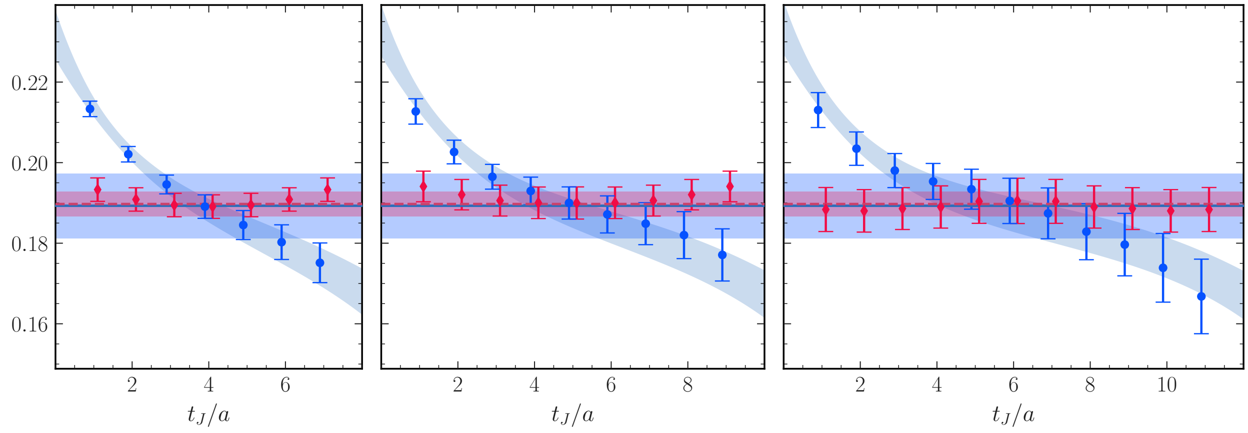

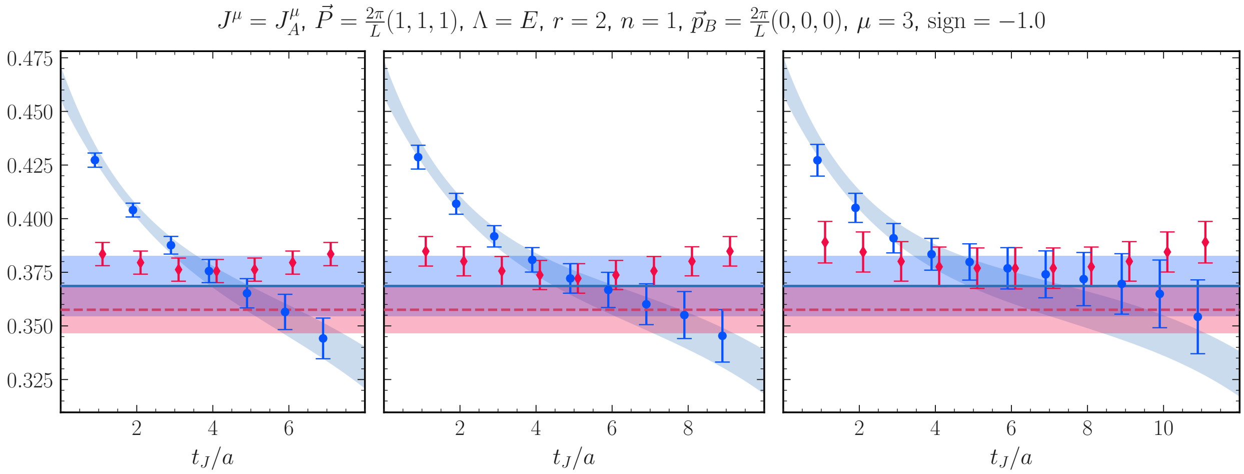
$J^\mu = J_A^\mu$, $\vec{P} = \frac{2\pi}{L}(1,1,1)$, $\Lambda = E$, $r = 2$, $n = 1$, $\vec{p}_B = \frac{2\pi}{L}(0,0,0)$, $\mu = 3$, sign $= -1.0$
0.475
0.450
0.425
0.400
0.375
0.350
0.325
$t_J/a$
$t_J/a$
$t_J/a$

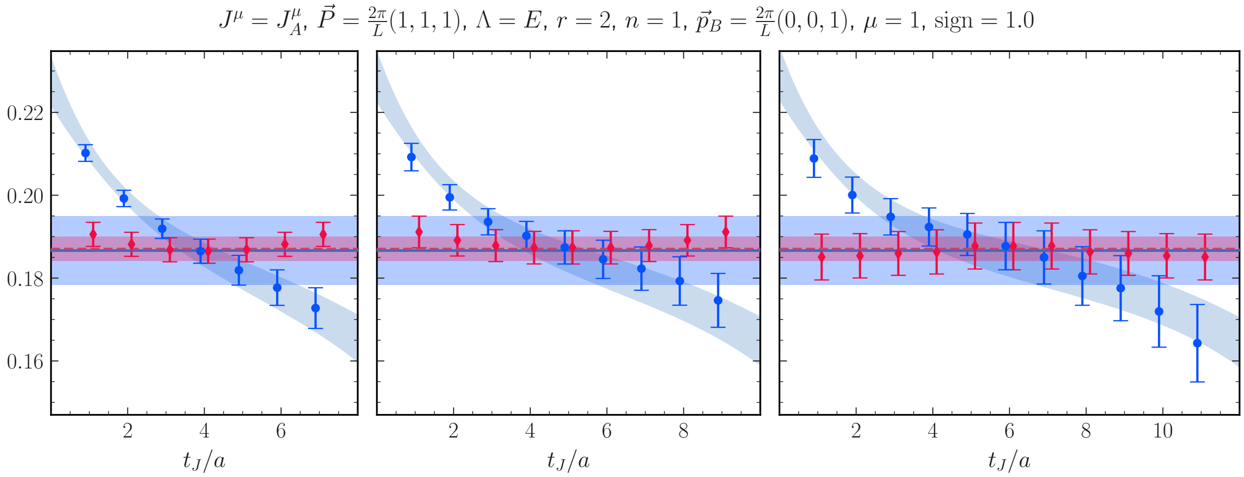
$J^\mu = J_A^\mu$, $\vec{P} = \frac{2\pi}{L}(1,1,1)$, $\Lambda = E$, $r = 2$, $n = 1$, $\vec{p}_B = \frac{2\pi}{L}(0,0,1)$, $\mu = 1$, sign $= 1.0$
0.22
0.20
0.18
0.16
$t_J/a$
$t_J/a$
$t_J/a$

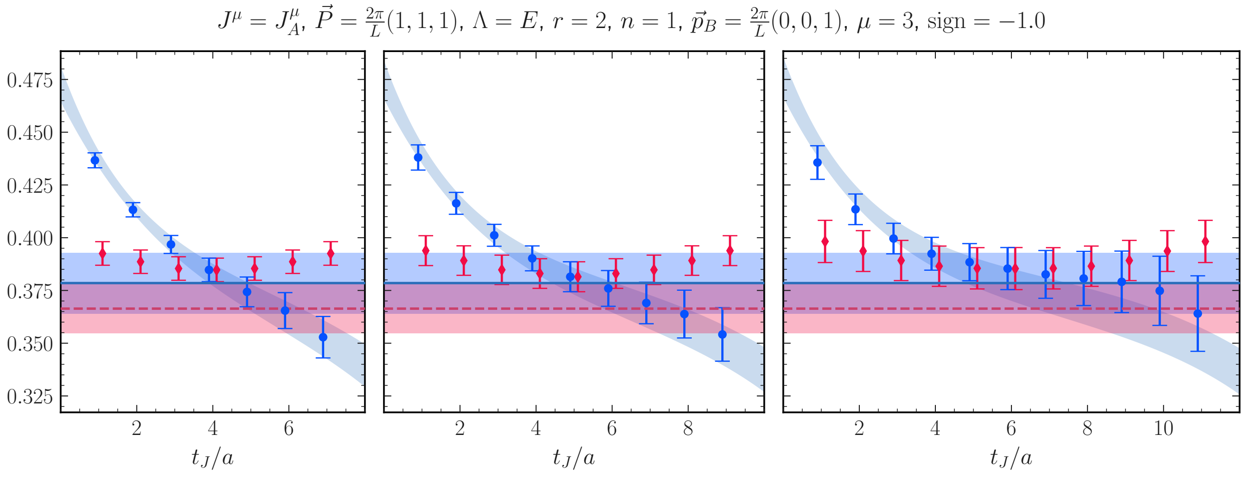
$J^\mu = J_A^\mu$, $\vec{P} = \frac{2\pi}{L}(1,1,1)$, $\Lambda = E$, $r = 2$, $n = 1$, $\vec{p}_B = \frac{2\pi}{L}(0,0,1)$, $\mu = 3$, sign $= -1.0$
0.475
0.450
0.425
0.400
0.375
0.350
0.325
$t_J/a$
$t_J/a$
$t_J/a$

$J^\mu = J^\mu_A$, $\vec{P} = \frac{2\pi}{L}(1,1,1)$, $\Lambda = E$, $r = 2$, $n = 1$, $\vec{p}_B = \frac{2\pi}{L}(0,1,0)$, $\mu = 1$, sign $= 1.0$

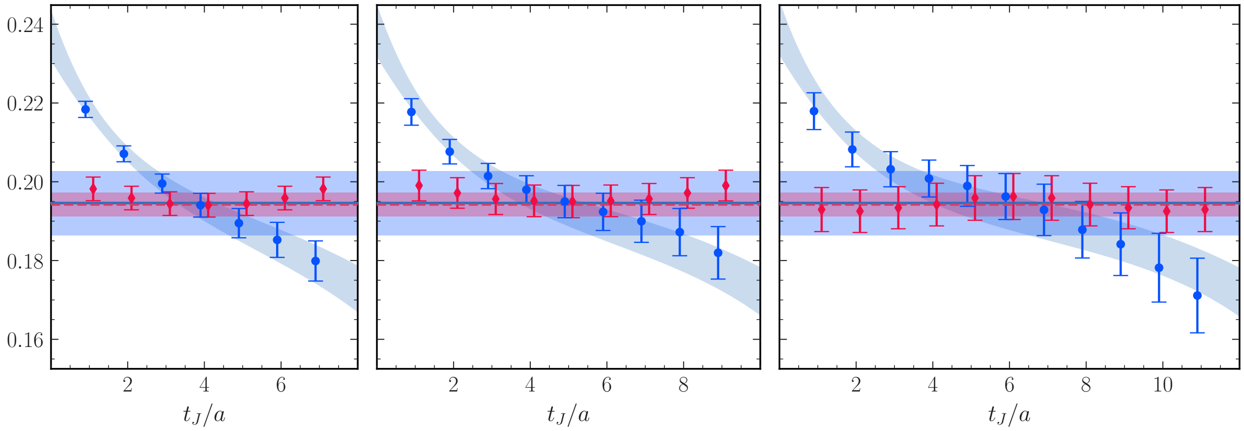


$J^\mu = J^\mu_A$, $\vec{P} = \frac{2\pi}{L}(1,1,1)$, $\Lambda = E$, $r = 2$, $n = 1$, $\vec{p}_B = \frac{2\pi}{L}(0,1,0)$, $\mu = 2$, sign $= 1.0$

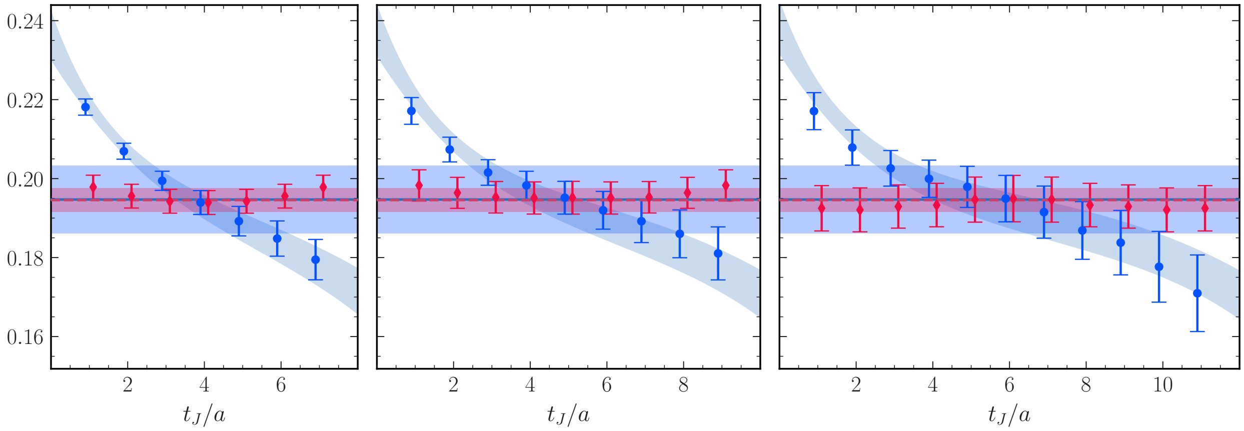


$J^\mu = J^\mu_A$, $\vec{P} = \frac{2\pi}{L}(1,1,1)$, $\Lambda = E$, $r = 2$, $n = 1$, $\vec{p}_B = \frac{2\pi}{L}(0,1,0)$, $\mu = 3$, sign $= -1.0$

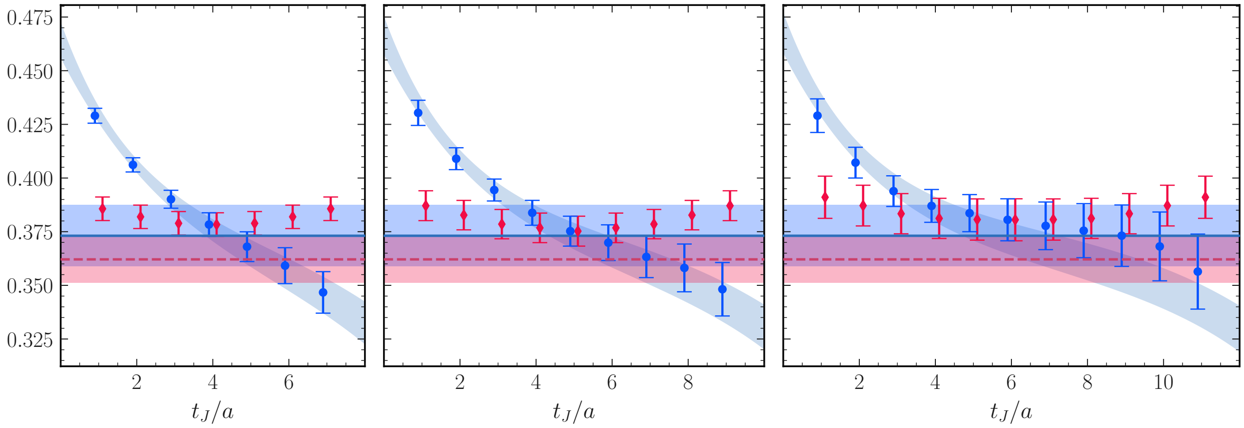

$J^{\mu} = J^{\mu}_{A}$, $\vec{P} = \frac{2\pi}{L}(1,1,1)$, $\Lambda = E$, $r = 2$, $n = 1$, $\vec{p}_B = \frac{2\pi}{L}(0,1,1)$, $\mu = 1$, sign $= 1.0$

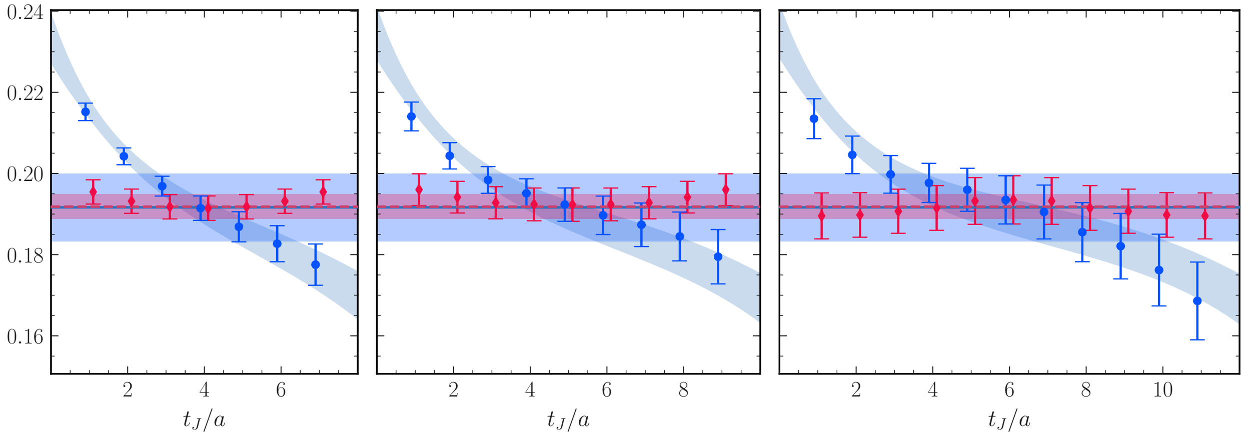


$J^{\mu} = J^{\mu}_{A}$, $\vec{P} = \frac{2\pi}{L}(1,1,1)$, $\Lambda = E$, $r = 2$, $n = 1$, $\vec{p}_B = \frac{2\pi}{L}(0,1,1)$, $\mu = 2$, sign $= 1.0$

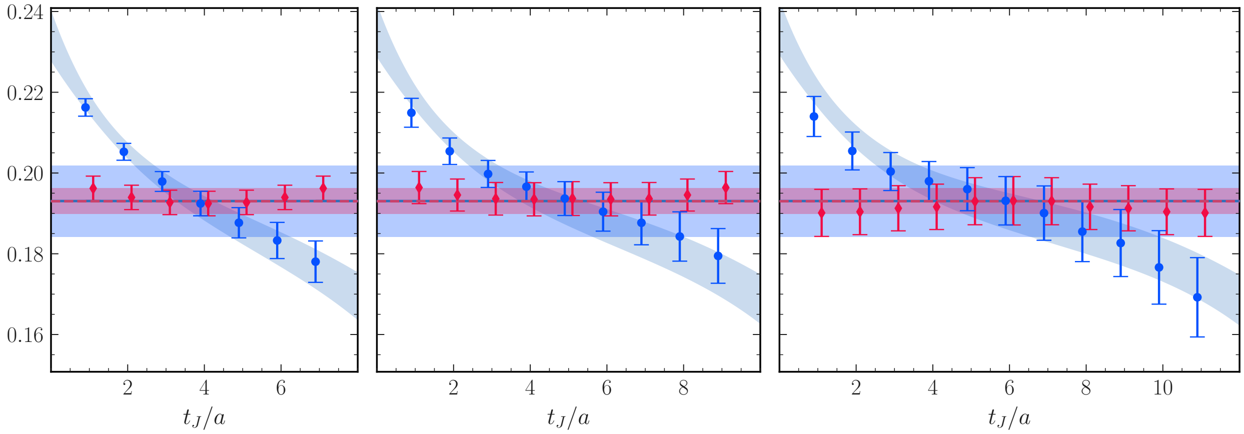


$J^{\mu} = J^{\mu}_{A}$, $\vec{P} = \frac{2\pi}{L}(1,1,1)$, $\Lambda = E$, $r = 2$, $n = 1$, $\vec{p}_B = \frac{2\pi}{L}(0,1,1)$, $\mu = 3$, sign $= -1.0$

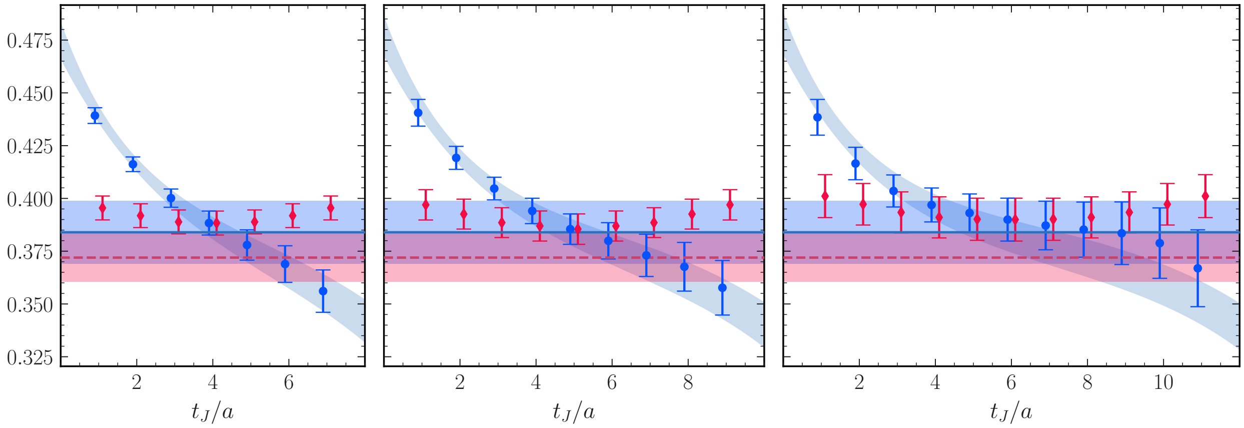

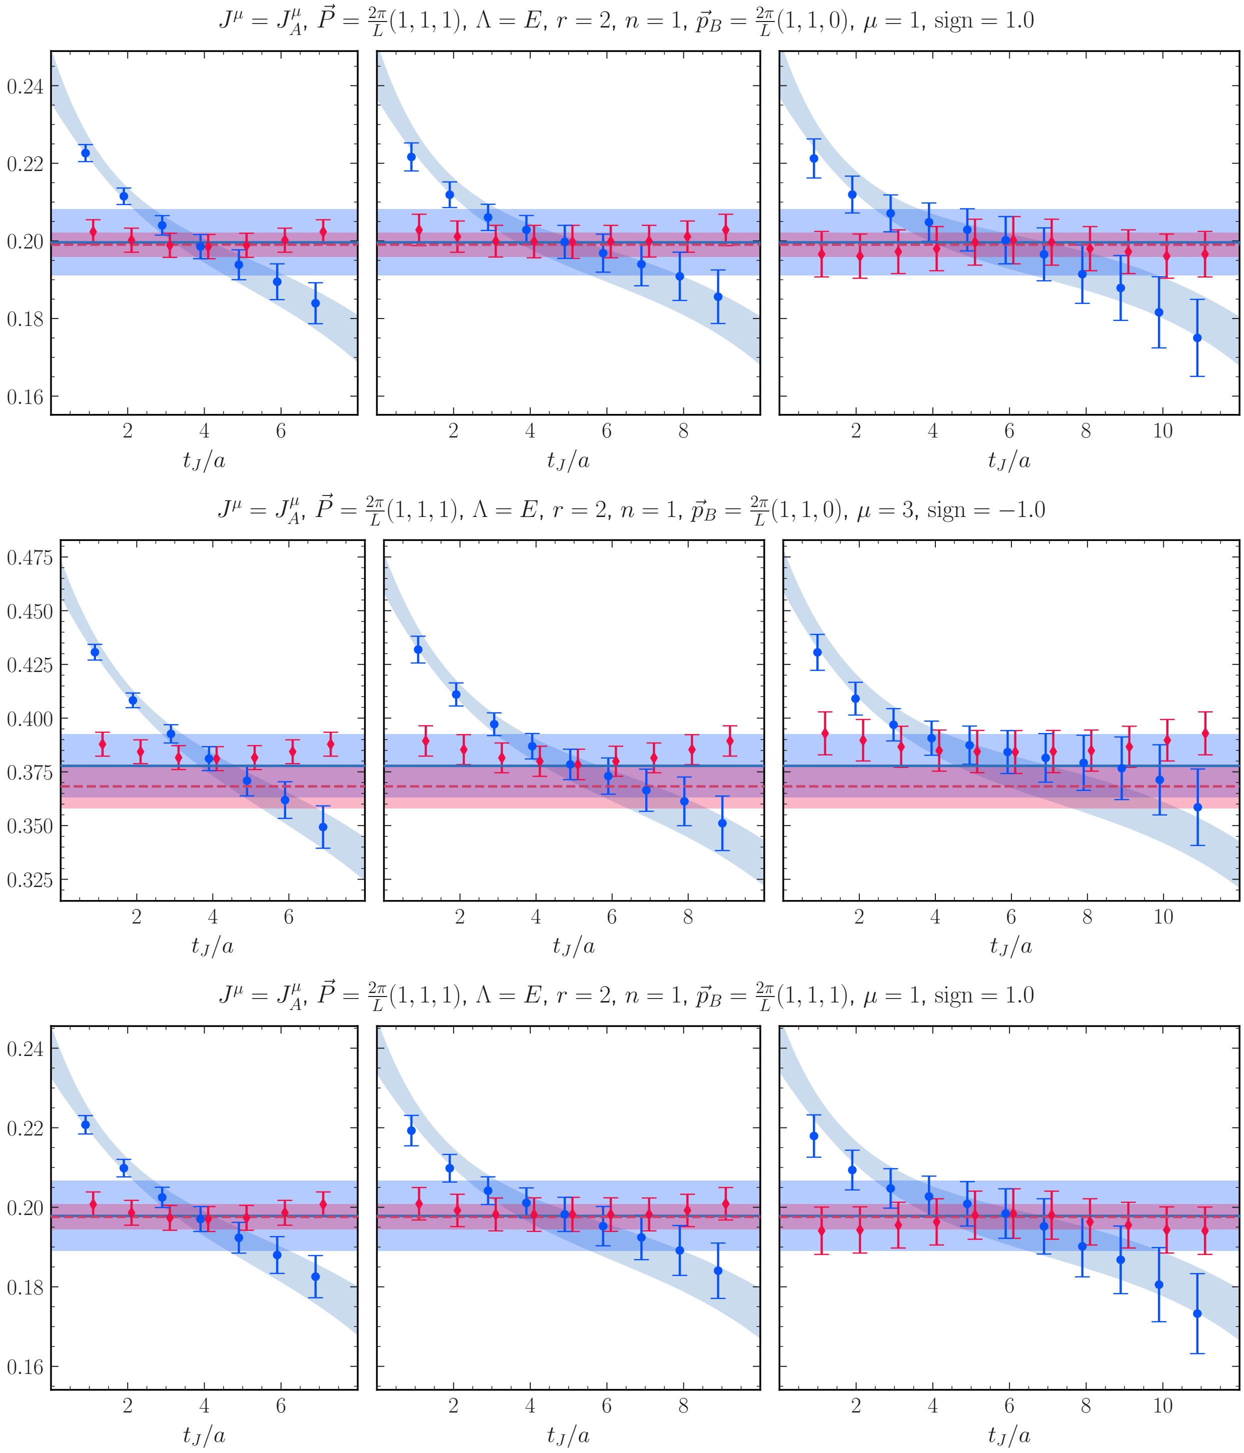

$J^{\mu} = J^{\mu}_{A}$, $\vec{P} = \frac{2\pi}{L}(1,1,1)$, $\Lambda = E$, $r = 2$, $n = 1$, $\vec{p}_B = \frac{2\pi}{L}(1,1,0)$, $\mu = 1$, sign $= 1.0$
$t_J/a$
$J^{\mu} = J^{\mu}_{A}$, $\vec{P} = \frac{2\pi}{L}(1,1,1)$, $\Lambda = E$, $r = 2$, $n = 1$, $\vec{p}_B = \frac{2\pi}{L}(1,1,0)$, $\mu = 3$, sign $= -1.0$
$t_J/a$
$J^{\mu} = J^{\mu}_{A}$, $\vec{P} = \frac{2\pi}{L}(1,1,1)$, $\Lambda = E$, $r = 2$, $n = 1$, $\vec{p}_B = \frac{2\pi}{L}(1,1,1)$, $\mu = 1$, sign $= 1.0$
$t_J/a$

$J^\mu = J_A^\mu$, $\vec{P} = \frac{2\pi}{L}(1,1,1)$, $\Lambda = E$, $r = 2$, $n = 1$, $\vec{p}_B = \frac{2\pi}{L}(1,1,1)$, $\mu = 3$, sign $= -1.0$

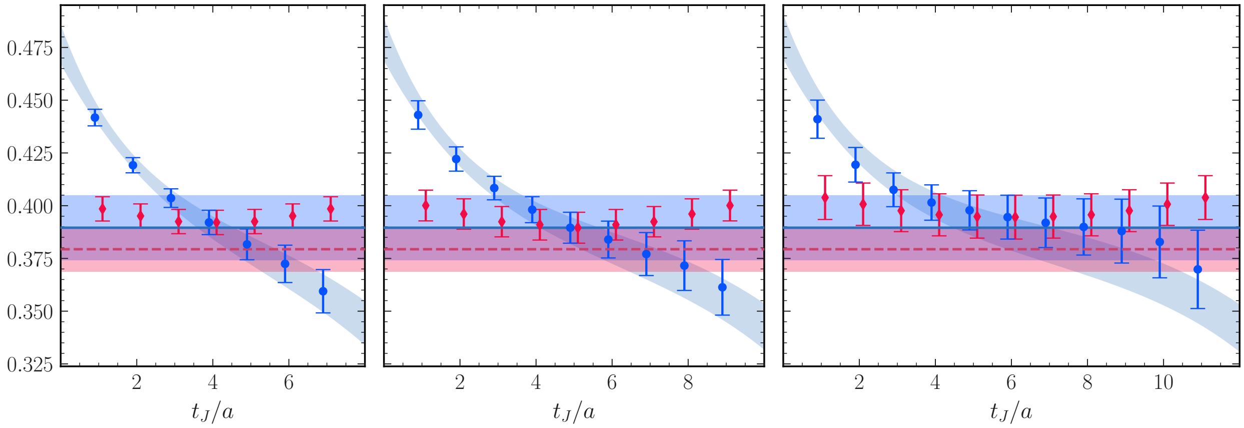


$J^\mu = J_A^\mu$, $\vec{P} = \frac{2\pi}{L}(1,1,1)$, $\Lambda = E$, $r = 2$, $n = 2$, $\vec{p}_B = \frac{2\pi}{L}(0,0,0)$, $\mu = 1$, sign $= 1.0$

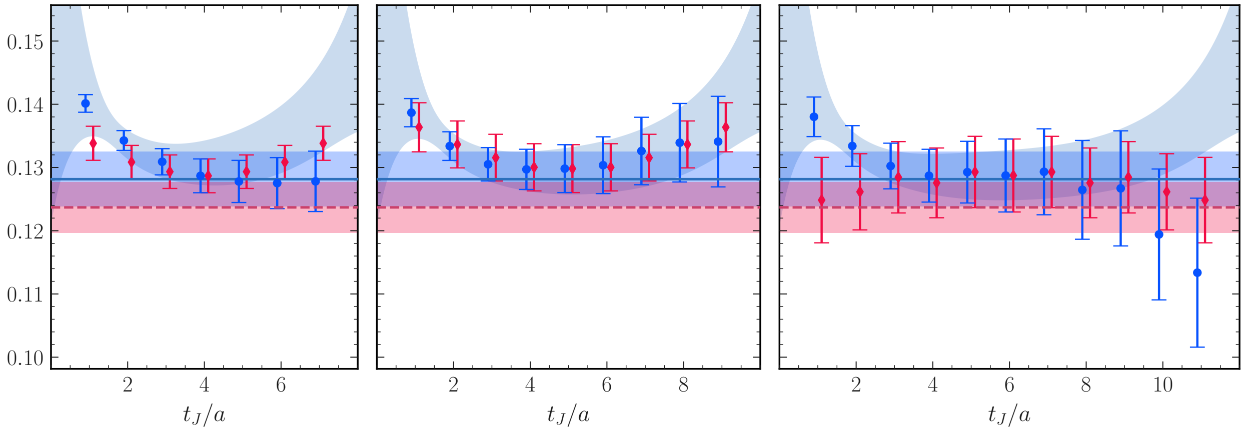


$J^\mu = J_A^\mu$, $\vec{P} = \frac{2\pi}{L}(1,1,1)$, $\Lambda = E$, $r = 2$, $n = 2$, $\vec{p}_B = \frac{2\pi}{L}(0,0,0)$, $\mu = 3$, sign $= -1.0$

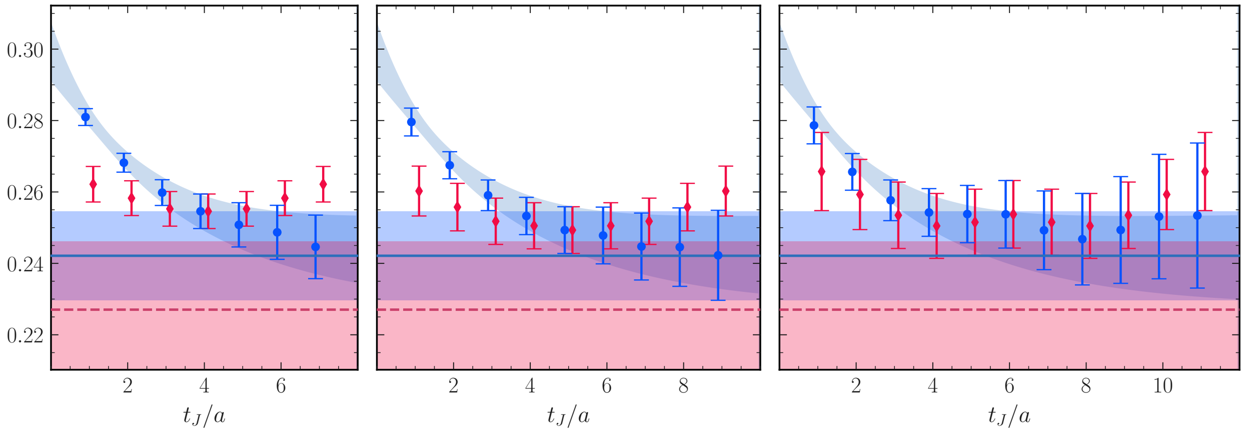

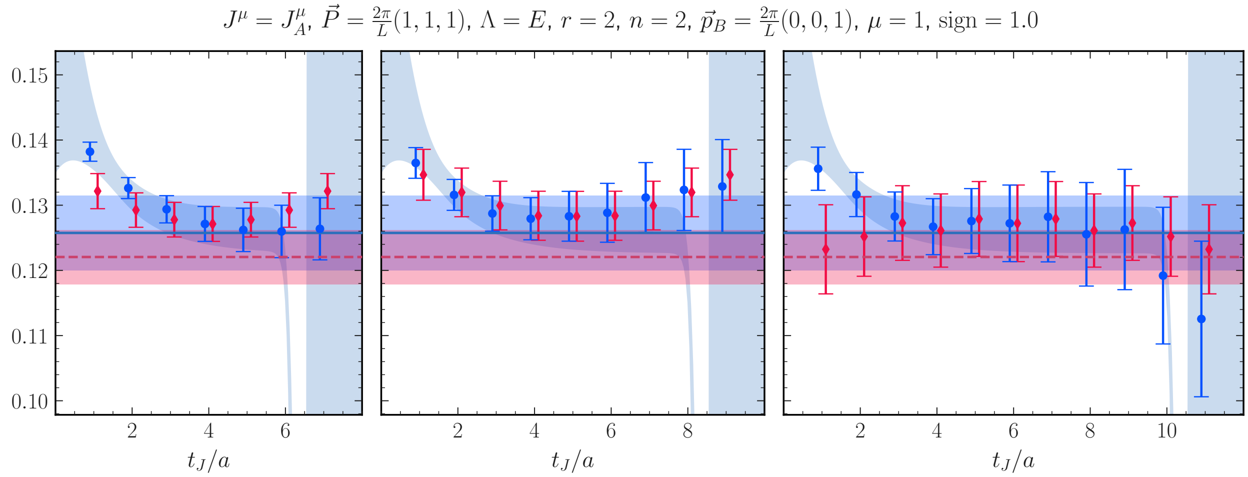

$J^\mu = J_A^\mu$, $\vec{P} = \frac{2\pi}{L}(1,1,1)$, $\Lambda = E$, $r = 2$, $n = 2$, $\vec{p}_B = \frac{2\pi}{L}(0,0,1)$, $\mu = 1$, sign = 1.0
0.15
0.14
0.13
0.12
0.11
0.10
2 4 6 8 10
$t_J/a$


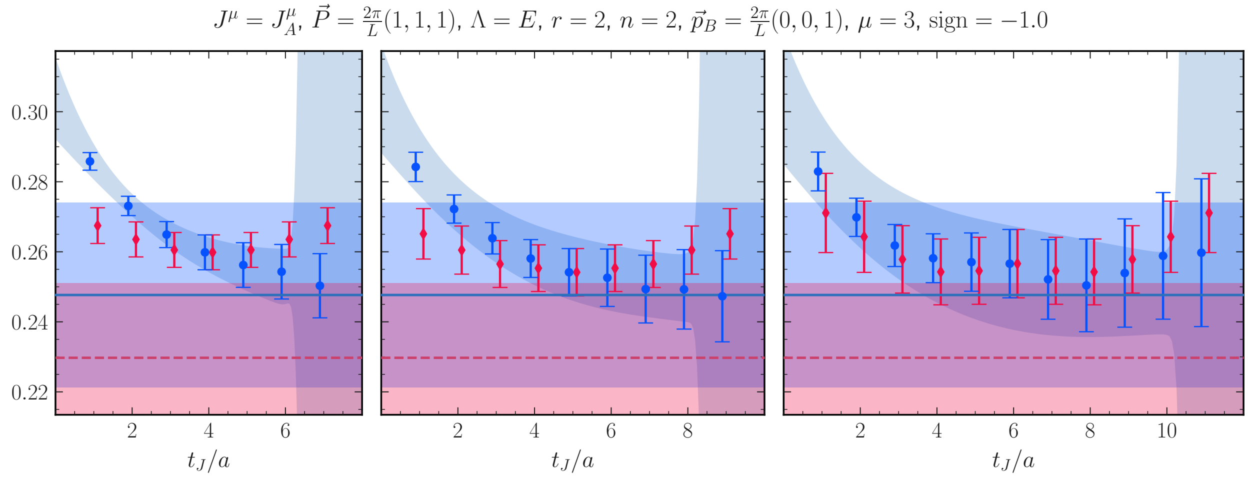

$J^\mu = J_A^\mu$, $\vec{P} = \frac{2\pi}{L}(1,1,1)$, $\Lambda = E$, $r = 2$, $n = 2$, $\vec{p}_B = \frac{2\pi}{L}(0,0,1)$, $\mu = 3$, sign = −1.0
0.30
0.28
0.26
0.24
0.22
2 4 6 8 10
$t_J/a$


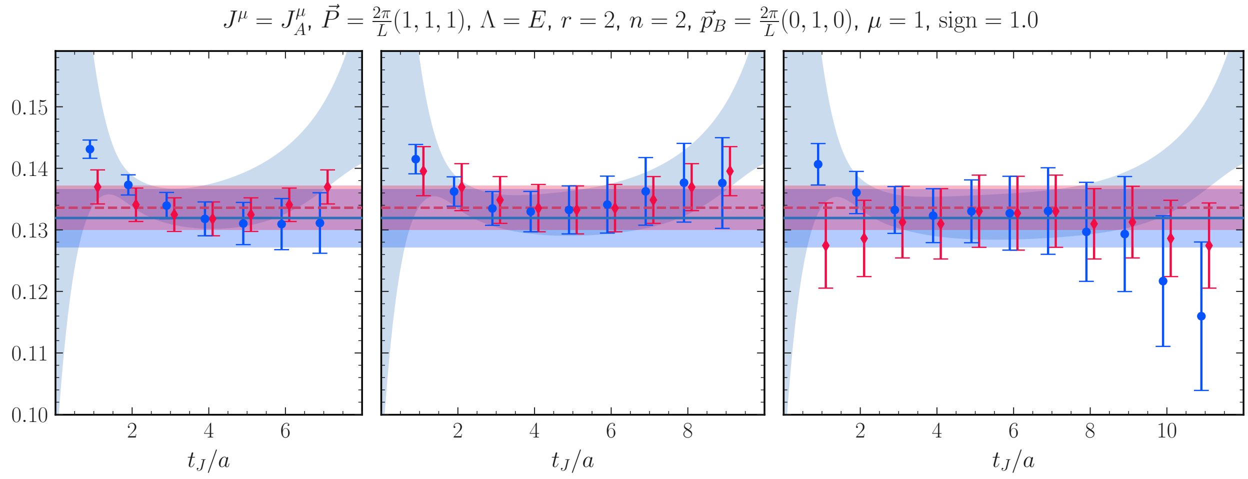

$J^\mu = J_A^\mu$, $\vec{P} = \frac{2\pi}{L}(1,1,1)$, $\Lambda = E$, $r = 2$, $n = 2$, $\vec{p}_B = \frac{2\pi}{L}(0,1,0)$, $\mu = 1$, sign = 1.0
0.15
0.14
0.13
0.12
0.11
0.10
2 4 6 8 10
$t_J/a$

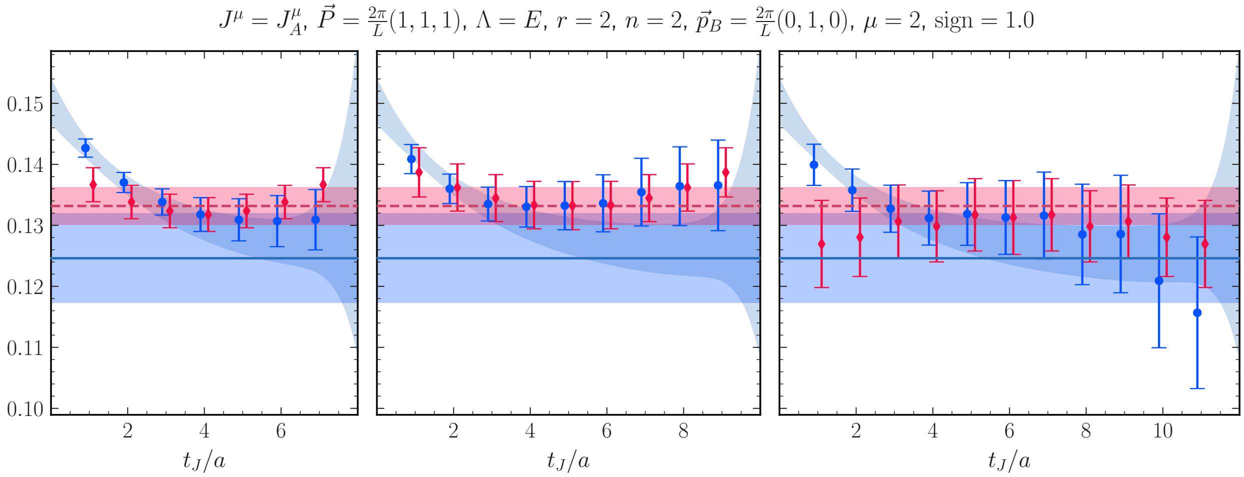
$J^\mu = J^\mu_A$, $\vec{P} = \frac{2\pi}{L}(1,1,1)$, $\Lambda = E$, $r = 2$, $n = 2$, $\vec{p}_B = \frac{2\pi}{L}(0,1,0)$, $\mu = 2$, sign $= 1.0$
0.10
0.11
0.12
0.13
0.14
0.15
$t_J/a$
$t_J/a$
$t_J/a$

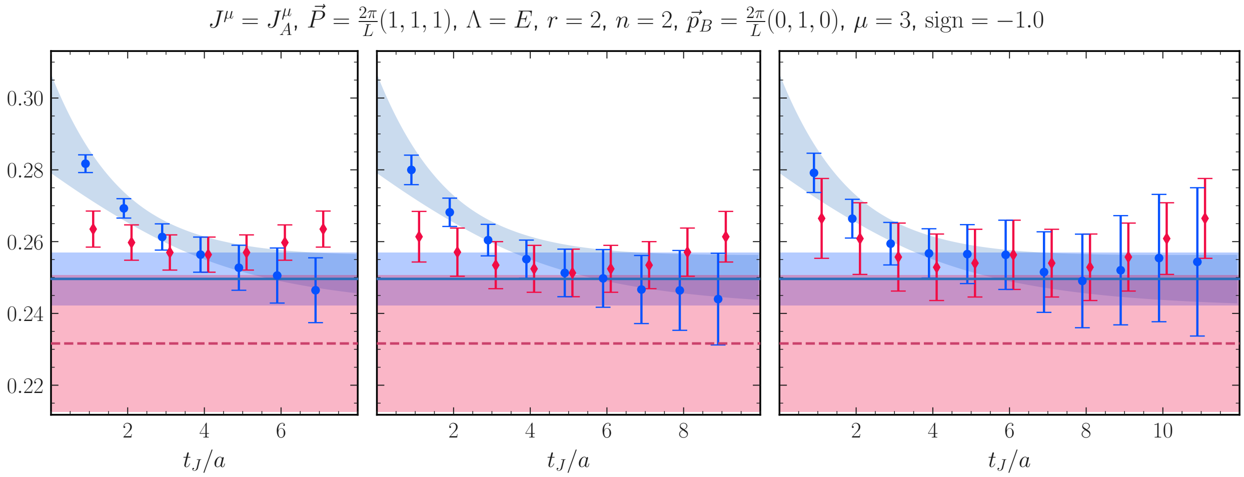
$J^\mu = J^\mu_A$, $\vec{P} = \frac{2\pi}{L}(1,1,1)$, $\Lambda = E$, $r = 2$, $n = 2$, $\vec{p}_B = \frac{2\pi}{L}(0,1,0)$, $\mu = 3$, sign $= -1.0$
0.22
0.24
0.26
0.28
0.30
$t_J/a$
$t_J/a$
$t_J/a$

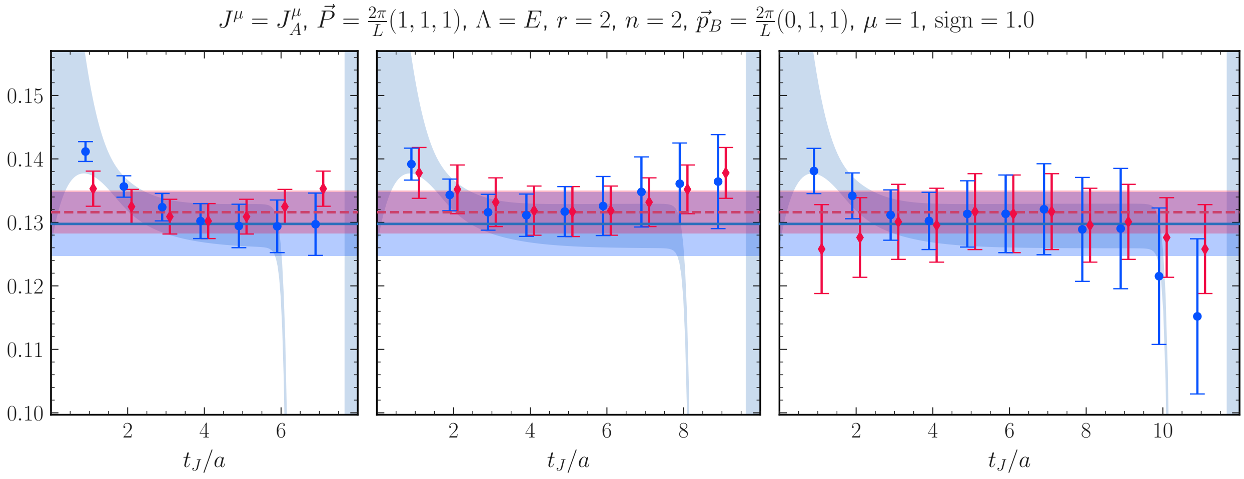
$J^\mu = J^\mu_A$, $\vec{P} = \frac{2\pi}{L}(1,1,1)$, $\Lambda = E$, $r = 2$, $n = 2$, $\vec{p}_B = \frac{2\pi}{L}(0,1,1)$, $\mu = 1$, sign $= 1.0$
0.10
0.11
0.12
0.13
0.14
0.15
$t_J/a$
$t_J/a$
$t_J/a$

$J^\mu = J_A^\mu$, $\vec{P} = \frac{2\pi}{L}(1,1,1)$, $\Lambda = E$, $r = 2$, $n = 2$, $\vec{p}_B = \frac{2\pi}{L}(0,1,1)$, $\mu = 2$, sign $= 1.0$

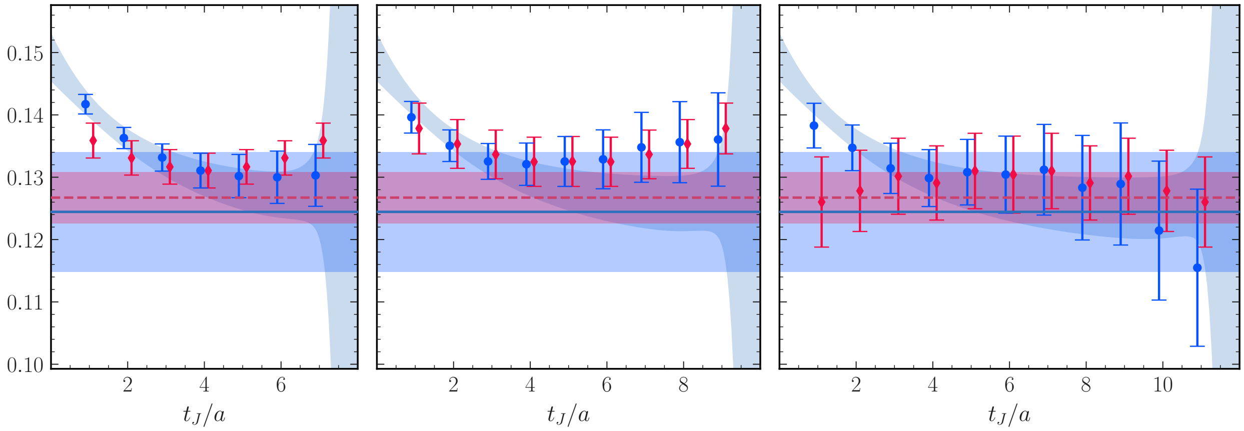


$J^\mu = J_A^\mu$, $\vec{P} = \frac{2\pi}{L}(1,1,1)$, $\Lambda = E$, $r = 2$, $n = 2$, $\vec{p}_B = \frac{2\pi}{L}(0,1,1)$, $\mu = 3$, sign $= -1.0$

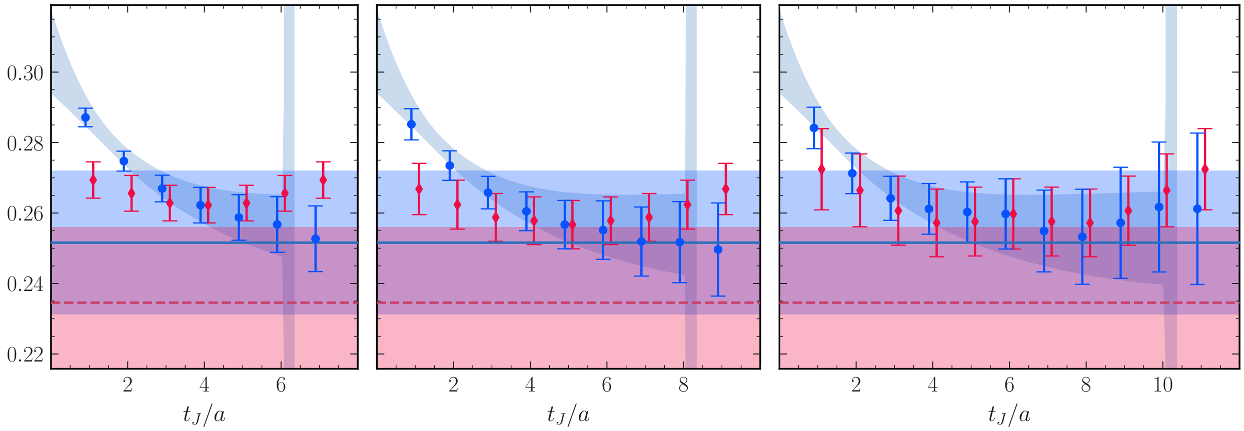


$J^\mu = J_A^\mu$, $\vec{P} = \frac{2\pi}{L}(1,1,1)$, $\Lambda = E$, $r = 2$, $n = 2$, $\vec{p}_B = \frac{2\pi}{L}(1,1,0)$, $\mu = 1$, sign $= 1.0$

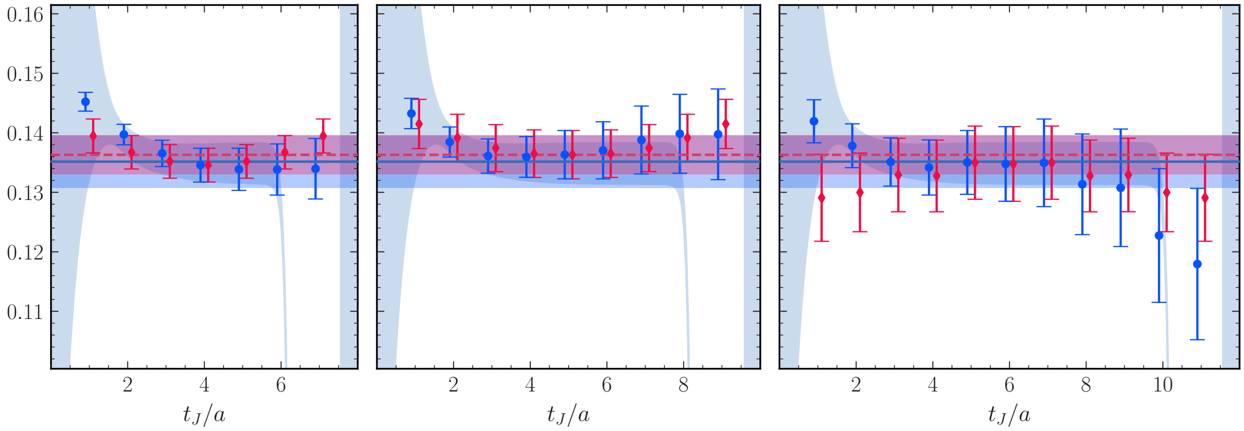

$J^\mu = J_A^\mu$, $\vec{P} = \frac{2\pi}{L}(1,1,1)$, $\Lambda = E$, $r = 2$, $n = 2$, $\vec{p}_B = \frac{2\pi}{L}(1,1,0)$, $\mu = 3$, sign $= -1.0$

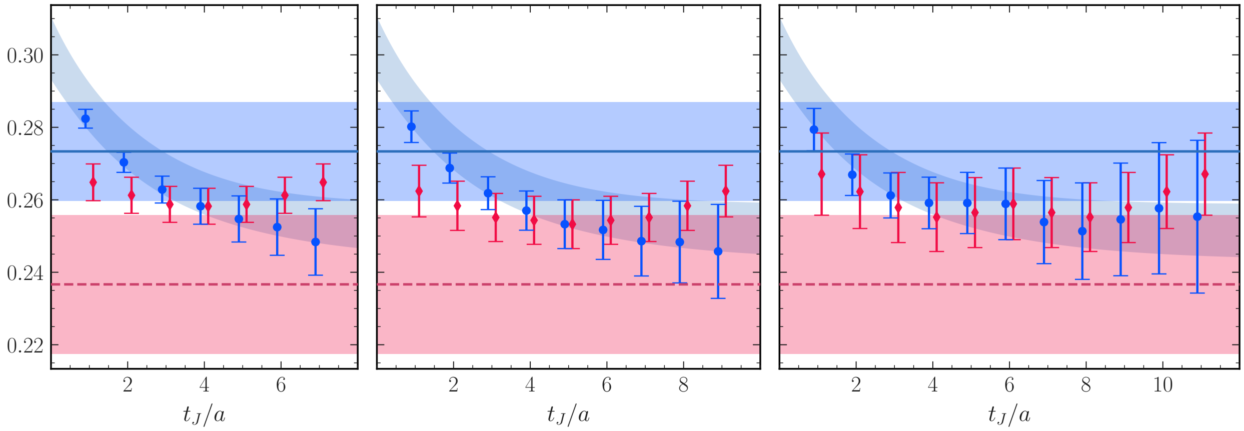


$J^\mu = J_A^\mu$, $\vec{P} = \frac{2\pi}{L}(1,1,1)$, $\Lambda = E$, $r = 2$, $n = 2$, $\vec{p}_B = \frac{2\pi}{L}(1,1,1)$, $\mu = 1$, sign $= 1.0$

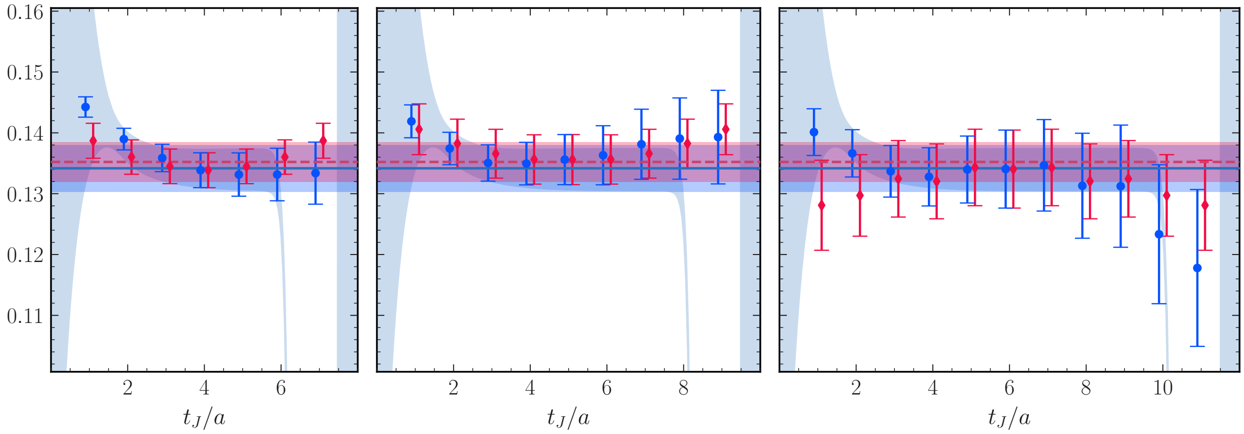


$J^\mu = J_A^\mu$, $\vec{P} = \frac{2\pi}{L}(1,1,1)$, $\Lambda = E$, $r = 2$, $n = 2$, $\vec{p}_B = \frac{2\pi}{L}(1,1,1)$, $\mu = 3$, sign $= -1.0$

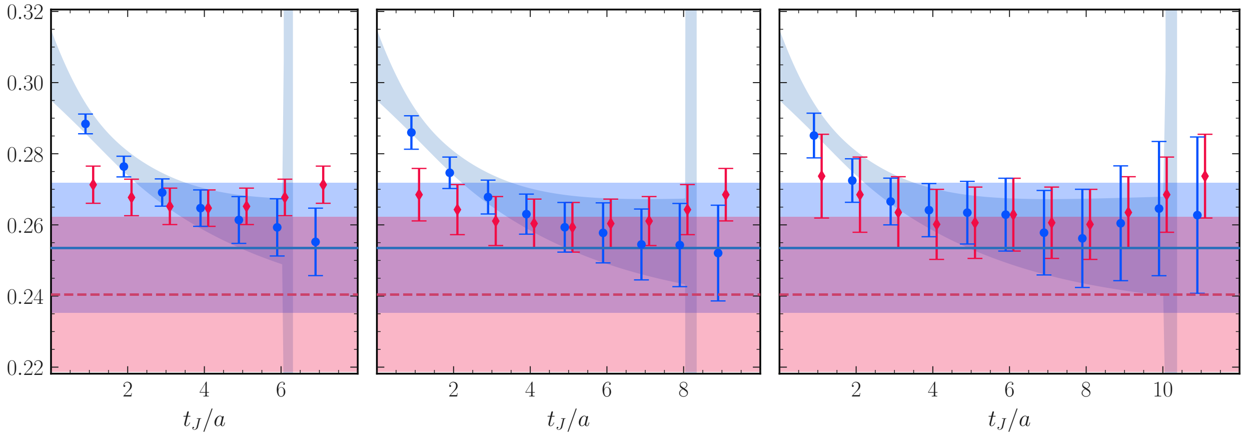

[1] C. Alexandrou, L. Leskovec, S. Meinel, J. Negele, S. Paul, M. Petschlies, A. Pochinsky, G. Rendon, and S. Syritsyn, "$P$-wave $\pi\pi$ scattering and the $\rho$ resonance from lattice QCD," Phys. Rev. D **96** no. 3, (2017) 034525, arXiv:1704.05439 [hep-lat].

[2] K. G. Wilson, "Confinement of Quarks," Phys. Rev. D **10** (1974) 2445–2459.

[3] B. Sheikholeslami and R. Wohlert, "Improved Continuum Limit Lattice Action for QCD with Wilson Fermions," Nucl. Phys. B **259** (1985) 572.

[4] C. Morningstar and M. J. Peardon, "Analytic smearing of SU(3) link variables in lattice QCD," Phys. Rev. D **69** (2004) 054501, arXiv:hep-lat/0311018.

[5] K. Symanzik, "Improved lattice actions for nonlinear $\sigma$ model and nonabelian Gauge theory," in *Workshop on Non-perturbative Field Theory and QCD*. 1983.

[6] K. Symanzik, "Continuum Limit and Improved Action in Lattice Theories. 1. Principles and $\varphi^4$ Theory," Nucl. Phys. B **226** (1983) 187–204.

[7] K. Symanzik, "Continuum Limit and Improved Action in Lattice Theories. 2. O(N) Nonlinear Sigma Model in Perturbation Theory," Nucl. Phys. B **226** (1983) 205–227.

[8] M. Luscher and P. Weisz, "Computation of the Action for On-Shell Improved Lattice Gauge Theories at Weak Coupling," Phys. Lett. B **158** (1985) 250–254.

[9] **HPQCD** Collaboration, C. T. H. Davies, E. Follana, I. D. Kendall, G. P. Lepage, and C. McNeile, "Precise determination of the lattice spacing in full lattice QCD," Phys. Rev. D **81** (2010) 034506, arXiv:0910.1229 [hep-lat].

[10] S. Meinel, "Bottomonium spectrum at order $v^6$ from domain-wall lattice QCD: Precise results for hyperfine splittings," Phys. Rev. D **82** (2010) 114502, arXiv:1007.3966 [hep-lat].

[11] G. P. Lepage, L. Magnea, C. Nakhleh, U. Magnea, and K. Hornbostel, "Improved nonrelativistic QCD for heavy quark physics," Phys. Rev. D **46** (1992) 4052–4067, arXiv:hep-lat/9205007.

[12] P. Chen, "Heavy quarks on anisotropic lattices: The Charmonium spectrum," Phys.Rev. **D64** (2001) 034509, arXiv:hep-lat/0006019 [hep-lat].

[13] A. X. El-Khadra, A. S. Kronfeld, and P. B. Mackenzie, "Massive fermions in lattice gauge theory," Phys.Rev. **D55** (1997) 3933–3957, arXiv:hep-lat/9604004 [hep-lat].

[14] S. Aoki, Y. Kuramashi, and S.-i. Tominaga, "Relativistic heavy quarks on the lattice," Prog.Theor.Phys. **109** (2003) 383–413, arXiv:hep-lat/0107009 [hep-lat].

[15] S. Aoki, Y. Kayaba, and Y. Kuramashi, "A Perturbative determination of mass dependent $O(a)$ improvement coefficients in a relativistic heavy quark action," Nucl.Phys. **B697** (2004) 271–301, arXiv:hep-lat/0309161 [hep-lat].

[16] N. H. Christ, M. Li, and H.-W. Lin, "Relativistic Heavy Quark Effective Action," Phys.Rev. **D76** (2007) 074505, arXiv:hep-lat/0608006 [hep-lat].

[17] H.-W. Lin and N. Christ, "Non-perturbatively Determined Relativistic Heavy Quark Action," Phys.Rev. **D76** (2007) 074506, arXiv:hep-lat/0608005 [hep-lat].

[18] **RBC, UKQCD** Collaboration, Y. Aoki, N. H. Christ, J. M. Flynn, T. Izubuchi, C. Lehner, M. Li, H. Peng, A. Soni, R. S. Van de Water, and O. Witzel, "Nonperturbative tuning of an improved relativistic heavy-quark action with application to bottom spectroscopy," Phys. Rev. D **86** (2012) 116003, arXiv:1206.2554 [hep-lat].

[19] S. Hashimoto, A. X. El-Khadra, A. S. Kronfeld, P. B. Mackenzie, S. M. Ryan, and J. N. Simone, "Lattice QCD calculation of $\bar{B} \to D\ell\bar{\nu}$ decay form-factors at zero recoil," Phys. Rev. D **61** (1999) 014502, arXiv:hep-ph/9906376.

[20] A. X. El-Khadra, A. S. Kronfeld, P. B. Mackenzie, S. M. Ryan, and J. N. Simone, "The Semileptonic decays $B \to \pi\ell\nu$ and $D \to \pi\ell\nu$ from lattice QCD," Phys. Rev. D **64** (2001) 014502, arXiv:hep-ph/0101023.

[21] J. Green, N. Hasan, S. Meinel, M. Engelhardt, S. Krieg, J. Laeuchli, J. Negele, K. Orginos, A. Pochinsky, and S. Syritsyn, "Up, down, and strange nucleon axial form factors from lattice QCD," Phys. Rev. D **95** no. 11, (2017) 114502, arXiv:1703.06703 [hep-lat].

[22] C. Alexandrou, L. Leskovec, S. Meinel, J. Negele, S. Paul, M. Petschlies, A. Pochinsky, G. Rendon, and S. Syritsyn, "$\pi\gamma \to \pi\pi$ transition and the $\rho$ radiative decay width from lattice QCD," Phys. Rev. D **98** no. 7, (2018) 074502, arXiv:1807.08357 [hep-lat]. [Erratum: Phys.Rev.D 105, 019902 (2022)].

[23] S. Gusken, U. Low, K. H. Mutter, R. Sommer, A. Patel, and K. Schilling, "Nonsinglet Axial Vector Couplings of the Baryon Octet in Lattice QCD," Phys. Lett. B **227** (1989) 266–269.

[24] **APE** Collaboration, M. Albanese *et al.*, "Glueball Masses and String Tension in Lattice QCD," Phys. Lett. B **192** (1987) 163–169.
[25] W. I. Jay and E. T. Neil, "Bayesian model averaging for analysis of lattice field theory results," Phys. Rev. D **103** (2021) 114502, arXiv:2008.01069 [stat.ME].
[26] W. Detmold, C. Lehner, and S. Meinel, "$\Lambda_b \to p\ell^-\bar{\nu}_\ell$ and $\Lambda_b \to \Lambda_c\ell^-\bar{\nu}_\ell$ form factors from lattice QCD with relativistic heavy quarks," Phys. Rev. D **92** no. 3, (2015) 034503, arXiv:1503.01421 [hep-lat].
